# Supplementary material for: Adjoint Reactive GUI
Source: arXiv:2010.12338 ancillary file (2020-10-26)
Supplement: Supplementary file 1 [file technical-rapport.pdf]

# Adjoint Reactive Programming

## Technical Appendix

Neel Krishnaswami, Dimitrij Szamozvancev and Christian Graulund

## 1 Types, Terms, Indices and Contexts

In this section we define the types, terms, indices and context of the language.

**Definition 1.1** (Indices). We allow quantification over indices, which are either identifiers or time steps.

$$\sigma ::= \text{id} \mid \text{time}$$

**Definition 1.2** (Types). Two grammars of types: nonlinear types  $X, Y$  and linear types  $A, B$ . As in Benton–Wadler adjoint logic, there are type constructors  $\mathbf{G}$  and  $\mathbf{F}$  to move between the two. We also have  $\forall$ - and  $\exists$ -types which quantify over indices, indexed widget and prefix types, and arbitrary and explicit type delays.

$$\begin{aligned} X, Y &::= 1 \mid X \rightarrow Y \mid \mathbf{G} A \\ A, B &::= \mathbf{l} \mid A \otimes B \mid A \multimap B \mid \mathbf{F} X \mid \forall i: \sigma. A \mid \exists i: \sigma. A \\ &\mid \text{Widget}^\ell \mid \text{Prefix}^\ell(\tau) \mid \Diamond A \mid A @ \tau \end{aligned}$$

**Definition 1.3** (Contexts). Standard nonlinear contexts  $\Gamma$ , linear, time-indexed context  $\Delta$  and (identifier- or time-) index context  $\Theta$ .

$$\begin{aligned} \Gamma &::= \cdot \mid \Gamma, x: X \\ \Delta &::= \cdot \mid \Delta, a:_{\tau} A \\ \Theta &::= \cdot \mid \Theta, i: \sigma \end{aligned}$$

As we often need to split or combine linear contexts, we overload the context extension operator to also work as context concatenation, writing  $\Delta, \Delta'$  to mean that we repeatedly add variables from  $\Delta'$  to  $\Delta$  to create a unified context:

$$\begin{aligned} \Delta, \cdot &= \Delta \\ \Delta, (\Delta', a:_{\tau} A) &= (\Delta, \Delta'), a:_{\tau} A \end{aligned}$$

**Definition 1.4** (Terms). Index terms  $s$ , Cartesian terms  $e$  and linear terms  $t$ , with standard constructor-destructor terms for functions, units, pairs, events, universal and existential quantification of indices, time delay and the adjoint pair  $\mathbf{G}$  and  $\mathbf{F}$ . There is also a term **select** for temporal branching, and bindings for  $\tau$ -delayed unit and pair terms.

$$s ::= i \mid \tau \mid \iota$$

$$\begin{aligned}
e &::= x \mid \lambda x. e \mid e_1 e_2 \mid \bullet \mid \mathbf{G} \, t \\
t &::= a \mid \lambda a. t \mid t_1 t_2 \mid \langle \rangle \mid \text{let } \langle \rangle = t_1 \text{ in } t_2 \mid (t_1, t_2) \mid \text{let } (a, b) = t_1 \text{ in } t_2 \\
&\mid t @ s \mid \text{let } a @ s = t_1 \text{ in } t_2 \mid \text{runG } e \mid \mathbf{F} \, e \mid \text{let } \mathbf{F} \, a = t_1 \text{ in } t_2 \\
&\mid \text{evt } t \mid \text{let evt } a = t_1 \text{ in } t_2 \mid \Lambda s : \sigma. t \mid s_i \mid \{s, t\} \mid \text{let } \{s, a\} = t_1 \text{ in } t_2 \\
&\mid \text{select } (t_1, t_2) \text{ as } [a \mapsto t'_1] \parallel [b \mapsto t'_2] \mid \text{let } \langle \rangle_\tau = t_1 \text{ in } t_2 \mid \text{let } (a, b)_\tau = t_1 \text{ in } t_2
\end{aligned}$$

**Definition 1.5** (Context delay). The context delay operation shifts a linear context of  $\tau$ -delayed variables by  $\tau$ . If any of the time indices in  $\Delta$  are not equal to  $\tau$ , the function is undefined (and therefore it implicitly acts both as a predicate and a context transformation).

$$\begin{aligned}
\cdot \downarrow^\tau &= \cdot \\
(\Delta, a :_\tau A) \downarrow^\tau &= \Delta \downarrow^\tau, a : A
\end{aligned}$$

**Lemma 1.6** (Splitting delayed contexts). Given a pair of linear contexts  $\Delta_1, \Delta_2$ , if  $(\Delta_1, \Delta_2) \downarrow^\tau = \Delta'$  for some  $\tau$  and  $\Delta'$ , there exist  $\Delta'_1$  and  $\Delta'_2$  such that  $\Delta'_1, \Delta'_2 = \Delta'$ ,  $\Delta_1 \downarrow^\tau = \Delta'_1$  and  $\Delta_2 \downarrow^\tau = \Delta'_2$ .

*Proof.* By induction, we know that  $(\Delta_1, \Delta_2) \downarrow^\tau = (\Delta_1 \downarrow^\tau, \Delta_2 \downarrow^\tau)$ , and hence by assumption we have

$$(\Delta_1 \downarrow^\tau, \Delta_2 \downarrow^\tau) = \Delta'.$$

Hence, we chose  $\Delta'_1 = \Delta_1 \downarrow^\tau$  and  $\Delta'_2 = \Delta_2 \downarrow^\tau$  and we are done.  $\square$

## 1.1 Typing rules

**Definition 1.7** (Index judgements). Given an index context  $\Theta$ , we define an index judgment, written  $\Theta \vdash_s s : \sigma$ , by the following rules:

$$\begin{array}{ccc}
\frac{\tau \in \text{Time}}{\Theta \vdash_s \tau : \text{time}} \text{TIME} & \frac{\iota \in \text{Id}}{\Theta \vdash_s \iota : \text{id}} \text{ID} & \frac{s : \sigma \in \Theta}{\Theta \vdash_s s : \sigma} \text{VAR}
\end{array}$$

where Time denotes the natural numbers, and Id is any countable set of identifiers (such as pointer addresses).

**Definition 1.8** (Well-formed types). Given an index context  $\Theta$ , we define the judgments  $\Theta \vdash_c X \text{ type}$  and  $\Theta \vdash_\ell A \text{ type}$  for well-formed Cartesian and linear types.

$$\begin{array}{l}
\frac{}{\Theta \vdash_c 1 \text{ type}} (1) \quad \frac{\Theta \vdash_c X \text{ type} \quad \Theta \vdash_c Y \text{ type}}{\Theta \vdash_c X \rightarrow Y \text{ type}} (\rightarrow) \quad \frac{\Theta \vdash_\ell A \text{ type}}{\Theta \vdash_c \mathbf{G} A \text{ type}} (\mathbf{G}) \quad \frac{}{\Theta \vdash_\ell \mathbf{I} \text{ type}} (\mathbf{I}) \\
\frac{\Theta \vdash_\ell A \text{ type} \quad \Theta \vdash_\ell B \text{ type}}{\Theta \vdash_\ell A \multimap B \text{ type}} (\multimap) \quad \frac{\Theta \vdash_\ell A \text{ type} \quad \Theta \vdash_\ell B \text{ type}}{\Theta \vdash_\ell A \otimes B \text{ type}} (\otimes) \quad \frac{\Theta \vdash_\ell A \text{ type}}{\Theta \vdash_\ell \diamond A \text{ type}} (\diamond) \\
\frac{\Theta \vdash \tau : \text{time} \quad \Theta \vdash_\ell A \text{ type}}{\Theta \vdash_\ell A @ \tau \text{ type}} (@) \quad \frac{\Theta \vdash_c X \text{ type}}{\Theta \vdash_\ell \mathbf{F} X \text{ type}} (\mathbf{F}) \quad \frac{\Theta, s : \sigma \vdash_\ell A \text{ type}}{\Theta \vdash_\ell \forall s : \sigma. A \text{ type}} (\forall) \\
\frac{\Theta, s : \sigma \vdash_\ell A \text{ type}}{\Theta \vdash_\ell \exists s : \sigma. A \text{ type}} (\exists) \quad \frac{\Theta \vdash_s \iota : \text{id}}{\Theta \vdash_\ell \text{Widget}^\iota \text{ type}} (\text{WIDGET}) \quad \frac{\Theta \vdash_s \tau : \text{time} \quad \Theta \vdash_s \iota : \text{id}}{\Theta \vdash_\ell \text{Prefix}^\iota(\tau) \text{ type}} (\text{PREFIX})
\end{array}$$

**Definition 1.9** (Well-formed Cartesian context). We define a Cartesian context  $\Gamma$  to be well-formed over an index context  $\Theta$ , written  $\Theta \vdash_c \Gamma$ , by the following rules

$$\frac{}{\Theta \vdash_c \cdot} \quad \frac{\Theta \vdash_c \Gamma \quad x \notin \text{dom}(\Gamma) \quad \Theta \vdash_c X \text{ type}}{\Theta \vdash_c \Gamma, x : X}$$

**Definition 1.10** (Well-formed linear context). We define a linear context  $\Delta$  to be well-formed over an index context  $\Theta$ , written  $\Theta \vdash_\ell \Delta$ , by the following rules

$$\frac{}{\Theta \vdash_\ell \cdot} \quad \frac{\Theta \vdash_\ell \Delta \quad x \notin \text{dom}(\Delta) \quad \Theta \vdash_\ell A \text{ type} \quad \Theta \vdash_s \tau : \text{time}}{\Theta \vdash_\ell \Delta, a :_\tau A}$$

**Definition 1.11** (Cartesian term typing rules). We define the Cartesian judgement  $\vdash_c$  given both an index and a Cartesian context:

$$\begin{array}{ccc} \frac{}{\Theta \mid \Gamma \vdash_c \bullet : 1} \text{ (1-I)} & \frac{x : A \in \Gamma}{\Theta \mid \Gamma \vdash_c x : A} \text{ (VAR)} & \frac{\Theta \mid \Gamma, x : X \vdash_c e : Y}{\Theta \mid \Gamma \vdash_c \lambda x. e : X \rightarrow Y} \text{ (}\rightarrow\text{-I)} \\[10pt] \frac{\Theta \mid \Gamma \vdash_c e_1 : X \rightarrow Y \quad \Theta \mid \Gamma \vdash_c e_2 : X}{\Theta \mid \Gamma \vdash_c e_1 e_2 : Y} \text{ (}\rightarrow\text{-E)} & & \frac{\Theta \mid \Gamma; \cdot \vdash_\ell t : A}{\Theta \mid \Gamma \vdash_c \mathsf{G} t : \mathsf{G} A} \text{ (G-I)} \end{array}$$

**Definition 1.12** (Linear term typing rules). Linear typing judgments can be indexed by the time when typability is checked. Hence, the linear judgment  $\Theta \mid \Gamma; \Delta \vdash_\ell t :_\tau A$  is read as “In the index context  $\Theta$ , Cartesian context  $\Gamma$  and linear context  $\Delta$ , the linear term  $t$  has type  $A$  at time  $\tau$ ”. We also have a separate linear judgement without a time index; semantically,  $\Theta \mid \Gamma; \Delta \vdash_\ell t : A$  is the same as  $\Theta \mid \Gamma; \Delta \vdash_\ell t :_0 A$ , but syntactically they are differentiated so the (delay) rule cannot be repeated arbitrarily.

$$\begin{array}{c}
\text{(VAR)} \frac{}{\Theta \mid \Gamma; a : A \vdash_\ell a : A} \quad \frac{\Theta \mid \Gamma; \Delta, a : A \vdash_\ell t : B}{\Theta \mid \Gamma; \Delta \vdash_\ell \lambda a. t : A \multimap B} \text{ (}\multimap\text{-I)} \quad \frac{\Theta \mid \Gamma; \Delta_1 \vdash_\ell t_1 : A \multimap B \quad \Theta \mid \Gamma; \Delta_2 \vdash_\ell t_2 : A}{\Theta \mid \Gamma; \Delta_1, \Delta_2 \vdash_\ell t_1 t_2 : B} \text{ (}\multimap\text{-E)} \\
\\
\text{(I-I)} \frac{}{\Theta \mid \Gamma; \cdot \vdash_\ell \langle \rangle : \mathbb{I}} \quad \frac{\Theta \mid \Gamma; \Delta_1 \vdash_\ell t_1 : \mathbb{I} \quad \Theta \mid \Gamma; \Delta_2 \vdash_\ell t_2 : C}{\Theta \mid \Gamma; \Delta_1, \Delta_2 \vdash_\ell \text{let } \langle \rangle = t_1 \text{ in } t_2 : C} \text{ (I-E)} \\
\\
\text{(\otimes-I)} \frac{\Theta \mid \Gamma; \Delta_1 \vdash_\ell t_1 : A \quad \Theta \mid \Gamma; \Delta_2 \vdash_\ell t_2 : B}{\Theta \mid \Gamma; \Delta_1 \Delta_2 \vdash_\ell (t_1, t_2) : A \otimes B} \quad \frac{\Theta \mid \Gamma; \Delta_1 \vdash_\ell t_1 : A \otimes B \quad \Theta \mid \Gamma; \Delta_2, a : A, b : B \vdash_\ell t_2 : C}{\Theta \mid \Gamma; \Delta_1, \Delta_2 \vdash_\ell \text{let } (a, b) = t_1 \text{ in } t_2 : C} \text{ (}\otimes\text{-E)} \\
\\
\text{(\diamond-I)} \frac{\Theta \mid \Gamma; \Delta \vdash_\ell t : A}{\Theta \mid \Gamma; \Delta \vdash_\ell \text{evt } t : \diamond A} \quad \frac{\Theta \mid \Gamma; \Delta \vdash_\ell t_1 : \diamond A \quad \Theta \mid \Gamma; a : A \vdash_\ell t_2 : \diamond B}{\Theta \mid \Gamma; \Delta \vdash_\ell \text{let evt } a = t_1 \text{ in } t_2 : \diamond B} \text{ (}\diamond\text{-E)} \\
\\
\text{(@-I)} \frac{\Theta \vdash \tau : \text{time} \quad \Theta \mid \Gamma; \Delta \vdash_\ell t :_\tau A}{\Theta \mid \Gamma; \Delta \vdash_\ell t @ \tau : A @ \tau} \quad \frac{\Theta \vdash \tau : \text{time} \quad \Theta \mid \Gamma; \Delta_1 \vdash_\ell t_1 : A @ \tau \quad \Theta \mid \Gamma; \Delta_2, a :_\tau A \vdash_\ell t_2 : B}{\Theta \mid \Gamma; \Delta_1, \Delta_2 \vdash_\ell \text{let } a @ \tau = t_1 \text{ in } t_2 : B} \text{ (@-E)} \\
\\
\text{(G-E)} \frac{\Theta \mid \Gamma \vdash_c e : \mathbb{G} A}{\Theta \mid \Gamma; \cdot \vdash_\ell \text{runG } e : A} \quad \text{(F-I)} \frac{\Theta \mid \Gamma \vdash_c e : X}{\Theta \mid \Gamma; \cdot \vdash_\ell \text{F } e : \text{F } X} \quad \frac{\Theta \mid \Gamma; \Delta_1 \vdash_\ell t_1 : \text{F } X \quad \Theta \mid \Gamma, x : X; \Delta_2 \vdash_\ell t_2 : B}{\Theta \mid \Gamma; \Delta_1, \Delta_2 \vdash_\ell \text{let F } x = t_1 \text{ in } t_2 : B} \text{ (F-E)} \\
\\
\text{(\forall-I)} \frac{\Theta, i : \sigma \mid \Gamma; \Delta \vdash_\ell t : A}{\Theta \mid \Gamma; \Delta \vdash_\ell \Lambda i : \sigma. t : \forall i : \sigma. A} \quad \frac{\Theta \vdash s : \sigma \quad \Theta \mid \Gamma; \Delta \vdash_\ell t : \forall i : \sigma. A}{\Theta \mid \Gamma; \Delta \vdash_\ell t_s : \{s/i\}A} \text{ (\forall-I)} \\
\\
\text{(\exists-I)} \frac{\Theta \vdash s : \sigma \quad \Theta \mid \Gamma; \Delta \vdash_\ell t : \{s/i\}A}{\Theta \mid \Gamma; \Delta \vdash_\ell \{s, t\} : \exists i : \sigma. A} \quad \frac{\Theta \mid \Gamma; \Delta_1 \vdash_\ell t_1 : \exists i : \sigma. A \quad \Theta, s : \sigma \mid \Gamma; \Delta_2, a : \{s/i\}A \vdash_\ell t_2 : B}{\Theta \mid \Gamma; \Delta_1, \Delta_2 \vdash_\ell \text{let } \{s, a\} = t_1 \text{ in } t_2 : B} \text{ (\exists-E)} \\
\\
\frac{\Theta \mid \Gamma; \Delta_1 \vdash_\ell t_1 : \diamond A \quad \Theta \mid \Gamma; \Delta_2 \vdash_\ell t_2 : \diamond B \quad \Theta \mid \Gamma; a : A, t_2 : \diamond B \vdash_\ell t'_1 : \diamond C \quad \Theta \mid \Gamma; t_1 : \diamond A, b : B \vdash_\ell t'_2 : \diamond C}{\Theta \mid \Gamma; \Delta_1, \Delta_2 \vdash_\ell \text{select } (t_1, t_2) \text{ as } [a \mapsto t'_1] \parallel [b \mapsto t'_2] : \diamond C} \text{ (SELECT)} \\
\\
\frac{\Theta \vdash \tau : \text{time} \quad \Delta' = \Delta \downarrow^\tau \quad \Theta \mid \Gamma; \Delta' \vdash_\ell t : A}{\Theta \mid \Gamma; \Delta \vdash_\ell t :_\tau A} \text{ (DELAY)} \\
\\
\text{(I}_\tau\text{-E)} \frac{\Theta \vdash \tau : \text{time} \quad \Theta \mid \Gamma; \Delta_1 \vdash_\ell t_1 :_\tau \mathbb{I} \quad \Theta \mid \Gamma; \Delta_2 \vdash_\ell t_2 : B}{\Theta \mid \Gamma; \Delta_1, \Delta_2 \vdash_\ell \text{let } \langle \rangle_\tau = t_1 \text{ in } t_2 : B} \quad \frac{\Theta \vdash \tau : \text{time} \quad \Theta \mid \Gamma; \Delta_1 \vdash_\ell t_1 :_\tau A @ B \quad \Theta \mid \Gamma; \Delta_2, a :_\tau A, b :_\tau B \vdash_\ell t_2 : C}{\Theta \mid \Gamma; \Delta_1, \Delta_2 \vdash_\ell \text{let } (a, b)_\tau = t_1 \text{ in } t_2 : B} \text{ (}\otimes_\tau\text{-E)}
\end{array}$$

## 2 Syntactic Substitution

Given the number of contexts and judgments we have, substitution is quite an intricate issue. The most interesting case is substitution for indices, as they may appear in terms, types and even the meta-judgment itself. The substitution of Cartesian terms into Cartesian and linear terms, and linear substitution into linear terms is the usual notion of mutually recursive substitution that we get with Benton–Wadler adjoint logic.

### 2.1 Index substitution

#### 2.1.1 Weakening

First, we introduce the syntactic weakening relation between two contexts – while it is a special case of a substitution (renaming, or substituting variables for variables), we need the weakening lemma in order to prove the syntactic and semantic substitution lemma.

**Definition 2.1** (Index context membership). We define the index context membership relation  $s : \sigma \in \Theta$  with the following rules and axioms:

$$\frac{}{s : \sigma \in \Theta, s : \sigma} \qquad \frac{s : \sigma \in \Theta \quad s \neq s'}{s : \sigma \in \Theta, s' : \sigma'}$$

**Definition 2.2** (Subcontext relation). We define the subcontext relation  $\Theta' \supseteq \Theta$  with the following rules and axioms:

$$\frac{}{\cdot \supseteq \cdot} \qquad \frac{\Theta' \supseteq \Theta \quad i \notin \text{dom}(\Theta')}{\Theta', i : \sigma \supseteq \Theta} \qquad \frac{\Theta' \supseteq \Theta \quad i \notin \text{dom}(\Theta')}{\Theta', i : \sigma \supseteq \Theta, i : \sigma}$$

**Lemma 2.3** (Weakening of index membership).

$$\frac{s : \sigma \in \Theta \quad \Theta' \supseteq \Theta}{s : \sigma \in \Theta'}$$

*Proof.* We proceed by induction on the context membership  $s : \sigma \in \Theta$ .

- $s : \sigma \in \Theta'', s : \sigma$ :  
By assumption,  $\Theta' \supseteq \Theta'', s : \sigma$ . There are two rules for the subcontext relation that can have this conclusion:
  - $\hat{\Theta}, s : \sigma \supseteq \Theta'', s : \sigma$ : by the membership axiom, we have that  $s : \sigma \in \hat{\Theta}, s : \sigma$ , and since  $\hat{\Theta}, s : \sigma = \Theta'$ , we get the required conclusion  $s : \sigma \in \Theta'$ .
  - $\hat{\Theta}, s' : \sigma' \supseteq \Theta'', s : \sigma$ : using the hypothesis  $\hat{\Theta} \supseteq \Theta'', s : \sigma$  and the fact that  $s : \sigma \in \Theta'', s : \sigma$ , the IH gives us  $s : \sigma \in \hat{\Theta}$ . Extending this with an extra variable  $s' : \sigma'$  gives  $s : \sigma \in \hat{\Theta}, s' : \sigma' = \Theta'$ , as required.
- $s : \sigma \in \Theta'', s' : \sigma'$ :  
By assumption,  $\Theta' \supseteq \Theta'', s' : \sigma'$  and  $s : \sigma \in \Theta''$ . There are two rules for the subcontext relation that can have this conclusion:
  - $\hat{\Theta}, s' : \sigma' \supseteq \Theta'', s' : \sigma'$ : the hypotheses  $\hat{\Theta} \supseteq \Theta''$  and  $s : \sigma \in \Theta''$  give us  $s : \sigma \in \hat{\Theta}$  by induction, and extending the context results in  $s : \sigma \in \hat{\Theta}, s' : \sigma' = \Theta'$ , as require.

- $\hat{\Theta}, \hat{s}: \hat{\sigma} \supseteq \Theta'', s': \sigma'$ : the hypotheses  $\hat{\Theta} \supseteq \Theta'', s': \sigma'$  and  $s: \sigma \in \Theta'', s': \sigma'$  give us  $s: \sigma \in \hat{\Theta}$  by induction, and extending the context results in  $s: \sigma \in \hat{\Theta}, s': \sigma' = \Theta'$ , as required.

□

**Lemma 2.4** (Weakening of sort judgements).

$$\frac{\Theta' \supseteq \Theta \quad \Theta \vdash_s s : \sigma}{\Theta' \vdash_s s : \sigma}$$

*Proof.* We perform induction on the derivation of  $\Theta \vdash_s s : \sigma$ .

- $\Theta \vdash_s \tau : \text{time}$  and  $\Theta \vdash_s \iota : \text{id}$ :  
In the base cases,  $\tau$  and  $\iota$  are natural numbers which do not depend on the context – thus  $\Theta$  can be freely weakened.
- $\Theta \vdash_s s : \sigma$ :  
From the hypothesis we know that  $s : \sigma \in \Theta$ . By the previous lemma, this means that  $s : \sigma \in \Theta'$ , which gives us the conclusion that  $\Theta' \vdash_s s : \sigma$ .

□

**Lemma 2.5** (Weakening of Cartesian type judgements).

$$\frac{\Theta' \supseteq \Theta \quad \Theta \vdash_c X \text{ type}}{\Theta' \vdash_c X \text{ type}}$$

*Proof.* We perform induction on the derivation of  $\Theta \vdash_c X \text{ type}$ .

- $\Theta \vdash_c 1 \text{ type}$ :  
1 is a closed type and does not depend on the index context, which can be freely weakened.
- $\Theta \vdash_c X \rightarrow Y \text{ type}$ :  
From the hypotheses and the IH, we deduce that  $\Theta' \vdash_c X \text{ type}$  and  $\Theta' \vdash_c Y \text{ type}$ . Applying the well-formedness rule for functions, we conclude that  $\Theta' \vdash_c X \rightarrow Y \text{ type}$ .
- $\Theta \vdash_c G A \text{ type}$ :  
From the hypothesis and mutual IH, we deduce that  $\Theta' \vdash_\ell A \text{ type}$ . Applying the well-formedness rule for  $G$ , we conclude that  $\Theta' \vdash_c G A \text{ type}$ .

□

**Lemma 2.6** (Weakening of linear type judgements).

$$\frac{\Theta' \supseteq \Theta \quad \Theta \vdash_\ell A \text{ type}}{\Theta' \vdash_\ell A \text{ type}}$$

*Proof.* We perform induction on the derivation of  $\Theta \vdash_\ell A \text{ type}$ .

- $\Theta \vdash_\ell \langle \rangle \text{ type}$ :  
 $\langle \rangle$  is a closed type and does not depend on the index context, which can be freely weakened.

- $\Theta \vdash_\ell A \multimap B$  type:  
From the hypotheses and the IH, we deduce that  $\Theta' \vdash_\ell A$  type and  $\Theta' \vdash_\ell B$  type. Applying the type formation rule for linear functions, we can conclude that  $\Theta' \vdash_\ell A \multimap B$  type.
- $\Theta \vdash_\ell \Diamond A$  type:  
From the hypothesis and the IH, we deduce that  $\Theta' \vdash_c A$  type. Applying the type formation rule for events, we conclude that  $\Theta' \vdash_\ell \Diamond A$  type.
- $\Theta \vdash_\ell A @ \tau$  type:  
From the hypothesis, the IH and the previous lemma, we deduce that  $\Theta' \vdash_c A$  type and  $\Theta' \vdash_s \tau : \text{time}$ . Applying the type formation rule for delayed types, we conclude that  $\Theta' \vdash_\ell A @ \tau$  type.
- $\Theta \vdash_\ell F X$  type:  
From the hypothesis and mutual IH, we deduce that  $\Theta' \vdash_c X$  type. Applying the type formation rule for  $F$ , we conclude that  $\Theta' \vdash_\ell F X$  type.
- $\Theta \vdash_\ell \forall s : \sigma. A$  type:  
The hypothesis of the judgment is  $\Theta, s : \sigma \vdash_\ell A$  type. In order to apply the induction hypothesis, we need to extend the subcontext assumption  $\Theta' \supseteq \Theta$  to  $\Theta', s : \sigma \supseteq \Theta, s : \sigma$ . Applying the IH gives  $\Theta', s : \sigma \vdash_\ell A$  type, and from the type formation rule for index quantification we conclude that  $\Theta \vdash_\ell \forall s : \sigma. A$  type.
- $\Theta \vdash_\ell \exists s : \sigma. A$  type:  
The hypothesis of the judgment is  $\Theta, s : \sigma \vdash_\ell A$  type. In order to apply the induction hypothesis, we need to extend the subcontext assumption  $\Theta' \supseteq \Theta$  to  $\Theta', s : \sigma \supseteq \Theta, s : \sigma$ . Applying the IH gives  $\Theta', s : \sigma \vdash_\ell A$  type, and from the type formation rule for index quantification we conclude that  $\Theta \vdash_\ell \exists s : \sigma. A$  type.
- $\Theta \vdash_\ell \text{Widget}^l$  type:  
The hypothesis is  $\Theta \vdash_s \iota : \text{id}$ . By the previous lemma and the assumption  $\Theta' \supseteq \Theta$ , as well as the type formation rule for widgets, we conclude that  $\Theta' \vdash_\ell \text{Widget}^l$  type.
- $\Theta \vdash_\ell \text{Prefix}^l(\tau)$  type:  
The hypotheses are  $\Theta \vdash_s \tau : \text{time}$  and  $\Theta \vdash_s \iota : \text{id}$ . By the previous lemma and the assumption  $\Theta' \supseteq \Theta$ , as well as the type formation rule for widgets, we conclude that  $\Theta' \vdash_\ell \text{Prefix}^l(\tau)$  type.

□

**Lemma 2.7** (Weakening of Cartesian terms).

$$\frac{\Theta' \supseteq \Theta \quad \Theta \mid \Gamma \vdash_c e : X}{\Theta' \mid \Gamma \vdash_c e : X}$$

*Proof.* Since the grammar of Cartesian terms does not involve changing the index context, all the cases are straightforward recursive applications of the IH (mutual IH, in the case of  $G t$ ) to the subterms. □

**Lemma 2.8** (Weakening of linear terms).

$$\frac{\Theta' \supseteq \Theta \quad \Theta \mid \Gamma; \Delta \vdash_\ell t :_\tau A}{\Theta' \mid \Gamma; \Delta \vdash_\ell t :_\tau A}$$

*Proof.* We perform induction on the derivation of  $\Theta \mid \Gamma; \Delta \vdash_\ell t :_\tau A$ . Most of the cases are applications of the IH to the subterms followed by the application of the typing rule. Below are the cases that involve the index context:

- $\Theta \mid \Gamma; \Delta \vdash_\ell t @ \tau : A @ \tau$ :  
From the two hypotheses, the IH, and Lemma 2.4, we deduce that  $\Theta' \vdash_s \tau : \text{time}$  and  $\Theta' \mid \Gamma; \Delta \vdash_\ell t :_\tau A$ . Applying the typing rule gives us  $\Theta' \mid \Gamma; \Delta \vdash_\ell t @ \tau : A @ \tau$ , as required.
- $\Theta \mid \Gamma; \Delta \vdash_\ell \text{let } \tau @ t_1 = x \text{ in } t_2 : B$ :  
From the two hypotheses, the IH, and Lemma 2.4, we deduce that  $\Theta' \vdash_s \tau : \text{time}$ ,  $\Theta' \mid \Gamma; \Delta_1 \vdash_\ell t_1 : A @ \tau$  and  $\Theta' \mid \Gamma; \Delta_2, x :_\tau A \vdash_\ell t_2 : B$ . Applying the typing rule gives us  $\Theta' \mid \Gamma; \Delta \vdash_\ell \text{let } \tau @ t_1 = x \text{ in } t_2 : B$ , as required.
- $\Theta \mid \Gamma; \Delta \vdash_\ell \Lambda s : \sigma. t : \forall s : \sigma. A$ :  
The hypothesis of the rule is  $\Theta, s : \sigma \mid \Gamma; \Delta \vdash_\ell t : A$ . By applying the congruence rule to  $\Theta' \supseteq \Theta$  to get  $\Theta', s : \sigma \supseteq \Theta, s : \sigma$ , we get  $\Theta', s : \sigma \mid \Gamma; \Delta \vdash_\ell t : A$  by induction. The typing rule then gives us  $\Theta' \mid \Gamma; \Delta \vdash_\ell \Lambda s : \sigma. t : \forall s : \sigma. A$ , as required.
- $\Theta \mid \Gamma; \Delta \vdash_\ell t_s : \{s/i\}A$ :  
From the two hypotheses, the IH, and Lemma 2.4, we deduce that  $\Theta' \vdash_s \tau : \text{time}$  and  $\Theta' \mid \Gamma; \Delta \vdash_\ell t : \forall i : \sigma. A$ . Applying the typing rule gives  $\Theta' \mid \Gamma; \Delta \vdash_\ell t_s : \{s/i\}A$ .
- $\Theta \mid \Gamma; \Delta \vdash_\ell \{s, t\} : \exists i : \sigma. A$ :  
From the two hypotheses, the IH, and Lemma 2.4, we deduce that  $\Theta' \vdash_s \tau : \text{time}$  and  $\Theta' \mid \Gamma; \Delta \vdash_\ell t : \{s/i\}A$ . Applying the typing rule gives  $\Theta' \mid \Gamma; \Delta \vdash_\ell \{s, t\} : \exists i : \sigma. A$ .
- $\Theta \mid \Gamma; \Delta_1, \Delta_2 \vdash_\ell \text{let } \{s, a\} = t_1 \text{ in } t_2 : B$ :  
Applying the IH to the first hypothesis gives  $\Theta' \mid \Gamma; \Delta_1 \vdash_\ell t_1 : \exists i : \sigma. A$ . To apply the IH to the second hypothesis, we need to extend the subcontext relation assumption to get  $\Theta', s : \sigma \supseteq \Theta, s : \sigma$  – induction then gives  $\Theta', s : \sigma \mid \Gamma; \Delta_2, x : a\{s/i\}A \vdash_\ell t_2 : B$ . Applying the typing rule results in  $\Theta' \mid \Gamma; \Delta_1, \Delta_2 \vdash_\ell \text{let } \{s, a\} = t_1 \text{ in } t_2 : B$ , as required.

□

### 2.1.2 Simultaneous index substitution

**Definition 2.9** (Index Substitutions). We define a simultaneous index substitution as:

$$\zeta ::= \diamond \mid \zeta, i \mapsto s$$

where  $i$  is an index variable and  $s$  is an index. The domain of a substitution  $\zeta$ ,  $\text{dom}(\zeta)$ , is define by induction:

$$\begin{aligned} \text{dom}(\diamond) &\triangleq \emptyset \\ \text{dom}(\zeta, x \mapsto t) &\triangleq \text{dom}(\zeta) \cup \{x\} \end{aligned}$$

The set of free-variables of a substitution  $\zeta$ ,  $\text{fv}(\zeta)$ , is define as:

$$\text{fv}(\diamond) \triangleq \emptyset$$



$$\text{fv}(\zeta, i \mapsto s) \triangleq \text{fv}(\zeta) \cup \text{fv}(s)$$

where we assume the usual definition of free variables in a term. We will use the shorthand:

$$\zeta \# i \triangleq i \notin (\text{dom}(\zeta) \cup \text{fv}(\zeta))$$

Finally, we will write  $\{s/i\}$  for the single substitution  $(i \mapsto s)$ .

**Definition 2.10** (Composition of Substitutions). Given two index substitution  $\zeta_1, \zeta_2$ , s.t.

$$(\forall (i \in \text{dom}(\zeta_1)). \zeta_2 \# i) \wedge (\forall (i \in \text{dom}(\zeta_2)). \zeta_1 \# i)$$

we define the composition of them, written just as  $\zeta_1, \zeta_2$ , as:

$$\begin{aligned} \zeta_1, \diamond &\triangleq \zeta_1 \\ \zeta_1, (\zeta_2', i \mapsto s) &\triangleq (\zeta_1, \zeta_2'), i \mapsto s \end{aligned}$$

**Definition 2.11** (Well-typed index substitution). We define a well-typed index substitution, written  $\Theta' \vdash_s \zeta \triangleright \Theta$  by the following rules:

$$\frac{}{\Theta' \vdash_s \diamond \triangleright \cdot} \qquad \frac{\Theta' \vdash_s \zeta \triangleright \Theta \quad i \notin \text{dom}(\Theta) \quad \Theta' \vdash_s s : \sigma}{\Theta' \vdash_s (\zeta, i \mapsto s) \triangleright (\Theta, i : \sigma)}$$

### 2.1.3 Index substitution into indices

**Definition 2.12** (Index substitution into indices). We define the application of a simultaneous index substitution into indices. Assuming a substitution  $\zeta$ , we proceed by induction over indices:

$$\begin{aligned} \zeta(\tau) &\triangleq \tau & \tau \in \text{Time} \\ \zeta(\iota) &\triangleq \iota & \iota \in \text{Id} \\ \diamond(i) &\triangleq i \\ (\zeta, i \mapsto s)(i) &\triangleq s \\ (\zeta, i \mapsto s)(j) &\triangleq \zeta(s) & j \neq i \end{aligned}$$

**Lemma 2.13** (Weakening of an index substitution).

$$\frac{\Theta' \vdash_s \zeta \triangleright \Theta \quad \hat{\Theta} \supseteq \Theta'}{\hat{\Theta} \vdash_s \zeta \triangleright \Theta}$$

*Proof.* We perform induction on  $\Theta' \vdash_s \zeta \triangleright \Theta$ .

- $\Theta' \vdash_s \diamond \triangleright \cdot$ :  
The conclusion  $\hat{\Theta} \vdash_s \diamond \triangleright \cdot$  follows directly from the empty substitution axiom.
- $\Theta' \vdash_s \zeta, i \mapsto s \triangleright \Theta, i : \sigma$ :  
By assumption we have  $\Theta' \vdash_s \zeta \triangleright \Theta$  and  $\Theta' \vdash_s s : \sigma$ . By the IH we have  $\hat{\Theta} \vdash_s \zeta \triangleright \Theta$  and by Lemma 2.4  $\hat{\Theta} \vdash_s s : \sigma$ . Applying the substitution rule we get  $\hat{\Theta} \vdash_s \zeta, i \mapsto s \triangleright \Theta, i : \sigma$ , as required.

□

**Lemma 2.14** (Index substitution extension). If  $\Theta' \vdash_s \zeta \triangleright \Theta$  and  $i \notin \text{dom}(\Theta) \cup \text{dom}(\Theta')$  then  $(\Theta', i : \sigma) \vdash_s (\zeta, i \mapsto i) \triangleright (\Theta, i : \sigma)$

*Proof.* By the previous lemma and the axiom  $\Theta', i : \sigma \supseteq \Theta'$ , we have that  $\Theta', i : \sigma \vdash_s \zeta \triangleright \Theta$ . We can extend it with the mapping  $i \mapsto i$  to get  $(\Theta', i : \sigma) \vdash_s (\zeta, i \mapsto i) \triangleright (\Theta, i : \sigma)$ , as required. □

**Lemma 2.15** (Preservation of index judgement under index substitution).

$$\frac{\Theta' \vdash_s \zeta \triangleright \Theta \quad \Theta \vdash_s s : \sigma}{\Theta' \vdash_s \zeta(s) : \sigma}$$

*Proof.* We proceed by induction over  $\zeta$ :

- $(\diamond)$ :  
Since  $\Theta = \cdot$  and we assume  $\Theta \vdash_s s : \sigma$ , we know  $s$  must be either  $\tau$  s.t.  $\tau \in \mathbb{N}_\top$  or  $\iota$  s.t.  $\iota \in \mathbb{N}$ . In either case, can type  $s$  in any context, and hence the conclusion follows.
- $(\Theta' \vdash_s \zeta, i \mapsto s' \triangleright \Theta, i : \sigma)$ :  
We proceed by cases on  $\Theta \vdash_s s : \sigma$ 
  - $(\Theta, i : \sigma \vdash_s \tau : \text{time})$ :  
By definition of index judgments, we know that  $\tau \in \mathbb{N}_\top$  and definition of index substitution we know that  $(\zeta, x \mapsto s')(\tau) = \tau$ . Since  $\tau : \text{time}$  is well-formed in any index context we can conclude  $\Theta' \vdash_s (\zeta, i \mapsto s')(\tau) : \text{time}$  as wanted.
  - $(\Theta, i : \sigma \vdash_s \iota : \text{id})$ :  
By definition of index judgments, we know that  $i \in \mathbb{N}$  and definition of index substitution we know that  $(\zeta, i \mapsto s')(i) = i$ . Since  $i : \text{id}$  is well-formed in any index context we can conclude  $\Theta' \vdash_s (\zeta, i \mapsto s')(i) : \text{id}$  as wanted.
  - $(\Theta, i : \sigma' \vdash_s s : \sigma)$ :  
We have two cases depending on whether  $i = s$ . If  $i = s$ , then we know that  $\sigma' = \sigma$  and by assumption of a well-typed index substitution that  $\Theta' \vdash_s i : \sigma'$  which is precisely the conclusion we want. If  $i \neq s$ , then  $(\zeta, x \mapsto s')(s) = \zeta(s)$  and the conclusion follows by application of the inductive hypothesis.

□

#### 2.1.4 Index substitution into types

**Definition 2.16** (Index substitution into Cartesian and linear types). We define capture-avoiding index substitution into types. Assuming a substitution  $\zeta$ , we proceed by mutual induction on Cartesian and linear types:

$$\begin{aligned} \zeta(1) &\triangleq 1 \\ \zeta(X \rightarrow Y) &\triangleq \zeta(X) \rightarrow \zeta(Y) \\ \zeta(\mathsf{G} A) &\triangleq \mathsf{G} (\zeta(A)) \end{aligned}$$

$$\begin{aligned}
\zeta(\langle \rangle) &\triangleq \langle \rangle \\
\zeta(A \otimes B) &\triangleq \zeta(A) \otimes \zeta(B) \\
\zeta(A \multimap B) &\triangleq \zeta(A) \multimap \zeta(B) \\
\zeta(A @ s) &\triangleq \zeta(A) @ \zeta(s) \\
\zeta(\Diamond A) &\triangleq \Diamond(\zeta(A)) \\
\zeta(F X) &\triangleq F \zeta(X) \\
\zeta(\forall i: \sigma. A) &\triangleq \forall i: \sigma. \zeta(A) & \zeta \# i \\
\zeta(\exists i: \sigma. A) &\triangleq \exists i: \sigma. \zeta(A) & \zeta \# i \\
\zeta(\text{Widget}^\iota) &\triangleq \text{Widget}^{\zeta(\iota)} \\
\zeta(\text{Prefix}^\iota(\tau)) &\triangleq \text{Prefix}^{\zeta(\iota)}(\zeta(\tau))
\end{aligned}$$

**Lemma 2.17** (Identity substitution preserves type). For any type  $X$  and any index variable  $i$ ,  $X = (i \mapsto i)(X)$ .

*Proof.* The proof follows by a simple induction over the definition of types and the fact that we only consider types up to  $\alpha$ -equivalence and hence can always assume  $i$  fresh.  $\square$

**Lemma 2.18** (Preservation of type wellformedness judgment under index substitution).

$$\frac{\Theta' \vdash_s \zeta \triangleright \Theta \quad \Theta \vdash_c X \text{ type}}{\Theta' \vdash_c \zeta(X) \text{ type}} \qquad \frac{\Theta' \vdash_s \zeta \triangleright \Theta \quad \Theta \vdash_\ell A \text{ type}}{\Theta' \vdash_\ell \zeta(A) \text{ type}}$$

*Proof.* We proceed by induction over the derivation of  $X$  or  $A$  being well-formed over  $\Theta$ :

- $(\Theta \vdash_c 1 \text{ type})$ :  
Since for any substitution  $\zeta(1) = 1$  and for  $1$  is well-formed for any index context, the conclusion is immediate.
- $(\Theta \vdash_c X \rightarrow Y \text{ type})$ :  
By the definition of well-formed types, we know  $\Theta \vdash_c X \text{ type}$  and  $\Theta \vdash_c Y \text{ type}$ . By application of our inductive hypothesis we know that  $\Theta' \vdash_c \zeta(X) \text{ type}$  and  $\Theta' \vdash_c \zeta(Y) \text{ type}$ . By definition of substitution application, we know that  $\zeta(X \rightarrow Y) = \zeta(X) \rightarrow \zeta(Y)$ . We can now apply the rule for well-formed arrow types to conclude  $\Theta' \vdash_c \zeta(X \rightarrow Y) \text{ type}$  as wanted.
- $(\Theta \vdash_c G A \text{ type})$ :  
By the definition of well-formed types, we know that  $\Theta \vdash_\ell A \text{ type}$ . By application of our inductive hypothesis we know that  $\Theta' \vdash_\ell \zeta(A) \text{ type}$ . By definition of substitution application, know that  $\zeta(G A) = G \zeta(A)$ . We can now apply the rule for well-formed  $G$  types to conclude  $\Theta' \vdash_c \zeta(G A) \text{ type}$  as wanted.
- $(\Theta \vdash_\ell I \text{ type})$ :  
Since for any substitution  $\zeta(I) = I$  and for  $I$  is well-formed for any index context, the conclusion is immediate.
- $(\Theta \vdash_\ell A \multimap B \text{ type})$ :  
By the definition of well-formed types, we know  $\Theta \vdash_\ell X \text{ type}$  and  $\Theta \vdash_\ell Y \text{ type}$ . By application

of our inductive hypothesis we know that  $\Theta' \vdash_\ell \zeta(A)$  type and  $\Theta' \vdash_\ell \zeta(B)$  type. By definition of substitution application, we know that  $\zeta(A \multimap B) = \zeta(A) \multimap \zeta(B)$ . We can now apply the rule for well-formed linear function types to conclude  $\Theta' \vdash_\ell \zeta(A \multimap B)$  type as wanted.

- ( $\Theta \vdash_\ell A \otimes B$  type):

By the definition of well-formed types, we know  $\Theta \vdash_\ell X$  type and  $\Theta \vdash_\ell Y$  type. By application of our inductive hypothesis we know that  $\Theta' \vdash_\ell \zeta(A)$  type and  $\Theta' \vdash_\ell \zeta(B)$  type. By definition of substitution application, we know that  $\zeta(A \otimes B) = \zeta(A) \otimes \zeta(B)$ . We can now apply the rule for well-formed tensor product types to conclude  $\Theta' \vdash_\ell \zeta(A \otimes B)$  type as wanted.

- ( $\Theta \vdash_\ell F X$  type):

By the definition of well-formed types, we know that  $\Theta \vdash_c X$  type. By application of our inductive hypothesis we know that  $\Theta' \vdash_c \zeta(X)$  type. By definition of substitution application, we know that  $\zeta(F X) = F \zeta(X)$ . We can now apply the rule for well-formed  $G$  types to conclude  $\Theta' \vdash_\ell \zeta(F X)$  type as wanted.

- ( $\Theta \vdash_\ell A @ \tau$  type):

By the definition of well-formed types, we know that  $\Theta \vdash_s \tau : \text{time}$  and  $\Theta \vdash_\ell A$  type. By application of our induction hypothesis, we know that  $\Theta' \vdash_\ell \zeta(A)$  type and by Lemma 2.15 we now  $\Theta' \vdash_s \zeta(\tau) : \text{time}$ . By definition  $\zeta(A @ \tau) = \zeta(A) @ \zeta(\tau)$ . Combining the above we can now conclude  $\Theta' \vdash_\ell \zeta(A @ \tau)$  type as wanted.

- ( $\Theta \vdash_\ell \forall i : \sigma. A$  type):

By definition of well-formed types we know that  $\Theta, i : \sigma \vdash_\ell A$  type. By Lemma 2.14 we can form  $(\Theta', i : \sigma) \vdash_s (\zeta, i \mapsto i) \triangleright (\Theta, i : \sigma)$  where we use the fact that we only consider types up to  $\alpha$ -equivalence of indices to ensure  $i \notin \text{dom}(\Theta')$ . We can apply our induction hypothesis with  $\zeta, i \mapsto i$  to conclude that  $\Theta', i : \sigma \vdash_\ell (\zeta, i \mapsto i)(A)$  type and hence  $\Theta' \vdash_\ell \forall s : \sigma. (\zeta, i \mapsto i)(A)$  type. By Lemma 2.17 we know that  $(\zeta, i \mapsto i)(A) = \zeta(A)$ . Combining the above we can now conclude  $\Theta' \vdash_\ell \zeta(\forall i : \sigma. A)$  type as wanted.

- ( $\Theta \vdash_\ell \exists i : \sigma. A$  type):

This case follows by the same reasoning as the above case.

- ( $\Theta \vdash_\ell \text{Widget}^\iota$  type):

By the definition of well-formed types, we know that  $\Theta \vdash_s \iota : \text{id}$ . By application of Lemma 2.15 we get that  $\Theta' \vdash_s \zeta(\iota) : \text{id}$  and then  $\Theta' \vdash_\ell \text{Widget}^{\zeta(\iota)}$  type. Since  $\zeta(\text{Widget}^\iota) = \text{Widget}^{\zeta(\iota)}$  we are done.

- ( $\Theta \vdash_\ell \text{Prefix}^\iota(\tau)$  type):

By the definition of well-formed types, we know that  $\Theta \vdash_s \tau : \text{time}$  and  $\Theta \vdash_s \iota : \text{id}$ . By application of Lemma 2.15 we get that  $\Theta' \vdash_s \zeta(\tau) : \text{time}$  and  $\Theta' \vdash_s \zeta(\iota) : \text{id}$  and then  $\Theta \vdash_\ell \text{Prefix}^{\zeta(\iota)}(\zeta(\tau))$  type. Since  $\zeta(\text{Prefix}^\iota(\tau)) = \text{Prefix}^{\zeta(\iota)}(\zeta(\tau))$  we are done.

□

### 2.1.5 Index substitution into terms

**Definition 2.19** (Index substitution into Cartesian and linear terms). We define simultaneous index substitution into Cartesian and linear terms. For conciseness, we will not distinguish between

Cartesian and linear terms in the case for variable, lambda abstraction and lambda application.

$$\begin{aligned}
\zeta(x) &\triangleq x \\
\zeta(\lambda x. e) &\triangleq \lambda x. \zeta(e) \\
\zeta(e_1 e_2) &\triangleq \zeta(e_1) \zeta(e_2) \\
\zeta(\bullet) &\triangleq \bullet \\
\zeta(\mathbf{G} t) &\triangleq \mathbf{G} \zeta(t) \\
\\ 
\zeta(a) &\triangleq a \\
\zeta(\lambda a. t) &\triangleq \lambda a. \zeta(t) \\
\zeta(t_1 t_2) &\triangleq \zeta(t_1) \zeta(t_2) \\
\zeta(\langle \rangle) &\triangleq \langle \rangle \\
\zeta(\text{let } \langle \rangle = t_1 \text{ in } t_2) &\triangleq \text{let } \langle \rangle = \zeta(t_1) \text{ in } \zeta(t_2) \\
\zeta((t_1, t_2)) &\triangleq (\zeta(t_1), \zeta(t_2)) \\
\zeta(\text{let } (a, b) = t_1 \text{ in } t_2) &\triangleq \text{let } (a, b) = \zeta(t_1) \text{ in } \zeta(t_2) \\
\zeta(\text{evt } t) &\triangleq \text{evt } \zeta(t) \\
\zeta(\text{let evt } a = t_1 \text{ in } t_2) &\triangleq \text{let evt } a = \zeta(t_1) \text{ in } \zeta(t_2) \\
\zeta(t @ \tau) &\triangleq \zeta(t) @ \zeta(i) \\
\zeta(\text{let } x @ \tau = t_1 \text{ in } t_2) &\triangleq \text{let } x @ \tau = \zeta(t_1) \text{ in } \zeta(t_2) & \zeta \# \tau \\
\zeta(\text{runG } e) &\triangleq \text{runG } (\zeta(e)) \\
\zeta(\mathbf{F} e) &\triangleq \mathbf{F} (\zeta(e)) \\
\zeta(\text{let } \mathbf{F} x = t_1 \text{ in } t_2) &\triangleq \text{let } \mathbf{F} x = \zeta(t_1) \text{ in } \zeta(t_2) \\
\zeta(\Lambda i : \sigma. t) &\triangleq \Lambda i : \sigma. \zeta(t) & \zeta \# i \\
\zeta(t_s) &\triangleq \zeta(t)_{\zeta(s)} \\
\zeta(\{i, t\}) &\triangleq \{i, \zeta(t)\} & \zeta \# i \\
\zeta(\text{let } \{s, a\} = t_1 \text{ in } t_2) &\triangleq \text{let } \{s, a\} = \zeta(t_1) \text{ in } \zeta(t_2) & \zeta \# s \\
\zeta(\text{select } (t_1, t_2) \text{ as } [a \mapsto t'_1] \parallel [b \mapsto t'_2]) &\triangleq \text{select } (\zeta(t_1), \zeta(t_2)) \text{ as } [a \mapsto \zeta(t'_1)] \parallel [b \mapsto \zeta(t'_2)] \\
\zeta(\text{let } \langle \rangle_\tau = t_1 \text{ in } t_2) &\triangleq \text{let } \langle \rangle_\tau = \zeta(t_1) \text{ in } \zeta(t_2) \\
\zeta(\text{let } (a, b)_\tau = t_1 \text{ in } t_2) &\triangleq \text{let } (a, b)_\tau = \zeta(t_1) \text{ in } \zeta(t_2)
\end{aligned}$$

**Definition 2.20** (Index substitution on contexts). We define the application of a substitution on contexts as:

$$\begin{aligned}
\zeta(\cdot) &\triangleq \cdot \\
\zeta(\Gamma, x : X) &\triangleq \zeta(\Gamma), x : \zeta(X) \\
\zeta(\Delta, a :_\tau A) &\triangleq \zeta(\Delta), a :_\tau \zeta(A)
\end{aligned}$$

**Lemma 2.21** (Identity substitution preserves terms). For any Cartesian or linear term  $t$  and any index variable  $i$ ,  $t = (i \mapsto i)(t)$ .

*Proof.* The proof follows by a simple induction over the definition of terms and the fact that we only consider terms up to  $\alpha$ -equivalence and hence can always assume  $i$  fresh.  $\square$

**Lemma 2.22** (Preservation of term wellformedness judgment under index substitution).

$$\frac{\Theta' \vdash_s \zeta \triangleright \Theta \quad \Theta \mid \Gamma \vdash_c e : X}{\Theta' \mid \zeta(\Gamma) \vdash_c \zeta(e) : \zeta(X)} \quad \frac{\Theta' \vdash_s \zeta \triangleright \Theta \quad \Theta \mid \Gamma; \Delta \vdash_\ell t :_\tau A}{\Theta' \mid \zeta(\Gamma); \zeta(\Delta) \vdash_\ell \zeta(t) :_\tau \zeta(A)}$$

*Proof.* We prove the statements by mutual induction on the typing derivations. Most cases follows directly by the definition of substitutions and/or application of the inductive hypothesis. We shall only prove the ones that do not. For the substitution into linear judgements, in most cases the judgement will always be “now”, i.e. of the form  $t :_0 A$ , and hence will not be changed by the substitution. In those cases we will not write the subscript.

- $(\Theta \mid \Gamma \vdash_c x : X)$ :

By definition of typing we know  $x : X \in \Gamma$ . By definition of substitution we know

$$\zeta(x) : \zeta(X) \in \zeta(\Gamma)$$

and hence we can conclude

$$\Theta' \mid \zeta(\Gamma) \vdash_c \zeta(x) : \zeta(X)$$

as wanted.

- $(\Theta \mid \Gamma \vdash_c G t : G A)$ :

By definition of typing we know  $\Theta \mid \Gamma; \cdot \vdash_\ell t : A$ . By application of the inductive hypothesis we know

$$\Theta' \mid \zeta(\Gamma); \zeta(\cdot) \vdash_\ell \zeta(t) : \zeta(A)$$

Since  $\zeta(\cdot) = \cdot$ ,  $\zeta(G t) = G(\zeta(t))$  and  $\zeta(G A) = G(\zeta(A))$  we can conclude

$$\Theta' \mid \zeta(\Gamma) \vdash_c \zeta(G t) : \zeta(G A)$$

- $(\Theta \mid \Gamma; a :_\tau A \vdash_\ell a :_\tau A)$ :

By definition we know that  $\zeta(a : A) = \zeta(a) : \zeta(A)$ , and hence we get directly

$$\Theta' \mid \zeta(\Gamma); \zeta(a : A) \vdash_\ell \zeta(a) : \zeta(A)$$

as wanted.

- $(\Theta \mid \Gamma; \Delta \vdash_\ell t @ \tau : A @ \tau)$ :

By typing we know that  $\Theta \vdash_s \tau : \text{time}$  and  $\Theta \mid \Gamma; \Delta \vdash_\ell t :_\tau A$ . By Lemma 2.15 we get  $\Theta' \vdash_s \zeta(\tau) : \text{time}$ , and by application of the induction hypothesis

$$\Theta' \mid \zeta(\Gamma); \zeta(\Delta) \vdash_\ell \zeta(t) :_{\zeta(\tau)} \zeta(A)$$

By typing, and the definition of substitution, we can now conclude

$$\Theta' \mid \zeta(\Gamma); \zeta(\Delta) \vdash_\ell \zeta(t @ \tau) : \zeta(A @ \tau)$$

as wanted.

- $(\Theta \mid \Gamma; \Delta_1, \Delta_2 \vdash_\ell \text{let } a @ \tau = t_1 \text{ in } t_2 : B)$ :  
By typing we know that  $\Theta \vdash_s \tau : \text{time}$ ,

$$\Theta \mid \Gamma; \Delta_1 \vdash_\ell t_1 : A @ \tau$$

and

$$\Theta \mid \Gamma; \Delta_2, a :_\tau A \vdash_\ell t_2 : B$$

By application of Lemma 2.15 and the induction hypothesis, we know  $\Theta' \vdash_s \zeta(\tau) : \text{time}$ ,

$$\Theta' \mid \zeta(\Gamma); \zeta(\Delta_1) \vdash_\ell \zeta(t_1) : \zeta(A @ \tau)$$

and

$$\Theta' \mid \zeta(\Gamma); \zeta(\Delta_2, a :_\tau A) \vdash_\ell \zeta(t_2) : \zeta(B)$$

We note that  $\zeta(A @ \tau) = \zeta(A) @ \zeta(\tau)$  and  $\zeta(\Delta_2, a :_\tau A) = \zeta(\Delta_2), a :_{\zeta(\tau)} \zeta(A)$ . It now follows by typing, and the definition of substitution, that

$$\Theta' \mid \zeta(\Gamma); \zeta(\Delta_1, \Delta_2) \vdash_\ell \zeta(\text{let } a @ \tau = t_1 \text{ in } t_2) : \zeta(B)$$

as wanted.

- $(\Theta \mid \Gamma; \Delta \vdash_\ell \Lambda i : \sigma. t : \forall i : \sigma. A)$ :  
By typing we know  $\Theta, i : \sigma \mid \Gamma; \Delta \vdash_\ell t : A$ . Since we only consider terms up to alpha equivalence, we may consider  $i$  s.t.  $\zeta \# i$ . By Lemma 2.14 we know

$$\Theta', i : \sigma \vdash_s (\zeta, i \mapsto i) \triangleright \Theta, i : \sigma$$

We can now apply the induction hypothesis with Lemma 2.17 and 2.21 to conclude

$$\Theta, i : \sigma \mid \zeta(\Gamma); \zeta(\Delta) \vdash_\ell \zeta(t) : \zeta(A)$$

It now follows by typing and the definition of substitution that

$$\Theta' \mid \zeta(\Gamma); \zeta(\Delta) \vdash_\ell \zeta(\Lambda i : \sigma. t) : \zeta(\forall i : \sigma. A)$$

as wanted.

- $(\Theta \mid \Gamma; \Delta \vdash_\ell t[s] : \{s/i\}A)$ :  
By typing we know that  $\Theta \vdash_s s : \sigma$  and

$$\Theta \mid \Gamma; \Delta \vdash_\ell t : \forall i : \sigma. A$$

By the definition of substitutions, we need  $\zeta \# i$ , but since we only consider terms up to alpha equivalence this is safe to assume. By application of the induction hypothesis and Lemma 2.15 we now know  $\Theta' \vdash_s \zeta(s) : \sigma$  and

$$\Theta' \mid \zeta(\Gamma); \zeta(\Delta) \vdash_\ell \zeta(t) : \zeta(\forall i : \sigma. A)$$

Since  $\zeta \# i$ , we note  $\zeta(\{s/i\}A) = \{\zeta(s)/i\}\zeta(A)$ . Combining the above, we can conclude

$$\Theta \mid \zeta(\Gamma); \zeta(\Delta) \vdash_\ell \zeta(t[s]) : \zeta(\{s/i\}A)$$

as wanted.

- $(\Theta \mid \Gamma; \Delta \vdash_\ell \{s, t\} : \exists i : \sigma. A)$ :  
By typing we know  $\Theta \vdash_s s : \sigma$  and

$$\Theta \mid \Gamma; \Delta \vdash_\ell t : \{s/i\}A$$

By the definition of substitutions, we need  $\zeta \# i$ , but since we only consider terms up to alpha equivalence this is safe to assume. By application of the induction hypothesis and Lemma 2.15 we know  $\Theta' \vdash_s \zeta(s) : \sigma$  and

$$\Theta \mid \zeta(\Gamma); \zeta(\Delta) \vdash_\ell \zeta(t) : \zeta(\{s/i\}A)$$

Since  $\zeta \# i$ , we note  $\zeta(\{s/i\}A) = \{\zeta(s)/i\}\zeta(A)$ . Combining the above, we can now conclude

$$\Theta \mid \zeta(\Gamma); \zeta(\Delta) \vdash_\ell \zeta(\{s, t\}) : \zeta(\exists s' : \sigma. A)$$

as wanted.

- $(\Theta \mid \Gamma; \Delta_1, \Delta_2 \vdash_\ell \text{let } \{s, a\} = t_1 \text{ in } t_2 : B)$ :  
By typing we know

$$\Theta \mid \Gamma; \Delta_1 \vdash_\ell t_1 : \exists i : \sigma. A$$

and

$$\Theta, s : \sigma \mid \Gamma; \Delta_2, a : \{s/i\}A \vdash_\ell t_2 : B$$

By the definition of substitutions, we need  $\zeta \# i$ , but since we only consider terms up to alpha equivalence this is safe to assume. Since  $\zeta \# i$ , we note  $\zeta(\{s/i\}A) = \{\zeta(s)/i\}\zeta(A)$ . By application of the induction hypothesis we get

$$\Theta \mid \zeta(\Gamma); \zeta(\Delta_1) \vdash_\ell \zeta(t_1) : \zeta(\exists i : \sigma. A)$$

and

$$\Theta, s : \sigma \mid \zeta(\Gamma); \zeta(\Delta_2, a : \{s/i\}A) \vdash_\ell \zeta(t_2) : \zeta(B)$$

Combining the above, and using the definition of substitutions, we now get

$$\Theta \mid \zeta(\Gamma); \zeta(\Delta_1, \Delta_2) \vdash_\ell \zeta(\text{let } \{s, a\} = t_1 \text{ in } t_2) : \zeta(B)$$

as wanted. □

## 2.2 Cartesian term substitution

### 2.2.1 Cartesian weakening

Again, we will need the notion of Cartesian context weakening in order to prove the syntactic and semantic substitution lemmas.

**Definition 2.23** (Cartesian context membership). We define the Cartesian context membership relation  $x : X \in_\Theta \Gamma$  for a well-formed type  $\Theta \vdash_c X$  type and context  $\Theta \vdash_c \Gamma$  with the following rules and axioms:

$$\frac{}{x : X \in_\Theta \Gamma, x : X} \qquad \frac{x : X \in_\Theta \Gamma \quad x \neq x'}{x : X \in_\Theta \Gamma, x : X}$$



**Definition 2.24** (Subcontext relation). We define the subcontext relation  $\Gamma' \supseteq_{\Theta} \Gamma$  between well-formed contexts  $\Theta \vdash_c \Gamma'$  and  $\Theta \vdash_c \Gamma$  with the following rules and axioms:

$$\frac{}{\cdot \supseteq_{\Theta} \cdot} \quad \frac{\Gamma' \supseteq_{\Theta} \Gamma \quad x \notin \text{dom}(\Gamma')}{\Gamma', x : X \supseteq_{\Theta} \Gamma} \quad \frac{\Gamma' \supseteq_{\Theta} \Gamma \quad x \notin \text{dom}(\Gamma', \Gamma)}{\Gamma', x : X \supseteq_{\Theta} \Gamma, x : X}$$

**Lemma 2.25** (Weakening of Cartesian membership).

$$\frac{x : X \in_{\Theta} \Gamma \quad \Gamma' \supseteq_{\Theta} \Gamma}{x : X \in_{\Theta} \Gamma'}$$

*Proof.* We proceed by induction on the context membership  $x : X \in_{\Theta} \Gamma$ .

- $x : X \in_{\Theta} \Gamma'', x : X$ :  
By assumption,  $\Gamma' \supseteq_{\Theta} \Gamma'', x : X$ . There are two rules for the subcontext relation that can have this conclusion:
  - $\hat{\Gamma}, x : X \supseteq_{\Theta} \Gamma'', x : X$ : by the membership axiom, we have that  $x : X \in_{\Theta} \hat{\Gamma}, x : X$ , and since  $\hat{\Gamma}, x : X = \Gamma'$ , we get the required conclusion  $x : X \in_{\Theta} \Gamma'$ .
  - $\hat{\Gamma}, x' : X' \supseteq_{\Theta} \Gamma'', x : X$ : using the hypothesis  $\hat{\Gamma} \supseteq_{\Theta} \Gamma'', x : X$  and the fact that  $x : X \in_{\Theta} \Gamma'', x : X$ , the IH gives us  $x : X \in_{\Theta} \hat{\Gamma}$ . Extending this with an extra variable  $x' : X'$  gives  $x : X \in_{\Theta} \hat{\Gamma}, x' : X' = \Gamma'$ , as required.
- $x : X \in_{\Theta} \Gamma'', x' : X'$ :  
By assumption,  $\Gamma' \supseteq_{\Theta} \Gamma'', x' : X'$  and  $x : X \in_{\Theta} \Gamma''$ . There are two rules for the subcontext relation that can have this conclusion:
  - $\hat{\Gamma}, x' : X' \supseteq_{\Theta} \Gamma'', x' : X'$ : the hypotheses  $\hat{\Gamma} \supseteq_{\Theta} \Gamma''$  and  $x : X \in_{\Theta} \Gamma''$  give us  $x : X \in_{\Theta} \hat{\Gamma}$  by induction, and extending the context results in  $x : X \in_{\Theta} \hat{\Gamma}, x' : X' = \Gamma'$ , as required.
  - $\hat{\Gamma}, \hat{x} : \hat{X} \supseteq_{\Theta} \Gamma'', x' : X'$ : the hypotheses  $\hat{\Gamma} \supseteq_{\Theta} \Gamma'', x' : X'$  and  $x : X \in_{\Theta} \Gamma'', x' : X'$  give us  $x : X \in_{\Theta} \hat{\Gamma}$  by induction, and extending the context results in  $x : X \in_{\Theta} \hat{\Gamma}, x' : X' = \Gamma'$ , as required.

□

**Lemma 2.26** (Index weakening of Cartesian subcontext relation). Weakening of the  $\Theta$  index context gives us a way to weaken the Cartesian subcontext relation.

$$\frac{\Gamma' \supseteq_{\Theta} \Gamma \quad \Theta' \supseteq \Theta}{\Gamma' \supseteq_{\Theta'} \Gamma}$$

*Proof.* By induction on  $\Gamma' \supseteq_{\Theta} \Gamma$ .

□

**Lemma 2.27** (Cartesian weakening of Cartesian terms).

$$\frac{\Gamma' \supseteq_{\Theta} \Gamma \quad \Theta \mid \Gamma \vdash_c e : X}{\Theta \mid \Gamma' \vdash_c e : X}$$

*Proof.* By induction on the derivation of  $\Theta \mid \Gamma \vdash_c e : X$ . We show the cases for variables and abstraction – the rest of the terms follow directly from the (mutual) induction hypothesis.

- $\Theta \mid \Gamma \vdash_c x : X$ :  
By the hypotheses,  $x : X \in_\Theta \Gamma$  and  $\Gamma' \supseteq_\Theta \Gamma$ , so by Lemma 2.25, we get  $\Theta \mid \Gamma' \vdash_c x : X$ , as required.
- $\Theta \mid \Gamma \vdash_c \lambda x. e : X \rightarrow Y$ :  
The hypothesis of the rule is  $\Theta \mid \Gamma, x : X \vdash_c e : Y$ . In order to apply the induction hypothesis, we need to extend the subcontext assumption  $\Gamma' \supseteq_\Theta \Gamma$  to  $\Gamma', x : X \supseteq_\Theta \Gamma, x : X$  using the third rule of the definition. Then, applying the IH gives us  $\Theta \mid \Gamma', x : X \vdash_c e : Y$  and from the function typing rule we conclude that  $\Theta \mid \Gamma' \vdash_c \lambda x. e : X \rightarrow Y$ .

□

**Lemma 2.28** (Cartesian weakening of linear terms).

$$\frac{\Gamma' \supseteq_\Theta \Gamma \quad \Theta \mid \Gamma; \Delta \vdash_\ell t :_\tau A}{\Theta \mid \Gamma'; \Delta \vdash_\ell t :_\tau A}$$

*Proof.* We perform induction on the derivation of  $\Theta \mid \Gamma; \Delta \vdash_\ell t :_\tau A$ . Most of the linear terms (other than the F-binding) do not involve the Cartesian context so the proof follows by induction on the subterms. In the case of the index quantification rules, we need to perform index weakening on the Cartesian subcontext relation itself.

- $\Theta \mid \Gamma; \Delta_1, \Delta_2 \vdash_\ell \text{let } F \ x = t_1 \text{ in } t_2 : B$ :  
The two hypotheses of the rule are  $\Theta \mid \Gamma; \Delta_1 \vdash_\ell t_1 : F \ X$  and  $\Theta \mid \Gamma, x : X; \Delta_2 \vdash_\ell t_2 : B$ . By the IH on the first one, we get  $\Theta \mid \Gamma'; \Delta_1 \vdash_\ell t_1 : F \ X$ . To apply the IH on the second one, we need to extend the weakening to  $\Gamma', x : X \supseteq_\Theta \Gamma, x : X$  to get  $\Theta \mid \Gamma', x : X; \Delta_2 \vdash_\ell t_2 : B$ . Then, using the typing rule for F-binding we conclude that  $\Theta \mid \Gamma'; \Delta_1, \Delta_2 \vdash_\ell \text{let } F \ x = t_1 \text{ in } t_2 : B$ .
- $\Theta \mid \Gamma; \Delta \vdash_\ell \Lambda s : \sigma. t : \forall s : \sigma. A$ :  
The hypothesis of the rule is  $\Theta, i : \sigma \mid \Gamma; \Delta \vdash_\ell t : A$ . The subcontext relation  $\Gamma' \supseteq_\Theta \Gamma$  can be weakened using Lemma 2.26 to  $\Gamma' \supseteq_{\Theta, i : \sigma} \Gamma$  – this, combined with the assumption gives us  $\Theta, i : \sigma \mid \Gamma'; \Delta \vdash_\ell t : A$  by the IH. Finally, by applying the typing rule we conclude that  $\Theta \mid \Gamma'; \Delta \vdash_\ell \Lambda s : \sigma. t : \forall s : \sigma. A$ .
- $\Theta \mid \Gamma; \Delta_1, \Delta_2 \vdash_\ell \text{let } \{s, a\} = t_1 \text{ in } t_2 : B$ :  
Applying the IH to the first hypothesis gives  $\Theta \mid \Gamma'; \Delta_1 \vdash_\ell t_1 : \exists i : \sigma. A$ . To apply the IH to the second hypothesis, we need to weaken the subcontext relation assumption to get  $\Gamma' \supseteq_{\Theta, s : \sigma} \Gamma, x : X$  – induction then gives  $\Theta, s : \sigma \mid \Gamma'; \Delta_2, x : a\{s/i\} A \vdash_\ell t_2 : B$ . Applying the typing rule results in  $\Theta \mid \Gamma'; \Delta_1, \Delta_2 \vdash_\ell \text{let } \{s, a\} = t_1 \text{ in } t_2 : B$ , as required.

□

### 2.2.2 Cartesian substitution

**Definition 2.29** (Syntax of Cartesian term substitution). We define a simultaneous Cartesian term substitution as:

$$\xi ::= \diamond \mid \xi, x \mapsto e$$

where  $x$  is a Cartesian variable and  $e$  is a Cartesian expression.

**Definition 2.30** (Well-typed Cartesian substitutions). Given an index context  $\Theta$ , we define a well-typed Cartesian substitution, written  $\Theta \mid \Gamma' \vdash_c \xi \triangleright \Gamma$  by:

$$\frac{}{\Theta \mid \Gamma \vdash_c \diamond \triangleright \cdot} \quad \frac{\Theta \mid \Gamma' \vdash_c \xi \triangleright \Gamma \quad x \notin \text{dom}(\Gamma) \quad \Theta \mid \Gamma' \vdash_c e : X}{\Theta \mid \Gamma' \vdash_c (\zeta, x \mapsto e) \triangleright \Gamma, x : X}$$

**Definition 2.31** (Identity Cartesian substitution). We define the Cartesian identity substitution on a cartesian context  $\Gamma$ , denoted  $\text{id}_\Gamma$  by induction:

- $\text{id}_\cdot = \diamond$ .
- $\text{id}_{\Gamma, x : X} = \text{id}_\Gamma, (x \mapsto x)$ .

**Lemma 2.32** (Identity Cartesian substitution is the identity). For any term  $t$  and any Cartesian variable  $x$ , for the  $t = [\text{id}_{(x:X)}]t$ .

*Proof.* The proof follows by a simple induction over the definition of terms and the fact that we only consider terms up to  $\alpha$ -equivalence and hence can always assume  $x$  fresh.  $\square$

**Lemma 2.33** (Weakening Cartesian substitutions).

$$\frac{\Theta \mid \Gamma' \vdash_c \xi \triangleright \Gamma \quad \hat{\Gamma} \supseteq_\Theta \Gamma'}{\Theta \mid \hat{\Gamma} \vdash_c \xi \triangleright \Gamma}$$

*Proof.* We perform induction on  $\Theta \mid \Gamma' \vdash_c \xi \triangleright \Gamma$ .

- $\Theta \mid \Gamma' \vdash_c \diamond \triangleright \cdot$ : The conclusion  $\Theta \mid \hat{\Gamma} \vdash_c \diamond \triangleright \cdot$  follows directly from the empty substitution axiom.
- $\Theta \mid \Gamma' \vdash_c \xi, x \mapsto e \triangleright \Gamma, x : X$ : By assumption we have  $\Theta \mid \Gamma' \vdash_c \xi \triangleright \Gamma$  and  $\Theta \mid \Gamma' \vdash_c e : X$ . By the IH we have  $\Theta \mid \hat{\Gamma} \vdash_c \xi \triangleright \Gamma$  and by Lemma 2.27  $\Theta \mid \Gamma' \vdash_c e : X$ . Combining these we get  $\Theta \mid \hat{\Gamma} \vdash_c \xi, x \mapsto e \triangleright \Gamma, x : X$ , as required.

$\square$

**Lemma 2.34** (Cartesian substitution extension). If  $\Theta \mid \Gamma' \vdash_c \xi \triangleright \Gamma$  and  $x \notin \text{dom}(\Gamma) \cup \text{dom}(\Gamma')$  then  $\Theta \mid \Gamma', x : X \vdash_c (\xi, x \mapsto x) \triangleright \Gamma, x : X$

*Proof.* By the previous lemma and the axiom  $\Gamma', x : X \supseteq_\Theta \Gamma'$ , we have that  $\Theta \mid \Gamma', x : X \vdash_c \xi \triangleright \Gamma$ . We can extend it with the mapping  $x \mapsto x$  to get  $\Theta \mid \Gamma', x : X \vdash_c (\xi, x \mapsto x) \triangleright \Gamma, x : X$ , as required.  $\square$

**Definition 2.35** (Cartesian substitution into terms). Given a Cartesian expression  $e$ , we define the application of the Cartesian substitution  $\xi$  to  $e$ , written  $[\xi]e$  mutually inductively on the structure of expressions:

$$\begin{aligned} [\diamond]x &\triangleq x \\ [(\xi, x \mapsto e)]x &\triangleq e \\ [(\xi, x \mapsto e)]y &\triangleq [\xi]y & x \neq y \\ [\xi]\bullet &\triangleq \bullet \end{aligned}$$

$$\begin{aligned}
[\xi](\lambda x. e) &\triangleq \lambda x. [\xi]e & \xi \# x \\
[\xi](e_1 e_2) &\triangleq ([\xi]e_1) ([\xi]e_2) \\
[\xi]\mathbf{G} \, t &\triangleq \mathbf{G} \, ([\hat{\xi}]t)
\end{aligned}$$

Given a linear term  $t$ , we define the application of the Cartesian substitution  $\xi$  to  $t$ , written  $[\xi]t$  mutually inductively on the structure of expressions:

$$\begin{aligned}
[\xi]a &\triangleq a \\
[\xi](\lambda a. t) &\triangleq \lambda a. [\xi]t \\
[\xi](t_1 t_2) &\triangleq ([\xi]t_1) ([\xi]t_2) \\
[\xi]\langle \rangle &\triangleq \langle \rangle \\
[\xi](\text{let } \langle \rangle = t_1 \text{ in } t_2) &\triangleq \text{let } \langle \rangle = [\xi]t_1 \text{ in } [\xi]t_2 \\
[\xi]((t_1, t_2)) &\triangleq ([\xi]t_1, [\xi]t_2) \\
[\xi](\text{let } (a, b) = t_1 \text{ in } t_2) &\triangleq \text{let } (a, b) = [\xi]t_1 \text{ in } [\xi]t_2 \\
[\xi](\text{evt } t) &\triangleq \text{evt } ([\xi]t) \\
[\xi](\text{let evt } a = t_1 \text{ in } t_2) &\triangleq \text{let evt } a = [\xi]t_1 \text{ in } [\xi]t_2 \\
[\xi](t @ \tau) &\triangleq ([\xi]t) @ \tau \\
[\xi](\text{let } a @ \tau = t_1 \text{ in } t_2) &\triangleq \text{let } a @ \tau = [\xi]t_1 \text{ in } [\xi]t_2 \\
[\xi](\text{runG } e) &\triangleq \text{runG } ([\xi]e) \\
[\xi](\mathbf{F} \, e) &\triangleq \mathbf{F} \, ([\xi]e) \\
[\xi](\text{let } \mathbf{F} \, x = t_1 \text{ in } t_2) &\triangleq \text{let } \mathbf{F} \, x = [\xi]t_1 \text{ in } [\xi]t_2 & \xi \# x \\
[\xi](\Lambda i : \sigma. t) &\triangleq \Lambda i : \sigma. [\zeta(\xi)]t \\
[\xi](t_s) &\triangleq ([\xi]t)_s \\
[\xi](\{i, t\}) &\triangleq \{i, [\xi]t\} \\
[\xi](\text{let } \{s, a\} = t_1 \text{ in } t_2) &\triangleq \text{let } \{s, a\} = [\xi]t_1 \text{ in } [\xi]t_2 \\
[\xi](\text{select } (t_1, t_2) \text{ as } [a \mapsto t'_1] \parallel [b \mapsto t'_2]) &\triangleq \text{select } ([\xi]t_1, [\xi]t_2) \text{ as } [a \mapsto [\xi]t'_1] \parallel [b \mapsto [\xi]t'_2]
\end{aligned}$$

**Theorem 2.36** (Preservation of term well-formedness judgement under Cartesian substitution).

$$\frac{\Theta \mid \Gamma' \vdash_c \xi \triangleright \Gamma \quad \Theta \mid \Gamma \vdash_c e : X}{\Theta \mid \Gamma' \vdash_c [\xi]e : X} \qquad \frac{\Theta \mid \Gamma' \vdash_c \xi \triangleright \Gamma \quad \Theta \mid \Gamma; \Delta \vdash_\ell t :_\tau A}{\Theta \mid \Gamma'; \Delta \vdash_\ell [\xi]t :_\tau A}$$

*Proof.* We proceed by mutual induction over the typing judgement. Most cases follows directly by the definition of substitutions and/or application of the inductive hypothesis. We shall only prove the ones that do not. For the substitution into linear judgements, in most cases the judgement will always be “now”, i.e. of the form  $t :_0 A$ , and hence will not be changed by the substitution. In those cases we will not write the subscript.

- $(\Theta \mid \Gamma \vdash_c x : X)$ :

By definition of typing we know  $x : X \in \Gamma$ . By the definition of substitution then also know that  $[\xi]x : X \in \Gamma'$ . Hence we can conclude

$$\Theta \mid \Gamma' \vdash_c [\xi]x : X$$

as wanted.

- $(\Theta \mid \Gamma \vdash_c \lambda x.e : X \rightarrow Y)$ :

By typing we know

$$\Theta \mid \Gamma, x : X \vdash_c e : Y$$

Since we only consider terms up to alpha equivalence, we may assume  $\xi \# x$ . By Lemma 2.34 we get

$$\Theta \mid \Gamma', x : X \vdash_c (\xi, x \mapsto x) \triangleright \Gamma, x : X$$

and hence by application of the induction hypothesis

$$\Theta \mid \Gamma, x : X \vdash_c [\xi, x \mapsto x]e : Y.$$

By Lemma 2.32 we know  $[\xi, x \mapsto x]t = [\xi]t$  and hence we can conclude

$$\Theta \mid \Gamma' \vdash_c [\xi](\lambda x.t) : X \rightarrow Y$$

where we use the definition of substitutions.

- $(\Theta \mid \Gamma \vdash_c \mathsf{G} t : \mathsf{G} A)$ :

By definition of typing we know

$$\Theta \mid \Gamma; \cdot \vdash_\ell t : A$$

By application of the induction hypothesis we get

$$\Theta \mid \Gamma'; \cdot \vdash_\ell [\xi]t : A$$

Using the typing rule, we can thus conclude

$$\Theta \mid \Gamma' \vdash_c [\xi]\mathsf{G} t : \mathsf{G} A$$

where we have used the definition of substitution on terms.

- $(\Theta \mid \Gamma; a : A \vdash_\ell a : A)$ :

Since  $[\xi]a = a$ , we immediately get

$$\Theta \mid \Gamma'; a : A \vdash_\ell a : A$$

- $(\Theta \mid \Gamma; \cdot \vdash_\ell \mathsf{F} e : \mathsf{F} X)$ :

By typing we have

$$\Theta \mid \Gamma \vdash_c e : X$$

and then by application of the inductive hypothesis

$$\Theta \mid \Gamma' \vdash_c [\xi]e : X.$$

From this, and the definition of substitution we can now conclude

$$\Theta \mid \Gamma'; \cdot \vdash_\ell [\xi](F e) : F X$$

as wanted.

- $(\Theta \mid \Gamma; \Delta_1, \Delta_2 \vdash_\ell \text{let } F x = t_1 \text{ in } t_2 : B):$   
By typing we know

$$\Theta \mid \Gamma; \Delta_1 \vdash_\ell t_1 : F X$$

and

$$\Theta \mid \Gamma, x : X; \Delta_2 \vdash_\ell t_2 : B$$

By assumption we know that  $x$  is fresh for  $\Gamma$  and since we only consider terms up to alpha equivalence we may only consider it fresh for  $\Gamma'$  and hence also  $\zeta \# x$ . By Lemma 2.34 we know

$$\Theta \mid \Gamma', x : X \vdash_c \xi, x \mapsto x \triangleright \Gamma, x : X.$$

We can now apply the induction hypothesis twice to get

$$\Theta \mid \Gamma'; \Delta_1 \vdash_\ell [\xi]t_1 : F X$$

and

$$\Theta \mid \Gamma', x : X; \Delta_2 \vdash_\ell [\xi, x \mapsto x]t_2 : B$$

By Lemma 2.32 we know  $[\xi, x \mapsto x]t_2 = [\xi]t_2$ . We can now combine the above to conclude

$$\Theta \mid \Gamma'; \Delta_1, \Delta_2 \vdash_\ell [\xi](\text{let } F x = t_1 \text{ in } t_2) : B$$

where we also use the definition of substitution.

- $(\Theta \mid \Gamma; \Delta_1, \Delta_2 \vdash_\ell \text{let } a @ \tau = t_1 \text{ in } t_2 : B):$   
By typing  $\Theta \vdash_s \tau : \text{time}$ ,

$$\Theta \mid \Gamma; \Delta_1 \vdash_\ell t_1 : A @ \tau$$

and

$$\Theta \mid \Gamma; \Delta_2, a :_\tau A \vdash_\ell t_2 : B.$$

We note that since  $\xi$  is a Cartesian substitution, we trivially have  $\xi \# a$ . By two application of the induction hypothesis we then have

$$\Theta \mid \Gamma'; \Delta_1 \vdash_\ell [\xi]t_1 : A @ \tau$$

and

$$\Theta \mid \Gamma'; \Delta_2, a :_{\tau} A \vdash_{\ell} [\xi]t_2 : B.$$

ombining the above we can thus conclude:

$$\Theta \mid \Gamma; \Delta_1, \Delta_2 \vdash_{\ell} [\xi](\text{let } a @ \tau = t_1 \text{ in } t_2) : B)$$

where we have used the definition of substitutions.

- $(\Theta \mid \Gamma; \Delta \vdash_{\ell} t :_{\tau} A)$ :

By definition of typing we know  $\Theta \vdash_s \tau : \text{time}$ ,  $\Delta' = \Delta \downarrow^{\tau}$  and

$$\Theta \mid \Gamma; \Delta' \vdash_{\ell} t : A.$$

By application of the induction hypothesis we know

$$\Theta \mid \Gamma'; \Delta' \vdash_{\ell} [\xi]t : A$$

Combining the above we can thus conclude

$$\Theta \mid \Gamma'; \Delta \vdash_{\ell} [\xi]t :_{\tau} A$$

as wanted. □

### 2.3 Linear term substitution

**Definition 2.37** (Syntax of linear term substitution). We define a simultaneous Linear term substitution as:

$$\hat{\xi} ::= \diamond \mid \hat{\xi}, a \mapsto t$$

where  $a$  is a linear variable and  $t$  is a linear term.

**Definition 2.38** (Well-typed linear substitutions). Given an index context  $\Theta$ , we define a well-typed linear substitution, written  $\Theta; \Gamma \mid \Delta' \vdash_{\ell} \hat{\xi} \triangleright \Delta$  by:

$$\frac{}{\Theta; \Gamma \mid \cdot \vdash_{\ell} \diamond \triangleright \cdot} \quad \frac{\Theta; \Gamma \mid \Delta'_1 \vdash_{\ell} \hat{\xi} \triangleright \Delta_1 \quad a \notin \text{dom}(\Delta_1) \quad \Theta \mid \Gamma; \Delta'_2 \vdash_{\ell} t :_{\tau} A}{\Theta; \Gamma \mid \Delta'_1, \Delta'_2 \vdash_{\ell} \hat{\xi}, a \mapsto t \triangleright \Delta_1, a :_{\tau} A}$$

**Definition 2.39** (Concatenation of linear substitutions). Given two linear substitutions  $\Theta; \Gamma \mid \Delta'_1 \vdash_{\ell} \hat{\xi}_1 \triangleright \Delta_1$  and  $\Theta; \Gamma \mid \Delta'_2 \vdash_{\ell} \hat{\xi}_2 \triangleright \Delta_2$ , we define their concatenation  $\Theta; \Gamma \mid \Delta'_1, \Delta'_2 \vdash_{\ell} \hat{\xi}_1, \hat{\xi}_2 \triangleright \Delta_1, \Delta_2$  as:

$$\begin{aligned} & \Theta; \Gamma \mid \Delta'_1, \cdot \vdash_{\ell} \hat{\xi}_1, \diamond \triangleright \Delta_1, \cdot \triangleq \Theta; \Gamma \mid \Delta'_1 \vdash_{\ell} \hat{\xi}_1 \triangleright \Delta_1 \\ & \Theta; \Gamma \mid \Delta'_1, (\Delta'_2, \Delta'') \vdash_{\ell} \hat{\xi}_1, (\hat{\xi}_2, a \mapsto t) \triangleright \Delta_1, (\Delta_2, a : A) \triangleq (\Theta; \Gamma \mid \Delta'_1, \Delta'_2 \vdash_{\ell} \hat{\xi}_1, \hat{\xi}_2 \triangleright \Delta_1, \Delta_2), a \mapsto t \end{aligned}$$

**Definition 2.40** (Linear identity substitution). We define the linear identity substitution on a linear context  $\Delta$ , denoted  $\Theta; \Gamma \mid \Delta \vdash_{\ell} \text{id}_{\Delta} \triangleright \Delta$  by induction:

- $\hat{\text{id}}. = \diamond$ .
- $\hat{\text{id}}_{\Delta, a:A} = \hat{\text{id}}_{\Delta}, (a \mapsto a)$ .

**Lemma 2.41** (Linear identity substitution preserves terms). For any term  $t$  and any linear variable  $a$ , for the  $t = [\hat{\text{id}}_{(a:A)}]t$ .

*Proof.* The proof follows by a simple induction over the definition of terms and the fact that we only consider terms up to  $\alpha$ -equivalence and hence can always assume  $a$  fresh.  $\square$

**Lemma 2.42** (Linear identity extension). Given a well-typed linear substitution

$$\Theta; \Gamma \mid \Delta' \vdash_{\ell} \hat{\xi} \triangleright \Delta$$

and any linear context  $\Delta''$ , we have

$$\Theta; \Gamma \mid \Delta', \Delta'' \vdash_{\ell} \hat{\xi}, \hat{\text{id}}_{\Delta''} \triangleright \Delta, \Delta''$$

*Proof.* By induction on  $\Delta''$ .

- $\cdot$ :  
Since  $\hat{\xi}$  is also assumed to be a well-typed substitution, and  $\hat{\text{id}}. = \diamond$ ,  $\Theta; \Gamma \mid \Delta', \cdot \vdash_{\ell} \hat{\xi}, \diamond \triangleright \Delta, \cdot = \Theta; \Gamma \mid \Delta' \vdash_{\ell} \hat{\xi} \triangleright \Delta$  by the definition of context and substitution concatenation.
- $(\Delta'', a :_{\tau} A)$ :  
By application of the induction hypothesis, we get  $\hat{\xi}'$  s.t

$$\Theta; \Gamma \mid \Delta', \Delta'' \vdash_{\ell} \hat{\xi}, \hat{\xi}' \triangleright \Delta, \Delta''$$

By assumption  $a \notin \text{dom}(\Delta, \Delta'')$ . Trivially, we have

$$\Theta \mid \Gamma; a :_{\tau} A \vdash_{\ell} a :_{\tau} A$$

By definition of well-typed linear substitutions we can thus conclude

$$\Theta; \Gamma \mid \Delta', \Delta'', a :_{\tau} A \vdash_{\ell} \hat{\xi}, \hat{\xi}', a \mapsto a \triangleright \Delta, \Delta'', a :_{\tau} A$$

as wanted.  $\square$

**Lemma 2.43** (Linear substitution preserves time). For any well-typed linear substitution

$$\Theta; \Gamma \mid \Delta' \vdash_{\ell} \hat{\xi} \triangleright \Delta,$$

and some well-formed linear context  $\Delta_{\tau}$  s.t.  $\Delta \downarrow^{\tau} = \Delta_{\tau}$ , then there exists  $\Delta'_{\tau}$  s.t.  $\Delta' \downarrow^{\tau} = \Delta'_{\tau}$ .

*Proof.* By induction on  $\hat{\xi}$ .

- $(\Theta; \Gamma \mid \cdot \vdash_{\ell} \diamond \triangleright \cdot)$ :  
Since both  $\Delta'$  and  $\Delta$  is empty, the conclusion follows trivially by choosing  $\Delta'_{\tau} = \cdot$ .



- $(\Theta; \Gamma \mid \Delta'_1, \Delta'_2 \vdash_\ell \hat{\xi}, a \mapsto t \triangleright \Delta_1, a :_s A)$ :  
By definition of well-typed substitutions, we know  $a \notin \text{dom}(\Delta_1)$ ,

$$\Theta; \Gamma \mid \Delta'_1 \vdash_\ell \hat{\xi} \triangleright \Delta_1$$

and

$$\Theta \mid \Gamma; \Delta'_2 \vdash_\ell t :_s A$$

By assumption we have  $\Delta_\tau$  s.t.  $\Delta_\tau = (\Delta_1, a :_s A) \downarrow^\tau$ . By definition of context delay, we hence know that  $s = \tau$  and

$$(\Delta_1, a :_\tau A) \downarrow^\tau = (\Delta_1 \downarrow^\tau), a : A$$

Hence we know  $\Delta_\tau = (\Delta_1 \downarrow^\tau), a : A$ . We can thus write  $\Delta_\tau$  as  $\Delta'_\tau, a : A$  and we see that  $\Delta'_\tau = \Delta_1 \downarrow^\tau$ . By application of the induction hypothesis we now get  $\Delta'_\tau$  s.t.  $\Delta'_1 \downarrow^\tau = \Delta'_\tau$ . Since  $\tau = s$  we have

$$\Theta \mid \Gamma; \Delta'_2 \vdash_\ell t :_\tau A$$

and definition of typing we thus know  $\Theta \vdash_s \tau : \text{time}$  and

$$\Theta \mid \Gamma; \Delta''_2 \vdash_\ell t : A$$

where  $\Delta''_2 = \Delta'_2 \downarrow^\tau$ . We now set  $\Delta'_\tau = \Delta'_\tau, \Delta''_2$  and the conclusion follows by definition of context delays. □

**Lemma 2.44** (Splitting of linear substitutions). Given a well-typed linear substitution  $\Theta; \Gamma \mid \Delta' \vdash_\ell \hat{\xi} \triangleright \Delta_1, \Delta_2$ , then  $\hat{\xi}$  can be split into two well-typed substitutions  $\hat{\xi}_1$  and  $\hat{\xi}_2$ , with well-formed contexts  $\Delta'_1, \Delta'_2$  s.t.  $\Delta' = \Delta'_1, \Delta'_2$  and

$$\Theta; \Gamma \mid \Delta'_1 \vdash_\ell \hat{\xi}_1 \triangleright \Delta_1$$

and

$$\Theta; \Gamma \mid \Delta'_2 \vdash_\ell \hat{\xi}_2 \triangleright \Delta_2$$

such that  $\hat{\xi} = \hat{\xi}_1, \hat{\xi}_2$ .

*Proof.* By induction on  $\hat{\xi}$ .

- $\Theta; \Gamma \mid \cdot \vdash_\ell \diamond \triangleright \cdot, \cdot$ :  
We can choose  $\hat{\xi}_1 = \hat{\xi}_2 = \diamond$ , since  $\cdot, \cdot = \cdot$  and  $\diamond, \diamond = \diamond$ .
- $\Theta; \Gamma \mid \Delta, \Delta' \vdash_\ell \hat{\xi}, a \mapsto t \triangleright \Delta_1, \Delta_2, a :_\tau A$ :  
By the definition of well-typed substitutions,  $\Theta; \Gamma \mid \Delta \vdash_\ell \hat{\xi} \triangleright \Delta_1, \Delta_2$ , so the induction hypothesis on  $\hat{\xi}$  gives us  $\Theta; \Gamma \mid \Delta'_1 \vdash_\ell \hat{\xi}_1 \triangleright \Delta_1$  and  $\Theta; \Gamma \mid \Delta'_2 \vdash_\ell \hat{\xi}_2 \triangleright \Delta_2$ . Then, we split the original substitution  $\Theta; \Gamma \mid \Delta, \Delta' \vdash_\ell \hat{\xi}, a \mapsto t \triangleright \Delta_1, \Delta_2, a :_\tau A$  into

$$\Theta; \Gamma \mid \Delta'_1 \vdash_\ell \hat{\xi}_1 \triangleright \Delta_1$$

and

$$\Theta; \Gamma \mid \Delta'_2, \Delta' \vdash_\ell \hat{\xi}_2, a \mapsto t \triangleright \Delta_2, a :_\tau A$$

which satisfy the required conditions by the definition of well-typed substitutions.

□

**Lemma 2.45** (Delayed linear substitution). Give a well-typed linear substitution

$$\Theta; \Gamma \mid \Delta' \vdash_{\ell} \hat{\xi} \triangleright \Delta$$

and well-formed linear contexts  $\Theta \vdash_{\ell} \Delta'_{\tau}$ ,  $\Theta \vdash_{\ell} \Delta_{\tau}$  s.t.

$$\begin{aligned} \Delta' \downarrow^{\tau} &= \Delta'_{\tau} \\ \Delta \downarrow^{\tau} &= \Delta_{\tau} \end{aligned}$$

there exists a well-typed linear substitution

$$\Theta; \Gamma \mid \Delta'_{\tau} \vdash_{\ell} \hat{\xi}_{\tau} \triangleright \Delta_{\tau}$$

*Proof.* We proceed by induction over  $\hat{\xi}$ .

- $\Theta; \Gamma \mid \cdot \vdash_{\ell} \diamond \triangleright \cdot$ :  
Since both contexts are empty, choosing  $\hat{\xi}_{\tau} = \diamond$  trivially gives the conclusion.
- $\Theta; \Gamma \mid \Delta'_1, \Delta'_2 \vdash_{\ell} \hat{\xi}', a \mapsto t \triangleright \Delta_1, a :_s A$ :  
By definition of a well-typed substitution, we know that

$$\Theta; \Gamma \mid \Delta'_1 \vdash_{\ell} \hat{\xi}' \triangleright \Delta_1,$$

$a \notin \text{dom}(\Delta_1)$  and

$$\Theta \mid \Gamma; \Delta'_2 \vdash_{\ell} t :_{\tau} A.$$

We start by noting that  $s = \tau$ . By definition we then know that

$$\Delta_1, a :_{\tau} A \downarrow^{\tau} = (\Delta_1 \downarrow^{\tau}), a : A.$$

By Lemma 2.43 we then get  $\Delta'_{1\tau}$  s.t.  $\Delta'_1 \downarrow^{\tau} = \Delta'_{1\tau}$ . By application of the induction hypothesis we then get

$$\Theta; \Gamma \mid \Delta'_{1\tau} \vdash_{\ell} \hat{\xi}_1 \triangleright \Delta_1 \downarrow^{\tau}.$$

By the definition of typing we know that

$$\Theta \mid \Gamma; \Delta'_{2\tau} \vdash_{\ell} t : A.$$

s.t.  $\Delta'_2 \downarrow^{\tau} = \Delta'_{2\tau}$ . We know  $(a :_{\tau} A) \downarrow^{\tau} = a : A$ . We can thus create the substitution

$$\Theta; \Gamma \mid \Delta'_{2\tau} \vdash_{\ell} a \mapsto t \triangleright a : A.$$

Combining the above we thus get

$$\Theta; \Gamma \mid \Delta'_{1\tau}, \Delta'_{2\tau} \vdash_{\ell} \hat{\xi}_1, a \mapsto t \triangleright \Delta_1 \downarrow^{\tau}, a : A$$

as wanted. □

**Corollary 2.46** (Application of delayed substitutions). Given  $\hat{\xi}$  and  $\hat{\xi}_\tau$  as described in Lemma 2.45, then for any term  $t$  we have

$$[\hat{\xi}]t = [\hat{\xi}_\tau]t$$

*Proof.* This follows directly by definition of substitutions and the fact that neither variable names nor terms change between  $\hat{\xi}$  and  $\hat{\xi}_\tau$ .  $\square$

**Definition 2.47** (Linear substitution into terms). Linear substitution into Cartesian terms in a no-op: most of the terms do not involve the linear context, and while  $\mathbf{G} t$  has a linear subterm, its linear context is empty and therefore there are no free linear variables to apply the substitution to (which will necessarily be  $\Theta; \Gamma \mid \cdot \vdash_\ell \diamond \triangleright \cdot$ ).

Given a linear term  $t$ , we define the application of the linear substitution  $\hat{\xi}$  to  $t$ , written  $[\hat{\xi}]t$  mutually inductively on the structure of expressions:

$$\begin{aligned}
[\hat{\xi}]a &\triangleq a \\
[\diamond]a &\triangleq a \\
[(\xi, a \mapsto t)]a &\triangleq t \\
[(\xi, a \mapsto t)]b &\triangleq [\hat{\xi}]b && x \neq y \\
[\hat{\xi}](\lambda a. t) &\triangleq \lambda a. [\hat{\xi}]t && \hat{\xi} \# a \\
[\hat{\xi}](t_1 t_2) &\triangleq ([\hat{\xi}]t_1) ([\hat{\xi}]t_2) \\
[\hat{\xi}]\langle \rangle &\triangleq \langle \rangle \\
[\hat{\xi}](\text{let } \langle \rangle = t_1 \text{ in } t_2) &\triangleq \text{let } \langle \rangle = [\hat{\xi}]t_1 \text{ in } [\hat{\xi}]t_2 \\
[\hat{\xi}](t_1, t_2) &\triangleq ([\hat{\xi}]t_1, [\hat{\xi}]t_2) \\
[\hat{\xi}](\text{let } (a, b) = t_1 \text{ in } t_2) &\triangleq \text{let } (a, b) = [\hat{\xi}]t_1 \text{ in } [\hat{\xi}]t_2 && \hat{\xi} \# a, b \\
[\hat{\xi}](\text{evt } t) &\triangleq \text{evt } ([\hat{\xi}]t) \\
[\hat{\xi}](\text{let evt } a = t_1 \text{ in } t_2) &\triangleq \text{let evt } a = [\hat{\xi}]t_1 \text{ in } t_2 && \hat{\xi} \# a \\
[\hat{\xi}](t @ \tau) &\triangleq ([\hat{\xi}]t) @ \tau \\
[\hat{\xi}](\text{let } a @ \tau = t_1 \text{ in } t_2) &\triangleq \text{let } a @ \tau = [\hat{\xi}]t_1 \text{ in } [\hat{\xi}]t_2 && \hat{\xi} \# a \\
[\hat{\xi}](\text{runG } e) &\triangleq \text{runG } e \\
[\hat{\xi}](\mathbf{F} e) &\triangleq \mathbf{F} e \\
[\hat{\xi}](\text{let } \mathbf{F} x = t_1 \text{ in } t_2) &\triangleq \text{let } \mathbf{F} x = [\hat{\xi}]t_1 \text{ in } [\hat{\xi}]t_2 \\
[\hat{\xi}](\Lambda i : \sigma. t) &\triangleq \Lambda i : \sigma. [\hat{\xi}]t \\
[\hat{\xi}](t_s) &\triangleq ([\hat{\xi}]t)_s \\
[\hat{\xi}](\{i, t\}) &\triangleq \{i, [\hat{\xi}]t\} \\
[\hat{\xi}](\text{let } \{s, a\} = t_1 \text{ in } t_2) &\triangleq \text{let } \{s, a\} = [\hat{\xi}]t_1 \text{ in } [\hat{\xi}]t_2 && \hat{\xi} \# a \\
[\hat{\xi}](\text{select } (t_1, t_2) \text{ as } [a \mapsto t'_1] \parallel [b \mapsto t'_2]) &\triangleq \text{select } ([\hat{\xi}]t_1, [\hat{\xi}]t_2) \text{ as } [a \mapsto t'_1] \parallel [b \mapsto t'_2] && \hat{\xi} \# a, b
\end{aligned}$$

Note that the substitution is not always applied to all subterms, if the subterm is a Cartesian expression (such as  $[\hat{\xi}](\text{runG } e) = \text{runG } e$ ) or its linear context is restricted (such as event binding, where the context of the body consists only of the bound variable which is assumed not to be in  $\hat{\xi}$ ).

**Theorem 2.48** (Preservation of term wellformedness judgment under linear substitution).

$$\frac{\Theta; \Gamma \mid \Delta \vdash_{\ell} \hat{\xi} \triangleright \Delta' \quad \Theta \mid \Gamma; \Delta \vdash_{\ell} t : A}{\Theta \mid \Gamma; \Delta' \vdash_{\ell} [\hat{\xi}]t : A}$$

*Proof.* We proceed by induction over the typing judgement. Many of the cases follows by definition of substitutions and/or application of the induction hypothesis. We will only do the interesting cases.

- $(\Theta \mid \Gamma; a : A \vdash_{\ell} a : A) :$   
The only well-typed substitution in this case is the identity substitution  $\Theta; \Gamma \mid a : A \vdash_{\ell} \text{id}_{a:A} \triangleright a : A$  and hence the conclusion follows by assumption.
- $(\Theta \mid \Gamma; \Delta \vdash_{\ell} \lambda a. t : A \multimap B) :$   
By definition of typing we know that

$$\Theta \mid \Gamma; \Delta, a : A \vdash_{\ell} t : B.$$

Since we only work up to alpha equivalence of terms, we may assume  $\hat{\xi} \# a$ . By definition of well-formed contexts, we know that  $a \notin \text{dom}(\Delta)$ . Trivially,  $\Theta \mid \Gamma; a : A \vdash_{\ell} a : A$ . We can now form the substitution

$$\Theta; \Gamma \mid \Delta', a : A \vdash_{\ell} \hat{\xi}, a \mapsto a \triangleright \Delta, a : A.$$

By application of the induction hypothesis we get:

$$\Theta \mid \Gamma; \Delta', a : A \vdash_{\ell} [\hat{\xi}, a \mapsto a]t : B.$$

By Lemma 2.41, the definition of substitutions and the fact  $\hat{\xi} \# a$ , we know that

$$[\hat{\xi}, a \mapsto a]t = [\hat{\xi}]t$$

We thus have

$$\Theta \mid \Gamma; \Delta', a : A \vdash_{\ell} [\hat{\xi}]t : B.$$

and by typing and the definition of substitution, we can now conclude

$$\Theta \mid \Gamma; \Delta' \vdash_{\ell} [\hat{\xi}](\lambda a. t) : A \multimap B$$

as wanted.

- $(\Theta \mid \Gamma; \Delta_1, \Delta_2 \vdash_{\ell} \text{let } (a, b) = t_1 \text{ in } t_2 : C) :$   
We have two cases depending on whether  $t_1 : A \otimes B$  or  $t_1 :_{\tau} A \otimes B$ . We will only do the latter case, as the former is a special case of this. By definition of typing we then know  $\Theta \vdash_s \tau : \text{time}$ ,

$$\Theta \mid \Gamma; \Delta_1 \vdash_{\ell} t_1 :_{\tau} A \otimes B$$

and

$$\Theta \mid \Gamma; \Delta_2, a :_{\tau} A, b :_{\tau} B \vdash_{\ell} t_2 : C$$

Since we only consider terms up to alpha equivalence, we may assume  $\hat{\xi} \# a$  and  $\hat{\xi} \# y$ . By Lemma 2.44 we get

$$\Theta; \Gamma \mid \Delta'_1 \vdash_{\ell} \hat{\xi}_1 \triangleright \Delta_1$$

and

$$\Theta; \Gamma \mid \Delta'_2 \vdash_{\ell} \hat{\xi}_2 \triangleright \Delta_2$$

s.t.  $\Delta' = \Delta'_1, \Delta'_2$ . By definition of well-formed contexts, we know that  $a, b \notin \Delta_2$ . By Lemma 2.42 we get

$$\Theta; \Gamma \mid \Delta'_2, a :_{\tau} A, b :_{\tau} B \vdash_{\ell} \hat{\xi}_2, a \mapsto a, b \mapsto b \triangleright \Delta_2, a :_{\tau} A, b :_{\tau} B.$$

By application of the induction hypothesis and then Lemma 2.41 we get

$$\Theta \mid \Gamma; \Delta'_2, a :_{\tau} A, b :_{\tau} B \vdash_{\ell} [\hat{\xi}_2]t_2 : C.$$

By a second application of the induction hypothesis we get

$$\Theta \mid \Gamma; \Delta'_1 \vdash_{\ell} [\hat{\xi}_1]t_1 :_{\tau} A \otimes B.$$

Combining the above, and using the definition of well-typed linear substitutions, we can now conclude

$$\Theta \mid \Gamma; \Delta' \vdash_{\ell} [\hat{\xi}](\text{let } (a, b) = t_1 \text{ in } t_2) : C$$

as wanted.

- $(\Theta \mid \Gamma; \Delta \vdash_{\ell} t @ \tau : A @ \tau):$

By definition of typing we know that  $\Theta \vdash_s \tau : \text{time}$  and

$$\Theta \mid \Gamma; \Delta \vdash_{\ell} t :_{\tau} A$$

By application of the induction hypothesis we get

$$\Theta \mid \Gamma; \Delta' \vdash_{\ell} [\hat{\xi}]t :_{\tau} A$$

and then by typing, and then definition of substitution,

$$\Theta \mid \Gamma; \Delta \vdash_{\ell} [\hat{\xi}](t @ \tau) : A @ \tau$$

as wanted.

- $(\Theta \mid \Gamma; \Delta_1, \Delta_2 \vdash_{\ell} \text{let } a @ \tau = t_1 \text{ in } t_2 : C):$

By definition of typing we know that  $\Theta \vdash_s \tau : \text{time}$ ,

$$\Theta \mid \Gamma; \Delta_1 \vdash_{\ell} t_1 : A @ \tau$$

and

$$\Theta \mid \Gamma; \Delta_2, a :_{\tau} A \vdash_{\ell} t_2 : C.$$

Since we only consider terms up to alpha equivalence, we may assume  $\hat{\xi} \# a$ . By Lemma 2.44 we get

$$\Theta; \Gamma \mid \Delta'_1 \vdash_{\ell} \hat{\xi}_1 \triangleright \Delta_1$$

and

$$\Theta; \Gamma \mid \Delta'_1 \vdash_{\ell} \hat{\xi}_1 \triangleright \Delta_1$$

s.t.  $\Delta' = \Delta'_1, \Delta'_2$ . By definition of well-formed contexts, we know that  $x \notin \Delta_2$ . By Lemma 2.42 we get

$$\Theta; \Gamma \mid \Delta'_2, a :_{\tau} A \vdash_{\ell} \hat{\xi}_2, x \mapsto x \triangleright \Delta_2, a :_{\tau} A.$$

By application of the induction hypothesis and then Lemma 2.41 we get

$$\Theta \mid \Gamma; \Delta'_2, a :_{\tau} A \vdash_{\ell} [\hat{\xi}_2]t_2 : C.$$

By a second application of the induction hypothesis, we get

$$\Theta \mid \Gamma; \Delta'_1 \vdash_{\ell} [\hat{\xi}]t_1 : A @ \tau$$

Combining the above, and using the definition of substitutions, we can now conclude

$$\Theta \mid \Gamma; \Delta' \vdash_{\ell} [\hat{\xi}](\text{let } a @ \tau = t_1 \text{ in } t_2) : C$$

as wanted.

- $(\Theta \mid \Gamma; \cdot \vdash_{\ell} \text{runG } e : A)$ :  
Since the linear context of the term is  $\cdot$ , the substitution must be of the form  $\Theta; \Gamma \mid \cdot \vdash_{\ell} \diamond \triangleright \cdot$  so  $\Theta \mid \Gamma; \cdot \vdash_{\ell} [\diamond](\text{runG } e) : A$  holds directly.
- $(\Theta \mid \Gamma; \cdot \vdash_{\ell} \text{F } e : \text{F } X)$ :  
Similar to above.
- $(\Theta \mid \Gamma; \Delta_1, \Delta_2 \vdash_{\ell} \text{let F } x = t_1 \text{ in } t_2 : B)$ :  
By typing we know  $\Theta \mid \Gamma; \Delta_1 \vdash_{\ell} t_1 : \text{F } X$  and  $\Theta \mid \Gamma, x : X; \Delta_2 \vdash_{\ell} t_2 : B$ . From the substitution  $\Theta; \Gamma \mid \Delta'_1, \Delta'_2 \vdash_{\ell} \hat{\xi} \triangleright \Delta_1, \Delta_2$  Lemma 2.44 we get

$$\Theta; \Gamma \mid \Delta'_1 \vdash_{\ell} \hat{\xi}_1 \triangleright \Delta_1$$

and

$$\Theta; \Gamma \mid \Delta'_2 \vdash_{\ell} \hat{\xi}_2 \triangleright \Delta_2$$

s.t.  $\Delta' = \Delta'_1, \Delta'_2$ . By the IH on the first substitution and t\_1 we get  $\Theta \mid \Gamma; \Delta'_1 \vdash_{\ell} [\hat{\xi}_1]t_1 : \text{F } X$ . The second substitution is weakened by  $\Gamma, x : X \supseteq_{\Theta} \Gamma$  to get  $\Theta; \Gamma, x : X \mid \Delta'_2 \vdash_{\ell} \hat{\xi}_2 \triangleright \Delta_2$ , and the IH gives us  $\Theta \mid \Gamma, x : X; \Delta'_2 \vdash_{\ell} [\hat{\xi}_2]t_2 : B$ . Combining the two terms and applying the def. of substitution on linear terms we get  $\Theta \mid \Gamma; \Delta'_1, \Delta'_2 \vdash_{\ell} [\hat{\xi}](\text{let F } x = t_1 \text{ in } t_2) : B$ , as required.

- $(\Theta \mid \Gamma; \Delta_1, \Delta_2 \vdash_\ell \text{let } \{s, a\} = t_1 \text{ in } t_2 : B)$ :  
By typing we know

$$\Theta \mid \Gamma; \Delta_1 \vdash_\ell t_1 : \exists(i : \sigma).A$$

and

$$\Theta, s : \sigma \mid \Gamma; \Delta_2, a : \{s/i\}A \vdash_\ell t_2 : B$$

Since we only consider terms up to alpha equivalence, we may assume  $\zeta \# x$ . By Lemma 2.44 we get

$$\Theta; \Gamma \mid \Delta'_1 \vdash_\ell \hat{\xi}_1 \triangleright \Delta_1$$

and

$$\Theta; \Gamma \mid \Delta'_2 \vdash_\ell \hat{\xi}_2 \triangleright \Delta_2$$

s.t.  $\Delta' = \Delta'_1, \Delta'_2$ . By definition of well-formed contexts, we know that  $x \notin \Delta_2$ . By Lemma 2.42 we get

$$\Theta; \Gamma \mid \Delta'_2, a : \{s/i\}A \vdash_\ell \hat{\xi}_2, a \mapsto a \triangleright \Delta_2, a : \{s/i\}A.$$

By application of the induction hypothesis and then Lemma 2.41 we get

$$\Theta \mid \Gamma; \Delta'_2, a : \{s/i\}A \vdash_\ell [\hat{\xi}_2]t_2 : B.$$

By a second application of the induction hypothesis, we get

$$\Theta \mid \Gamma; \Delta'_1 \vdash_\ell [\hat{\xi}]t_1 : \exists(i : \sigma).A.$$

Combining the above, and using the definition of substitutions, we can now conclude

$$\Theta \mid \Gamma; \Delta' \vdash_\ell [\hat{\xi}](\text{let } \{s, a\} = t_1 \text{ in } t_2) : B$$

as wanted.

- $(\Theta \mid \Gamma; \Delta_1, \Delta_2 \vdash_\ell \text{select } (t_1, t_2) \text{ as } [a \mapsto t'_1] \parallel [b \mapsto t'_2] : \Diamond C)$ :  
By definition of typing we get

$$\Theta \mid \Gamma; \Delta_1 \vdash_\ell t_1 : \Diamond A,$$

$$\Theta \mid \Gamma; \Delta_2 \vdash_\ell t_2 : \Diamond B,$$

$$\Theta \mid \Gamma; a : A, b : \Diamond B \vdash_\ell t'_1 : \Diamond C$$

and

$$\Theta \mid \Gamma; a : \Diamond A, b : B \vdash_\ell t'_1 : \Diamond C$$

By two applications of the induction hypothesis we get

$$\Theta \mid \Gamma; \Delta'_1 \vdash_\ell [\hat{\xi}]t_1 : \Diamond A,$$

$$\Theta \mid \Gamma; \Delta'_2 \vdash_\ell [\hat{\xi}]t_2 : \Diamond B,$$

Since  $t'_1$  and  $t'_2$  does not depend on anything in  $\Delta_1, \Delta_2$ , we trivially have  $[\hat{\xi}]t'_1 = t'_1$  and  $[\hat{\xi}]t'_2 = t'_2$ . Combining the above and using the definition of substitution, we can thus conclude

$$\Theta \mid \Gamma; \Delta' \vdash_\ell [\hat{\xi}](\text{select } (t_1, t_2) \text{ as } [a \mapsto t'_1] \parallel [b \mapsto t'_2]) : \Diamond C$$

as wanted.

- $(\Theta \mid \Gamma; \Delta \vdash_\ell t :_\tau A)$ :

By definition of typing we know  $\Theta \vdash_s \tau : \text{time}$ ,  $\Delta'' = \Delta \downarrow^\tau$  and

$$\Theta \mid \Gamma; \Delta'' \vdash_\ell t : A$$

By Lemma 2.43 we get  $\Delta'_\tau$  s.t.  $\Delta' \downarrow^\tau = \Delta'_\tau$ . By application of the induction hypothesis we get

$$\Theta \mid \Gamma; \Delta'' \vdash_\ell t : A$$

By Lemma 2.45 we get

$$\Theta; \Gamma \mid \Delta'_\tau \vdash_\ell \hat{\xi}' \triangleright \Delta''.$$

By application of the induction hypothesis with  $\hat{\xi}'$  we get

$$\Theta \mid \Gamma; \Delta'_\tau \vdash_\ell [\hat{\xi}']t : A$$

and then by definition of typing and the fact that  $\Delta'_\tau = \Delta' \downarrow^\tau$ ,

$$\Theta \mid \Gamma; \Delta' \vdash_\ell [\hat{\xi}']t :_\tau A$$

By Corollary 2.46 we know  $[\hat{\xi}']t = [\hat{\xi}]t$  and hence we have

$$\Theta \mid \Gamma; \Delta' \vdash_\ell [\hat{\xi}]t :_\tau A$$

as wanted

□

### 3 The Category of Reactive Types

The categorical semantics of our language is built upon *reactive types*, implemented as time-indexed sets. However, rather than simply using  $\mathbf{Set}^{\mathbb{N}}$ , we will work on the presheaf category  $\mathbf{Set}^{\mathbb{N}_{\top}^{\text{op}}}$  introduced below. We will usually denote  $\mathbf{Set}^{\mathbb{N}_{\top}^{\text{op}}}$  as  $\mathcal{R}$ .



### 3.1 Objects and arrows

The objects are presheaves on the category of flat natural numbers with a top element  $\mathbb{N}_\top$ , and the arrows are natural transformations between two such presheaves. We can visualize an object in  $\mathcal{R}$  as a series of disconnected sets  $A_n$  indexed by natural numbers, with with set  $A_\top$  at the top point with projections  $\pi_n^A: A_\top \rightarrow A_n$  for all naturals  $n$ .

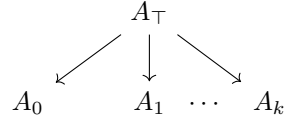

An arrow  $f: A \rightarrow B$  is a collection of maps  $f_\top, f_0, f_1, \dots$  in **Set**, with a coherence condition ensuring commutativity of all squares (which is just the naturality condition for the natural transformation between the two presheaves).

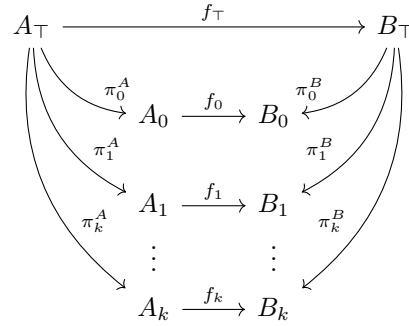

The commutativity then states that for all  $n \in \mathbb{N}$ ,  $f_n \circ \pi_n^A = \pi_n^B \circ f_\top$ , or as a diagram:

$$\begin{array}{ccc}
 A_\top & \xrightarrow{f_\top} & B_\top \\
 \pi_n^A \downarrow & & \downarrow \pi_n^B \\
 A_n & \xrightarrow{f_n} & B_n
 \end{array}$$

### 3.2 Topos structure

As  $\mathbf{Set}^{\mathbb{N}_\top^{\text{op}}}$  is a presheaf category, it gets the bi-Cartesian closed structure of **Set** by pointwise indexing. In addition,  $\mathbf{Set}^{\mathbb{N}_\top^{\text{op}}}$  also has a topos structure, exhibited by a canonical object of truth values  $\Omega$  defined at  $k \in \mathbb{N}_\top$  as the set of sieves on  $k$ . We can calculate this explicitly as the following object  $\Omega \in \mathcal{R}$  (where  $\mathbb{1} = \{*\}$  is the terminal singleton set and  $\mathbb{B} = \{0, 1\}$  is the set of Boolean values):

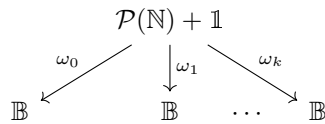

with the projections  $\pi_n^\Omega$ , which we will denote  $\omega_n: \mathcal{P}(\mathbb{N}) + \mathbb{1} \rightarrow \mathbb{B}$ , defined as:

$$\begin{aligned}\omega_n(\text{inr } *) &\triangleq 1 \\ \omega_n(\text{inl } N) &\triangleq n \in N\end{aligned}$$

Equivalently,  $\omega_n$  is the copairing  $[n \in -, \text{true}_{\text{Set}}]: \mathcal{P}(\mathbb{N}) + \mathbb{1} \rightarrow \mathbb{B}$ , where  $\text{true}_{\text{Set}} = * \mapsto 1$  is the subobject classifier in **Set**. The subobject classifier in  $\mathcal{R}$ ,  $\text{true}: \mathbb{1} \rightarrow_{\mathcal{R}} \Omega \in \mathcal{R}$ , is defined as:

$$\begin{aligned}\text{true}_\top(*) &\triangleq \text{inr } * \\ \text{true}_n(*) &\triangleq 1\end{aligned}$$

This is a well-defined map in  $\mathcal{R}$ , since projections from  $\mathbb{1}_\top = \mathbb{1}$  are just the identity  $\text{id}_\mathbb{1}$ , so we have the coherence condition

$$(\text{true}_n \circ \text{id}_\mathbb{1})(*) = \text{true}_n(*) = 1 = \omega_n(\text{inr } *) = (\omega_n \circ \text{true}_\top)(*)$$

Intuitively, truth at the individual projections corresponds to standard Boolean truth or falsity. However, at the top point, we can distinguish between global truth (the right injection of  $\mathcal{P}(\mathbb{N}) + \mathbb{1}$ ), or truth only at certain timesteps (the left injection). In particular, we can differentiate between something being true at every timestep but not at the top point (corresponding to  $\text{inl } \mathbb{N}$ ), and something being true at “globally”, in the top point as well (corresponding to  $\text{inr } *$ ). Accordingly, for a global truth value  $P \in \Omega_\top = \mathcal{P}(\mathbb{N}) + \mathbb{1}$ , we will simply write  $P$  for the Boolean predicate “ $P$  is globally true”, i.e.  $P = \text{inr } *$ . For instance,  $\text{true}_\top(*)$  holds, because  $\text{true}_\top(*) = \text{inr } *$ .

To show that  $\text{true}$  is a subobject classifier, we need to show that every subobject  $S$  of  $A \in \text{Rel}_{\mathcal{R}}$  determines a characteristic function  $\chi_S: A \rightarrow_{\mathcal{R}} \Omega$ :

$$\begin{array}{ccc} S & \xrightarrow{!_S} & \mathbb{1} \\ m \downarrow & & \downarrow \text{true} \\ A & \xrightarrow{\chi_S} & \Omega \end{array}$$

We define the characteristic function  $\chi_S: A \rightarrow_{\mathcal{R}} \Omega$  as:

$$\begin{aligned}(\chi_S)_n(a: A_n) &\triangleq a \in S_n \\ (\chi_S)_\top(a: A_\top) &\triangleq \begin{cases} \text{inr } * & \text{if } a \in S_\top \\ \text{inl } \{n \in \mathbb{N} \mid \pi_n^A(a) \in S_n\} & \text{otherwise} \end{cases}\end{aligned}$$

The projections are standard set-theoretic characteristic functions on the subset  $S_n$ . At the top point we need to handle two possibilities: if  $a \in A_\top$  is also in the subset  $S_\top$ , we return the “global truth”  $\text{inr } *$ . If  $a \notin S_\top$ , not all is lost, as the element may still be in one of the projections; we collect all the time steps  $n$  for which  $\pi_n^A(a) \in S_n$  in the left injection. The commutativity condition

$$\chi_S \circ m = \text{true} \circ !_S$$

becomes

$$\begin{aligned}(\chi_S)_n(m_n(s \in S_n)) &= m_n(s) \in S_n = 1 = \text{true}_n(!_S(s)) \\ (\chi_S)_\top(m_\top(s \in S_\top)) &= \text{inr } * = \text{true}_\top(!_S(s))\end{aligned}$$

**Power objects** Since  $\mathcal{R}$  is a topos, it must have power objects given by the exponential  $\Omega^-$ . The canonical construction of exponentials of presheaves is the following:

**Definition 3.1** (Exponential object in presheaf categories). Given a locally small category  $\mathcal{C}$ , the exponential of two presheaves  $A, B \in \mathbf{Set}^{\mathcal{C}^{\text{op}}}$  is defined as

$$\begin{aligned} B^A(C) &\triangleq \mathbf{Set}^{\mathcal{C}^{\text{op}}}(y_C \times A, B) \\ B^A(f) &\triangleq \mathbf{Set}^{\mathcal{C}^{\text{op}}}(y_f \times A, B) \end{aligned}$$

where  $y_- : \mathcal{C} \rightarrow \mathbf{Set}^{\mathcal{C}^{\text{op}}}$ ,  $A \mapsto \mathbf{Set}(-, A)$  is the Yoneda embedding of objects in  $\mathcal{C}$  into presheaves on  $\mathcal{C}$ . Thus, the power object of  $A$  in a presheaf topos is  $\Omega^A$ , a generalisation of the powerset.

For  $\mathcal{C} = \mathbb{N}_{\top}$ , we can calculate the power object  $P(A) \in \mathcal{R}$  of  $A \in \mathcal{R}$  explicitly to be.

$$\begin{aligned} P(A)_{\top} &\triangleq \mathcal{R}(A, \Omega) \\ P(A)_n &\triangleq \mathcal{P}(A_n) \\ \pi_n^{P(A)}(s) &\triangleq s_n \end{aligned}$$

The power object of  $A$  at each timestep  $n$  is the powerset of  $A_n$ , while at the top point it is the set of morphisms from  $A$  to the subobject classifier. Projections at time  $n$  map a morphism  $s : A \rightarrow \Omega$  to the morphism  $s_n : A_n \rightarrow \Omega_n = A_n \rightarrow \mathbb{B}$ , which is the characteristic function of a subset of  $A_n$  and therefore isomorphic to an element of  $\mathcal{P}(A_n)$ . We can show that the definition of  $P(A)$  is isomorphic to the canonical power object in presheaf toposes, so  $P$  is precisely the power object functor in  $\mathcal{R}$ .

**Shorthand notation for  $\mathcal{R}$ -predicates** Given that we will mostly working in the category of internal relations on  $\mathcal{R}$ , the majority of the constructs that we define will be  $\Omega$ -valued relations and predicates. Because of the structure of  $\Omega \in \mathcal{R}$ , defining functions  $f : A \rightarrow_{\mathcal{R}} \Omega$  can become quite cumbersome, given that we need to handle the projections  $f_n$ , and return the appropriate injection in the top case  $f_{\top}$ . Looking at our definition for  $\chi_S$ , we can notice a lot of similarities between the three set-theoretic predicates that determine the cases of the definition: we have  $a \in S_n$  for  $a \in A_n$ , and  $a \in S_{\top}$  or  $\pi_n^A(a) \in S_n$  for  $a \in A_{\top}$ . In fact,  $\pi_n^A(a) \in S_n$  is analogous to  $(\chi_S)_n(\pi_n^A(a))$  for  $a \in A_{\top}$ , and this will be the case for most of our definitions. To make the rest of the discussion clearer and more concise, we will abuse the notation somewhat and define  $\Omega$ -valued functions as if they were standard Boolean-valued predicates, with the understanding that the definition can be extended to a proper  $\Omega$ -valued  $\mathcal{R}$  morphism in a canonical way.

In this shorthand notation, we will define  $f : A \rightarrow_{\mathcal{R}} \Omega$  as

$$f(a : A) \triangleq P(a)$$

for a Boolean-valued expression  $P$  that involves  $\mathcal{R}$ -objects and morphisms as if they were simple sets and functions, and the free variable  $a$  as if it was an element. To reconstruct the formal definition,  $P$  is split into true  $\mathbf{Set}$ -predicates  $P_n : A_n \rightarrow \mathbb{B}$  and  $P_{\top} : A_{\top} \rightarrow \mathbb{B}$  by subscripting every occurrence of a  $\mathcal{R}$ -object or morphism in  $P$  with the appropriate  $\mathbb{N}_{\top}$  object  $n \in \mathbb{N}$  or  $\top$ . Then, the formal definition of  $f : A \rightarrow_{\mathcal{R}} \Omega$  becomes:

$$f_n(a \in A_n) \triangleq P_n(a)$$

$$f_{\top}(a \in A_{\top}) \triangleq \begin{cases} \text{inr} * & \text{if } P_{\top}(a) \\ \text{inl } \{ n \in \mathbb{N} \mid P_n(\pi_n^A(a)) \} & \text{otherwise} \end{cases}$$

Another advantage of the shorthand is that the coherence condition  $f_n \circ \pi_n^A = \omega_n \circ f_{\top}$  simplifies to showing  $P_{\top}(a) \implies P_n(\pi_n^A(a))$  for all  $a \in A_{\top}$ . To establish  $f_n(\pi_n^A(a)) = \omega_n(f_{\top}(a))$ , we case-analyse on the possible output of  $f_{\top}(a)$ , which amounts to case-splitting on  $P_{\top}(a)$ . If  $P_{\top}(a)$  holds,  $\omega_n(f_{\top}(a))$  reduces to  $\omega_n(\text{inr} *) = 1$ , while the LHS becomes  $f_n(\pi_n^A(a)) = P_n(\pi_n^A(a))$  – this is our proof obligation, with the previous assumption  $P_{\top}(a)$ . On the other hand, if  $P_{\top}(a)$  doesn't hold,  $\omega_n(f_{\top}(a)) = \omega_n(\text{inl } \{ k \in \mathbb{N} \mid P_k(\pi_k^A(a)) \}) = P_n(\pi_n^A(a))$ , which is precisely the LHS  $f_n(\pi_n^A(a)) = P_n(\pi_n^A(a))$ .

For instance,  $\chi_S : A \rightarrow_{\mathcal{R}} \Omega$  can simply be defined as

$$\chi_S(a : A) = a \in S$$

with  $P(a) = a \in S$ , from which we get  $P_n(a : A_n) = a \in S_n$  and  $P_{\top}(a : A_{\top}) = a \in S_{\top}$  that directly gives us the full definition above. To establish the coherence condition  $(\chi_S)_n \circ \pi_n^A = \omega_n \circ (\chi_S)_{\top}$ , it is sufficient to prove that for all  $a \in S_{\top}$ ,  $\pi_n^A(a) \in S_n$ , which follows from the coherence of the monomorphism  $m : S \hookrightarrow A$  that embeds  $S$  into  $A$ .

As a further simplification, we will sometimes define  $\mathcal{R}$ -predicates via set comprehension:

$$f \triangleq \{ a \mid P(a) \}$$

This is especially useful when defining multivariable relations, avoiding the need for equality constraints on arguments. For instance, instead of defining the identity relation as

$$\text{id}_A(a, a') \triangleq a = a'$$

we simply write

$$\text{id}_A \triangleq \{ (a, a) \mid a \in A \}$$

These shorthand notations save a lot of writing and make the conceptual idea behind the definitions a lot clearer, since they are not obscured by the details of our particular topos. However, none of the shorthands will only be used if the transformation into the rigorous definition is ambiguous or not a direct application of the approach above.

## 4 The Category of Internal Relations

### 4.1 Internal Relations in $\mathcal{R}$

Internal relations generalise set-theoretic relations (binary predicates) in an arbitrary topos.

**Definition 4.1** (Internal relations in  $\mathcal{R}$ ). Given two objects  $A, B \in \mathcal{R}$ , an *internal relation* on  $A$  and  $B$  is defined as a subobject of the product  $A \times B$ . This is equivalently a map  $r : A \times B \rightarrow_{\mathcal{R}} \Omega$ .

Hence, relations on  $A$  and  $B$  form a set denoted  $\text{Rel}_{\mathcal{R}}(A, B) = \mathcal{R}(A \times B, \Omega)$ .

$$\begin{array}{ccc}
 (A \times B)_{\top} & \xrightarrow{r_{\top}} & \mathcal{P} + \mathbb{1} \\
 \downarrow \pi_0^{(A \times B)} & & \uparrow \omega_0 \\
 A_0 \times B_0 & \xrightarrow{r_0} & \mathbb{B} \\
 \downarrow \pi_1^{(A \times B)} & & \uparrow \omega_1 \\
 A_1 \times B_1 & \xrightarrow{r_1} & \mathbb{B} \\
 \vdots & & \vdots \\
 \downarrow \pi_k^{(A \times B)} & & \uparrow \omega_k \\
 A_k \times B_k & \xrightarrow{r_k} & \mathbb{B}
 \end{array}$$

All internal relations  $r: A \rightarrow_{\mathcal{R}} B$  must satisfy the coherence condition, which simplifies to:

$$r_n \circ (\pi_n^A \otimes \pi_n^B) = \omega_n \circ r_{\top}$$

or, for  $a \in A_{\top}, b \in B_{\top}$ ,

$$r_n(\pi_n^A(a), \pi_n^B(b)) = \omega_n(r_{\top}(a, b))$$

If  $r$  is defined in terms of a two-place predicate  $R$  using the shorthand described above, the sufficient condition is  $R_{\top}(a, b) \implies R_n(\pi_n^A(a), \pi_n^B(b))$ .

**Definition 4.2** (Identity relation). Given an object  $A \in \mathcal{R}$ , we define the identity relation as

$$\text{id}_A \triangleq \{(a, a) \mid a \in A\} \in \text{Rel}_{\mathcal{R}}(A, A)$$

As explained above, this shorthand notation “desugars” to

$$\begin{aligned}
 \text{id}_{A,n}(a, a') &\triangleq a = a' \\
 \text{id}_{A,\top}(a, a') &\triangleq \begin{cases} \text{inr} * & \text{if } a = a' \\ \text{inl} \{ n \in \mathbb{N} \mid \pi_n^A(a) = \pi_n^A(a') \} & \text{otherwise} \end{cases}
 \end{aligned}$$

At any time index, the identity relation is the diagonal. At the infinity point, the identity is the right injection for elements equal at the limit, or the set of indices where the projections match. The sufficient condition for coherence is  $a = a' \implies \pi_n^A(a) = \pi_n^A(a')$  for  $a, a' \in A_{\top}$ , which clearly holds.

**Definition 4.3** (Composition of relations). Given two relations  $r \in \text{Rel}_{\mathcal{R}}(A, B)$  and  $s \in \text{Rel}_{\mathcal{R}}(B, C)$ , we define their composition  $s \circ r \in \text{Rel}_{\mathcal{R}}(A, C)$  as:

$$(s \circ r)(a, c) \triangleq \exists b \in B. r(a, b) \wedge s(b, c)$$

Again, this formally desugars into

$$\begin{aligned}
 (s \circ r)_n(a, c) &\triangleq \exists b \in B_n. r_n(a, b) \wedge s_n(b, c) \\
 (s \circ r)_{\top}(a, c) &\triangleq \begin{cases} \text{inr} * & \text{if } \exists b \in B_{\top}. r_{\top}(a, b) = \text{inr}(*) \wedge s_{\top}(b, c) = \text{inr}(*) \\ \text{inl} \{ n \in \mathbb{N} \mid \exists b \in B_{\top}. r_n(\pi_n^A(a), \pi_n^B(b)) \wedge s_n(\pi_n^B(b), \pi_n^C(c)) \} & \text{otherwise} \end{cases}
 \end{aligned}$$

At each step, the composition is the regular composition of relations (so, for  $n \in \mathbb{N}$ ,  $(s \circ r)_n = s_n \circ_{\text{Rel}} r_n$ , where  $\circ_{\text{Rel}}$  is the standard composition of relations on sets), and at the top point, the composition is “related at the limit” if there exists a  $b$  such that both  $(a, b)$  and  $(b, c)$  are “related at the limit”. Otherwise we give the set of natural numbers defining “when” there exists a  $b$  such that  $(a, b)$  and  $(b, c)$  are related. The sufficient condition for coherence is

$$\exists b \in B_{\top}. r_{\top}(a, b) = \text{inr}(\ast) \wedge s_{\top}(b, c) = \text{inr}(\ast) \implies \exists b \in B_{\top}. r_n(\pi_n^A(a), \pi_n^B(b)) \wedge s_n(\pi_n^B(b), \pi_n^C(c))$$

for  $a \in A_{\top}$  and  $c \in C_{\top}$ . Since by coherence  $r_n(\pi_n^A(a), \pi_n^B(b)) = \omega_n(r_{\top}(a, b)) = \omega_n(\text{inr}(\ast)) = 1$ , and similarly for  $s$ , the conjunction holds.

Associativity of composition follows from the associativity of conjunction in its definition. The unit laws for identity and composition follow from the coherence of  $\mathcal{R}$  morphisms.

We are now ready to define the category  $\text{Rel}_{\mathcal{R}}$  of internal relations on  $\mathcal{R}$ .

**Definition 4.4.** The objects of  $\text{Rel}_{\mathcal{R}}$  are the objects of  $\mathcal{R}$ , the arrows  $\text{Rel}_{\mathcal{R}}(A, B)$  are the internal relations  $\mathcal{R}(A \times B, \Omega)$ . We will denote a relation  $r \in \text{Rel}_{\mathcal{R}}(A, B)$  as  $r: A \rightarrow_{\mathcal{R}} B$ . The identity arrow is the identity relation, and composition is given by relation composition, both defined above.

## 4.2 Symmetric monoidal closed structure

To be a model of linear logic and type theory, our category  $\text{Rel}_{\mathcal{R}}$  must be symmetric monoidal closed. Below we list the operations and laws needed to make  $\text{Rel}_{\mathcal{R}}$  a symmetric monoidal closed category. In our relational setting, all these structural operations (associators, unitors, braiding) are simply equalities between arguments – correspondingly, the laws and identities simply reduce to equalities of the arguments, or projections of the arguments (in the  $\top$  case).

The only lemma which we need to use in the  $\text{inl}$  case for the definition of infinity points is the commutativity condition  $\pi_n^{\Omega} \circ f_{\top} = f_k \circ \pi_k^{A \times B}$ , which results in a conjunction of equalities on the projections of arguments.

**Underlying category** We demonstrated above that  $\text{Rel}_{\mathcal{R}}$  is a category and will be used as the basis of our model.

**Tensor product** We define the tensor product

$$\otimes: \text{Rel}_{\mathcal{R}} \times \text{Rel}_{\mathcal{R}} \rightarrow \text{Rel}_{\mathcal{R}}$$

as the Cartesian product of two  $\mathcal{R}$ -objects (i.e. pointwise product of the indexed sets):

$$A \otimes B \triangleq A \times_{\mathcal{R}} B$$

The projections  $\pi_n^{A \otimes B}: (A \otimes B)_{\top} \rightarrow (A \otimes B)_n$  are the **Set**-pairing of the individual projection maps  $\langle \pi_n^A, \pi_n^B \rangle$ .

Given two relations  $r: A \rightarrow_{\mathcal{R}} B$  and  $r': A' \rightarrow_{\mathcal{R}} B'$ , we form their monoidal product (the functorial action of the bifunctor  $\otimes$ )  $r \otimes r': A \otimes A' \rightarrow_{\mathcal{R}} B \otimes B'$  as:

$$(r \otimes r')((a, a'), (b, b')) \triangleq r(a, b) \wedge r'(a', b')$$

The coherence condition again follows from the coherence of  $r$  and  $r'$ .

**Unit object** The unit  $\mathbf{I} \in \mathbf{Rel}_{\mathcal{R}}$  of our category is the CCC unit of  $\mathcal{R}$ , namely the pointwise constant singleton set  $\mathbb{I}_k \triangleq \mathbb{I} = \{*\}$ .

**Left unitor** The natural isomorphism  $\lambda_A: \mathbf{I} \otimes A \rightarrow_{\mathcal{R}} A$  defined as

$$\lambda_A \triangleq \{((*, a), a) \mid a \in A\}$$

with the inverse  $\lambda_A^{-1}$  being equal to the opposite relation of  $\lambda_A$ . The coherence condition follows by equality. The naturality condition is for all  $r: A \rightarrow B$ ,  $r \circ \lambda_A = \lambda_B \circ (\text{id}_{\mathbf{I}} \otimes r)$ , which holds by definition.

**Right unitor** The natural isomorphism  $\rho_A: A \otimes \mathbf{I} \rightarrow_{\mathcal{R}} A$  defined as

$$\rho_A \triangleq \{((a, *), a) \mid a \in A\}$$

with the inverse  $\rho_A^{-1}$  being equal to the opposite relation of  $\rho_A$ . The coherence condition follows by equality. The naturality condition is for all  $r: A \rightarrow B$ ,  $r \circ \rho_A = \rho_B \circ (r \otimes \text{id}_{\mathbf{I}})$ , which holds by definition.

**Associator** The natural isomorphism  $\alpha_{A,B,C}: (A \otimes B) \otimes C \rightarrow_{\mathcal{R}} A \otimes (B \otimes C)$  defined as

$$\alpha_{A,B,C} \triangleq \{(((a, b), c), (a, (b, c))) \mid a \in A, b \in B, c \in C\}$$

with the inverse  $\alpha_{A,B,C}^{-1}$  being equal to the opposite relation of  $\alpha_{A,B,C}$ . The coherence condition follows by equality. All three naturality conditions follow definitionally.

**Braiding** The natural isomorphism  $\sigma_{A,B}: A \otimes B \rightarrow_{\mathcal{R}} B \otimes A$  defined as

$$\sigma_{A,B} \triangleq \{((a, b), (b, a)) \mid a \in A, b \in B\}$$

with the inverse  $\sigma_{A,B}^{-1}$  being equal to the opposite relation of  $\sigma_{A,B}$ . The coherence condition follows by equality. Both naturality conditions follow definitionally.

**Exponential** As is common with relational models of linear logic, the exponential  $\multimap: \mathbf{Rel}_{\mathcal{R}} \times \mathbf{Rel}_{\mathcal{R}} \rightarrow \mathbf{Rel}_{\mathcal{R}}$  is also defined as the monoidal product:

$$A \multimap B \triangleq A \otimes B$$

The evaluation map  $\text{eval}_{A,B}: (A \multimap B) \otimes A \rightarrow_{\mathcal{R}} B$  involves no actual evaluation, as the “output” is already available in the second part of the tuple:

$$\text{eval}_{A,B} \triangleq \{(((a, b), a), b) \mid a \in A, b \in B\}$$

For a relation  $r: (A \otimes B) \rightarrow_{\mathcal{R}} C$ , the exponential transpose  $\text{curry}(r): A \rightarrow_{\mathcal{R}} (B \multimap C)$  is:

$$\text{curry}(r)(a, (b, c)) \triangleq r((a, b), c)$$

As before, the coherence conditions for these morphisms follow by equality and coherence of  $r$ . To establish this as the internal hom of the category, we need to prove that for all  $B \in \mathbf{Rel}_{\mathcal{R}}$ , we have the adjunction  $- \otimes B \dashv B \multimap -$ ; that is, there is a natural isomorphism

$$\mathbf{Rel}_{\mathcal{R}}(A \otimes B, C) \cong \mathbf{Rel}_{\mathcal{R}}(A, B \multimap C)$$

for all  $A, B, C \in \mathbf{Rel}_{\mathcal{R}}$ . Since  $B \multimap C = B \otimes C$ , this is simply the associativity of the tensor product, exhibited by the natural isomorphism  $\alpha$ .

All the above categorical structure needs to satisfy additional coherence laws: triangle, pentagon, and hexagon identities. As all the definitions are just equality constraints on tuple components, the laws hold by the appropriate properties of logical conjunction (associativity, commutativity, etc.), as well as the coherence conditions of  $\mathcal{R}$ -morphisms. Below we list these conditions for completeness:

#### Triangle identity

$$(\text{id}_A \otimes \lambda_B) \circ \alpha_{A, \mathbf{l}, B} = \rho_A \circ \text{id}_B \quad : (A \otimes \mathbf{l}) \otimes B \rightarrow_{\mathcal{R}} A \otimes B$$

#### Pentagon identity

$$(\text{id}_A \otimes \alpha_{B, C, D}) \circ \alpha_{A, B \otimes C, D} \circ (\alpha_{A, B, C} \circ \text{id}_D) = \alpha_{A, B, C \otimes D} \circ \alpha_{A \otimes B, C, D} \\ : ((A \otimes B) \otimes C) \otimes D \rightarrow_{\mathcal{R}} A \otimes (B \otimes (C \otimes D))$$

#### Hexagon identity

$$(\text{id}_B \circ \sigma_{A, C}) \circ \alpha_{B, A, C} \circ (\sigma_{A, B} \circ \text{id}_C) = \alpha_{B, C, A} \circ \sigma_{A, B \otimes C} \circ \alpha_{A, B, C} \\ : (A \otimes B) \otimes C \rightarrow B \otimes (C \otimes A)$$

#### Braiding identity

$$\sigma_{B, A} \circ \sigma_{A, B} = \text{id}_{A \otimes B}$$

## 5 Adjunction between Set and $\text{Rel}_{\mathcal{R}}$

In this section we define an adjunction between  $\text{Set}$  and  $\text{Rel}_{\mathcal{R}}$  as a composite of two adjunctions which we describe below.

$$\begin{array}{ccccc} \text{Set} & \xrightleftharpoons[\text{lim}]{\Delta} & \mathcal{R} & \xrightleftharpoons[P]{I} & \text{Rel}_{\mathcal{R}} \\ & \perp & & \perp & \end{array}$$

### 5.1 Adjunction between Set and $\mathcal{R}$

**Definition 5.1** (Constant presheaf).

$$\begin{aligned} \Delta : \text{Set} &\rightarrow \mathcal{R} \\ \Delta(X)_k &\triangleq X \quad \pi_k^{\Delta(X)} = \text{id}_X \\ \Delta(f : X \rightarrow Y)_k &\triangleq f \end{aligned}$$

The *constant presheaf*  $\Delta : \text{Set} \rightarrow \mathcal{R}$  is a functor that maps a set  $X \in \text{Set}$  to an  $\mathcal{R}$ -object that is  $X$  at every step, with the identity function as the projections. A function  $f : X \rightarrow Y$  is mapped to the coherent  $\mathcal{R}$ -morphism



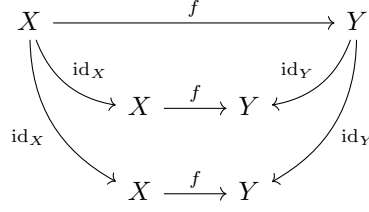

**Definition 5.2** (Limit functor).

$$\lim: \mathcal{R} \rightarrow \mathbf{Set}$$

$$\lim(A) \triangleq A_{\top}$$

$$\lim(f: A \rightarrow_{\mathcal{R}} B) \triangleq f_{\top}$$

The *limit functor*  $\lim: \mathcal{R} \rightarrow \mathbf{Set}$  maps a presheaf to a set by evaluation at the top point.

If we consider an object  $A \in \mathcal{R} = \mathbf{Set}^{\mathbb{N}_{\top}^{\text{op}}}$  as  $\mathbf{Set}$ -valued diagram of shape  $\mathbb{N}_{\top}^{\text{op}}$  (i.e. a functor  $A: \mathbb{N}_{\top}^{\text{op}} \rightarrow \mathbf{Set}$ ), the functor defined above is precisely the categorical limit construction

$$\lim: \mathbf{Set}^{\mathbb{N}_{\top}^{\text{op}}} \rightarrow \mathbf{Set}$$

**Proposition 5.3.** The limit functor  $\lim: \mathcal{R} \rightarrow \mathbf{Set}$  defined above assigns, to each  $A \in \mathcal{R} = \mathbf{Set}^{\mathbb{N}_{\top}^{\text{op}}}$ , the categorical limit  $A_{\top}$  of the  $\mathbf{Set}$ -valued diagram  $A$  of shape  $\mathbb{N}_{\top}^{\text{op}}$ .

*Proof.* This can be easily established by considering the universal property of limits: given a diagram  $A \in \mathcal{R}$ , the infinity point  $A_{\top}$  and projection morphisms  $\pi_n^A$  form the terminal cone (the limit) if for any other object  $L$  and projection morphisms  $\pi_n^L$  there is a unique mediator morphism  $u: L \rightarrow A_{\top}$  which commutes with all projection morphisms. However, by the construction of  $\mathcal{R}$ , the only possible candidate cone is  $A_{\top}$  itself, with the identity  $\text{id}_{A_{\top}}$  as the unique mediator, since there are no other morphisms with the codomain  $A_{\top}$ .

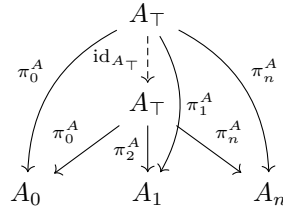

□

The adjunction between  $\Delta \dashv \lim$  is an instance of the standard adjunction construction between the generic diagonal functor  $\Delta_{\mathbb{N}_{\top}^{\text{op}}}: \mathbf{Set} \rightarrow \mathbf{Set}^{\mathbb{N}_{\top}^{\text{op}}}$  and the limit  $\lim: \mathbf{Set}^{\mathbb{N}_{\top}^{\text{op}}} \rightarrow \mathbf{Set}$ .

**Lemma 5.4.** We have an adjunction between  $\mathbf{Set}$  and  $\mathcal{R}$  formed by the functors  $\Delta$  and  $\lim$ .

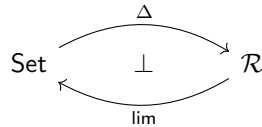

*Proof.* We prove that there is a natural isomorphism

$$\mathcal{R}(\Delta(X), B) \cong \mathbf{Set}(X, \lim(B))$$

Since  $\lim(B) \cong B_\top$ , it is enough to show  $\mathbf{Hom}_{\mathcal{R}}(\Delta(X), B) \cong \mathbf{Hom}_{\mathbf{Set}}(X, B_\top)$ . Going from left to right, assume we have a map  $f: \Delta(X) \rightarrow B \in \mathcal{R}$ . We know from  $\mathcal{R}$ -coherence that

$$\forall n \in \mathbb{N}, f_n \circ \pi_n^{\Delta(X)} = \pi_n^B \circ f_\top,$$

but since  $\pi_n^{\Delta(X)} = \text{id}_X$  it follows that

$$\forall n \in \mathbb{N}, f_n = \pi_n^B \circ f_\top,$$

i.e.  $f$  is fully specified by the map  $f_\top \in \mathbf{Set}(X, B_\top)$ . Thus we can define the isomorphism  $\phi$  as

$$\begin{aligned} \phi_{X,B}(f: \Delta X \rightarrow_{\mathcal{R}} B)_k &= f_\top & : X \rightarrow B_\top \in \mathbf{Set} \\ \phi_{X,B}^{-1}(g: X \rightarrow B_\top)_k &= \pi_k^B \circ g & : \Delta(X) \rightarrow B \in \mathcal{R} \end{aligned}$$

Naturality follows from the definition of the adjoint functors and  $\phi$ . □

## 5.2 Adjunction between $\mathcal{R}$ and $\mathbf{Rel}_{\mathcal{R}}$

The adjunction between  $\mathcal{R}$  and  $\mathbf{Rel}_{\mathcal{R}}$  is an analogue of the adjunction between  $\mathbf{Set}$  and  $\mathbf{Rel}$  stemming from the isomorphism  $\mathbf{Rel}(X, Y) \cong \mathbf{Set}(X, \mathcal{P}(Y))$ , i.e. that every  $\mathbf{Set}$ -relation  $R: X \rightarrow Y$  can be transformed into a function  $X \rightarrow \mathcal{P}(Y)$ . The adjoint functors in play are the inclusion  $\mathbf{Set} \rightarrow \mathbf{Rel}$  (that maps a function to its graph), and the relational image functor  $\mathbf{Rel} \rightarrow \mathbf{Set}$  (that maps a relation  $R: X \rightarrow Y$  to its relational direct image  $\vec{R}: \mathcal{P}(X) \rightarrow \mathcal{P}(Y)$ ). We can adapt this same construction to our time-indexed setting.

**Definition 5.5** (Inclusion functor).

$$\begin{aligned} I: \mathcal{R} &\rightarrow \mathbf{Rel}_{\mathcal{R}} \\ I(A) &\triangleq A \\ I(f: A \rightarrow_{\mathcal{R}} B)(a, b) &\triangleq f(a) = b \end{aligned}$$

The *inclusion functor*  $I: \mathcal{R} \rightarrow \mathbf{Rel}_{\mathcal{R}}$  is defined to be the identity on objects and maps morphisms  $f: A \rightarrow_{\mathcal{R}} B$  to their underlying internal graph relation  $A \times B \rightarrow_{\mathcal{R}} \Omega$ . As usual, the shorthand for the relation definition desugars into

$$\begin{aligned} I(f: A \rightarrow_{\mathcal{R}} B)_n(a, b) &\triangleq f_n(a) = b \\ I(f: A \rightarrow_{\mathcal{R}} B)_\top(a, b) &\triangleq \begin{cases} \text{inr } * & \text{if } f_\top(a) = b \\ \text{inl } \{ n \in \mathbb{N} \mid f_n(\pi_n^A(a)) = \pi_n^B(b) \} & \text{otherwise} \end{cases} \end{aligned}$$

At the top point, “truth” is represented by  $\text{inr}(*)$  while “falsity” is the set of time indices where the relation holds.

**Definition 5.6** (Relational image functor).

$$\begin{aligned}
P &: \mathbf{Rel}_{\mathcal{R}} \rightarrow \mathcal{R} \\
P(A) &\triangleq \mathbf{P}(A) \\
P(r: A \leftrightarrow_{\mathcal{R}} B)_n(\chi_S: A_n \rightarrow \mathbb{B}) &\triangleq \{ b \in B_n \mid \exists a \in A_n. \chi_S(a) \wedge r_n(a, b) \} \\
P(r: A \leftrightarrow_{\mathcal{R}} B)_{\top}(s: A \rightarrow_{\mathcal{R}} \Omega) &\triangleq \{ b \in B \mid \exists a \in A. s(a) \wedge r(a, b) \}
\end{aligned}$$

The *power object functor*  $P: \mathbf{Rel}_{\mathcal{R}} \rightarrow \mathcal{R}$  is analogous to the covariant powerset functor from relations to sets, which is what the (simplified) definition above intends to capture. Indeed, at individual projections,  $P(r)_n$  is precisely the direct relational image functor  $\vec{r}_n^{\rightarrow}$  on (characteristic functions of) subsets of  $A_n$ . At the top point the overall shape of the function is similar, except instead of a characteristic function  $\chi_S: A_n \rightarrow \mathbb{B}$  of a subset  $S$ , we get the characteristic morphism  $s: A \rightarrow_{\mathcal{R}} \Omega$  for a subobject of  $A \in \mathcal{R}$ . Of course, due to the structure of  $\Omega \in \mathcal{R}$ , the full, desugared definition is more complicated:

$$\begin{aligned}
P(r: A \leftrightarrow_{\mathcal{R}} B)_{\top}(s: A \rightarrow_{\mathcal{R}} \Omega)_n(b: B_n) &\triangleq \exists a \in A_n. r_n(a, b) \wedge s_n(a) \\
P(r: A \leftrightarrow_{\mathcal{R}} B)_{\top}(s: A \rightarrow_{\mathcal{R}} \Omega)_{\top}(b: B_{\top}) &= \\
&\begin{cases} \text{inr } * & \text{if } \exists a \in A_{\top}. s_{\top}(a) = \text{inr}(*) \wedge r_{\top}(a, b) = \text{inr}(*) \\ \text{inl } \{ n \in \mathbb{N} \mid \exists a \in A_{\top}. s_n(\pi_n^A(a)) \wedge r_n(\pi_n^A(a), \pi_n^B(b)) \} & \text{otherwise} \end{cases}
\end{aligned}$$

The similar structure comes from the definition of power objects in  $\mathbf{P}(A) \in \mathcal{R}$ : the projections are powersets  $\mathcal{P}(A_n) \cong \mathbf{Set}(A_n, \mathbb{B})$ , while at the top point, it is the space of characteristic maps  $\mathcal{R}(A, \Omega)$ . However, to return  $\mathbf{P}(B)_{\top}$ , we need to define a  $\mathcal{R}$ -predicate at the top point and time steps, hence the additional branching on the index. In the latter case, we are defining a subset of  $B_n$  given  $s_n: A_n \rightarrow \Omega_n = A_n \rightarrow \mathbb{B}$  which represents a subset of  $A_n$ , so the definition is analogous to a direct image. In the latter case, we adapt our predicate to return values of  $\mathcal{P}(\mathbb{N}) + \mathbb{1}$  in the usual way, requiring it to hold at the top point or selecting the time steps when it holds in the projections.

**Lemma 5.7.** We have an adjunction between  $\mathcal{R}$  and  $\mathbf{Rel}_{\mathcal{R}}$  formed by the functors  $I$  and  $P$ .

$$\begin{array}{ccc}
& I & \\
\mathcal{R} & \xrightarrow{\quad} & \mathbf{Rel}_{\mathcal{R}} \\
& \perp & \\
& \xleftarrow{\quad} & \\
& P &
\end{array}$$

*Proof.* To prove this we can either establish the isomorphism

$$\mathbf{Rel}_{\mathcal{R}}(I(A), B) \cong \mathcal{R}(A, P(B))$$

or provide the natural transformations  $\eta: \text{Id}_{\mathcal{R}} \Rightarrow PI$  and  $\epsilon: IP \Rightarrow \text{Id}_{\mathbf{Rel}_{\mathcal{R}}}$ .

$$\begin{aligned}
\eta_A &: A \rightarrow_{\mathcal{R}} P(I(A)) \\
\eta_{A,n}(a: A_n) &\triangleq \{ a \} \\
\eta_{A,\top}(a)(a') &\triangleq a = a'
\end{aligned}$$

The unit of the adjunction maps  $A$  to its power object. Each case is the appropriate version of a “singleton set” construction: at the projections  $a$  maps to  $\{a\}$ , at the top point (where  $(P(A))_{\top} = \mathcal{R}(A, \Omega)$ ) we either return the singleton set of the projection of  $a$ , or the analogous construction for subobjects  $A_{\top} \rightarrow \mathcal{P}(\mathbb{N}) + 1$ .

$$\begin{aligned}\epsilon_A &: I(P(A)) \rightarrow_{\mathcal{R}} A \\ \epsilon_A(s, a) &= s(a)\end{aligned}$$

The counit represents the  $\ni$  relation between a subset of  $A$  and an element of  $A$ . At the projections, we ask whether the element is in the subset  $S \subseteq A_n$  (represented by the characteristic function  $s_n: A_n \rightarrow \mathbb{B}$ ), while at the top point we use the characteristic morphism  $s_{\top}: A_{\top} \rightarrow_{\mathcal{R}} \mathcal{P}(\mathbb{N}) + 1$  on the second element  $a: A_{\top}$ .

Both the unit and the counit derive from the homset-isomorphism and therefore satisfy naturality and the adjunction laws. Thus, we have the adjunction  $I \dashv P$ , as required.  $\square$

We are now ready to state the main result of the section. The required theorem is a standard result about composites of adjoint functors applied to  $\Delta \dashv \lim$  and  $I \dashv P$ .

**Theorem 5.8.** The composites  $F = I \circ \Delta$  and  $G = \lim \circ P$  form a pair of adjoint functors for the adjunction  $F \dashv G = (I \circ \Delta) \dashv (\lim \circ P)$  between  $\mathbf{Set}$  and  $\mathbf{Rel}_{\mathcal{R}}$ .

*Proof.* This follows from a standard result about composites of adjoint functors: if  $L \dashv R$  and  $L' \dashv R'$ , then  $L' \circ L \dashv G \circ R'$ . In our concrete case, the adjunction also gives rise to the following natural transformations:

$$\begin{aligned}\eta_X: X &\rightarrow GFX = & \epsilon_A: FGA &\rightarrow_{\mathcal{R}} A = \\ \eta_X: X &\rightarrow \lim(P(I(\Delta X))) = & \epsilon_A: I(\Delta(\lim(PA))) &\rightarrow_{\mathcal{R}} A = \\ &X \rightarrow \mathcal{R}(\Delta X, \Omega) & I(\Delta(\mathcal{R}(A, \Omega))) &\rightarrow_{\mathcal{R}} A \\ \eta_X(x \in X)_n(x' \in X) &\triangleq x = x' & \epsilon_{A,k}(s: A \rightarrow \Omega, a: A_k) &\triangleq s_k(a) \\ \eta_X(x \in X)_{\top}(x' \in X) &\triangleq \begin{cases} \text{inr } * & \text{if } x = x' \\ \text{inl } \emptyset & \text{otherwise} \end{cases}\end{aligned}$$

The unit is similar to a curried version of the equality predicate, mapping two inputs to  $x = x'$  in the projections and  $\text{inr } *$  or  $\text{inl } \emptyset$  at the top point, depending on whether the equality holds or not. Given that the two inputs come from sets, they stay temporally constant so the set of timesteps where  $\pi_n^{\Delta X}(x) = \pi_n^{\Delta X}(x')$  holds will be necessarily empty if  $x \neq x'$ . The counit again represents the inverse element relation  $\ni$  using the characteristic morphism of a subobject of  $A$  with an element at an arbitrary timestep.  $\square$

## 6 Temporal operations

Our reactive category  $\mathcal{R}$  admits several temporal operations that can be lifted to  $\mathbf{Rel}_{\mathcal{R}}$ .

## 6.1 Shifting

First, we need a family of helper functions  $\text{shift}^k: \mathcal{P}(\mathbb{N}) \rightarrow \mathcal{P}(\mathbb{N})$  for all  $k \in \mathbb{N}$  that shift the elements of a set of natural numbers by some value, adding all values below  $k$  to the set.

$$\text{shift}^k(N) \triangleq [k] \cup \{n + k \mid n \in N\}$$

Here,  $[k]$  denotes the finite set  $\{0, 1, \dots, k-1\}$  of size  $k$  (in particular,  $[0] = \emptyset$ , so  $\text{shift}^0 = \text{id}_{\mathcal{P}(\mathbb{N})}$ ). We will simply write  $\text{shift}$  for  $\text{shift}^1$ . For example, we have:

$$\text{shift}(\{2, 3, 5, 7\}) = \{0, 3, 4, 6, 8\} \quad \text{shift}^3(\{0, 1, 2\}) = \{0, 1, 2, 3, 4, 5\} \quad \text{shift}^k(\emptyset) = [k]$$

We will make use of the following properties, which follow directly from the definition:

**Lemma 6.1.** For  $n, k \in \mathbb{N}$  and a set  $N \subseteq \mathbb{N}$ , we have the following:

$$[k] \subseteq \text{shift}^k(N) \quad n + k \in \text{shift}^k(N) \iff n \in N$$

The following corollary takes care of all the projections smaller than the shift.

**Corollary 6.2.** If  $k < l$ , we have:

$$\omega_k \circ (\text{shift}^l + \text{id}_1) = \text{const}(1)$$

*Proof.* In the  $\text{inr}(\ast)$  case,  $\omega_k(\text{inr}(\ast))$  holds. In the  $\text{inl}(N)$  case for  $N \subseteq \mathbb{N}$ , we have:

$$\omega_k(\text{inl}(\text{shift}^l(N))) = k \in \text{shift}^l(N) \iff k \in [l]$$

where the bi-implication holds from the property  $[l] \subseteq \text{shift}^l(N)$ . If  $k < l$ ,  $k$  will certainly be an element of  $[l]$ . Note that we need  $l$  to be strictly greater than  $k$ , since  $k \notin [k] = \{0, 1, \dots, k-1\}$ .  $\square$

## 6.2 Delays

A single object in  $\mathcal{R}$  represents a collection of time-indexed sets with a top element. By shifting the indices, we can model delaying the stream of data associated with the object by some number of time steps.

**Definition 6.3** (Later modality). The *later modality*  $\triangleright: \text{Rel}_{\mathcal{R}} \rightarrow \text{Rel}_{\mathcal{R}}$  is an endofunctor that represents a one-step delay of the object. On objects  $A \in \text{Rel}_{\mathcal{R}}$  and arrows  $r: A \rightarrow_{\mathcal{R}} B$ , it is defined as:

$$\begin{aligned} (\triangleright A)_0 &\triangleq \mathbb{1} & (\triangleright r)_0 &\triangleq \text{const}(1) \\ (\triangleright A)_{k+1} &\triangleq A_k & (\triangleright r)_{k+1} &\triangleq r_k \\ (\triangleright A)_{\top} &\triangleq A_{\top} & (\triangleright r)_{\top} &\triangleq (\text{shift} + \text{id}_1) \circ r_{\top} \end{aligned}$$

The projections  $\pi_k^{\triangleright A}: A_{\top} \rightarrow (\triangleright A)_k$  are:

$$\pi_0^{\triangleright A} \triangleq !_{A_{\top}}: A_{\top} \rightarrow \mathbb{1} \quad \pi_{k+1}^{\triangleright A} \triangleq \pi_k^A: A_{\top} \rightarrow A_k$$

The slightly unusual definition of  $(\triangleright r)_{\top}$  (which uses the shifting operation and the coproduct/disjoint union bifunctor  $+$ ) is required to ensure that transforming the top element takes the one-step delay into account. This is the only definition that satisfies the coherence condition for the functorial mapping:  $(\triangleright r)_n(\pi_n^{\triangleright A}(a), \pi_n^{\triangleright B}(b)) = \omega_n((\triangleright r)_{\top}(a, b))$ .

- For  $n = 0$ , the LHS reduces to  $1$ . The RHS is  $\omega_0((\triangleright r)_\top(a, b)) = \omega_0((\text{shift} + \text{id}_\perp)(r_\top(a, b)))$ . From Corollary 6.2 and  $1 > 0$ , this automatically holds.
- For  $n = k + 1$ , we have the following:

$$\begin{aligned}
(\triangleright r)_{k+1}(\pi_{k+1}^{\triangleright A}(a), \pi_{k+1}^{\triangleright B}(b)) &= r_k(\pi_k^{\triangleright A}(a), \pi_k^{\triangleright B}(b)) \\
&= \omega_k(r_\top(a, b)) && \text{(coherence of } r) \\
&= [k \in -, \text{true}](r_\top(a, b)) && \text{(equivalent def. of } \omega_k) \\
&= [k + 1 \in (\text{shift}^1(-)), \text{true}](r_\top(a, b)) && \text{(Lemma 6.1)} \\
&= [k + 1 \in -, \text{true}]((\text{shift} + \text{id}_\perp)(r_\top(a, b))) && \text{(coproduct property)} \\
&= \omega_{k+1}((\text{shift} + \text{id}_\perp)(r_\top(a, b))) \\
&= \omega_{k+1}((\triangleright r)_\top(a, b))
\end{aligned}$$

The functor laws are as follows:

### Identity

$$\begin{aligned}
(\triangleright \text{id}_A)_0(*, *) &= 1 = \text{id}_{\perp, 0}(*, *) = \text{id}_{\triangleright A, 0}(*, *) \\
(\triangleright \text{id}_A)_{k+1}(a, a') &= \text{id}_{A, k}(a, a') = \text{id}_{\triangleright A, k+1}(a, a') \\
(\triangleright \text{id}_A)_\top(a, a') &= (\text{shift} + \text{id}_\perp)(\text{id}_{A, \top}(a, a')) \\
&= \begin{cases} \text{inr}(*, *) = \text{id}_{\triangleright A, \top}(a, a') & \text{if } a = a' \\ \text{inl}\{n + 1 \mid \pi_n^A(a) = \pi_n^A(a')\} \\ \quad = \text{inl}(\{n + 1 \mid \pi_{n+1}^A(a) = \pi_{n+1}^A(a')\}) = \text{id}_{\triangleright A, \top}(a, a') & \text{otherwise} \end{cases}
\end{aligned}$$

### Composition

$$\begin{aligned}
(\triangleright (s \circ r))_0(*, *) &= 1 = (\triangleright s)_0(*, *) \wedge (\triangleright r)_0(*, *) = (\triangleright s \circ \triangleright r)_0(*, *) \\
(\triangleright (s \circ r))_{k+1} &= (s \circ r)_k = s_k \circ r_k = (\triangleright s)_{k+1} \circ (\triangleright r)_{k+1} = (\triangleright s \circ \triangleright r)_{k+1} \\
(\triangleright (s \circ r))_\top(a, c) &= (\text{shift} + \text{id}_\perp)((s \circ r)_\top(a, c)) \\
&= \begin{cases} \text{inr} * & \text{if } (s \circ r)_\top(a, c) = \text{inr}(*, *) \\ \text{inl} \{n \in \mathbb{N} \mid (s \circ r)_n(\pi_n^A(a), \pi_n^C(c))\} & \text{otherwise} \end{cases} \\
&= \begin{cases} \text{inr} * & \text{if } \exists b \in B_\top. r_\top(a, b) = \text{inr}(*, *) \wedge s_\top(b, c) = \text{inr}(*, *) \\ \text{inl} \{n + 1 \mid \exists b \in B_\top. r_n(\pi_n^A(a), \pi_n^B(b)) \wedge s_n(\pi_n^B(b), \pi_n^C(c))\} & \text{otherwise} \end{cases} \\
&= \begin{cases} \text{inr} * & \text{if } \exists b \in (\triangleright B)_\top. (\text{shift} + \text{id}_\perp)(r_\top(a, b)) = \text{inr}(*, *) \wedge (\text{shift} + \text{id}_\perp)(s_\top(b, c)) = \text{inr}(*, *) \\ \text{inl} \{n + 1 \mid \exists b \in B_\top. (\triangleright r)_{n+1}(\pi_{n+1}^A(a), \pi_{n+1}^B(b)) \wedge (\triangleright s)_{n+1}(\pi_{n+1}^B(b), \pi_{n+1}^C(c))\} & \text{otherwise} \end{cases} \\
&= \begin{cases} \text{inr} * & \text{if } \exists b \in (\triangleright B)_\top. (\triangleright r)_\top(a, b) \wedge (\triangleright s)_\top(b, c) \\ \text{inl} \{n \in \mathbb{N} \mid \exists b \in B_\top. (\triangleright r)_n(\pi_n^A(a), \pi_n^B(b)) \wedge (\triangleright s)_n(\pi_n^B(b), \pi_n^C(c))\} & \text{otherwise} \end{cases} \\
&= (\triangleright s \circ \triangleright r)_\top(a, c)
\end{aligned}$$

### 6.3 Iterated delays

**Definition 6.4.** For every  $n \in \mathbb{N}$ , we define the  $n$ -time delay functor  $\triangleright^n : \text{Rel}_{\mathcal{R}} \rightarrow \text{Rel}_{\mathcal{R}}$  as:

$$\begin{aligned} \triangleright^0 (A : \text{Rel}_{\mathcal{R}}) &\triangleq A & \triangleright^0 (r : A \rightarrow_{\mathcal{R}} B) &\triangleq r \\ \triangleright^{k+1} (A : \text{Rel}_{\mathcal{R}}) &\triangleq \triangleright(\triangleright^k A) & \triangleright^{k+1} (r : A \rightarrow_{\mathcal{R}} B) &\triangleq \triangleright(\triangleright^k r) \end{aligned}$$

The projections are:

$$\pi_k^{\triangleright^n A} = \begin{cases} !_{A_{\top}} & \text{if } k < n \\ \pi_{k-n}^A & \text{otherwise} \end{cases}$$

Since  $\triangleright^n$  is just an iterated application of  $\triangleright$ , the coherence and functoriality properties hold by induction. In addition, we have the equivalence  $(\triangleright^n r)_{\top} = (\text{shift}^n + \text{id}_{\mathbb{1}}) \circ r_{\top}$ , and the coherence condition therefore becomes

$$(\triangleright^n r)_k(\pi_k^{\triangleright^n A}(a), \pi_k^{\triangleright^n B}(b)) = \omega_k((\text{shift}^n + \text{id}_{\mathbb{1}})(r_{\top}(a, b)))$$

If  $k < n$ , we get the equality as a consequence of Corollary 6.2. Otherwise  $k = n + l$  for some  $l \in \mathbb{N}$ , and the LHS reduces to  $r_l(\pi_l^A(a), \pi_l^B(b)) = \omega_l(r_{\top}(a, b))$ , while the RHS (for the  $r_{\top}(a, b) = \text{inl}(N)$  case) is

$$n + l \in \text{shift}^n(N) \iff l \in N$$

which holds precisely when  $\omega_l(r_{\top}(a, b))$  does.

Iterated delays let us shift a sequence of values by a given number of steps. However, the top point is not affected by any delays, so for any  $A \in \text{Rel}_{\mathcal{R}}$  and  $k \in \mathbb{N}_{\top}$ ,  $A_{\top} = (\triangleright^n A)_{\top}$ . This property will implicitly be used in the definitions below. We also have the following important lemma, which says that extra delay can be cancelled out by extra waiting:

**Lemma 6.5** (Cancellation of delays). For any  $A \in \text{Rel}_{\mathcal{R}}$ , and  $n, k, l \in \mathbb{N}$ , we have:

$$(\triangleright^{k+l} A)_{n+l} = (\triangleright^k A)_n$$

*Proof.* By induction on  $k$ . □

A corollary of this lemma is that  $(\triangleright^k A)_n = \mathbb{1}$  for any  $k > n$ , so  $*$  :  $(\triangleright^k A)_n$  for any type  $A$  and indices  $n, k$  with  $k > n$ . Below we will use  $\triangleright^+$  to denote a delay iterated at least once; thus, the only inhabitant of  $(\triangleright^+ A)_0$  is  $*$ .

### 6.4 The event monad

The events in our syntax will be interpreted as a value with an unknown, arbitrary delay, represented by a dependent sum.

**Definition 6.6.** The *arbitrary delay* or *event* functor  $\diamond : \text{Rel}_{\mathcal{R}} \rightarrow \text{Rel}_{\mathcal{R}}$  is defined as:

$$\begin{aligned} \diamond : \text{Rel}_{\mathcal{R}} &\rightarrow \text{Rel}_{\mathcal{R}} \\ \diamond(A : \text{Rel}_{\mathcal{R}})_{\top} &\triangleq A_{\top} \\ \diamond(A : \text{Rel}_{\mathcal{R}})_n &\triangleq \sum_{k \in \mathbb{N}} (\triangleright^k A)_n \end{aligned}$$

$$\begin{aligned}\diamond(r : A \multimap_{\mathcal{R}} B)_{\top}(a : A_{\top}, b : B_{\top}) &\triangleq r_{\top}(a, b) \\ \diamond(r : A \multimap_{\mathcal{R}} b)_n &\triangleq \{ ((k, a : (\triangleright^k A)_n), (k, b : (\triangleright^k B)_n)) \mid (\triangleright^k r)_n(a, b) \}\end{aligned}$$

The projections  $\pi_n^{\diamond A} : A_{\top} \rightarrow (\diamond A)_n$  map  $a : A_{\top}$  to  $(0, \pi_n^A(a))$ : since  $\pi_n^A(a) : A_n$  and  $(\triangleright^0 A)_n = A_n$ , the pair is indeed of type  $\sum_{k \in \mathbb{N}} (\triangleright^k A)_n = (\diamond A)_n$ .

The coherence condition for the functorial map is  $(\diamond r)_n \circ (\pi_n^{\diamond A} \otimes \pi_n^{\diamond B}) = \omega_n \circ (\diamond r)_{\top}$ ; for  $a \in A_{\top}$  and  $b \in B_{\top}$ , we have:

$$\begin{aligned}(\diamond r)_n(\pi_n^{\diamond A}(a), \pi_n^{\diamond B}(b)) &= (\diamond r)_n((0, \pi_n^A(a)), (0, \pi_n^B(b))) \\ &= (\triangleright^0 r)_n(\pi_n^A(a), \pi_n^B(b)) \\ &= r_n(\pi_n^A(a), \pi_n^B(b)) \\ &= \omega_n(r_{\top}(a, b)) \\ &= \omega_n((\diamond r)_{\top}(a, b))\end{aligned}$$

The functoriality laws hold definitionally.

**Theorem 6.7.** The event endofunctor  $\diamond : \text{Rel}_{\mathcal{R}} \rightarrow \text{Rel}_{\mathcal{R}}$  is a monad with unit and multiplication:

$$\begin{aligned}\eta_A : A \multimap_{\mathcal{R}} \diamond A & & \mu_A : \diamond \diamond A \multimap_{\mathcal{R}} \diamond A \\ \eta_{A, \top} &\triangleq \text{id}_{A, \top} & \mu_{A, \top} &\triangleq \text{id}_{A, \top} \\ \eta_{A, n} &\triangleq \{ (a, (0, a)) \mid a \in A_n \} & \mu_{A, n} &\triangleq \{ ((k, (l, a)), (k + l, a)) \mid k \leq n, l \in \mathbb{N}, a \in (\triangleright^l A)_{n-k} \} \\ & & &\cup \{ ((k, * : (\triangleright^k \diamond A)_n), (k, * : (\triangleright^k A)_n)) \mid k > n \}\end{aligned}$$

*Proof.* The proof involves several steps: proving coherence, naturality, and the three monad laws.

**Coherence** We begin by showing that  $\eta$  and  $\mu$  are both valid  $\text{Rel}_{\mathcal{R}}$ -morphisms.

$$\eta_{A, n}(\pi_n^A(a), \pi_n^{\diamond A}(a')) = \omega_n(\eta_{A, \top}(a, a')) \quad \mu_{A, n}(\pi_n^{\diamond \diamond A}(a), \pi_n^{\diamond A}(a')) = \omega_n(\mu_{A, \top}(a, a'))$$

For the first one, we have

$$\eta_{A, n}(\pi_n^A(a), \pi_n^{\diamond A}(a')) = \eta_{A, n}(\pi_n^A(a), (0, \pi_n^A(a'))) \iff \pi_n^A(a) = \pi_n^A(a')$$

while the RHS reduces either to  $a = a'$  or  $\pi_n^A(a) = \pi_n^A(a')$ . Similarly, for the second one, we have

$$\mu_{A, n}(\pi_n^{\diamond \diamond A}(a), \pi_n^{\diamond A}(a')) = \mu_{A, n}((0, (0, \pi_n^A(a))), (0, \pi_n^A(a'))) \iff \pi_n^A(a) = \pi_n^A(a')$$

while the RHS reduces either to  $a = a'$  or  $\pi_n^A(a) = \pi_n^A(a')$ .

**Naturality** Next, we show that both  $\eta$  and  $\mu$  satisfy the naturality conditions: for a relation  $r : A \multimap_{\mathcal{R}} B$ , we have

$$\diamond r \circ \eta_A = \eta_B \circ r \quad \diamond r \circ \mu_A = \mu_B \circ \diamond \diamond r$$

Let  $r : A \multimap_{\mathcal{R}} B$  be a morphism in  $\text{Rel}_{\mathcal{R}}$ . At the top point both  $\eta$  and  $\mu$  are the identity, so naturality follows from the naturality of  $\text{id}$ . At a timestep  $n$ , we have:

$$(\diamond r \circ \eta_A)_n(a : A_n, (k, b : (\triangleright^k A)_n))$$



$$\begin{aligned}
&= (\diamond r)_n((0, a), (k, b)) \\
&= (\triangleright^k r)_n(a, b : (\triangleright^k B)_n) \wedge k = 0 \\
&= r_n(a, b) \wedge k = 0 \\
&= \exists b' : B_n \cdot r_n(a, b') \wedge k = 0 \wedge b' = b \\
&= \exists b' : B_n \cdot r_n(a, b') \wedge \eta_{B,n}(b', (k, b)) \\
&= (\eta_B \circ r)_n(a : A_n, (k, b : (\triangleright^k A)_n))
\end{aligned}$$

and

$$\begin{aligned}
&(\diamond r \circ \mu_A)_n((k, e_a : (\triangleright^k \diamond A)_n), (m, b : (\triangleright^m B)_n)) \\
&= \begin{cases} (\diamond r \circ \mu_A)_n((k, (l, a)), (m, b)) & \text{if } k \leq n \\ (\diamond r \circ \mu_A)_n((k, *), (m, b)) & \text{otherwise} \end{cases} \\
&= \begin{cases} \mu_{A,n}((k, (l, a)), (k + l, a)) \wedge (\diamond r)_n((k + l, a), (m, b)) & \text{if } k \leq n \\ \mu_{A,n}((k, *), (k, *)) \wedge (\diamond r)_n((k, *), (m, b)) & \text{otherwise} \end{cases} \\
&= \begin{cases} k + l = m \wedge (\triangleright^{k+l} r)_n(a, b) & \text{if } k \leq n \\ m = k \wedge b = * & \text{otherwise} \end{cases} \\
&= \begin{cases} (\diamond \diamond r)_n((k, (l, a)), (k, (l, b))) \wedge \mu_{B,n}((k, (l, b)), (m, b)) & \text{if } k \leq n \\ (\diamond \diamond r)_n((k, *), (k, *)) \wedge \mu_{B,n}((k, *), (m, b)) & \text{otherwise} \end{cases} \\
&= \begin{cases} (\mu_B \circ \diamond \diamond r)_n((k, (l, a)), (m, b)) & \text{if } k \leq n \\ (\mu_B \circ \diamond \diamond r)_n((k, *), (m, b)) & \text{otherwise} \end{cases} \\
&= (\mu_B \circ \diamond \diamond r)_n((k, e_a : (\triangleright^k \diamond A)_n), (m, b : (\triangleright^m B)_n))
\end{aligned}$$

**Monad laws** Next, we turn to the monad laws.

$$\mu \circ \eta \diamond = \text{id}_\diamond \quad \mu \circ \diamond \eta = \text{id}_\diamond \quad \mu \circ \mu \diamond = \mu \circ \diamond \mu$$

**Right unit** For an object  $A \in \text{Rel}_{\mathcal{R}}$ , the right unit law is:

$$\mu_A \circ \eta_{\diamond A} = \text{id}_{\diamond A} : \diamond A \rightarrow_{\mathcal{R}} \diamond A$$

At the top point, both  $\mu$  and  $\eta$  are the identity morphism so their composition is the identity. At a timestep  $n$ :

$$\begin{aligned}
&(\mu_A \circ \eta_{\diamond A})_n((k, a : (\triangleright^k A)_n), (l, a' : (\triangleright^l A)_n)) \\
&= \mu_{A,n}((0, (k, a)), (l, a')) \\
&= 0 + k = l \wedge a = a' \\
&= (k, a) = (l, a')
\end{aligned}$$

**Left unit** For an object  $A \in \text{Rel}_{\mathcal{R}}$ , the right unit law is:

$$\mu_A \circ \diamond \eta_A = \text{id}_{\diamond A} : \diamond A \rightarrow_{\mathcal{R}} \diamond A$$

At the top point, both  $\mu$  and  $\eta$  are the identity morphism so their composition is the identity. At a timestep  $n$ :

$$\begin{aligned}
& (\mu_A \circ \diamond \eta_A)_n((k, a : (\triangleright^k A)_n), (l, a' : (\triangleright^l A)_n)) \\
&= \begin{cases} (\mu_A \circ \diamond \eta_A)_n((k, a : A_{n-k}), (l, a' : (\triangleright^l A)_n)) & \text{if } k \leq n \\ (\mu_A \circ \diamond \eta_A)_n((k, *), (l, a' : (\triangleright^l A)_n)) & \text{otherwise} \end{cases} \\
&= \begin{cases} (\diamond \eta_A)_n((k, a), (k, (0, a))) \wedge \mu_{A,n}((k, (0, a)), (l, a')) & \text{if } k \leq n \\ (\diamond \eta_A)_n((k, *), (k, *)) \wedge \mu_{A,n}((k, *), (l, *)) & \text{otherwise} \end{cases} \\
&= \begin{cases} k = l \wedge a = a' & \text{if } k \leq n \\ k = l & \text{otherwise} \end{cases} \\
&= \begin{cases} (k, a) = (l, a') & \text{if } k \leq n \\ (k, *) = (l, *) & \text{otherwise} \end{cases} \\
&= \text{id}_{\diamond A, n}((k, a), (l, a'))
\end{aligned}$$

The last case of the proof relies on the fact that we want the delay of the right argument to be equal to  $k$ , not just an arbitrary value greater than  $n$  (which would still make the definition of  $\diamond_{A,n}^k$  typecheck).

**Associativity** For an object  $A \in \text{Rel}_{\mathcal{R}}$ , the right unit law is:

$$\mu_A \circ \mu_{\diamond A} = \mu_A \circ \diamond \mu_A : \diamond \diamond \diamond A \rightarrow_{\mathcal{R}} \diamond A$$

At the top point, both  $\mu$  and  $\eta$  are the identity morphism so their composition is the identity. In the projections the proof is as follows:

$$\begin{aligned}
& (\mu_A \circ \mu_{\diamond A})_n((k, e_{e_a} : (\triangleright^k \diamond \diamond A)_n), (m, a' : (\triangleright^l A)_n)) \\
&= \begin{cases} (\mu_A \circ \mu_{\diamond A})_n((k, (l, e_a : (\triangleright^l \diamond A)_{n-k})), (m, a' : (\triangleright^m A)_n)) & \text{if } k \leq n \\ (\mu_A \circ \mu_{\diamond A})_n((k, *), (m, a' : (\triangleright^m A)_n)) & \text{otherwise} \end{cases} \\
&= \begin{cases} \mu_{\diamond A, n}((k, (l, e_a)), (k + l, e_a)) \wedge \mu_{A, n}((k + l, e_a), (m, a')) & \text{if } k \leq n \\ \mu_{\diamond A, n}((k, *), (k, *)) \wedge \mu_{A, n}((k, *), (m, a')) & \text{otherwise} \end{cases} \\
&= \begin{cases} \mu_{A, n}((k + l, (j, a : (\triangleright^j A)_{n-k+l})), (m, a' : (\triangleright^m A)_n)) & \text{if } k + l \leq n \\ \mu_{A, n}((k + l, *), (m, a')) & \text{if } k \leq n < k + l \\ \mu_{A, n}((k, *), (m, a')) & \text{if } n < k \end{cases} \\
&= \begin{cases} m = k + l + j \wedge a = a' & \text{if } k + l \leq n \\ m = k + l \wedge a' = * & \text{if } k \leq n < k + l \\ m = k \wedge a' = * & \text{if } n < k \end{cases} \\
&= \begin{cases} (\mu_A)_{n-k}((l, (j, a)), (l + j, a)) \wedge \mu_{A, n}((k, (l + j, a)), (m, a')) & \text{if } k + l \leq n \\ (\mu_A)_{n-k}((l, *), (l, *)) \wedge \mu_{A, n}((k, (l, *)), (m, a')) & \text{if } k \leq n < k + l \\ m = k \wedge a' = * & \text{if } n < k \end{cases}
\end{aligned}$$

$$\begin{aligned}
&= \begin{cases} (\mu_A)_{n-k}((l, e_a), e'_a : (\Diamond A)_{n-k}) \wedge \mu_{A,n}((k, e'_a), (m, a')) & \text{if } k \leq n \\ k = m \wedge a' = * & \text{otherwise} \end{cases} \\
&= \begin{cases} (\Diamond \mu_A)_n((k, (l, e_a)), (k, e'_a : (\triangleright^k \Diamond A)_n)) \wedge \mu_{A,n}((k, e'_a), (m, a')) & \text{if } k \leq n \\ (\Diamond \mu_A)_n((k, *), (k, *)) \wedge \mu_{A,n}((k, *), (m, a')) & \text{otherwise} \end{cases} \\
&= \begin{cases} (\mu_A \circ \Diamond \mu_A)_n((k, (l, e_a : (\triangleright^l \Diamond A)_{n-k})), (m, a' : (\triangleright^m A)_n)) & \text{if } k \leq n \\ (\mu_A \circ \Diamond \mu_A)_n((k, *), (m, a' : (\triangleright^l A)_n)) & \text{otherwise} \end{cases} \\
&= (\mu_A \circ \Diamond \mu_A)_n((k, e_{e_a} : (\triangleright^k \Diamond \Diamond A)_n), (m, a' : (\triangleright^l A)_n))
\end{aligned}$$

Since the monad laws hold, we can conclude that  $\Diamond$  with  $\mu$  and  $\eta$  is a monad.  $\square$

## 6.5 Strength

As Moggi demonstrated, having only a monad structure for a type former is not enough to give a categorical semantics to a monadic language: the interpretation of a monadic binding rule such as `let evt  $x = t_1$  in  $t_2$`  requires us to go from an object like  $\llbracket \Gamma \rrbracket \otimes T\llbracket B \rrbracket$  to  $T(\llbracket \Gamma \rrbracket \otimes \llbracket B \rrbracket)$  so we can interpret  $t_2$  in the context under the monad  $T$ . Such a monad must be *strong*, i.e. be associated with a natural transformation

$$\text{st}_{A,B} : A \times TB \rightarrow T(A \times B)$$

called the *tensorial strength* of  $T$ .

In our specific case, tensorial strength is not appropriate: given that we want  $\Diamond$  to model temporal possibility, expecting a natural transformation  $A \otimes TB \rightarrow_{\mathcal{R}} T(A \otimes B)$  to exist for any  $A, B \in \text{Rel}_{\mathcal{R}}$  would mean asking for the temporal logic axiom  $A \wedge \Diamond B \implies \Diamond(A \wedge B)$ , which is not universally true (e.g. if it is raining now and will eventually stop raining, eventually it will be both raining and not raining).

Kobayashi introduced the notion of a  $\mathcal{L}$ -strong monad  $T$  for a monoidal comonad  $\mathcal{L}$  with a  $\mathcal{L}$ -tensorial strength transformation:

$$\text{st}_{A,B}^{\mathcal{L}} : \mathcal{L}A \times TB \rightarrow T(\mathcal{L}A \times B)$$

This formulation overcomes the problem above: as the comonad would model temporal necessity, a variant of tensorial strength can be introduced which ensures that the left side of the conjunct always holds – in particular when the event occurs. That is, we can give a model of constructive S4 temporal logic if we have a monoidal comonad  $\Box$ , and a  $\Box$ -strong monad  $\Diamond$  with  $\Box$ -tensorial strength

$$\text{st}_{A,B}^{\Box} : \Box A \times \Diamond B \rightarrow \Diamond(\Box A \times B)$$

Our calculus does not use a comonad – instead, we have a monoidal functor  $F : \text{Set} \rightarrow \text{Rel}_{\mathcal{R}}$  which plays a similar role in the language semantics (lifting the Cartesian context  $\Gamma$  into  $\text{Rel}_{\mathcal{R}}$ , allowing for duplication or deletion of the nonlinear context). We can adapt Kobayashi's notion of comonad-strong monads to define  $F$ -strong monads for a monoidal functor  $F$ .

**Definition 6.8.** Let  $\mathbb{C}, \mathbb{D}$  be two monoidal categories with units  $1_{\mathbb{C}}, 1_{\mathbb{D}}$  and tensor products  $\otimes, \times$  respectively. Let  $(F : \mathbb{D} \rightarrow \mathbb{C}, \mathbf{m}, \mathbf{u})$  be a (symmetric) monoidal functor and  $(T : \mathbb{C} \rightarrow \mathbb{C}, \eta, \mu)$  a

monad on  $\mathbb{C}$ . For an object  $X \in \mathbb{D}$  and  $A \in \mathbb{C}$ , we define the *F-tensorial strength* to be a natural transformation

$$\text{st}_{X,A}^F : FX \otimes TA \rightarrow T(FX \otimes A)$$

with the following coherence conditions:

$$\begin{array}{ccc} & F1_{\mathbb{D}} \otimes TA & \\ \text{st}_{1_{\mathbb{D}},A}^F \swarrow & & \searrow \lambda_{TA}^F \\ T(F1_{\mathbb{D}} \otimes A) & \xrightarrow{T\lambda_A^F} & TA \\ & T\lambda_A^F \circ \text{st}_{1_{\mathbb{D}},A}^F = \lambda_{TA}^F & \end{array}$$

$$\begin{array}{ccc} F(X \times Y) \otimes TA & \xrightarrow{\alpha_{X,Y,TA}^F} & FX \otimes (FY \otimes TA) \\ \text{st}_{X \times Y,A}^F \downarrow & & \downarrow \text{id}_{FX} \otimes \text{st}_{Y,A}^F \\ T(F(X \times Y) \otimes A) & & FX \otimes T(FY \otimes A) \\ & \searrow T\alpha_{X,Y,A}^F \quad \swarrow \text{st}_{X,FY \otimes A}^F & \\ & T(FX \otimes (FY \otimes A)) & \end{array}$$

$$T\alpha_{X,Y,A}^F \circ \text{st}_{X \times Y,A}^F = \text{st}_{X,FY \otimes A}^F \circ (\text{id}_{FX} \otimes \text{st}_{Y,A}^F) \circ \alpha_{X,Y,TA}^F$$

$$\begin{array}{ccccc} & FX \otimes A & & & \\ \text{id}_{FX} \otimes \eta_A \downarrow & \searrow \eta_{FX \otimes A} & & & \\ FX \otimes TA & \xrightarrow{\text{st}_{X,A}^F} & T(FX \otimes A) & & \\ \text{id}_{FX} \otimes \mu_A \uparrow & & \swarrow \mu_{FX \otimes A} & & \\ FX \otimes TTA & \xrightarrow{\text{st}_{X,TA}^F} & T(FX \otimes TA) & \xrightarrow{T\text{st}_{X,A}^F} & TT(FX \otimes A) \end{array}$$

$$\begin{aligned} \text{st}_{X,A}^F \circ (\text{id}_{FX} \otimes \eta_A) &= \eta_{FX \otimes A} \\ \mu_{FX \otimes A} \circ T\text{st}_{X,A}^F \circ \text{st}_{X,TA}^F &= \text{st}_{X,A}^F \circ (\text{id}_{FX} \otimes \mu_A) \end{aligned}$$

Here,  $\lambda_A^F : FT_{\mathbb{D}} \otimes A \rightarrow A$  denotes the “second projection”  $\lambda_A^{\mathbb{C}} \circ (u^{-1} \otimes \text{id}_A)$  where  $u : 1_{\mathbb{C}} \rightarrow F1_{\mathbb{D}}$  is the unit map of the monoidal functor  $F$  and  $\lambda_A^{\mathbb{C}} : 1_{\mathbb{C}} \otimes A \rightarrow A$  is the left unitor of  $\mathbb{C}$ . Similarly,  $\alpha_{X,Y,A}^F : F(X \times Y) \otimes A \rightarrow FX \otimes (FY \otimes TA)$  is the distributing associator  $\alpha_{FX,FY,TA}^{\mathbb{C}} \circ (\mathbf{m}_{X,Y}^{-1} \otimes \text{id}_{TA})$  where  $\mathbf{m}_{X,Y} : FX \otimes FY \rightarrow F(X \times Y)$  is the multiplication map of  $F$ .

Note that comonad-strong monads can be equivalently defined to have the natural transformation  $\text{st}_{A,B}^{\mathcal{L}} : \mathcal{L}A \times TB \rightarrow T(A \times B)$ , since the comonad  $\mathcal{L}$  can be freely dropped or duplicated to derive either version from the other. In our case this is of course not possible, since  $F$  is required to lift  $X \in \mathbb{D}$  to  $\mathbb{C}$ .

### 6.5.1 Strength for $\diamond$

To interpret our syntax, we need to show that  $\diamond : \text{Rel}_{\mathcal{R}} \rightarrow \text{Rel}_{\mathcal{R}}$  is a  $F$ -strong monad for the functor  $F = \text{id} \circ \Delta : \text{Set} \rightarrow \text{Rel}_{\mathcal{R}}$ . That is, we need to provide a natural transformation  $\text{st}^F$  with components

$$\text{st}_{X,A}^F : FX \otimes \diamond A \rightarrow_{\mathcal{R}} \diamond(FX \otimes A)$$

at  $X \in \text{Set}$  and  $A \in \text{Rel}_{\mathcal{R}}$ .

At the top point  $(FX)_{\top} = (\text{id} \Delta X)_{\top} = X$  and  $(\diamond A)_{\top} = A_{\top}$ , so  $\text{st}_{X,A,\top}^F : X \times A_{\top} \rightarrow X \times A_{\top}$  is the identity relation. At a timestep  $n$ , the transformation swaps two elements of the input tuple, unless the wait time has not been long enough.

$$\begin{aligned} \text{st}_{X,A}^F &: FX \otimes \diamond A \rightarrow_{\mathcal{R}} \diamond(FX \otimes A) \\ \text{st}_{X,A,\top}^F &: X \times A_{\top} \rightarrow X \times A_{\top} \\ \text{st}_{X,A,\top}^F &\triangleq \text{id}_{X \times A_{\top}} \\ \text{st}_{X,A,n}^F &: X \times \sum_{k \in \mathbb{N}} (\triangleright^k A)_n \rightarrow \sum_{l \in \mathbb{N}} (\triangleright^l (FX \otimes A))_n \\ \text{st}_{X,A,n}^F &\triangleq \{ ((x, (k, a)), (k, (x, a))) \mid k \leq n, x : X, a : (\triangleright^k A)_n \} \\ &\quad \cup \{ ((x, (k, *)), (k, *)) \mid k > n, x : X \} \end{aligned}$$

In the typing we use the fact that  $\triangleright^k$  is monoidal, so  $(\triangleright^k (FX \otimes A))_n = (\triangleright^k FX)_n \times (\triangleright^k A)_n$ . However, even though  $F$  is essentially the constant functor, we cannot say that  $(\triangleright^k FX)_n = X$ : the delay cannot be ignored since it changes the type at the first  $k$  timesteps. Thus, if  $k > n$ , both  $(\triangleright^k FX)_n$  and  $(\triangleright^k A)_n$  are  $\text{id}_0$ , even if the LHS of the relation only had  $a = *$  but  $x$  was a proper element of type  $X$ .

**Coherence** First, we need to prove the coherence condition: for all  $x, x' \in X, a, a' \in A_{\top}$

$$\text{st}_{X,A,n}^F \left( (\pi_n^{FX}(x), \pi_n^{\diamond A}(a)), \pi_n^{\diamond(FX \otimes A)}(x', a') \right) = \omega_n(\text{st}_{X,A,\top}^F((x, a), (x', a')))$$

The RHS is just the identity relation, and the LHS reduces to

$$\text{st}_{X,A,n}^F((x, (0, \pi_n^A(a))), (0, (x', \pi_n^A(a')))) \iff x = x' \wedge \pi_n^A(a) = \pi_n^A(a')$$

**Naturality** Below we prove the two naturality conditions for  $F$ -tensorial strength.

For  $f : X \rightarrow Y \in \text{Set}$ ,  $A \in \text{Rel}_{\mathcal{R}}$ , arguments  $(x, (k, a)) : X \times (\diamond A)_n$  and  $(l, s) : \diamond(FY \otimes A)_n$ , we have two cases:

**Case  $l \leq n$**

$$\begin{aligned} &(\diamond(Ff \otimes \text{id}_A) \circ \text{st}_{X,A}^F)_n((x : X, (k, a : (\triangleright^k A)_n)), (l, (y : Y, a' : A_{n-l}))) \\ &= (\diamond(Ff \otimes \text{id}_A))_n((k, (x, a)), (l, (y, a'))) \\ &= k = l \wedge (Ff \otimes \text{id}_A)_{n-l}((x, a), (y, a')) \\ &= k = l \wedge f(x) = y \wedge a = a' \\ &= f(x) = y \wedge (k, a) = (l, a') \\ &= ((Ff \otimes \text{id}_{\diamond A}))_n((x : X, (k, a : (\triangleright^k A)_n)), (y, (l, a'))) \\ &= (\text{st}_{Y,A}^F \circ (Ff \otimes \text{id}_{\diamond A}))_n((x : X, (k, a : (\triangleright^k A)_n)), (l, (y : Y, a' : A_{n-l}))) \end{aligned}$$

**Case  $l > n$**

$$\begin{aligned}
& (\diamond(Ff \otimes \text{id}_A) \circ \text{st}_{X,A}^F)_n((x : X, (k, a : (\triangleright^k A)_n)), (l, *)) \\
&= (\diamond(Ff \otimes \text{id}_A))_n((k, (x, a)), (l, *)) \\
&= k = l \wedge (\triangleright^+(Ff \otimes \text{id}_A))_0((x, a), *) \\
&= k = l \\
&= (\exists y' : Y. f(x) = y') \wedge k = l \\
&= \exists(y' : Y, (p, \hat{a} : (\triangleright^p A)_n)). (Ff)_n(x, y') \wedge (k, a) = (p, \hat{a}) \wedge p = l \\
&= \exists(y' : Y, (p, \hat{a} : (\triangleright^p A)_n)). (Ff \otimes \text{id}_{\diamond A})_n((x, (k, a)), (y', (p, \hat{a}))) \wedge \text{st}_{Y,A,n}^F((y', (p, \hat{a})), (l, *)) \\
&= (\text{st}_{Y,A}^F \circ (Ff \otimes \text{id}_{\diamond A}))_n((x : X, (k, a : (\triangleright^k A)_n)), (l, *))
\end{aligned}$$

For  $r : A \rightarrow_{\mathcal{R}} B \in \text{Rel}_{\mathcal{R}}$ ,  $X \in \text{Set}$ , arguments  $(x, (k, a)) : X \times (\diamond A)_n$  and  $(l, s) : \diamond(FX \otimes B)_n$ , we have two cases:

**Case  $l \leq n$**

$$\begin{aligned}
& (\diamond(\text{id}_{FX} \otimes r) \circ \text{st}_{X,A}^F)_n((x : X, (k, a : (\triangleright^k A)_n)), (l, (x' : X, b : B_{n-l}))) \\
&= (\diamond(\text{id}_{FX} \otimes r))_n((k, (x, a)), (l, (x', b))) \\
&= k = l \wedge (\triangleright^l(\text{id}_{FX} \otimes r))_n((x, a), (x', b)) \\
&= k = l \wedge x = x' \wedge r_{n-l}(a, b) \\
&= x = x' \wedge (\text{id}_{FX} \otimes \diamond r)_n((k, a), (l, b)) \\
&= (\text{id}_{FX} \otimes \diamond r)_n((x, (k, a)), (x', (l, b))) \\
&= (\text{st}_{X,B}^F \circ (\text{id}_{FX} \otimes \diamond r))_n((x : X, (k, a : (\triangleright^k A)_n)), (l, (x' : X, b : B_{n-l})))
\end{aligned}$$

**Case  $l > n$**

$$\begin{aligned}
& (\diamond(\text{id}_{FX} \otimes r) \circ \text{st}_{X,A}^F)_n((x : X, (k, a : (\triangleright^k A)_n)), (l, *)) \\
&= (\diamond(\text{id}_{FX} \otimes r))_n((k, (x, a)), (l, *)) \\
&= k = l \wedge (\triangleright^+(\text{id}_{FX} \otimes r))_0((x, a), *) \\
&= k = l \\
&= (\exists \hat{x} : X. x = \hat{x}) \wedge k = l \wedge (\triangleright^{l-n} r)_0(a, *) \\
&= \exists(\hat{x} : X, (p, b' : (\triangleright^p B)_n)). x = \hat{x} \wedge (\diamond r)_n((k, a), (p, b')) \wedge p = l \\
&= \exists(\hat{x} : X, (p, b' : (\triangleright^p B)_n)). (\text{id}_{FX} \otimes \diamond r)_n((x, (k, a)), (\hat{x}, (p, b'))) \wedge \text{st}_{X,A,n}^F((\hat{x}, (p, b')), (l, *)) \\
&= (\text{st}_{X,B}^F \circ (\text{id}_{FX} \otimes \diamond r))_n((x : X, (k, a : (\triangleright^k A)_n)), (l, *))
\end{aligned}$$

**$F$ -tensorial strength laws** Below we prove the laws associated with  $F$ -tensorial strength.

For the unit law, let  $A$  be an object in  $\text{Rel}_{\mathcal{R}}$ . For arguments  $(*, (k, a)) : (F1 \otimes \diamond A)_n$  and  $(l, a') : (\diamond A)_n$ , we have two cases:

**Case  $l \leq n$**

$$(\diamond \lambda_A^F \circ \text{st}_{1,A}^F)_n((*, (k, a : (\triangleright^k A)_n)), (l, a' : (\triangleright^l A)_n))$$

$$\begin{aligned}
&= (\diamond \lambda_A^F)_n((k, (*, a)), (l, a')) \\
&= k = l \wedge (\triangleright^l \lambda_A^F)_n((* , a), a') \\
&= k = l \wedge a = a' \\
&= (\lambda_{\diamond A}^F)_n((* , (k, a : (\triangleright^k A)_n)), (l, a' : (\triangleright^l A)_n))
\end{aligned}$$

**Case  $l > n$**

$$\begin{aligned}
&(\diamond \lambda_A^F \circ \mathbf{st}_{1,A}^F)_n((* , (k, a : (\triangleright^k A)_n)), (l, *)) \\
&= \exists(m, p : (\triangleright^m(F1 \otimes A)_n)). \mathbf{st}_{1,A,n}^F((* , (k, a)), (m, p)) \wedge (\diamond \lambda_A^F)_n((m, p), (l, *)) \\
&= \exists(m, p : (\triangleright^m(F1 \otimes A)_n)). k = m \wedge p = (*, a) \wedge m = l \wedge (\triangleright^l \lambda_A^F)_n(p, *) \\
&= k = l \wedge (\triangleright^{l-n} \lambda_A^F)_0((* , a), *) \\
&= k = l \wedge a = * \\
&= (\lambda_{\diamond A}^F)_n((* , (k, a : (\triangleright^k A)_n)), (l, *))
\end{aligned}$$

For the associativity law, let  $X, Y \in \mathbf{Set}$  and  $A \in \mathbf{Rel}_{\mathcal{R}}$ . For arguments  $(*, (k, a)) : (F1 \otimes \diamond A)_n$  and  $(l, a') : (\diamond A)_n$ , we have two cases:

**Case  $l \leq n$**

$$\begin{aligned}
&(\mathbf{st}_{X,FY \otimes A}^F \circ (\mathbf{id}_{FX} \otimes \mathbf{st}_{Y,A}^F) \circ \alpha_{X,Y,\diamond A}^F)_n(((x, y), (k, a : (\triangleright^k A)_n)), (l, (x', (y', a' : A_{n-l})))) \\
&= (\mathbf{st}_{X,FY \otimes A}^F \circ (\mathbf{id}_{FX} \otimes \mathbf{st}_{Y,A}^F))_n((x, (y, (k, a))), (l, (x', (y', a')))) \\
&= (\mathbf{id}_{FX} \otimes \mathbf{st}_{Y,A}^F)_n((x, (y, (k, a))), (x', (l, (y', a')))) \\
&= x = x' \wedge \mathbf{st}_{Y,A,n}^F((y, (k, a)), (l, (y', a'))) \\
&= x = x' \wedge y = y' \wedge k = l \wedge a = a' \\
&= k = l \wedge (\alpha_{X,Y,A}^F)_{n-l}(((x, y), a), (x', (y', a'))) \\
&= (\diamond \alpha_{X,Y,A}^F)_n((k, ((x, y), a)), (l, (x', (y', a')))) \\
&= (\diamond \alpha_{X,Y,A}^F \circ \mathbf{st}_{X \times Y,A}^F)_n(((x, y), (k, a : (\triangleright^k A)_n)), (l, (x', (y', a' : A_{n-l}))))
\end{aligned}$$

**Case  $l > n$**

$$\begin{aligned}
&(\mathbf{st}_{X,FY \otimes A}^F \circ (\mathbf{id}_{FX} \otimes \mathbf{st}_{Y,A}^F) \circ \alpha_{X,Y,\diamond A}^F)_n(((x, y), (k, a : (\triangleright^k A)_n)), (l, *)) \\
&= (\mathbf{st}_{X,FY \otimes A}^F \circ (\mathbf{id}_{FX} \otimes \mathbf{st}_{Y,A}^F))_n((x, (y, (k, a))), (l, *)) \\
&= (\mathbf{st}_{X,FY \otimes A}^F)_n((x, (k, (y, a))), (l, *)) \\
&= k = l \\
&= k = l \wedge (\triangleright^{n-l} \alpha_{X,Y,A}^F)_0(((x, y), a), *) \\
&= (\diamond \alpha_{X,Y,A}^F)_n((k, ((x, y), a)), (l, *)) \\
&= (\diamond \alpha_{X,Y,A}^F \circ \mathbf{st}_{X \times Y,A}^F)_n(((x, y), (k, a : (\triangleright^k A)_n)), (l, *))
\end{aligned}$$

**$F$ -strong monad laws** Below we prove the laws associated with  $\diamond$  being an  $F$ -strong monad.

First, the law relating monadic unit and strength:

$$\begin{aligned}
& (\text{st}_{X,A}^F \circ (\text{id}_{FX} \otimes \eta_A))_n((x : X, a : A_n), (l, p : (\triangleright^l(FX \otimes A)_n))) \\
&= \text{st}_{X,A,n}^F((x : X, (0, a : A_n)), (l, p : (\triangleright^l(FX \otimes A)_N))) \\
&= l = 0 \wedge p = (x, a) \\
&= (\eta_{FX \otimes A})_n((x : X, a : A_n), (l, p : (\triangleright^l(FX \otimes A)_n)))
\end{aligned}$$

Note that we do not have to split the cases when  $l \leq n$  and  $l > n$ : since  $l$  has to be 0, the case  $l > n$  is impossible.

The law relating the monadic multiplication and strength:

**Case  $k \leq n$**

$$\begin{aligned}
& (\mu_{FX \otimes A} \circ \diamond \text{st}_{X,A}^F \circ \text{st}_{X,\diamond A}^F)_n((x : X, (k, (l, a : (\triangleright^l A)_{n-k}))), (m, s : (\triangleright^m(FX \otimes A)_n))) \\
&= (\mu_{FX \otimes A} \circ \diamond \text{st}_{X,A}^F)_n((k, (x, (l, a))), (m, s)) \\
&= (\mu_{FX \otimes A})_n((k, (l, (x, a))), (m, s)) \\
&= k + l = m \wedge s = (x, a) \\
&= \text{st}_{X,A,n}^F((x, (k + l, a)), (m, s)) \\
&= (\text{st}_{X,A}^F \circ (\text{id}_{FX} \otimes \mu_A))_n((x : X, (k, (l, a : (\triangleright^l A)_{n-k}))), (m, s : (\triangleright^m(FX \otimes A)_n)))
\end{aligned}$$

**Case  $k > n$**

$$\begin{aligned}
& (\mu_{FX \otimes A} \circ \diamond \text{st}_{X,A}^F \circ \text{st}_{X,\diamond A}^F)_n((x : X, (k, *)), (m, s : (\triangleright^m(FX \otimes A)_n))) \\
&= \exists(p, t : (\triangleright^p(FX \otimes \diamond A))_n). \text{st}_{X,\diamond A,n}^F((x, (k, *)), (p, t)) \wedge (\mu_{FX \otimes A} \circ \diamond \text{st}_{X,A}^F)_n((p, t), (m, s)) \\
&= \exists(p, t : (\triangleright^p(FX \otimes \diamond A))_n). k = p \wedge (\mu_{FX \otimes A} \circ \diamond \text{st}_{X,A}^F)_n((p, t), (m, s)) \\
&= (\mu_{FX \otimes A} \circ \diamond \text{st}_{X,A}^F)_n((k, *), (m, s)) \\
&= \exists(q, u : (\triangleright^q \diamond(FX \otimes A))_n). (\diamond \text{st}_{X,A}^F)_n((k, *), (q, u)) \wedge \mu_{FX \otimes A,n}((q, u), (m, s)) \\
&= \exists(q, u : (\triangleright^q \diamond(FX \otimes A))_n). k = q \wedge (\triangleright^+ \text{st}_{X,A}^F)_0(*, *) \wedge \mu_{FX \otimes A,n}((q, u), (m, s)) \\
&= k = m \\
&= \text{st}_{X,A,n}^F((x, (k, *)), (m, s)) \\
&= \exists(l, \hat{a} : (\triangleright^l A)_n). k = l \wedge \text{st}_{X,A,n}^F((x, (l, \hat{a})), (m, s)) \\
&= \exists(\hat{x} : X, (l, \hat{a} : (\triangleright^l A)_n)). x = \hat{x} \wedge \mu_{A,n}((k, *), (l, \hat{a})) \wedge \text{st}_{X,A,n}^F((\hat{x}, (l, \hat{a})), (m, s)) \\
&= \exists(\hat{x} : X, (l, \hat{a} : (\triangleright^l A)_n)). (\text{id}_{FX} \otimes \mu_A)_n((x, (k, *)), (\hat{x}, (l, \hat{a}))) \wedge \text{st}_{X,A,n}^F((\hat{x}, (l, \hat{a})), (m, s)) \\
&= (\text{st}_{X,A}^F \circ (\text{id}_{FX} \otimes \mu_A))_n((x : X, (k, *)), (m, s : (\triangleright^m(FX \otimes A)_n)))
\end{aligned}$$

Thus we can conclude that  $\diamond$  is an  $F$ -strong monad.

## 6.6 Linearity

An important operation in our syntax is comparing two events and executing different code based on which event fires first. To interpret this operation, we need to analyse how the product of two



events behaves: is  $\Diamond$  simply a monoidal functor or does it have extra structure? Temporally, we do not expect  $\Diamond A \wedge \Diamond B = \Diamond(A \wedge B)$  to be an axiom of LTL: the two events are not guaranteed to happen at the same time so they might not be true simultaneously. However, we can say that eventually at least one of the events must occur: either the first or the second, or both. That is, we should be able to expand  $\Diamond A \wedge \Diamond B$  to  $\Diamond((A \wedge \Diamond B) \vee (\Diamond A \wedge B) \vee (A \wedge B))$ . Accordingly, we can impose this linearity property on our event modality by providing a natural transformation

$$\text{race}_{A,B} : \Diamond A \otimes \Diamond B \rightarrow_{\mathcal{R}} \Diamond(A \otimes \Diamond B \oplus \Diamond A \otimes B)$$

that “races” two events and returns the sum of the possible outcomes, based on which event happened first. The third possibility (which corresponds to both events happening simultaneously) is subsumed by the fact that the morphisms in  $\text{Rel}_{\mathcal{R}}$  are relations: in case of ambiguity we can return both possibilities.

To define  $\text{race}$  in  $\text{Rel}_{\mathcal{R}}$ , we make use of a few helper functions. Since  $\text{race}$  has to compare the occurrence times of its two input events and choose the left or right injection based on their order, we factor out the

Since  $(\Diamond A)_{\top} = A_{\top}$ , at the top point the relation holds if the second argument is either the left or right injection of the first. At a timestep  $n$ , we need to compare the occurrence times of the two input events  $\Diamond A$  and  $\Diamond B$ , and return the appropriate injection based on which one happened first.

$$\begin{aligned} \text{race}_{A,B} &: \Diamond A \otimes \Diamond B \rightarrow_{\mathcal{R}} \Diamond(A \otimes \Diamond B \oplus \Diamond A \otimes B) \\ \text{race}_{A,B,\top} &: A_{\top} \times B_{\top} \rightarrow (A_{\top} \times B_{\top} + A_{\top} \times B_{\top}) \\ \text{race}_{A,B,\top}(p, \text{inl}(q)) &\triangleq \text{id}_{A \times B, \top}(p, q) \\ \text{race}_{A,B,\top}(p, \text{inr}(q)) &\triangleq \text{id}_{A \times B, \top}(p, q) \\ \text{race}_{A,B,n} &: \sum_k (\triangleright^k A)_n \times \sum_l (\triangleright^l B)_n \rightarrow \sum_m (\triangleright^m (A \otimes \Diamond B \oplus \Diamond A \otimes B))_n \\ \text{race}_{A,B,n}((k, a : (\triangleright^k A)_n), (l, b : (\triangleright^l B)_n), (m, s)) &\triangleq \\ &\begin{cases} m = k \wedge (\triangleright^k \text{inl} \circ m_{A, \Diamond B}^{\triangleright^k} \circ (\triangleright^k A \times \triangleright^k \text{evt}_B^{l-k}))_n((a, b), s) & \text{if } k < l \\ m = l \wedge (\triangleright^l \text{inr} \circ m_{\Diamond A, B}^{\triangleright^l} \circ (\triangleright^l \text{evt}_A^{k-l} \times \triangleright^l B))_n((a, b), s) & \text{if } k > l \\ m = k \wedge ((\triangleright^k \text{inl} \circ m_{A, \Diamond B}^{\triangleright^k} \circ (\triangleright^k A \times \triangleright^k \eta_B))_n((a, b), s) \vee \\ (\triangleright^l \text{inr} \circ m_{\Diamond A, B}^{\triangleright^l} \circ (\triangleright^l \eta_A \times \triangleright^l B))_n((a, b), s)) & \text{if } k = l \end{cases} \end{aligned}$$

Here,  $\text{evt}_A^k$  simply converts a delayed value into an event by attaching the time step as the first element of the dependent sum. In particular,  $\text{evt}_A^0 : A \rightarrow_{\mathcal{R}} \Diamond A = \eta_A$ .

$$\begin{aligned} \text{evt}_A^k &: \triangleright^k A \rightarrow_{\mathcal{R}} \Diamond A \\ \text{evt}_{A,n}^k(a, (m, a')) &\triangleq m = k \wedge a = a' \end{aligned}$$

We use this transformation to convert a value of type  $\triangleright^l B$  to  $\triangleright^k \Diamond B$ , assuming that  $l > k$ : by definition,  $\triangleright^l B = \triangleright^k (\triangleright^{l-k} B)$  so we can use  $\triangleright^k \text{evt}_B^{l-k}$  to transform the latter into  $\triangleright^k \Diamond B$ . Applying the multiplication of the monoidal functor  $\triangleright^k$  to  $\triangleright^k A$  and  $\triangleright^k \Diamond B$ , and injecting it into the left side of the sum gives us a value of the right type  $\triangleright^k (A \otimes \Diamond B \oplus \Diamond A \otimes B)$ . The case for  $k > l$  is constructed in a similar way. When  $k = l$ , there are no “leftover” delay steps to convert into an event so we apply  $m_{A,B}^{\triangleright^k}$  and check whether the result is either the left or right injection.

**Theorem 6.9.** The relation  $\text{race}$  is a natural transformation: for  $r : A \rightarrow_{\mathcal{R}} A'$ ,

$$\Diamond(r \otimes \Diamond B \oplus \Diamond r \otimes B) \circ \text{race}_{A,B} = \text{race}_{A',B} \circ \Diamond r \otimes \Diamond B$$

and for  $s : B \rightarrow_{\mathcal{R}} B'$ ,

$$\Diamond(A \otimes \Diamond r \oplus \Diamond A \otimes r) \circ \text{race}_{A,B} = \text{race}_{A,B'} \circ \Diamond A \otimes \Diamond r$$

*Proof.* Let  $r : A \rightarrow_{\mathcal{R}} A'$ . At the top point,  $\text{race}$  is essentially the right or left injection which is natural. At a timestep  $n$ , we have inputs  $(k, a) : \Diamond A$ ,  $(l, b) : \Diamond B$  and  $(m, s) : \Diamond(A \otimes \Diamond B \oplus \Diamond A \otimes B)$ . We can analyse the cases when  $k < l$ ,  $k > l$  or  $k = l$ . Below is the naturality proof for the  $k < l$  case; note that it is a categorical equational proof, so for simplicity we omit the arguments in the middle section of the proof.

$$\begin{aligned} & (\Diamond(r \otimes \Diamond B \oplus \Diamond r \otimes B) \circ \text{race}_{A,B})_n(((k, a), (l, b)), (m, s)) \\ &= (\triangleright^k(r \otimes \Diamond B \oplus \Diamond r \otimes B) \circ \triangleright^k \text{inl} \circ \mathbf{m}_{A, \Diamond B}^k \circ (\triangleright^k A \otimes \triangleright^k \text{evt}_B^{l-k}))_n((a, b), s) \\ &= \triangleright^k \text{inl} \circ \triangleright^k(r \otimes \Diamond B) \circ \mathbf{m}_{A, \Diamond B}^k \circ (\triangleright^k A \otimes \triangleright^k \text{evt}_B^{l-k}) \quad (\text{naturality of inl}) \\ &= \triangleright^k \text{inl} \circ \mathbf{m}_{A', \Diamond B}^k \circ (\triangleright^k r \otimes \triangleright^k \Diamond B) \circ (\triangleright^k A \otimes \triangleright^k \text{evt}_B^{l-k}) \quad (\text{naturality of } \mathbf{m}^k) \\ &= \triangleright^k \text{inl} \circ \mathbf{m}_{A', \Diamond B}^k \circ ((\triangleright^k r \circ \triangleright^k A) \otimes (\triangleright^k \Diamond B \circ \triangleright^k \text{evt}_B^{l-k})) \quad (\text{SMCC laws}) \\ &= \triangleright^k \text{inl} \circ \mathbf{m}_{A', \Diamond B}^k \circ ((\triangleright^k A' \circ \triangleright^k r) \otimes (\triangleright^k \text{evt}_B^{l-k} \circ \triangleright^k \triangleright^{l-k} B)) \quad (\text{naturality of id}) \\ &= \triangleright^k \text{inl} \circ \mathbf{m}_{A', \Diamond B}^k \circ (\triangleright^k A' \otimes \triangleright^k \text{evt}_B^{l-k}) \circ (\triangleright^k r \otimes \triangleright^l B) \quad (\text{SMCC laws}) \\ &= (\text{race}_{A',B} \circ (\triangleright^k r \otimes \triangleright^l B))_n((a, b), s) \quad (\text{def. of race}) \\ &= (\text{race}_{A',B} \circ \Diamond r \otimes \Diamond B)_n(((k, a), (l, b)), (m, s)) \end{aligned}$$

Due to the symmetric definition the proof for the  $k > l$  case is similar. When  $k = l$ , we can do case analysis on the argument  $s$  (assuming  $n \leq m$ , i.e.  $n \leq k$  – the proof is simple otherwise) and match either of the cases in the definition of  $\text{race}$ , at which point the naturality proof has the same structure as the one above. The second naturality proof (for  $s : B \rightarrow_{\mathcal{R}} B'$ ) the proof is again very similar due to the symmetric nature of the  $\text{race}$  relation.  $\square$

## 7 Widgets

### 7.1 Syntax of widgets

In the syntax of the language, widgets are represented by the first-class type  $\text{Widget}^\ell$  that is treated as an abstract data type with associated operations. This allows us flexibility to interpret and implement widgets in appropriate ways. We also have restricted form a widget called a prefix, which corresponds to a widget with a finite lifetime. Recall the type formation rule for widgets and prefixes:

$$\frac{\Theta \vdash_s \iota : \text{id}}{\Theta \vdash_\ell \text{Widget}^\ell \text{ type}} \text{ (WIDGET)} \qquad \frac{\Theta \vdash_s \tau : \text{time} \quad \Theta \vdash_s \iota : \text{id}}{\Theta \vdash_\ell \text{Prefix}^\ell(\tau) \text{ type}} \text{ (PREFIX)}$$

Both types are indexed by an identifier  $\iota$ , which is required to differentiate between widgets, especially when manipulating their temporal behaviour. The additional  $\tau$  index of prefixes represents the lifetime of the widget, i.e. the number of timesteps it is available. This distinction is required to implement widget splitting, when we separate the history of a widget into a finite prefix, and the rest of the history delayed by some number of time steps.

Construction and interaction with widgets happens through a collection of built-in primitives.

**Creation and deletion** In a linear setting we need to be explicit about creating and deleting widgets.

$$\begin{aligned} \text{create} &: \forall \iota : \text{id}. \mathbf{I} \multimap \text{Widget}^\iota \\ \text{delete} &: \forall \iota : \text{id}. \text{Widget}^\iota \multimap \mathbf{I} \end{aligned}$$

**Modification** A collection of linear functions for manipulating the state of a widget. Linearity means that the widget argument gets consumed, so we will never have access to the same widget's state both before and after the change.

$$\begin{aligned} \text{setLabel} &: \forall \iota : \text{id}. \text{Widget}^\iota \otimes \mathbf{F} \text{ String} \multimap \text{Widget}^\iota \\ \text{setColour} &: \forall \iota : \text{id}. \text{Widget}^\iota \otimes \mathbf{F} \text{ Colour} \multimap \text{Widget}^\iota \end{aligned}$$

**Event listening** Functions to register event listeners on the widgets. Alongside a linear copy of the widget, they return a value of type  $\Diamond A$ , representing an event that will give a value of type  $A$  at some point. We can then handle the event in the event binding constructs `let evt` and `select`.

$$\begin{aligned} \text{onClick} &: \forall \iota : \text{id}. \text{Widget}^\iota \multimap \text{Widget}^\iota \otimes \Diamond \mathbf{I} \\ \text{onKeyPress} &: \forall \iota : \text{id}. \text{Widget}^\iota \multimap \text{Widget}^\iota \otimes \Diamond (\mathbf{F} \text{ Char}) \end{aligned}$$

**Splitting** Inverse functions used to split and rejoin the temporal behaviour of a widget at a specific future time step. After splitting, we get the widget's prefix up to the time step, then we get the rest of the history as a widget delayed by  $\tau$  time steps. The `join` function glues these back together, reconstructing a full widget (the identifiers ensure that we don't attach the prefix of one widget to the future of another). The idea is that we can perform modifications on the delayed part of the widget (such as changing its colour), specifying how its state should change at a future time step. Combined with event handling, this lets us access the state of the widget at the exact point that an event happens.

$$\begin{aligned} \text{split} &: \forall \iota : \text{id}, \tau : \text{time}. \text{Widget}^\iota \multimap \text{Prefix}^\iota(\tau) \otimes (\text{Widget}^\iota @ \tau) \\ \text{join} &: \forall \iota : \text{id}, \tau : \text{time}. \text{Prefix}^\iota(\tau) \otimes (\text{Widget}^\iota @ \tau) \multimap \text{Widget}^\iota \end{aligned}$$

## 7.2 Semantics of widgets

Widgets are interpreted as distinguished objects in  $\text{Rel}_{\mathcal{R}}$  that capture both the static state and temporal behaviour of GUI elements. Instead of interpreting them as a fixed object with some state (its colour, label, etc.), or a stream of states, we use a “logbook semantics” that keeps track of the individual state changes that happen to the widget, including their time step. This fits in

nicely with the structure of objects in  $\text{Rel}_{\mathcal{R}}$ : the top point contains the full log of changes, while the individual projections at a timestep  $k$  select out only the changes that occurred before time  $k$ , thereby giving the specification for reconstructing the state of the widget at that time step. Two widgets that have the same temporal behaviour (i.e. the projections are the same at every time step) may have different global specifications and we can differentiate between through interaction – a semantics based on streams of states would not be able to distinguish between them.

### 7.2.1 Indices

Each widget is indexed by an identifier  $\iota : \text{Id}$ , where we take  $\text{Id}$  to be some countable set of indices – since there are no constants of the type  $\text{id}$  in the syntax, we don't need to commit to any particular representation and keep the details opaque. In an implementation, this could be a number or a pointer address, for example.

We also need a representation of the time steps associated with the log entries. These are different from the times that index the  $\text{Rel}_{\mathcal{R}}$  objects; in particular, each entry must be associated with a finite time step. The simplest choice is just  $\mathbb{N}$ , and we will denote this set by  $\text{Time}$  to make the distinction explicit.

### 7.2.2 Commands

We mark a state change on a widget by associating a primitive command with a time step. We assume some distinguished sets corresponding to various widget attributes:

$$\text{Char} \triangleq \{\mathbf{a}, \mathbf{b}, \mathbf{c}, \dots\} \quad \text{String} \triangleq \text{Char}^* \quad \text{Colour} \triangleq \{\mathbf{red}, \mathbf{blue}, \dots\}$$

The set of commands contains function symbols  $\text{setLabel}, \text{setColour}, \dots$  associated with some arguments.

$$\text{Cmd} \triangleq (\{\text{setLabel}\} \times \text{String}) \cup (\{\text{setColour}\} \times \text{Colour}) \cup (\{\text{setFont}\} \times \text{String}) \cup \dots$$

Two commands are compatible if they can be applied to the widget at the same time, without ambiguity: for instance, we can set the label and colour of a widget at the same time, but setting its label to two different strings at the same time will be ambiguous. The compatibility relation  $\bowtie : \text{Cmd} \rightarrow \text{Cmd}$  ensures this: for instance, we have  $(\text{setLabel}, \text{"OK"}) \bowtie (\text{setColour}, \text{"red"})$ , but not  $(\text{setLabel}, \text{"OK"}) \bowtie (\text{setLabel}, \text{"Cancel"})$ .

$$(op, arg) \bowtie (op', arg') \iff (op = op' \Rightarrow arg = arg')$$

We can lift command compatibility to log entry compatibility: two entries are compatible either if they occur at different times, or the commands are compatible.

$$(t, c) \bowtie (t', c') \iff (t \neq t' \vee c \bowtie c')$$

### 7.2.3 Widgets

**Definition 7.1.** The *widget object*  $\text{Widget}^\iota \in \text{Rel}_{\mathcal{R}}$  for an identifier  $\iota \in \text{Id}$  is defined as:

$$\begin{aligned} \text{Widget}_\top^\iota &\triangleq \{W \subseteq \text{Time} \times \text{Cmd} \mid \forall (t, c), (t', c') \in W. (t, c) \bowtie (t', c')\} \\ \text{Widget}_n^\iota &\triangleq \{W \subseteq \text{Widget}_\top^\iota \mid \forall (t, c) \in W. t \leq n\} \end{aligned}$$

The projections extract the entries below the time step:

$$\pi_n^{\text{Widget}^t}(W) \triangleq \{(t, c) \in W \mid t \leq n\}$$

We also define a restricted form of a widget which only persists for some number of time steps.

$$\begin{aligned} \text{Prefix}^t(\tau)_\top &\triangleq \{P \subseteq \text{Widget}_\top^t \mid \forall (t, c) \in P. t < \tau\} \\ \text{Prefix}^t(\tau)_n &\triangleq \begin{cases} \{P \subseteq \text{Prefix}^t(\tau)_\top \mid \forall (t, c) \in P. t \leq n\} & \text{if } n < \tau \\ \mathbf{1} & \text{otherwise} \end{cases} \end{aligned}$$

The projections return either the entries up to  $\tau$ , or the unit.

$$\pi_n^{\text{Prefix}^t(\tau)}(P) \triangleq \begin{cases} \{(t, c) \in P \mid t < \tau\} & \text{if } n < \tau \\ \langle \rangle & \text{otherwise} \end{cases}$$

Intuitively, a widget is interpreted as a  $\text{Rel}_{\mathcal{R}}$  object containing a collection of compatible entries of commands. At the top point, we get the full logbook of a widget's history: what commands get applied to it at which timestep. At the projections we only select the entries that happen before the projected time, so the state of the widget can be determined at any time  $k$  by applying the commands in the widget's  $k$ th projection. The compatibility ensures that we never get ambiguous or inconsistent results: a specific attribute of a widget won't be set to two different values at the same time. We do not fix a concrete representation of the state of a widget (such as its colour, label, etc.) and instead keep the projections as subsets of the full log; given a specific widget representation (such as a DOM element), we can determine its state at time  $k$  by executing the commands in order, up to  $k$ .

#### 7.2.4 Widget splitting

The `split` and `join` primitives allow us to directly manipulate the future history of the widgets, thereby having access to their state at a future time step.

**Definition 7.2** (Widget restriction). For a time step  $t \in \text{Time}$ , we define the following morphisms  $\text{Widget}^t \rightarrow_{\mathcal{R}} \text{Widget}^t$ :

$$\begin{aligned} (\downarrow \tau) &: \text{Widget}^t \rightarrow_{\mathcal{R}} \text{Prefix}^t(\tau) \\ (\downarrow \tau)_{k \in \mathbb{N}_\top} &\triangleq \{(W, \pi_k^{\text{Prefix}^t(\tau)} \{(t, c) \in W \mid t < \tau\}) \mid W : \text{Widget}_k^t\} \\ (\ominus \tau) &: \text{Widget}^t \rightarrow_{\mathcal{R}} \text{Widget}^t \\ (\ominus \tau) &\triangleq \{(W, \{(t - \tau, c) \mid (t, c) \in W \wedge \tau \leq t\}) \mid W : \text{Widget}^t\} \end{aligned}$$

Intuitively,  $\downarrow t$  relates a widget to its copy with all entries after time  $t$  removed, and  $\ominus t$  relates a widget to its copy with all entries shifted forward by  $t$ .

**Definition 7.3** (Splitting and joining widgets).

$$\begin{aligned} \text{split}_\tau &: \text{Widget}^t \rightarrow_{\mathcal{R}} \text{Prefix}^t(\tau) \otimes \triangleright^\tau \text{Widget}^t \\ \text{split}_{\tau, \top}(W : \text{Widget}_\top^t, (P : \text{Prefix}^t(\tau)_\top, W' : \text{Widget}_\top^t)) &\triangleq W (\downarrow \tau) P \wedge W (\ominus \tau) W' \end{aligned}$$

$$\begin{aligned}
split_{\tau,n}(W : \text{Widget}^t_n, (P : \text{Prefix}^t(\tau)_n, W' : (\triangleright^\tau \text{Widget}^t)_n)) &\triangleq \begin{cases} W = P & \text{if } n < \tau, W' = \text{I} \\ W (\ominus \tau) W' & \text{if } n \geq \tau, P = \text{I} \end{cases} \\
join_\tau : \text{Prefix}^t(\tau) \otimes \triangleright^\tau \text{Widget}^t &\rightarrow_{\mathcal{R}} \text{Widget}^t \\
join_{\tau,\top}((P : \text{Prefix}^t(\tau)_\top, W' : \text{Widget}^t_\top), W : \text{Widget}^t_\top) &\triangleq W (\downarrow \tau) P \wedge W (\ominus \tau) W' \\
join_{\tau,n}((P : \text{Prefix}^t(\tau)_n, W' : (\triangleright^\tau \text{Widget}^t)_n), W : \text{Widget}^t_n) &\triangleq \begin{cases} W = P & \text{if } n < \tau, W' = \text{I} \\ W (\ominus \tau) W' & \text{if } n \geq \tau, P = \text{I} \end{cases}
\end{aligned}$$

As an example of splitting and joining, consider a widget  $W : \text{Widget}^t$  that associates every time step with a character (e.g. a label):

$$W_\top = \{(0, \mathbf{a}), (1, \mathbf{b}), (2, \mathbf{c}), (3, \mathbf{d}), (4, \mathbf{e}), (5, \mathbf{f}), (6, \mathbf{g}), (7, \mathbf{h}), \dots\}$$

The individual projections  $W_n$  are all the entries up to  $n$ :

$$W_2 = \{(0, \mathbf{a}), (1, \mathbf{b}), (2, \mathbf{c})\} \quad W_4 = \{(0, \mathbf{a}), (1, \mathbf{b}), (2, \mathbf{c}), (3, \mathbf{d}), (4, \mathbf{e})\}$$

If we split  $W$  at time  $\tau = 4$ , the top point will contain the finite prefix up to (and not including) the entry at 4, then another widget with all the entries from 4, shifted back by four.

$$split_{4,\top}(W) = (\{(0, \mathbf{a}), (1, \mathbf{b}), (2, \mathbf{c}), (3, \mathbf{d})\}, \quad \{(0, \mathbf{e}), (1, \mathbf{f}), (2, \mathbf{g}), (3, \mathbf{h}), \dots\})$$

Despite both widgets “starting” at 0 when considered globally, they are temporally separated in the projections: the prefix entries stop after 4, while the suffix entries are not available before 4.

$$\begin{aligned}
split_{4,1}(W) &= (\{(0, \mathbf{a}), (1, \mathbf{b})\}, & \text{I}) \\
split_{4,3}(W) &= (\{(0, \mathbf{a}), (1, \mathbf{b}), (2, \mathbf{c}), (3, \mathbf{d})\}, & \text{I}) \\
split_{4,4}(W) &= (\text{I}, & \{(0, \mathbf{e})\}) \\
split_{4,6}(W) &= (\text{I}, & \{(0, \mathbf{e}), (1, \mathbf{f}), (2, \mathbf{g})\})
\end{aligned}$$

The *join* function is simply the opposite relation of *split*, so they are inverses of each other, as required:  $join \circ split = \text{id}_{\text{Widget}^t}$ .

### 7.2.5 Semantics of widget operations

We now have the required structure to interpret the syntax and operations associated with widgets. Note that all of the operations are closed terms, so the definitions do not mention the contexts for the sake of brevity.

**Widget types** We interpret the types  $\text{Widget}^t$  and  $\text{Prefix}^t(\tau)$  as follows:

$$\llbracket \Theta \vdash_\ell \text{Widget}^t \rrbracket \triangleq \text{Widget}^{\llbracket \Theta \vdash_{s\ell} : \text{id} \rrbracket} \quad \llbracket \Theta \vdash_\ell \text{Prefix}^t(\tau) \rrbracket \triangleq \text{Prefix}^{\llbracket \Theta \vdash_{s\ell} : \text{id} \rrbracket}(\llbracket \Theta \vdash_s \tau : \text{time} \rrbracket)$$

**Creation and deletion** Creation and deletion corresponds to a relation between the unit and the empty widget (as the empty set of commands).

$$\begin{aligned}
\llbracket \text{create} : \forall \ell : \text{id}. \text{I} \multimap \text{Widget}^t \rrbracket_i &\triangleq \{(\langle \rangle, \emptyset)\} \\
\llbracket \text{delete} : \forall \ell : \text{id}. \text{Widget}^t \multimap \text{I} \rrbracket_i &\triangleq \{(\emptyset, \langle \rangle)\}
\end{aligned}$$

**Modification** Modifying a widget corresponds to adding an entry to the command log. In practice we will only add entries at the beginning of the log (with time step 0) – modifying a widget in the future is possible by splitting it at the required time step, and adding an entry to the beginning of the suffix. We encapsulate this with the following operator, which adds a command at the beginning of the log, but only after removing every existing entry that is incompatible with  $c$ :

$$W \overset{\bowtie}{\cup} c \triangleq \{(t', c') \in W \mid (0, c) \bowtie (t', c')\} \cup (0, c)$$

Then, the interpretation of the modifying commands is simply adding the relevant command to the widget log.

$$\begin{aligned} \llbracket \text{setLabel} : \forall \iota : \text{id}. \text{Widget}^\iota \otimes \text{F String} \multimap \text{Widget}^\iota \rrbracket_i & \\ \triangleq \{((W, \text{lab}), W \overset{\bowtie}{\cup} (\text{setLabel}, \text{lab})) \mid W \in \text{Widget}^\iota \wedge \text{lab} \in \text{String}\} \\ \llbracket \text{setColour} : \forall \iota : \text{id}. \text{Widget}^\iota \otimes \text{F Colour} \multimap \text{Widget}^\iota \rrbracket_i & \\ \triangleq \{((W, \text{col}), W \overset{\bowtie}{\cup} (\text{setColour}, \text{col})) \mid W \in \text{Widget}^\iota \wedge \text{col} \in \text{Colour}\} \end{aligned}$$

**Event listening** The interpretation of the event listening is remarkably straightforward, thanks to the relational semantics: since we don't know when an event occurs, we simply associate a widget with an event at every time step at which it may occur, with all the possible values (e.g. characters) that the event may take. The widget  $W$  also remains unchanged: registering an event listener on a widget doesn't affect its behaviour, only if we actually modify it at the time when the event occurs.

$$\begin{aligned} \llbracket \text{onClick} : \forall \iota : \text{id}. \text{Widget}^\iota \multimap \text{Widget}^\iota \otimes \Diamond \mathbb{I} \rrbracket_i & \\ \triangleq \{(W, (W, (t, \langle \rangle))) \mid W \in \text{Widget}^\iota, t \in \text{Time}\} \\ \llbracket \text{onKeyPress} : \forall \iota : \text{id}. \text{Widget}^\iota \multimap \text{Widget}^\iota \otimes \Diamond (\text{F Char}) \rrbracket_i & \\ \triangleq \{(W, (W, (t, c))) \mid W \in \text{Widget}^\iota, n \in \text{Time}, c \in \text{Char}\} \end{aligned}$$

**Splitting** The splitting and joining functions are directly translated as the morphisms *split* and *join*.

$$\begin{aligned} \llbracket \text{split} : \forall \iota : \text{id}, \tau : \text{time}. \text{Widget}^\iota \multimap \text{Prefix}^\iota(\tau) \otimes (\text{Widget}^\iota @ \tau) \rrbracket_{i, \tau} &\triangleq \text{split}_\tau \\ \llbracket \text{join} : \forall \iota : \text{id}, \tau : \text{time}. \text{Prefix}^\iota(\tau) \otimes (\text{Widget}^\iota @ \tau) \multimap \text{Widget}^\iota \rrbracket_{i, \tau} &\triangleq \text{join}_\tau \end{aligned}$$

## 8 Modelling Quantifiers

On top of the categories  $\text{Set}$  and  $\text{Rel}_{\mathcal{R}}$ , we built a first order logic by the use of a hyperdoctrine.

To handle universal and existential quantification over timesteps and indices in the syntax, we build hyperdoctrines on the categories of contexts. Hyperdoctrines are categories indexed over objects in a context category  $\text{Ctx}$  with additional structure given by substitution and quantification functors.

**Definition 8.1** (Category of contexts). We take the category of contexts, denoted by  $\text{Ctx}$ , to be a Cartesian category that we can interpret our indexing contexts  $\Theta$  in. Objects are denoted by  $\Theta, \Theta'$ , while morphisms will be denoted by  $\delta: \Theta \rightarrow \Theta'$ . Elements of a context  $\Theta$  will usually be denoted by  $s \in \Theta, s' \in \Theta'$ .

Given that we are primarily working in the categories  $\text{Set}$  and  $\text{Rel}_{\mathcal{R}}$ , we will need two hyperdoctrines to support quantification in both. We aim to build a linear-nonlinear hyperdoctrine, ensuring that we lift the adjunction between  $\text{Set}$  and  $\text{Rel}_{\mathcal{R}}$  to their indexed counterparts.

## 8.1 Cartesian hyperdoctrine

**Definition 8.2.** The *Cartesian hyperdoctrine* on the category  $\text{Ctx}$  is the functor

$$\begin{aligned} C: \text{Ctx}^{\text{op}} &\rightarrow \mathcal{CCC} \\ C(\Theta: \text{Ctx}) &\triangleq \text{Set}^{\Theta} \\ C(\delta: \Theta \rightarrow \Theta')(X: \text{Set}^{\Theta'})_s &\triangleq X_{\delta(s)} \\ C(\delta: \Theta \rightarrow \Theta')(f: X \rightarrow Y \in \text{Set}^{\Theta'})_s(x: X_{\delta(s)}) &= f_{\delta(s)}(x) \end{aligned}$$

For  $\delta: \Theta \rightarrow \Theta' \in \text{Ctx}$ , the  $\mathcal{CCC}$ -functor  $C(\delta): \text{Set}^{\Theta'} \rightarrow \text{Set}^{\Theta}$  is the *reindexing functor* denoted by  $\delta^*$ . We may also define  $\delta^*$  as the precomposition functor with  $\delta^*(X) = X \circ \delta$ .

We get the Cartesian closed structure for every  $\text{Set}^{\Theta}$  by the pointwise lifting of operations in  $\text{Set}$ . To get the full hyperdoctrine structure, we also need the quantification functors  $\exists_{\delta}, \forall_{\delta}: \text{Set}^{\Theta} \rightarrow \text{Set}^{\Theta'}$  which are left and right adjoint to  $\delta^*$ , respectively.

### 8.1.1 Cartesian existential quantification

**Definition 8.3.** Given a  $\text{Ctx}$ -morphism  $\delta: \Theta \rightarrow \Theta'$ , the *existential quantification functor along  $\delta$*  is defined as

$$\begin{aligned} \exists_{\delta}: \text{Set}^{\Theta} &\rightarrow \text{Set}^{\Theta'} \\ \exists_{\delta}(X: \text{Set}^{\Theta})_{s'} &\triangleq \sum_{s \in \overleftarrow{\delta}\{s'\}} X_s \\ \exists_{\delta}(f: X \rightarrow Y)_{s'}(s: \overleftarrow{\delta}\{s'\}, x: X_s) &\triangleq (s, f_s(x)) \end{aligned}$$

That is,  $\exists_{\delta}$  sends every indexed set to an indexed sum over all of those indices which are mapped to  $s'$  by  $\delta$ . A witness of the existential object is a dependent pair consisting of an index  $s \in \overleftarrow{\delta}\{s'\}$  and an element  $x \in X_s$ .

To simplify the notation, we adopt a (commonly used) syntactic convention which uses the property that if  $s$  is in the inverse image  $\overleftarrow{\delta}\{s'\}$  of the singleton set  $\{s'\}$  under  $\delta$ , then  $\delta(s) = s'$ . Thus it makes sense to quantify over all of those  $s$  which are mapped to  $s'$  by  $\delta$ , written as  $\sum_{\delta(s)=s'} X_s$ . For example, the action of the existential functor on a morphism  $f: X \rightarrow Y$  will be written as

$$\exists_{\delta}(f: X \rightarrow Y): \sum_{\delta(s)=s'} X_s \rightarrow \sum_{\delta(s)=s'} Y_s$$



$$\exists_\delta(f: X \rightarrow Y)_{s'}(s, x: X_s) \triangleq (s, f_s(x))$$

We can show that for any choice of  $\delta: \Theta \rightarrow \Theta'$ , we have an adjunction  $\exists_\delta \dashv \delta^*$  with the natural transformations

$$\begin{array}{ll} \eta_X: X \rightarrow \delta^*(\exists_\delta(X)) & \epsilon_X: \exists_\delta(\delta^*(X)) \rightarrow X \\ \eta_{X,s}: X_s \rightarrow \sum_{\delta(i)=\delta(s)} X_i & \epsilon_{X,s'}: \sum_{\delta(s)=s'} X_{\delta(s)} \rightarrow X_{s'} \\ \eta_{X,s}(x: X_s) \triangleq (s, x) & \epsilon_{X,s'}(s, x: X_{\delta(s)}) \triangleq x \end{array}$$

The naturality of these transformations and the triangle identities follow from the definitions.

### 8.1.2 Cartesian universal quantification

**Definition 8.4.** Given a Ctx-morphism  $\delta: \Theta \rightarrow \Theta'$ , the *universal quantification functor along  $\delta$*  is defined as

$$\begin{array}{l} \forall_\delta: \mathbf{Set}^\Theta \rightarrow \mathbf{Set}^{\Theta'} \\ \forall_\delta(X: \mathbf{Set}^\Theta)_{s'} \triangleq \prod_{s \in \overleftarrow{\delta}\{s'\}} X_s \\ \forall_\delta(f: X \rightarrow Y)_{s'}(p: \prod_{s \in \overleftarrow{\delta}\{s'\}} X_s)(s \in \overleftarrow{\delta}\{s'\}) \triangleq f_s(p(s)) \end{array}$$

That is,  $\forall_\delta$  sends every indexed set to an indexed product over all of those indices which are mapped to  $s'$  by  $\delta$ . A witness of the universal object is a dependent function mapping an index  $s \in \overleftarrow{\delta}\{s'\}$  to an element  $x \in X_s$ .

Again, we will usually use the notation  $\prod_{\delta(s)=s'}$  instead of  $\prod_{s \in \overleftarrow{\delta}\{s'\}}$  and apply the known equality  $\delta(s) = s'$  implicitly, where needed.

We can show that for any choice of  $\delta: \Theta \rightarrow \Theta'$ , we have an adjunction  $\delta^* \dashv \forall_\delta$  with the natural transformations

$$\begin{array}{ll} \eta_X: X \rightarrow \forall_\delta(\delta^*(X)) & \epsilon_X: \delta^*(\forall_\delta(X)) \rightarrow X \\ \eta_{X,s'}: X_{s'} \rightarrow \prod_{\delta(s)=s'} X_{\delta(s)} & \epsilon_{X,s}: \prod_{\delta(i)=\delta(s)} X_i \rightarrow X_s \\ \eta_{X,s'}(x: X_{s'})(s \in \overleftarrow{\delta}\{s'\}) \triangleq x & \epsilon_{X,s}(p: \prod_{\delta(i)=\delta(s)} X_i) \triangleq p(s) \end{array}$$

As before, naturality and the triangle identities follow definitionally.

### 8.1.3 Frobenius reciprocity

Frobenius reciprocity concerns the interaction between products and existentials. The hyperdoctrine  $C: \mathbf{Ctx}^{\text{op}} \rightarrow \mathcal{CCC}$  satisfies the Frobenius reciprocity condition if, for any  $\delta: \Theta \rightarrow \Theta'$ , the adjunction  $\exists_\delta \dashv \delta^*$  satisfies the property that for any  $X: \mathbf{Set}^\Theta$  and  $Y: \mathbf{Set}^{\Theta'}$  there is a natural isomorphism

$$\phi_{X,Y}: \exists_\delta(X \times \delta^*(Y)) \xrightarrow{\cong} \exists_\delta(X) \times Y \quad \text{in } \mathbf{Set}^{\Theta'}.$$

Given that elements of the existential type are dependent pairs, the condition follows from the (weak) associativity of products, and the usual equality  $\delta(s) = s'$  for  $s \in \overleftarrow{\delta}\{s'\}$ :

$$\phi_{X,Y,s'}: (\sum_{\delta(s)=s'} (X_s \times Y_{\delta(s)})) \xrightarrow{\cong} (\sum_{\delta(s)=s'} X_s) \times Y_{s'} \quad \text{in } \mathbf{Set}$$

$$\begin{aligned}\phi_{X,Y,s'}(s: \overleftarrow{\delta} \{s'\}, (x: X_s, y: Y_{\delta(s)})) &= ((s, x), y) \\ \phi_{X,Y,s'}^{-1}((s: \overleftarrow{\delta} \{s'\}, x: X_s), y: Y_{s'}) &= (s, (x, y))\end{aligned}$$

Naturality and inverse laws follow by definition.

#### 8.1.4 Beck–Chevalley condition

The Beck–Chevalley condition concerns the commutativity of substitution and quantification for different context morphisms. In general, given a pullback square in  $\mathbf{Ctx}$  on the left:

$$\begin{array}{ccc} \Xi & \xrightarrow{\sigma} & \Xi' \\ \rho \downarrow & & \downarrow \mu \\ \Theta & \xrightarrow{\delta} & \Theta' \end{array} \quad \begin{array}{ccc} \mathbf{Set}^\Xi & \xleftarrow{\sigma^*} & \mathbf{Set}^{\Xi'} \\ F_\rho \downarrow & & \downarrow F_\mu \\ \mathbf{Set}^\Theta & \xleftarrow{\delta^*} & \mathbf{Set}^{\Theta'} \end{array}$$

a family of functors  $(F_\delta: \mathbf{Set}^{\Theta'} \rightarrow \mathbf{Set}^\Theta)_{\delta: \Theta \rightarrow \Theta'}$  satisfies the Beck–Chevalley condition if the right square in  $\mathcal{CCC}$  commutes (usually up to natural isomorphism). That is, if  $\mu \circ \sigma = \delta \circ \rho$  then we have a natural isomorphism  $F_\rho \circ \sigma^* \cong \delta^* \circ F_\mu$  in  $\mathcal{CCC}$ . We have to establish this property for both  $\exists\_$  and  $\forall\_$ .

**Existential** Assume  $\mu \circ \sigma = \delta \circ \rho$  as above. We are required to give a natural isomorphism  $\tau: \exists_\rho \circ \sigma^* \xrightarrow{\cong} \delta^* \circ \exists_\mu$  between  $\mathcal{CCC}$  functors. Its components at an  $X: \mathbf{Set}^{\Xi'}$  and index  $s: \Theta$  are:

$$\begin{aligned}\tau_{X,s}: \exists_\rho(\sigma^*(X))_s &\xrightarrow{\cong} \delta^*(\exists_\mu(X))_s \\ &: \sum_{\rho(i)=s} X_{\sigma(i)} \xrightarrow{\cong} \sum_{\mu(j)=\delta(s)} X_j \\ \tau_{X,s}(i: \overleftarrow{\rho} \{s\}, x: X_{\sigma(i)}) &\triangleq (\sigma(i), x) \\ \tau_{X,s}^{-1}(j: \overleftarrow{\mu} \{\delta(s)\}, x: X_j) &\triangleq (\mathbf{pb}(j, s), x)\end{aligned}$$

For the forward direction, we need to prove that if  $i \in \overleftarrow{\rho} \{s\}$  then  $\sigma(i) \in \overleftarrow{\mu} \{\delta(s)\}$ . As before, we have that  $\rho(i) = s$ , so we can show  $\sigma(i) \in \overleftarrow{\mu} \{\delta(\rho(i))\}$ . But by the commutativity of the pullback square,  $\delta(\rho(i)) = \mu(\sigma(i))$ , and  $\sigma(i)$  is indeed an element of  $\overleftarrow{\mu} \{\mu(\sigma(i))\}$ .

For the backward direction, we make use of the index  $\mathbf{pb}(j, s) \in \Xi$  which is the unique element of  $\Xi$  that we get from the universal property of the pullback square in  $\mathbf{Ctx}$  on the terminal object  $\mathbf{1}$  and the global element morphisms  $\hat{j}: \mathbf{1} \rightarrow \Xi$  and  $\hat{s}: \mathbf{1} \rightarrow \Theta$  associated with elements  $j \in \Xi'$  and  $s \in \Theta$ . More precisely,  $\mathbf{pb}(j, s)$  is the element of  $\Xi$  that the unique global element arrow  $h$  selects in the following pullback diagram:

$$\begin{array}{ccccc} & & \hat{j} & & \\ & & \curvearrowright & & \\ \mathbf{1} & \xrightarrow{\quad h \quad} & \Xi & \xrightarrow{\sigma} & \Xi' \\ & \searrow \hat{s} & \rho \downarrow & & \downarrow \mu \\ & & \Theta & \xrightarrow{\delta} & \Theta' \end{array}$$

By the universal property of pullbacks, we have that  $\rho(\mathbf{pb}(j, s)) = s$  and  $\sigma(\mathbf{pb}(j, s)) = j$ . Thus, we have that  $\mathbf{pb}(j, s) \in \overleftarrow{p}\{s\}$  (first element of the pair), and if  $x \in X_j$  then  $x \in X_{\sigma(\mathbf{pb}(j, s))}$  (second element of the pair). The inverse proofs make use of the above universal properties of pullbacks, as well as the uniqueness property  $\mathbf{pb}(\sigma(i), \rho(i)) = i$ .

**Universal** Assume  $\mu \circ \sigma = \delta \circ \rho$  as above. We are required to give a natural isomorphism  $\gamma: \forall_\rho \circ \sigma^* \xrightarrow{\cong} \delta^* \circ \forall_\mu$  between  $\mathcal{CCC}$  functors. Its components at an  $X: \mathbf{Set}^{\Xi'}$  and index  $s: \Theta$  are:

$$\begin{aligned} \gamma_{X,s}: \forall_\rho(\sigma^*(X))_s &\xrightarrow{\cong} \delta^*(\forall_\mu(X))_s \\ &: \prod_{\rho(i)=s} X_{\sigma(i)} \xrightarrow{\cong} \prod_{\mu(j)=\delta(s)} X_j \\ \gamma_{X,s}(p: \prod_{\rho(i)=s} X_{\sigma(i)})(j: \overleftarrow{\mu}\{\delta(s)\}) &= p(\mathbf{pb}(j, s)) \\ \gamma_{X,s}^{-1}(q: \prod_{\mu(j)=\delta(s)} X_j)(i: \overleftarrow{\rho}\{s\}) &= q(\sigma(i)) \end{aligned}$$

For the forward direction, we need to show that  $\rho(\mathbf{pb}(j, s)) = s$  and  $p(\mathbf{pb}(j, s)) \in X_j$ . Both follow from the universal property of the element  $\mathbf{pb}(j, s)$ . For the backward direction, we need to show that  $\mu(\sigma(i)) = \delta(s)$  and  $q(\sigma(i)) \in X_{\sigma(i)}$ . The first follows from the equality  $\rho(i) = s$  and the commutativity of the pullback square, while the second follows from the type of  $q$ . Again, we can prove that  $\gamma$  and  $\gamma^{-1}$  are inverses using the existence and uniqueness properties of pullbacks.

The existence of the adjoint triple  $\exists_\delta \dashv \delta^* \dashv \forall_\delta$  satisfying Frobenius reciprocity and the Beck-Chevalley condition makes the functor  $C: \mathbf{Ctx}^{\text{op}} \rightarrow \mathcal{CCC}$  a Cartesian hyperdoctrine, as required.

## 8.2 Linear hyperdoctrine

**Definition 8.5.** The *linear hyperdoctrine* on the category  $\mathbf{Ctx}$  is the functor

$$\begin{aligned} L: \mathbf{Ctx}^{\text{op}} &\rightarrow \mathcal{SMCC} \\ L(\Theta: \mathbf{Ctx}) &\triangleq \mathbf{Rel}_{\mathcal{R}}^\Theta \\ L(\delta: \Theta \rightarrow \Theta')(A: \mathbf{Rel}_{\mathcal{R}}^{\Theta'})_{s,k} &\triangleq A_{\delta(s),k} \\ L(\delta: \Theta \rightarrow \Theta')(r: A \rightarrow_{\mathcal{R}} B \in \mathbf{Rel}_{\mathcal{R}}^{\Theta'})_{s,k}(a: A_{\delta(s),k}, b: B_{\delta(s),k}) &\triangleq r_{\delta(s),k}(a, b) \end{aligned}$$

For  $\delta: \Theta \rightarrow \Theta' \in \mathbf{Ctx}$ , the  $\mathcal{SMCC}$ -functor  $L(\delta): \mathbf{Rel}_{\mathcal{R}}^{\Theta'} \rightarrow \mathbf{Rel}_{\mathcal{R}}^\Theta$  is the *linear reindexing functor* denoted by  $\delta^+$ . We may also define  $\delta^+$  as the precomposition functor with  $\delta^+(A) = A \circ \delta$ .

The symmetric monoidal structure on any  $\mathbf{Rel}_{\mathcal{R}}^\Theta$  follows from the  $\mathcal{SMCC}$  structure on  $\mathbf{Rel}_{\mathcal{R}}$  lifted pointwise. To get the full hyperdoctrine structure, we also need the quantification functors  $\hat{\exists}_\delta, \hat{\forall}_\delta: \mathbf{Rel}_{\mathcal{R}}^\Theta \rightarrow \mathbf{Rel}_{\mathcal{R}}^{\Theta'}$  which are left and right adjoint to  $\delta^+$ , respectively.

### 8.2.1 Linear existential quantification

**Definition 8.6.** Given a  $\mathbf{Ctx}$ -morphism  $\delta: \Theta \rightarrow \Theta'$ , the *linear existential quantification functor along  $\delta$*  is defined as

$$\hat{\exists}_\delta: \mathbf{Rel}_{\mathcal{R}}^\Theta \rightarrow \mathbf{Rel}_{\mathcal{R}}^{\Theta'}$$

$$\begin{aligned}\hat{\exists}_\delta(A : \mathbf{Rel}_{\mathcal{R}}^\Theta)_{s',k} &\triangleq \sum_{\delta(s)=s'} A_{s,k} \\ \hat{\exists}_\delta(r : A \multimap_{\mathcal{R}} B)_{s',k}((i : \overleftarrow{\delta}\{s'\}, a : A_{s,k}), (j : \overleftarrow{\delta}\{s'\}, b : B_{s,k})) &\triangleq i = j \wedge r_{i,k}(a, b)\end{aligned}$$

We can show that for any choice of  $\delta : \Theta \rightarrow \Theta'$ , we have an adjunction  $\hat{\exists}_\delta \dashv \delta^*$  with the natural transformations

$$\begin{aligned}\eta_A : A \rightarrow \delta^+(\hat{\exists}_\delta(A)) &\in \mathbf{Rel}_{\mathcal{R}}^\Theta & \epsilon_A : \hat{\exists}_\delta(\delta^+(A)) &\rightarrow A \in \mathbf{Rel}_{\mathcal{R}}^{\Theta'} \\ \eta_{A,s,k} : A_{s,k} \times \sum_{\delta(i)=\delta(s)} A_{i,k} &\rightarrow \Omega_k & \epsilon_{A,s',k} : \sum_{\delta(s)=s'} A_{\delta(s),k} \times A_{s',k} &\rightarrow \Omega_k \\ \eta_{A,s}(a : A_{s,k}, (i : \overleftarrow{\delta}\{\delta(s)\}, a' : A_{i,k})) &\triangleq s = i \wedge a = a' & \epsilon_{A,s',k}((s, x : A_{\delta(s),k}), a' : A_{s,k}) &\triangleq a = a'\end{aligned}$$

The naturality of these transformations and the triangle identities follow from the definitions.

### 8.2.2 Linear universal quantification

**Definition 8.7.** Given a Ctx-morphism  $\delta : \Theta \rightarrow \Theta'$ , the *linear universal quantification functor along  $\delta$*  is defined as

$$\begin{aligned}\hat{\forall}_\delta : \mathbf{Rel}_{\mathcal{R}}^\Theta &\rightarrow \mathbf{Rel}_{\mathcal{R}}^{\Theta'} \\ \hat{\forall}_\delta(A : \mathbf{Rel}_{\mathcal{R}}^\Theta)_{s',k} &\triangleq \prod_{\delta(s)=s'} A_{s,k} \\ \hat{\forall}_\delta(r : A \multimap_{\mathcal{R}} B)_{s',k}(p : \prod_{\delta(i)=s'} A_{i,k}, q : \prod_{\delta(j)=s'} B_{j,k}) &\triangleq \forall s \in \overleftarrow{\delta}\{s'\}. r_{s,k}(p(s), q(s))\end{aligned}$$

That is,  $\hat{\forall}_\delta$  maps a relation  $r : A \multimap_{\mathcal{R}} B$  to a relation on two dependent functions which holds if the two functions are extensionally related (i.e. for every input, the outputs of the functions are related by  $r$ ).

We can show that for any choice of  $\delta : \Theta \rightarrow \Theta'$ , we have an adjunction  $\delta^+ \dashv \hat{\forall}_\delta$  with the natural transformations

$$\begin{aligned}\eta_A : A \rightarrow \delta^+(\hat{\forall}_\delta(A)) &\in \mathbf{Rel}_{\mathcal{R}}^{\Theta'} & \epsilon_A : \delta^+(\hat{\forall}_\delta(A)) &\rightarrow A \in \mathbf{Rel}_{\mathcal{R}}^\Theta \\ \eta_{A,s',k} : A_{s',k} \times (\prod_{\delta(s)=s'} A_{\delta(s),k}) &\rightarrow \Omega_k & \epsilon_{A,s,k} : (\prod_{\delta(i)=\delta(s)} A_{i,k}) \times A_{s,k} &\rightarrow \Omega_k \\ \eta_{A,s',k}(a : A_{s',k}, p : \prod_{\delta(s)=s'} A_{\delta(s),k}) &\triangleq & \epsilon_{A,s,k}(p : \prod_{\delta(i)=\delta(s)} A_{i,k}, a : A_{s,k}) &\triangleq p(s) = a \\ & & \forall i \in \overleftarrow{\delta}\{s'\}. p(i) = a &\end{aligned}$$

As before, naturality and the triangle identities follow definitionally.

### 8.2.3 Frobenius reciprocity

The hyperdoctrine  $L : \mathbf{Ctx}^{\text{op}} \rightarrow \mathcal{SMCC}$  satisfies the Frobenius reciprocity condition if, for any  $\delta : \Theta \rightarrow \Theta'$ , the adjunction  $\hat{\exists}_\delta \dashv \delta^+$  satisfies the property that for any  $A : \mathbf{Rel}_{\mathcal{R}}^\Theta$  and  $B : \mathbf{Rel}_{\mathcal{R}}^{\Theta'}$  there is a natural isomorphism

$$\hat{\phi}_{A,B} : \hat{\exists}_\delta(A \times \delta^+(B)) \xrightarrow{\cong} \hat{\exists}_\delta(A) \times A \quad \text{in } \mathbf{Rel}_{\mathcal{R}}^{\Theta'}.$$

Given that elements of the existential type are dependent pairs, the condition follows from the (weak) associativity of products, and the usual equality  $\delta(s) = s'$  for  $s \in \overleftarrow{\delta}\{s'\}$ :

$$\begin{aligned}\hat{\phi}_{X,Y,s',k}: (\sum_{\delta(s)=s'} (A_{s,k} \times B_{\delta(s),k})) &\xrightarrow{\cong} (\sum_{\delta(s)=s'} A_{s,k}) \times B_{s',k} \quad \text{in } \text{Rel}_{\mathcal{R}} \\ \hat{\phi}_{X,Y,s',k}((i, (a: A_{i,k}, b: B_{\delta(i),k})), ((j, a': A_j), b': B_{s'})) &\triangleq i = j \wedge a = a' \wedge b = b' \\ \hat{\phi}_{X,Y,s',k}^{-1}(((j, a': A_j), b': B_{s'}), (i, (a: A_{i,k}, b: B_{\delta(i),k}))) &\triangleq i = j \wedge a = a' \wedge b = b'\end{aligned}$$

Naturality and inverse laws follow by definition.

#### 8.2.4 Beck–Chevalley condition

Assume we have the pullback square in  $\text{Ctx}$ :

$$\begin{array}{ccc} \Xi & \xrightarrow{\sigma} & \Xi' \\ \rho \downarrow & & \downarrow \mu \\ \Theta & \xrightarrow{\delta} & \Theta' \end{array}$$

A family of functors  $(F_\delta: \text{Rel}_{\mathcal{R}}^{\Theta'} \rightarrow \text{Rel}_{\mathcal{R}}^{\Theta})_{\delta: \Theta \rightarrow \Theta'}$  satisfies the Beck–Chevalley condition if the following square in  $\mathcal{SMCC}$  commutes (usually up to natural isomorphism):

$$\begin{array}{ccc} \text{Rel}_{\mathcal{R}}^{\Xi} & \xleftarrow{\sigma^*} & \text{Rel}_{\mathcal{R}}^{\Xi'} \\ F_\rho \downarrow & & \downarrow F_\mu \\ \text{Rel}_{\mathcal{R}}^{\Theta} & \xleftarrow{\delta^*} & \text{Rel}_{\mathcal{R}}^{\Theta'} \end{array}$$

That is, if  $\mu \circ \sigma = \delta \circ \rho$  then we have a natural isomorphism  $F_\rho \circ \sigma^* \cong \delta^* \circ F_\mu$  in  $\mathcal{SMCC}$ . We have to establish this property for both  $\hat{\Xi}_-$  and  $\hat{\mathbb{V}}_-$ .

**Existential** We are required to give a natural isomorphism  $\hat{\tau}: \hat{\Xi}_\rho \circ \sigma^+ \xrightarrow{\cong} \delta^+ \circ \hat{\Xi}_\mu$  between  $\mathcal{SMCC}$  functors. Its components at an  $A: \text{Rel}_{\mathcal{R}}^{\Xi'}$  and index  $s: \Theta$  at time  $k \in \mathbb{N}_\top$  are:

$$\begin{aligned}\hat{\tau}_{A,s,k}: \hat{\Xi}_\rho(\sigma^+(A))_{s,k} &\xrightarrow{\cong} \delta^+(\hat{\Xi}_\mu(A))_{s,k} = \sum_{\rho(i)=s} A_{\sigma(i),k} \xrightarrow{\cong} \sum_{\mu(j)=\delta(s)} A_{j,k} \\ \hat{\tau}_{A,s,k}((i: \overleftarrow{\rho}\{s\}, a: A_{\sigma(i),k}), (j: \overleftarrow{\mu}\{\delta(s)\}, a': A_{j,k})) &\triangleq \sigma(i) = j \wedge a = a' \\ \hat{\tau}_{A,s,k}^{-1}((j: \overleftarrow{\mu}\{\delta(s)\}, a \in A_{j,k}), (i: \overleftarrow{\rho}\{s\}, a': A_{\sigma(i),k})) &\triangleq \text{pb}(j, s) = i \wedge a = a'\end{aligned}$$

The proofs that the “types” match up are the same as for the Cartesian version, and the inverse proofs use the universal properties of pullbacks. Note that even though it seems like the definition for  $\tau$  and  $\tau^{-1}$  could be the same (as we don’t need to “invent” an element of  $\Xi$ , like we did in the Cartesian case), we need the extra condition on pullbacks to make the inverse proofs work – without it, we would get stuck at  $\sigma(i) = \sigma(i')$  when proving that  $i = i'$ .

**Universal** We are required to give a natural isomorphism  $\hat{\gamma}: \hat{\nabla}_\rho \circ \sigma^+ \xrightarrow{\cong} \delta^+ \circ \hat{\nabla}_\mu$  between  $\mathcal{SMCC}$  functors. Its components at an  $A: \text{Rel}_{\mathcal{R}}^{\Xi'}$  and index  $s: \Theta$  at time  $k \in \mathbb{N}_+$  are:

$$\begin{aligned} \hat{\gamma}_{A,s,k}: \hat{\nabla}_\rho(\sigma^+(A))_{s,k} &\xrightarrow{\cong} \delta^+(\hat{\nabla}_\mu(A))_{s,k} = \prod_{\rho(i)=s} A_{\sigma(i),k} \xrightarrow{\cong} \prod_{\mu(j)=\delta(s)} A_{j,k} \\ \hat{\gamma}_{A,s,k}(p: \prod_{\rho(i)=s} A_{\sigma(i),k}, q: \prod_{\mu(j)=\delta(s)} A_{j,k}) &\triangleq \forall j \in \overleftarrow{\mu}\{\delta(s)\}. p(\text{pb}(j, s)) = q(j) \\ \hat{\gamma}_{A,s,k}^{-1}(q: \prod_{\mu(j)=\delta(s)} A_{j,k}, p: \prod_{\rho(i)=s} A_{\sigma(i),k}) &\triangleq \forall i \in \overleftarrow{\rho}\{s\}. q(\sigma(i)) \triangleq p(i) \end{aligned}$$

Again, the proofs that the definition is well-formed and that the inverse laws hold follow from the existence and uniqueness properties of the pullback.

The existence of the adjoint triple  $\hat{\exists}_\delta \dashv \delta^+ \dashv \hat{\nabla}_\delta$  satisfying Frobenius reciprocity and the Beck–Chevalley condition makes the functor  $L: \text{Ctx}^{\text{op}} \rightarrow \mathcal{SMCC}$  a linear hyperdoctrine, as required.

### 8.3 Linear-nonlinear hyperdoctrine

In the previous two sections we described the individual hyperdoctrines for Cartesian and linear terms-in-context – however, we have not said anything about how the indexed Cartesian closed and symmetric monoidal closed categories  $\text{Set}^\Theta$  and  $\text{Rel}_{\mathcal{R}}^\Theta$  relate for a given  $\Theta \in \text{Ctx}$ . Given that we have a monoidal adjunction  $F \dashv G: \text{Set} \rightleftarrows \text{Rel}_{\mathcal{R}}$ , we expect there to be a fiberwise monoidal adjunction for every choice of index  $\Theta$  as well. This section formalises the requirements for this.

#### 8.3.1 Category of linear-nonlinear adjunctions

**Definition 8.8.** The category of *linear-nonlinear adjunctions*  $LNL$  has:

**Objects** Tuples  $(\mathcal{C}, \mathcal{L}, U: \mathcal{C} \rightarrow \mathcal{L}, R: \mathcal{L} \rightarrow \mathcal{C})$  forming a linear-nonlinear adjunction  $U \dashv R: \mathcal{C} \rightleftarrows \mathcal{L}$

**Morphisms** Arrows  $(\mathcal{C}, \mathcal{L}, U, R) \rightarrow (\mathcal{C}', \mathcal{L}', U', R')$  are tuples  $(K: \mathcal{C} \rightarrow \mathcal{C}', L: \mathcal{L} \rightarrow \mathcal{L}')$  such that:

- $LU = U'K$  and  $KR = R'L$ , i.e. the following square commutes in both directions:

$$\begin{array}{ccc} \mathcal{C} & \xrightleftharpoons[U]{U} & \mathcal{L} \\ K \downarrow & & \downarrow L \\ \mathcal{C}' & \xrightleftharpoons[U']{U'} & \mathcal{L}' \\ & \xleftarrow{R'} & \end{array}$$

- $K$  is a Cartesian functor
- $L$  is a strong symmetric monoidal closed functor
- $K\eta = \eta'K$  or equivalently  $\epsilon'L = L\epsilon$ , where  $(\eta, \epsilon)$  and  $(\eta', \epsilon')$  are the unit and counit of the adjunctions  $U \dashv R$  and  $U' \dashv R'$ , respectively.

We can generate a subcategory of  $LNL$  from our base adjunction  $F \dashv G: \text{Set} \rightleftarrows \text{Rel}_{\mathcal{R}}$  by indexing everything with an object of  $\text{Ctx}$ . In the previous sections we described the indexed categories  $\text{Set}^\Theta$  and  $\text{Rel}_{\mathcal{R}}^\Theta$  for  $\Theta \in \text{Ctx}$ , and below we give the definition of the indexed adjunction  $F^\Theta \dashv G^\Theta$ .

**Definition 8.9.** Given a  $\Theta \in \text{Ctx}$ , the functor  $F^\Theta: \text{Set}^\Theta \rightarrow \text{Rel}_{\mathcal{R}}^\Theta$  is the functor  $F = I \circ \Delta$  indexed by  $\Theta$ . Explicitly:

$$\begin{aligned} F^\Theta: \text{Set}^\Theta &\rightarrow \text{Rel}_{\mathcal{R}}^\Theta \\ F^\Theta(X: \text{Set}^\Theta)_{s,k} &\triangleq X_s \\ F^\Theta(f: X \rightarrow Y)_{s,k}(x: X_s, y: Y_s) &\triangleq f_s(x) = y \end{aligned}$$

**Definition 8.10.** Given a  $\Theta \in \text{Ctx}$ , the functor  $G^\Theta: \text{Rel}_{\mathcal{R}}^\Theta \rightarrow \text{Set}^\Theta$  is the functor  $G = \lim \circ P$  indexed by  $\Theta$ . Explicitly:

$$\begin{aligned} G^\Theta: \text{Rel}_{\mathcal{R}}^\Theta &\rightarrow \text{Set}^\Theta \\ G^\Theta(A: \text{Rel}_{\mathcal{R}}^\Theta)_s &\triangleq \mathcal{R}(A_s, \Omega) \\ G^\Theta(r: A \rightarrow_{\mathcal{R}} B)_s(f: A_s \rightarrow_{\mathcal{R}} \Omega)(b: B) &\triangleq \exists a \in A_s. f(a) \wedge r_s(a, b) \end{aligned}$$

For any choice of  $\Theta \in \text{Ctx}$ , we can show that  $F^\Theta$  is the left adjoint to  $G^\Theta$  with the natural transformations:

$$\begin{aligned} \eta_X^\Theta: X \rightarrow G^\Theta(F^\Theta(X)) &\in \text{Set}^\Theta & \epsilon_A^\Theta: F^\Theta(G^\Theta(A)) &\rightarrow_{\mathcal{R}} A \in \text{Rel}_{\mathcal{R}}^\Theta \\ \eta_{X,s}^\Theta: X_s \rightarrow \mathcal{R}(\Delta(X_s), \Omega) &\in \text{Set} & \epsilon_{A,s}^\Theta: I(\Delta(\mathcal{R}(A_s, \Omega))) &\rightarrow_{\mathcal{R}} A_s \in \text{Rel}_{\mathcal{R}} \\ \eta_{X,s}^\Theta(x: X_s)_{\top}(x': X_s) &\triangleq \begin{cases} \text{inr } * & \text{if } x = x' \\ \text{inl } \emptyset & \text{otherwise} \end{cases} & \epsilon_{A,s,k}^\Theta(f: A_s \rightarrow_{\mathcal{R}} \Theta, a: A_{s,k}) &\triangleq f_k(a) \end{aligned}$$

Naturality and the triangle identities follow from the definitions. Moreover,  $F^\Theta$  is strong monoidal and  $G^\Theta$  is monoidal (by pointwise indexing), so we get a monoidal adjunction.

Thus, for any choice of  $\Theta \in \text{Ctx}$ , we have an object  $(\text{Set}^\Theta, \text{Rel}_{\mathcal{R}}^\Theta, F^\Theta, G^\Theta)$  of the category  $LNL$ . Given another context  $\Theta'$  and a context morphism  $\delta: \Theta \rightarrow \Theta'$ , a canonical functor  $\text{Set}^{\Theta'} \rightarrow \text{Set}^\Theta$  is the reindexing functor  $\delta^*$  (similarly with the linear category and  $\delta^+$ ). We need to show that the pair  $(\delta^*, \delta^+)$  is an  $LNL$ -morphism  $(\text{Set}^{\Theta'}, \text{Rel}_{\mathcal{R}}^{\Theta'}, F^{\Theta'}, G^{\Theta'}) \rightarrow (\text{Set}^\Theta, \text{Rel}_{\mathcal{R}}^\Theta, F^\Theta, G^\Theta)$ .

- Both  $\delta^+ \circ F^{\Theta'} = F^\Theta \circ \delta^* \in \text{Rel}_{\mathcal{R}}^\Theta$  and  $\delta^* \circ G^{\Theta'} = G^\Theta \circ \delta^+ \in \text{Set}^\Theta$  hold definitionally.
- As indexing of products, exponentials, terminal objects, etc. in indexed CC and SMC categories is defined by pointwise indexing (e.g.  $(X \times_{\text{Set}^\Theta} Y)_s \triangleq X_s \times_{\text{Set}} Y_s$ ), both reindexing functors preserve the relevant structure. For example, the multiplication natural transformation

$$\mu_{X,Y}: \delta^*(X) \times_{\text{Set}^\Theta} \delta^*(Y) \rightarrow \delta^*(X \times_{\text{Set}^{\Theta'}} Y)$$

at index  $s \in \Theta$  has type  $X_{\delta(s)} \times_{\text{Set}^\Theta} Y_{\delta(s)} \rightarrow (X \times_{\text{Set}^{\Theta'}} Y)_{\delta(s)}$ , but  $(X \times_{\text{Set}^{\Theta'}} Y)_{\delta(s)} = X_{\delta(s)} \times_{\text{Set}} Y_{\delta(s)}$  so  $\mu_{X,Y}$  can just be the identity natural transformation. Hence,  $\delta^*$  is Cartesian closed and  $\delta^+$  is symmetric monoidal closed.

- We show that  $\epsilon^\Theta \delta^+ = \delta^+ \epsilon^{\Theta'}$  in  $\text{Rel}_{\mathcal{R}}^\Theta$ . Let  $A$  be an object of  $\text{Rel}_{\mathcal{R}}^{\Theta'}$ . At index  $s \in \Theta$  and timestep  $k$ , we have:

$$(\epsilon^\Theta \delta^+)_A: F^\Theta(G^\Theta(\delta^+(A))) \rightarrow_{\mathcal{R}} \delta^+(A) \in \text{Rel}_{\mathcal{R}}^\Theta$$

$$\begin{aligned}\epsilon_{\delta^+(A),s,k}^\Theta &: \mathcal{R}(A_{\delta(s)}, \Omega) \times A_{\delta(s),k} \rightarrow \Omega_k \in \mathbf{Set} \\ \epsilon_{\delta^+(A),s,k}^\Theta(f: A_{\delta(s)}, a: A_{\delta(s),k}) &= f_k(a)\end{aligned}$$

On the other hand,  $\delta^+(\epsilon_A^\Theta)_{s,k} = \epsilon_{A,\delta(s),k}^\Theta$ , and  $\epsilon_{A,\delta(s),k}^\Theta(f: A_{\delta(s)} \rightarrow \Omega, a: A_{\delta(s),k}) = f_k(a)$ , so we have the required equality.

Thus, we can conclude that for any  $\delta: \Theta \rightarrow \Theta' \in \mathbf{Ctx}$ ,  $(\delta^*, \delta^+)$  is a morphism between  $(\mathbf{Set}^{\Theta'}, \mathbf{Rel}_{\mathcal{R}}^{\Theta'}, F^{\Theta'}, G^{\Theta'})$  and  $(\mathbf{Set}^\Theta, \mathbf{Rel}_{\mathcal{R}}^\Theta, F^\Theta, G^\Theta)$  in  $LNL$ , as required.

### 8.3.2 $LNL$ -hyperdoctrine

We have the sufficient structure needed to define a hyperdoctrine via  $LNL$ .

**Definition 8.11.** The  *$LNL$ -hyperdoctrine* on the category  $\mathbf{Ctx}$  is the functor

$$\begin{aligned}T: \mathbf{Ctx}^{\text{op}} &\rightarrow LNL \\ T(\Theta: \mathbf{Ctx}) &\triangleq F^\Theta \dashv G^\Theta: \mathbf{Set}^\Theta \rightleftarrows \mathbf{Rel}_{\mathcal{R}}^\Theta \\ T(\delta: \Theta \rightarrow \Theta') &\triangleq (\delta^*, \delta^+): F^{\Theta'} \dashv G^{\Theta'} \rightarrow F^\Theta \dashv G^\Theta\end{aligned}$$

## 8.4 Weakening hyperdoctrine

In the categorical semantics the only context transformation we will encounter is weakening, i.e. extending the context by an extra variable – it therefore makes sense to specialise the discussion above to this particular case. Since hyperdoctrines on  $\mathbf{Ctx}$  are functors from  $\mathbf{Ctx}^{\text{op}}$ , the  $\mathbf{Ctx}$ -morphism we are considering is actually the first projection  $\pi_1^{\Theta,\sigma}: \Theta \times \sigma \rightarrow \Theta$ , which is mapped to  $(\pi_1^{\Theta,\sigma})^*: \mathbf{Set}^\Theta \rightarrow \mathbf{Set}^{\Theta \times \sigma}$  by the Cartesian hyperdoctrine. We will write  $\text{wk}_{\Theta,\sigma}$  for  $(\pi_1^{\Theta,\sigma})^*$ , or just  $\text{wk}_\sigma$  when the context  $\Theta$  is clear; similarly  $\hat{\text{wk}}_{\Theta,\sigma}$  is used for the linear weakening map  $(\pi_1^{\Theta,\sigma})^+: \mathbf{Rel}_{\mathcal{R}}^\Theta \rightarrow \mathbf{Rel}_{\mathcal{R}}^{\Theta \times \sigma}$ .

**Cartesian weakening hyperdoctrine** We now give explicit, derived definitions of the objects and morphisms associated with our hyperdoctrines. The weakening functor simply ignores one of the indices:

$$\begin{aligned}\text{wk}_\sigma(X: \mathbf{Set}^\Theta)_{(s,i) \in \Theta \times \sigma} &\triangleq X_s \\ \text{wk}_\sigma(f: X \rightarrow Y \in \mathbf{Set}^\Theta)_{(s,i)}(x: X_s) &= f_s(x)\end{aligned}$$

The existential quantification along the first projection has type  $\exists_{\pi_1}: \mathbf{Set}^{\Theta \times \sigma} \rightarrow \mathbf{Set}^\Theta$ ; by definition, on an object  $X: \mathbf{Set}^{\Theta \times \sigma}$  at index  $s \in \Theta$ , it is defined as the dependent sum

$$\sum_{(t,j) \in \pi_1^{-1}\{s\}} X_{(t,j)} = \sum_{\pi_1(t,j)=s} X_{(t,j)}$$

Quantifying over all pairs  $(t,j) \in \Theta \times \sigma$  where the first projection is equal to  $s$  is the same as quantifying over all  $j \in \sigma$  and indexing  $X$  by  $(s,j)$ . Thus, we can write this dependent sum as

$$\exists_{\pi_1^{\Theta \times \sigma}}(X)_s = \sum_{j \in \sigma} X_{(s,j)}$$



We will write  $\exists_{\Theta, \sigma}$  for  $\exists_{\pi_1^{\Theta \times \sigma}}$ , or  $\exists_{\sigma}$  if  $\Theta$  is clear from the context.

$$\begin{aligned}
\exists_{\sigma} &: \mathbf{Set}^{\Theta \times \sigma} \rightarrow \mathbf{Set}^{\Theta} \\
\exists_{\sigma}(X : \mathbf{Set}^{\Theta \times \sigma})_s &\triangleq \sum_{j \in \sigma} X_{(s, j)} \\
\exists_{\sigma}(f : X \rightarrow Y)_s (j \in \sigma, x \in X_{(s, j)}) &\triangleq (j, f_{(s, j)}(x)) \\
\eta_X : X &\rightarrow \mathbf{wk}_{\sigma}(\exists_{\sigma}(X)) & \epsilon_X : \exists_{\sigma}(\mathbf{wk}_{\sigma}(X)) &\rightarrow X \\
\eta_{X, (s, i)} : X_{(s, i)} &\rightarrow \sum_{j \in \sigma} X_{(s, j)} & \epsilon_{X, s} : (\sum_{j \in \sigma} X_s) &\rightarrow X_s \\
\eta_{X, (s, i)}(x : X_{(s, i)}) &\triangleq (s, x) & \epsilon_{X, s}(j, x : X_s) &\triangleq x
\end{aligned}$$

We can perform similar simplifications for universal quantification: the dependent product will range over the second element of the index pair.

$$\begin{aligned}
\forall_{\sigma} &: \mathbf{Set}^{\Theta \times \sigma} \rightarrow \mathbf{Set}^{\Theta} \\
\forall_{\sigma}(X : \mathbf{Set}^{\Theta \times \sigma})_s &\triangleq \prod_{j \in \sigma} X_{(s, j)} \\
\forall_{\sigma}(f : X \rightarrow Y)_s (p : \prod_{j \in \sigma} X_{(s, j)}) (j : \sigma) &\triangleq f_{(s, j)}(p(j)) \\
\eta_X : X &\rightarrow \forall_{\sigma}(\mathbf{wk}_{\sigma}(X)) & \epsilon_X : \mathbf{wk}_{\sigma}(\forall_{\sigma}(X)) &\rightarrow X \\
\eta_{X, s} : X_s &\rightarrow \prod_{j \in \sigma} X_{(s, j)} & \epsilon_{X, (s, i)} : (\prod_{j \in \sigma} X_{(s, j)}) &\rightarrow X_{(s, i)} \\
\eta_{X, s}(x : X_s) (j \in \sigma) &\triangleq x & \epsilon_{X, (s, i)}(p : \prod_{j \in \sigma} X_{(s, j)}) &\triangleq p(i)
\end{aligned}$$

The natural transformation exhibiting Frobenius reciprocity is still the product associator. The Beck–Chevalley condition is simplified as well, and in fact gives rise to an equality of functors, not just natural isomorphism. This is important as it makes the soundness proof for substitution strict. The specific pullback square that we are examining in `Ctx` is:

$$\begin{array}{ccc}
\Theta \times \sigma & \xrightarrow{\delta \times \text{id}} & \Theta' \times \sigma \\
\pi_1 \downarrow & & \downarrow \pi_1 \\
\Theta & \xrightarrow{\delta} & \Theta'
\end{array}$$

By the BC condition, the following square commutes up to natural isomorphism:

$$\begin{array}{ccc}
\mathbf{Set}^{\Theta \times \sigma} & \xleftarrow{(\delta \times \text{id})^*} & \mathbf{Set}^{\Theta' \times \sigma} \\
\exists_{\Theta, \sigma} \downarrow & & \downarrow \exists_{\Theta', \sigma} \\
\mathbf{Set}^{\Theta} & \xleftarrow{\delta^*} & \mathbf{Set}^{\Theta'}
\end{array}$$

The isomorphism has the type  $\tau : \exists_{\Theta, \sigma} \circ (\delta \times \text{id})^* \Rightarrow \delta^* \circ \exists_{\Theta', \sigma}$ , or at component  $X : \mathbf{Set}^{\Theta' \times \sigma}$  and index  $s \in \Theta$ :

$$\tau_{X, s} : \exists_{\Theta, \sigma}((\delta \times \text{id})^*(X))_s \rightarrow \delta^*(\exists_{\Theta', \sigma}(X))_s$$

$$\tau_{X,s}: \sum_{j \in \sigma} (X_{(\delta(s),a)}) \rightarrow \sum_{j \in \sigma} (X_{(\delta(s),a)})$$

Since both the source and the target is the same,  $\tau$  is simply the identity natural transformation, making the equality of the two functors on the nose. Similarly,  $\gamma_{X,s}: \prod_{j \in \sigma} (X_{(\delta(s),a)}) \rightarrow \prod_{j \in \sigma} (X_{(\delta(s),a)})$  is also the identity natural transformation.

**Linear weakening hyperdoctrine** We can similarly specialise the linear hyperdoctrine to the projection morphism.

$$\begin{aligned} \hat{w}k_\sigma(A: \text{Rel}_{\mathcal{R}}^\Theta)_{(s,i) \in \Theta \times \sigma} &\triangleq A_s \\ \hat{w}k_\sigma(r: A \rightarrow_{\mathcal{R}} B \in \text{Rel}_{\mathcal{R}}^\Theta)_{(s,i),k}(a: A_{s,k}, b: B_{s,k}) &\triangleq r_{s,k}(a, b) \end{aligned}$$

$$\begin{aligned} \hat{\exists}_\sigma: \text{Rel}_{\mathcal{R}}^{\Theta \times \sigma} &\rightarrow_{\mathcal{R}} \text{Rel}_{\mathcal{R}}^\Theta \\ \hat{\exists}_\sigma(A: \text{Rel}_{\mathcal{R}}^{\Theta \times \sigma})_{s,k} &\triangleq \sum_{j \in \sigma} A_{(s,j),k} \\ \hat{\exists}_\sigma(r: A \rightarrow_{\mathcal{R}} B)_{s,k}((i \in \sigma, a \in A_{(s,i),k}), (j \in \sigma, a \in B_{(s,j),k})) &\triangleq i = j \wedge r_{(s,i),k}(a, b) \end{aligned}$$

$$\begin{aligned} \eta_A: A \rightarrow_{\mathcal{R}} \hat{w}k_\sigma(\hat{\exists}_\sigma(A)) & \quad \epsilon_A: \hat{\exists}_\sigma(\hat{w}k_\sigma(A)) \rightarrow_{\mathcal{R}} A \\ \eta_{A,(s,i),k}: A_{(s,i),k} \rightarrow_{\mathcal{R}} \sum_{j \in \sigma} A_{(s,j),k} & \quad \epsilon_{A,s,k}: (\sum_{j \in \sigma} A_{s,k}) \rightarrow_{\mathcal{R}} A_{s,k} \\ \eta_{A,(s,i),k}(a: A_{(s,i),k}, (j: \sigma, a: A_{(s,j),k})) \triangleq i = j \wedge a = a' & \quad \epsilon_{A,s,k}((j, x: A_{s,k}), a': A_{s,k}) \triangleq a = a' \end{aligned}$$

$$\begin{aligned} \hat{V}_\sigma: \text{Rel}_{\mathcal{R}}^{\Theta \times \sigma} &\rightarrow_{\mathcal{R}} \text{Rel}_{\mathcal{R}}^\Theta \\ \hat{V}_\sigma(A: \text{Rel}_{\mathcal{R}}^{\Theta \times \sigma})_s &\triangleq \prod_{j \in \sigma} A_{(s,j)} \\ \hat{V}_\sigma(r: A \rightarrow_{\mathcal{R}} B)_{s,k}(p: \prod_{j \in \sigma} A_{(s,j),k}, q: \prod_{j \in \sigma} B_{(s,j),k}) &\triangleq \forall i \in \sigma. r_{(s,i),k}(p(i), q(i)) \end{aligned}$$

$$\begin{aligned} \eta_A: A \rightarrow_{\mathcal{R}} \hat{V}_\sigma(\hat{w}k_\sigma(A)) & \quad \epsilon_A: \hat{w}k_\sigma(\hat{V}_\sigma(A)) \rightarrow_{\mathcal{R}} A \\ \eta_{A,s,k}: A_{s,k} \rightarrow_{\mathcal{R}} \prod_{j \in \sigma} A_{s,k} & \quad \epsilon_{A,(s,i),k}: (\prod_{j \in \sigma} A_{(s,j),k}) \rightarrow_{\mathcal{R}} A_{(s,i),k} \\ \eta_{A,s}(a: A_{s,k}, p: \prod_{j \in \sigma} A_{s,k}) \triangleq \forall i \in \sigma. p(i) = a & \quad \epsilon_{A,(s,i),k}(p: \prod_{j \in \sigma} A_{(s,j),k}, a: A_{(s,i),k}) \triangleq p(i) = a \end{aligned}$$

As with the Cartesian weakening hyperdoctrine, the natural isomorphism establishing the Beck–Chevalley condition reduces to the identity natural transformation:

$$\begin{aligned} \hat{\tau}: \hat{\exists}_{\Theta,\sigma} \circ (\delta \times \text{id})^+ &\rightarrow \delta^+ \circ \hat{\exists}_{\Theta',\sigma} \\ \hat{\tau}_{A,s,k}: \sum_{j \in \sigma} A_{(\delta(s),j),k} &\rightarrow \sum_{j \in \sigma} A_{(\delta(s),j),k} \end{aligned}$$

Similarly,  $\hat{\gamma}: \hat{V}_{\Theta,\sigma} \circ (\delta \times \text{id})^+ \rightarrow \delta^+ \circ \hat{V}_{\Theta',\sigma}$  also becomes the identity relation at every component.

## 9 Interpretation of Sorts, Types and Contexts

### 9.1 Interpretation of Sorts

We define the interpretation of sorts  $\llbracket - \rrbracket$  as:

$$\begin{aligned}\llbracket \text{time} \rrbracket &\triangleq \text{Time} \\ \llbracket \text{id} \rrbracket &\triangleq \text{Id}\end{aligned}$$

### 9.2 Interpretation of Sort context

We define the interpretation of a sort context  $\Theta$  as:

$$\begin{aligned}\llbracket \cdot \rrbracket &\triangleq \mathbb{1} \\ \llbracket \Theta, x : \sigma \rrbracket &\triangleq \llbracket \Theta \rrbracket \times \llbracket \sigma \rrbracket\end{aligned}$$

The sorting judgment  $\Theta \vdash_s s : \sigma$  is then interpreted as a Ctx-arrow  $\llbracket \Theta \rrbracket \rightarrow \llbracket \sigma \rrbracket$  corresponding to the projection of the relevant element of the tuple  $\llbracket \Theta \rrbracket$ .

### 9.3 Interpretation of Cartesian and Linear types

Given a sort context  $\Theta$ , we interpret Cartesian and linear types in the sort context as objects in the indexed category  $\text{Set}^{[\Theta]}$  and  $\text{Rel}_{\mathcal{R}}^{[\Theta]}$ . Instead of carrying around an index explicitly, we lift the relevant objects, operations and functors to the relevant indexed category: for example,  $\otimes^{[\Theta]}$  is the product in  $\text{Rel}_{\mathcal{R}}^{[\Theta]}$ , calculated pointwise for each index  $\theta \in \llbracket \Theta \rrbracket$ . Similarly,  $\diamond^{[\Theta]}$  is the event monad in  $\text{Rel}_{\mathcal{R}}^{[\Theta]}$ , defined for each  $A : \text{Rel}_{\mathcal{R}}^{[\Theta]}$  and  $\theta : \llbracket \Theta \rrbracket$  as

$$(\diamond^{[\Theta]} A)_{\theta} \triangleq \diamond(A_{\theta})$$

Given that the lifting simply corresponds to precomposition, all the important structure and properties are preserved. A slightly different case is that of the lifted iterated delay functor: in  $\text{Rel}_{\mathcal{R}}$ , for every  $n \in \mathbb{N}_{\top}$  we have an endofunctor  $\triangleright^n : \text{Rel}_{\mathcal{R}} \rightarrow \text{Rel}_{\mathcal{R}}$ . In  $\text{Rel}_{\mathcal{R}}^{[\Theta]}$ , this family of functors is indexed by the *indexed* natural numbers instead: for every  $n' : \mathbb{N}_{\top}^{[\Theta]}$ , we get an endofunctor  $\triangleright^{n'} : \text{Rel}_{\mathcal{R}}^{[\Theta]} \rightarrow \text{Rel}_{\mathcal{R}}^{[\Theta]}$ , defined by pointwise indexing on the type and the delay:

$$(\triangleright^{n'} A)_{\theta} \triangleq \triangleright^{n'_{\theta}}(A_{\theta})$$

Where unambiguous, we will write  $\otimes'$  instead of  $\otimes^{[\Theta]}$ , and similarly for other indexed objects, functors and morphisms.

$$\begin{aligned}\llbracket \Theta \vdash_c X \rrbracket &: \text{Set}^{[\Theta]} \\ \llbracket \Theta \vdash_c \mathbb{1} \rrbracket &\triangleq \mathbb{1}' \\ \llbracket \Theta \vdash_c X \rightarrow Y \rrbracket &\triangleq \llbracket \Theta \vdash_c X \rrbracket \rightarrow' \llbracket \Theta \vdash_c Y \rrbracket \\ \llbracket \Theta \vdash_c \mathsf{G} A \rrbracket &\triangleq G' \llbracket \Theta \vdash_{\ell} A \rrbracket \\ \llbracket \Theta \vdash_{\ell} A \rrbracket &: \text{Rel}_{\mathcal{R}}^{[\Theta]}\end{aligned}$$

$$\begin{aligned}
\llbracket \Theta \vdash_\ell \mathbb{I} \rrbracket &\triangleq \mathbb{I}' \\
\llbracket \Theta \vdash_\ell A \otimes B \rrbracket &\triangleq \llbracket \Theta \vdash_\ell A \rrbracket \otimes' \llbracket \Theta \vdash_\ell B \rrbracket \\
\llbracket \Theta \vdash_\ell A \multimap B \rrbracket &\triangleq \llbracket \Theta \vdash_\ell A \rrbracket \multimap'_{\mathcal{R}} \llbracket \Theta \vdash_\ell B \rrbracket \\
\llbracket \Theta \vdash_\ell \mathbf{F} X \rrbracket &\triangleq F' \llbracket \Theta \vdash_c X \rrbracket \\
\llbracket \Theta \vdash_\ell A @ \tau \rrbracket &\triangleq \triangleright^{\llbracket \Theta \vdash_s \tau : \text{time} \rrbracket} \llbracket \Theta \vdash_\ell A \rrbracket \\
\llbracket \Theta \vdash_\ell \Diamond A \rrbracket &\triangleq \Diamond' \llbracket \Theta \vdash_\ell A \rrbracket \\
\llbracket \Theta \vdash_\ell \forall i : \sigma. A \rrbracket &\triangleq \widehat{\forall}_{[\sigma]} \llbracket \Theta, i : \sigma \vdash_\ell A \rrbracket \\
\llbracket \Theta \vdash_\ell \exists i : \sigma. A \rrbracket &\triangleq \widehat{\exists}_{[\sigma]} \llbracket \Theta, i : \sigma \vdash_\ell A \rrbracket \\
\llbracket \Theta \vdash_\ell \text{Widget}' \rrbracket &\triangleq \text{Widget}^{\llbracket \Theta \vdash_s \ell : \text{id} \rrbracket} \\
\llbracket \Theta \vdash_\ell \text{Prefix}'(\tau) \rrbracket &\triangleq \text{Prefix}^{\llbracket \Theta \vdash_s \ell : \text{id} \rrbracket}(\llbracket \Theta \vdash_s \tau : \text{time} \rrbracket)
\end{aligned}$$

## 9.4 Interpretation of Cartesian and Linear context

Given the above, we can now define the interpretation of cartesian and linear contexts. Both of these are indexed by a sort context.

$$\begin{aligned}
\llbracket \Theta \vdash_c \cdot \rrbracket &\triangleq \mathbb{I}' \\
\llbracket \Theta \vdash_c \Gamma, x : X \rrbracket &\triangleq \llbracket \Theta \vdash_c \Gamma \rrbracket \times' \llbracket \Theta \vdash_c X \rrbracket \\
\llbracket \Theta \vdash_\ell \cdot \rrbracket &\triangleq \mathbb{I}' \\
\llbracket \Theta \vdash_\ell \Delta, a :_\tau A \rrbracket &\triangleq \llbracket \Theta \vdash_\ell \Delta \rrbracket \otimes' \triangleright^{\llbracket \Theta \vdash_s \tau : \text{time} \rrbracket} \llbracket \Theta \vdash_\ell A \rrbracket
\end{aligned}$$

With this interpretation, the context concatenation  $\Delta_1, \Delta_2$  will be interpreted as a left-nested iterated tensor product. By reassociating the products, we can show that  $\llbracket \Theta \vdash_\ell \Delta_1, \Delta_2 \rrbracket$  is isomorphic to  $\llbracket \Theta \vdash_\ell \Delta_1 \rrbracket \otimes \llbracket \Theta \vdash_\ell \Delta_2 \rrbracket$ :

$$\begin{aligned}
\llbracket \Theta \vdash_\ell \Delta_1, \cdot \rrbracket &= \llbracket \Theta \vdash_\ell \Delta_1 \rrbracket \\
&\cong \llbracket \Theta \vdash_\ell \Delta_1 \rrbracket \otimes' \mathbb{I}' && \text{(right unit)} \\
\llbracket \Theta \vdash_\ell \Delta_1, (\Delta_2, a :_\tau A) \rrbracket &= \llbracket \Theta \vdash_\ell (\Delta_1, \Delta_2), a :_\tau A \rrbracket \\
&= \llbracket \Theta \vdash_\ell \Delta_1, \Delta_2 \rrbracket \otimes' \triangleright^{\llbracket \tau \rrbracket} \llbracket \Theta \vdash_\ell A \rrbracket \\
&\cong (\llbracket \Theta \vdash_\ell \Delta_1 \rrbracket \otimes' \llbracket \Theta \vdash_\ell \Delta_2 \rrbracket) \otimes' \triangleright^{\llbracket \tau \rrbracket} \llbracket \Theta \vdash_\ell A \rrbracket && \text{(IH)} \\
&\cong \llbracket \Theta \vdash_\ell \Delta_1 \rrbracket \otimes' (\llbracket \Theta \vdash_\ell \Delta_2 \rrbracket \otimes' \triangleright^{\llbracket \tau \rrbracket} \llbracket \Theta \vdash_\ell A \rrbracket) && \text{(associator)} \\
&= \llbracket \Theta \vdash_\ell \Delta_1 \rrbracket \otimes' \llbracket \Theta \vdash_\ell \Delta_2, a :_\tau A \rrbracket
\end{aligned}$$

For brevity, we will denote the natural isomorphism inductively constructed via this proof as

$$\text{sep}_{\Delta_1, \Delta_2} : \llbracket \Theta \vdash_\ell \Delta_1, \Delta_2 \rrbracket \xrightarrow{\cong} \llbracket \Theta \vdash_\ell \Delta_1 \rrbracket \otimes' \llbracket \Theta \vdash_\ell \Delta_2 \rrbracket$$

The naturality condition states that we interpret the concatenated context as the product of interpretations, modulo a natural isomorphism:

$$\text{sep}_{\Delta_1, \Delta_2} \circ \llbracket \hat{\xi}_1, \hat{\xi}_2 \rrbracket = \llbracket \hat{\xi}_1 \rrbracket \otimes \llbracket \hat{\xi}_2 \rrbracket \circ \text{sep}_{\Delta'_1, \Delta'_2}$$

## 10 Interpretation of Terms

### 10.1 Interpretation of Cartesian Terms

As with the above type interpretations, the term interpretation is index over a sort context but now also a Cartesian context (for Cartesian terms) and both a Cartesian and a linear context (for linear terms). Given a sort context  $\Theta$  and a Cartesian context  $\Gamma$ , we define the interpretation of a well-typed Cartesian term  $\Theta \mid \Gamma \vdash_c e : X$  as a morphism in the indexed category  $\mathbf{Set}^{[\Theta]}$ :

$$\begin{aligned}
\llbracket \Theta \mid \Gamma \vdash_c e : X \rrbracket &: \llbracket \Theta \vdash_c \Gamma \rrbracket \rightarrow' \llbracket \Theta \vdash_c X \rrbracket \\
\llbracket \Theta \mid \Gamma, x : X \vdash_c x : X \rrbracket &\triangleq \llbracket \Theta \vdash_c \Gamma \rrbracket \times' \llbracket \Theta \vdash_c X \rrbracket \xrightarrow{\pi'_2} \llbracket \Theta \vdash_c X \rrbracket \\
\llbracket \Theta \mid \Gamma, y : Y \vdash_c x : X \rrbracket &\triangleq \llbracket \Theta \vdash_c \Gamma \rrbracket \times' \llbracket \Theta \vdash_c Y \rrbracket \xrightarrow{\pi'_1} \llbracket \Theta \vdash_c \Gamma \rrbracket \xrightarrow{\llbracket \Theta \mid \Gamma \vdash_c x : X \rrbracket} \llbracket \Theta \vdash_c X \rrbracket \\
\llbracket \Theta \mid \Gamma \vdash_c \star : 1 \rrbracket &\triangleq \llbracket \Theta \vdash_c \Gamma \rrbracket \xrightarrow{l'_{\llbracket \Theta \vdash_c \Gamma \rrbracket}} 1' \\
\llbracket \Theta \mid \Gamma \vdash_c \lambda x. e : X \rightarrow Y \rrbracket &\triangleq \text{curry}' \left( \llbracket \Theta \vdash_c \Gamma \rrbracket \times' \llbracket \Theta \vdash_c X \rrbracket \xrightarrow{\llbracket \Theta \mid \Gamma, x : X \vdash_c e : Y \rrbracket} \llbracket \Theta \vdash_c Y \rrbracket \right) \\
\llbracket \Theta \mid \Gamma \vdash_c e_1 e_2 : Y \rrbracket &\triangleq \llbracket \Theta \vdash_c \Gamma \rrbracket \xrightarrow{\langle \llbracket e_1 \rrbracket, \llbracket e_2 \rrbracket \rangle'} \llbracket \Theta \vdash_c X \rightarrow Y \rrbracket \times' \llbracket \Theta \vdash_c X \rrbracket \xrightarrow{\text{eval}'} \llbracket \Theta \vdash_c Y \rrbracket \\
\llbracket \Theta \mid \Gamma \vdash_c G t : G A \rrbracket &\triangleq \llbracket \Theta \vdash_c \Gamma \rrbracket \xrightarrow{\eta'_{\llbracket \Theta \vdash_c \Gamma \rrbracket}} G' F' \llbracket \Theta \vdash_c \Gamma \rrbracket \xrightarrow{G'(\rho_F^{-1} \llbracket \Theta \vdash_c \Gamma \rrbracket)} G(F \llbracket \Theta \vdash_c \Gamma \rrbracket \otimes' 1') \\
&\xrightarrow{G' \llbracket \Theta \mid \Gamma; \vdash_\ell t : A \rrbracket} G \llbracket \Theta \vdash_\ell A \rrbracket
\end{aligned}$$

### 10.2 Interpretation of linear terms

Given a sort context  $\Theta$ , Cartesian context  $\Gamma$ , a linear context  $\Delta$  and timestep  $\tau$ , we define the interpretation of a well-typed linear term  $\Theta \mid \Gamma; \Delta \vdash_\tau t : A$  as a morphism in the indexed category  $\mathbf{Rel}_{\mathcal{R}}^{[\Theta]}$ . As before, if  $\tau = 0$ , we will omit the subscript. To simplify the definitions, we make use of a few derived operations, mainly for manipulating and reordering context interpretations. First, we use  $\varsigma$  for any appropriate sequence of reassociations ( $\alpha$ ) and reorderings ( $\sigma$ ) required to transform an object into a suitable form. This is always possible, since  $\mathbf{Rel}_{\mathcal{R}}$  (and  $\mathbf{Rel}_{\mathcal{R}}^{[\Theta]}$ ) is a symmetric monoidal closed category and the tensor product is associative and commutative. Linearity disallows projections and unit maps in general, but these can be implemented for sets embedded into  $\mathbf{Rel}_{\mathcal{R}}$  by the monoidal functor  $F$ . We therefore have two derived natural transformations for discarding and duplicating  $F$ -typed values:

$$\begin{aligned}
\text{disc}_X &: FX \rightarrow_{\mathcal{R}} 1 \in \mathbf{Rel}_{\mathcal{R}} & \text{dup}_X &: FX \rightarrow_{\mathcal{R}} FX \otimes FX \in \mathbf{Rel}_{\mathcal{R}} \\
\text{disc}_X &\triangleq FX \xrightarrow{F(1_X)} F1 \xrightarrow{u^{-1}} 1 & \text{dup}_X &\triangleq FX \xrightarrow{F(\langle \text{id}, \text{id} \rangle)} F(X \times X) \xrightarrow{m_{X,X}^{-1}} FX \otimes FX
\end{aligned}$$

Again, for the sake of brevity, the definitions below use more specialised operations derived from the ones above. These correspond to the common patterns of dropping the Cartesian context, or duplicating it and pairing it up with two halves of a linear context (required for nearly all terms which have two subterms and therefore independent linear contexts).

$$\text{drop}_{\Theta, \Gamma, \Delta} : F' \llbracket \Theta \vdash_c \Gamma \rrbracket \otimes' \llbracket \Theta \vdash_\ell \Delta \rrbracket \rightarrow_{\mathcal{R}} \llbracket \Theta \vdash_\ell \Delta \rrbracket$$

$$\begin{aligned}
\text{drop}_{\Theta, \Gamma, \Delta} &\triangleq \lambda'_{\llbracket \Theta \vdash_{\ell} \Delta \rrbracket} \circ (\text{disc}'_{\llbracket \Theta \vdash_c \Gamma \rrbracket} \otimes' \text{id}_{\llbracket \Theta \vdash_{\ell} \Delta \rrbracket}) \\
\text{split}_{\Theta, \Gamma, \Delta_1, \Delta_2} &: F'[\llbracket \Theta \vdash_c \Gamma \rrbracket] \otimes' [\llbracket \Theta \vdash_{\ell} \Delta_1, \Delta_2 \rrbracket] \\
&\quad \rightarrow_{\mathcal{R}} (F'[\llbracket \Theta \vdash_c \Gamma \rrbracket] \otimes' [\llbracket \Theta \vdash_{\ell} \Delta_1 \rrbracket]) \otimes' (F'[\llbracket \Theta \vdash_c \Gamma \rrbracket] \otimes' [\llbracket \Theta \vdash_{\ell} \Delta_2 \rrbracket]) \\
\text{split}_{\Theta, \Gamma, \Delta_1, \Delta_2} &\triangleq \varsigma' \circ (\text{dup}'_{\llbracket \Theta \vdash_c \Gamma \rrbracket} \otimes' \text{sep}'_{\Delta_1, \Delta_2})
\end{aligned}$$

We will omit the subscripts when they can be inferred from the context.

Below we give the interpretations of the linear terms. The semantics of **select** and the temporal quantification terms are given in more detail, since they rely on some metatheoretic properties of index substitution and the *LNL* hyperdoctrine structure.

$$\begin{aligned}
\llbracket \Theta \mid \Gamma; \Delta \vdash_{\ell} t :_{\tau} A \rrbracket &: F'[\llbracket \Theta \vdash_c \Gamma \rrbracket] \otimes' [\llbracket \Theta \vdash_{\ell} \Delta \rrbracket] \rightarrow'_{\mathcal{R}} [\llbracket \Theta \vdash_{\ell} A \rrbracket] \\
\llbracket \Theta \mid \Gamma; a : A \vdash_{\ell} a : A \rrbracket &\triangleq F'[\llbracket \Theta \vdash_c \Gamma \rrbracket] \otimes' [\llbracket \Theta \vdash_{\ell} A \rrbracket] \xrightarrow{\text{drop}'} [\llbracket \Theta \vdash_{\ell} A \rrbracket] \\
\llbracket \Theta \mid \Gamma; \cdot \vdash_{\ell} \langle \rangle : \mathbb{I} \rrbracket &\triangleq F'[\llbracket \Theta \vdash_c \Gamma \rrbracket] \otimes' \mathbb{I}' \xrightarrow{\text{drop}'} \mathbb{I}' \\
\llbracket \Theta \mid \Gamma; \Delta \vdash_{\ell} \lambda a. t : A \multimap B \rrbracket &\triangleq \text{curry}' \left( (F'[\llbracket \Theta \vdash_c \Gamma \rrbracket] \otimes' [\llbracket \Theta \vdash_{\ell} \Delta \rrbracket]) \otimes' [\llbracket \Theta \vdash_c A \rrbracket] \right. \\
&\quad \left. \xrightarrow{\llbracket \Theta \mid \Gamma; \Delta, a : A \vdash_{\ell} t : B \rrbracket \circ \varsigma^{\llbracket \Theta \rrbracket}} [\llbracket \Theta \vdash_{\ell} B \rrbracket] \right) \\
\llbracket \Theta \mid \Gamma; \Delta_1, \Delta_2 \vdash_{\ell} t_1 t_2 : B \rrbracket &\triangleq F'[\llbracket \Theta \vdash_c \Gamma \rrbracket] \otimes' [\llbracket \Theta \vdash_{\ell} \Delta_1, \Delta_2 \rrbracket] \\
&\xrightarrow{\text{split}'} (F'[\llbracket \Theta \vdash_c \Gamma \rrbracket] \otimes' [\llbracket \Theta \vdash_{\ell} \Delta_1 \rrbracket]) \otimes' (F'[\llbracket \Theta \vdash_c \Gamma \rrbracket] \otimes' [\llbracket \Theta \vdash_{\ell} \Delta_2 \rrbracket]) \\
&\xrightarrow{\llbracket t_1 \rrbracket \otimes' \llbracket t_2 \rrbracket} [\llbracket \Theta \vdash_{\ell} A \multimap B \rrbracket] \otimes' [\llbracket \Theta \vdash_{\ell} B \rrbracket] \xrightarrow{\text{eval}'} [\llbracket \Theta \vdash_{\ell} B \rrbracket] \\
\llbracket \Theta \mid \Gamma; \Delta_1, \Delta_2 \vdash_{\ell} \text{let } \langle \rangle = t_1 \text{ in } t_2 : B \rrbracket &\triangleq F'[\llbracket \Theta \vdash_c \Gamma \rrbracket] \otimes' [\llbracket \Theta \vdash_{\ell} \Delta_1, \Delta_2 \rrbracket] \\
&\xrightarrow{\llbracket t_1 \rrbracket \otimes' \llbracket t_2 \rrbracket \circ \text{split}'} \mathbb{I}' \otimes' [\llbracket \Theta \vdash_{\ell} B \rrbracket] \xrightarrow{\lambda'_{\llbracket \Theta \vdash_{\ell} B \rrbracket}} [\llbracket \Theta \vdash_{\ell} B \rrbracket] \\
\llbracket \Theta \mid \Gamma; \Delta_1, \Delta_2 \vdash_{\ell} (t_1, t_2) : A \otimes B \rrbracket &\triangleq F'[\llbracket \Theta \vdash_c \Gamma \rrbracket] \otimes' [\llbracket \Theta \vdash_{\ell} \Delta_1, \Delta_2 \rrbracket] \\
&\xrightarrow{\llbracket t_1 \rrbracket \otimes' \llbracket t_2 \rrbracket \circ \text{split}'} [\llbracket \Theta \vdash_{\ell} A \rrbracket] \otimes' [\llbracket \Theta \vdash_{\ell} B \rrbracket] \\
\llbracket \Theta \mid \Gamma; \Delta_1, \Delta_2 \vdash_{\ell} \text{let } (a, b) = t_1 \text{ in } t_2 : C \rrbracket &\triangleq F'[\llbracket \Theta \vdash_c \Gamma \rrbracket] \otimes' [\llbracket \Theta \vdash_{\ell} \Delta_1, \Delta_2 \rrbracket] \\
&\xrightarrow{(\llbracket t_1 \rrbracket \otimes' \text{id}) \circ \text{split}'} ([\llbracket \Theta \vdash_{\ell} A \rrbracket] \otimes' [\llbracket \Theta \vdash_{\ell} B \rrbracket]) \otimes' (F'[\llbracket \Theta \vdash_c \Gamma \rrbracket] \otimes' [\llbracket \Theta \vdash_{\ell} \Delta_2 \rrbracket]) \\
&\xrightarrow{\llbracket t_2 \rrbracket \circ \varsigma^{\llbracket \Theta \rrbracket}} [\llbracket \Theta \vdash_{\ell} C \rrbracket] \\
\llbracket \Theta \mid \Gamma; \Delta \vdash_{\ell} \text{evt } t : \diamond A \rrbracket &\triangleq F'[\llbracket \Theta \vdash_c \Gamma \rrbracket] \otimes' [\llbracket \Theta \vdash_{\ell} \Delta \rrbracket] \xrightarrow{\llbracket t \rrbracket} [\llbracket \Theta \vdash_{\ell} A \rrbracket] \xrightarrow{\eta'_{\llbracket \Theta \vdash_{\ell} A \rrbracket}} \diamond' [\llbracket \Theta \vdash_{\ell} A \rrbracket] \\
\llbracket \Theta \mid \Gamma; \Delta \vdash_{\ell} \text{let evt } x = t_1 \text{ in } t_2 : \diamond B \rrbracket &\triangleq F'[\llbracket \Theta \vdash_c \Gamma \rrbracket] \otimes' [\llbracket \Theta \vdash_{\ell} \Delta \rrbracket] \\
&\xrightarrow{\varsigma^{\llbracket \Theta \rrbracket} \circ (\text{dup}' \otimes \text{id})} F'[\llbracket \Theta \vdash_c \Gamma \rrbracket] \otimes' (F'[\llbracket \Theta \vdash_c \Gamma \rrbracket] \otimes' [\llbracket \Theta \vdash_{\ell} \Delta \rrbracket]) \\
&\xrightarrow{\text{id} \otimes' \llbracket t_1 \rrbracket} F'[\llbracket \Theta \vdash_c \Gamma \rrbracket] \otimes' \diamond' [\llbracket \Theta \vdash_{\ell} A \rrbracket] \\
&\xrightarrow{\text{st}_{\llbracket \Theta \vdash_c \Gamma \rrbracket, \llbracket \Theta \vdash_{\ell} A \rrbracket}^{F'}} \diamond' (F'[\llbracket \Theta \vdash_c \Gamma \rrbracket] \otimes' [\llbracket \Theta \vdash_{\ell} A \rrbracket])
\end{aligned}$$

$$\begin{aligned}
& \xrightarrow{\diamond' \llbracket t_2 \rrbracket} \diamond' \diamond' \llbracket \Theta \vdash_\ell B \rrbracket \xrightarrow{\mu'_{\llbracket \Theta \vdash_\ell B \rrbracket}} \diamond' \llbracket \Theta \vdash_\ell B \rrbracket \\
& \llbracket \Theta \mid \Gamma; \Delta \vdash_\ell t @ \tau : A @ \tau \rrbracket \triangleq F' \llbracket \Theta \vdash_c \Gamma \rrbracket \otimes' \llbracket \Theta \vdash_\ell \Delta \rrbracket \xrightarrow{\llbracket \Theta \mid \Gamma; \Delta \vdash_\ell t; \tau A \rrbracket} \triangleright \llbracket \Theta \vdash_{s\tau} : \text{time} \rrbracket \llbracket \Theta \vdash_\ell A \rrbracket \\
& \llbracket \Theta \mid \Gamma; \Delta_1, \Delta_2 \vdash_\ell \text{let } a @ \tau = t_1 \text{ in } t_2 : B \rrbracket \triangleq F' \llbracket \Theta \vdash_c \Gamma \rrbracket \otimes' \llbracket \Theta \vdash_\ell \Delta_1, \Delta_2 \rrbracket \\
& \xrightarrow{(\llbracket t_1 \rrbracket \otimes' \text{id}) \circ \text{split}'} \triangleright \llbracket \Theta \vdash_{s\tau} : \text{time} \rrbracket \llbracket \Theta \vdash_\ell A \rrbracket \otimes' (F' \llbracket \Theta \vdash_c \Gamma \rrbracket \otimes' \llbracket \Theta \vdash_\ell \Delta_2 \rrbracket) \\
& \xrightarrow{\zeta^{[\Theta]}} F' \llbracket \Theta \vdash_c \Gamma \rrbracket \otimes' (\llbracket \Theta \vdash_\ell \Delta_2 \rrbracket \otimes' \triangleright \llbracket \Theta \vdash_{s\tau} : \text{time} \rrbracket \llbracket \Theta \vdash_\ell A \rrbracket) \\
& \xrightarrow{\llbracket \Theta \mid \Gamma; \Delta_2, a; \tau A \vdash_\ell t_2 : B \rrbracket} \llbracket \Theta \vdash_\ell B \rrbracket \\
& \llbracket \Theta \mid \Gamma; \cdot \vdash_\ell \text{runG } e : A \rrbracket \triangleq F' \llbracket \Theta \vdash_c \Gamma \rrbracket \otimes' \text{!} \xrightarrow{\rho_{F' \llbracket \Theta \vdash_c \Gamma \rrbracket}} F' \llbracket \Theta \vdash_c \Gamma \rrbracket \\
& \xrightarrow{F' \llbracket \Theta \mid \Gamma \vdash_{ce} : \text{G } A \rrbracket} F' (G' \llbracket \Theta \vdash_\ell A \rrbracket) \xrightarrow{\varepsilon_{\llbracket \Theta \vdash_\ell A \rrbracket}} \llbracket \Theta \vdash_\ell A \rrbracket \\
& \llbracket \Theta \mid \Gamma; \cdot \vdash_\ell \text{F } e : \text{F } X \rrbracket \triangleq F' \llbracket \Theta \vdash_c \Gamma \rrbracket \otimes' \text{!} \xrightarrow{\rho_{F' \llbracket \Theta \vdash_c \Gamma \rrbracket}} F' \llbracket \Theta \vdash_c \Gamma \rrbracket \\
& \xrightarrow{F' \llbracket \Theta \mid \Gamma \vdash_{ce} : X \rrbracket} F' \llbracket \Theta \vdash_c X \rrbracket \\
& \llbracket \Theta \mid \Gamma; \Delta_1, \Delta_2 \vdash_\ell \text{let F } x = t_1 \text{ in } t_2 : B \rrbracket \triangleq F' \llbracket \Theta \vdash_c \Gamma \rrbracket \otimes' \llbracket \Theta \vdash_\ell \Delta_1, \Delta_2 \rrbracket \\
& \xrightarrow{(\llbracket t_1 \rrbracket \otimes' \text{id}) \circ \text{split}'} F' \llbracket \Theta \vdash_c X \rrbracket \otimes' (F' \llbracket \Theta \vdash_c \Gamma \rrbracket \otimes' \llbracket \Theta \vdash_\ell \Delta_2 \rrbracket) \\
& \xrightarrow{\text{m}_{\llbracket \Theta \vdash_c \Gamma \rrbracket, \llbracket \Theta \vdash_c X \rrbracket} \otimes' \text{id}_{\llbracket \Theta \vdash_\ell \Delta_2 \rrbracket} \circ \zeta^{[\Theta]}} F' (\llbracket \Theta \vdash_c \Gamma \rrbracket \otimes' \llbracket \Theta \vdash_c X \rrbracket) \otimes' \llbracket \Theta \vdash_\ell \Delta_2 \rrbracket \\
& \xrightarrow{\llbracket \Theta \mid \Gamma, x : X; \Delta_2 \vdash_\ell t_2 : B \rrbracket} \llbracket \Theta \vdash_\ell B \rrbracket
\end{aligned}$$

$$\llbracket \Theta \mid \Gamma; \Delta \vdash_\ell \Lambda i : \sigma. t : \forall i : \sigma. A \rrbracket :$$

$$\begin{aligned}
& h \triangleq \\
& \hat{\text{wk}}_{[\sigma]} (F^{[\Theta]} \llbracket \Theta \vdash_c \Gamma \rrbracket \otimes^{[\Theta]} \llbracket \Theta \vdash_\ell \Delta \rrbracket) \\
& \quad \downarrow \text{m}_{F^{[\Theta]} \llbracket \Theta \vdash_c \Gamma \rrbracket, \llbracket \Theta \vdash_\ell \Delta \rrbracket}^{-1} \\
& \hat{\text{wk}}_{[\sigma]} (F^{[\Theta]} \llbracket \Theta \vdash_c \Gamma \rrbracket) \otimes^{[\Theta] \times [\sigma]} \hat{\text{wk}}_{[\sigma]} \llbracket \Theta \vdash_\ell \Delta \rrbracket \\
& \quad \parallel \text{LNL property} \\
& F^{[\Theta] \times [\sigma]} (\hat{\text{wk}}_{[\sigma]} \llbracket \Theta \vdash_c \Gamma \rrbracket) \otimes^{[\Theta] \times [\sigma]} \hat{\text{wk}}_{[\sigma]} \llbracket \Theta \vdash_\ell \Delta \rrbracket \\
& \quad \parallel i \text{ is free in } \Gamma \text{ and } \Delta \\
& F^{[\Theta] \times [\sigma]} \llbracket \Theta, i : \sigma \vdash_c \Gamma \rrbracket \otimes^{[\Theta] \times [\sigma]} \llbracket \Theta, i : \sigma \vdash_\ell \Delta \rrbracket \\
& \quad \downarrow \llbracket \Theta, i : \sigma \mid \Gamma; \Delta \vdash_\ell t : A \rrbracket \\
& \llbracket \Theta, i : \sigma \vdash_\ell A \rrbracket
\end{aligned}
\qquad
\begin{aligned}
& F^{[\Theta]} \llbracket \Theta \vdash_c \Gamma \rrbracket \otimes^{[\Theta]} \llbracket \Theta \vdash_\ell \Delta \rrbracket \\
& \quad \downarrow \hat{\text{wk}}_{[\sigma]} \dashv \hat{\text{V}}_{[\sigma]} \text{ transpose for } h \\
& \hat{\text{V}}_{[\sigma]} \llbracket \Theta, i : \sigma \vdash_\ell A \rrbracket \\
& \quad \parallel \text{def. of } \forall \text{ type} \\
& \llbracket \Theta \vdash_\ell \forall i : \sigma. A \rrbracket
\end{aligned}$$

$$\begin{array}{c}
\llbracket \Theta \mid \Gamma; \Delta \vdash_{\ell} t_s : \{s/i\}A \rrbracket : \\
\\
F^{[\Theta]} \llbracket \Theta \vdash_c \Gamma \rrbracket \otimes^{[\Theta]} \llbracket \Theta \vdash_{\ell} \Delta \rrbracket \\
\downarrow \llbracket \Theta \mid \Gamma; \Delta \vdash_{\ell} t : \forall i : \sigma. A \rrbracket \\
\llbracket \Theta \vdash_{\ell} \forall i : \sigma. A \rrbracket \\
\parallel \text{def. of } \forall \text{ type} \\
\hat{V}_{[\sigma]} \llbracket \Theta, i : \sigma \vdash_{\ell} A \rrbracket \\
\parallel \text{weakening property} \\
\langle \text{id}_{[\Theta]}, \llbracket \Theta \vdash s : \sigma \rrbracket \rangle^+ (\hat{w}k_{[\sigma]} (\hat{V}_{[\sigma]} \llbracket \Theta, i : \sigma \vdash_{\ell} A \rrbracket)) \\
\downarrow \langle \text{id}_{[\Theta]}, \llbracket \Theta \vdash s : \sigma \rrbracket \rangle^+ (\varepsilon_{\llbracket \Theta, i : \sigma \vdash_{\ell} A \rrbracket}) \\
\langle \text{id}_{[\Theta]}, \llbracket \Theta \vdash s : \sigma \rrbracket \rangle^+ \llbracket \Theta, i : \sigma \vdash_{\ell} A \rrbracket \\
\parallel \text{soundness of substitution} \\
\llbracket \Theta \vdash_{\ell} \{s/i\}A \rrbracket
\end{array}
\qquad
\begin{array}{c}
\llbracket \Theta \mid \Gamma; \Delta \vdash_{\ell} \{s, t\} : \exists i : \sigma. A \rrbracket : \\
\\
F^{[\Theta]} \llbracket \Theta \vdash_c \Gamma \rrbracket \otimes^{[\Theta]} \llbracket \Theta \vdash_{\ell} \Delta \rrbracket \\
\downarrow \llbracket \Theta \mid \Gamma; \Delta \vdash_{\ell} t : \{s/i\}A \rrbracket \\
\llbracket \Theta \vdash_{\ell} \{s/i\}A \rrbracket \\
\parallel \text{soundness of substitution} \\
\langle \text{id}_{[\Theta]}, \llbracket \Theta \vdash s : \sigma \rrbracket \rangle^+ \llbracket \Theta, i : \sigma \vdash_{\ell} A \rrbracket \\
\downarrow \langle \text{id}_{[\Theta]}, \llbracket \Theta \vdash s : \sigma \rrbracket \rangle^+ (\eta_{\llbracket \Theta, i : \sigma \vdash_{\ell} A \rrbracket}) \\
\langle \text{id}_{[\Theta]}, \llbracket \Theta \vdash s : \sigma \rrbracket \rangle^+ (\hat{w}k_{[\sigma]} (\hat{\exists}_{[\sigma]} \llbracket \Theta, i : \sigma \vdash_{\ell} A \rrbracket)) \\
\parallel \text{weakening property} \\
\hat{\exists}_{[\sigma]} \llbracket \Theta, i : \sigma \vdash_{\ell} A \rrbracket \\
\parallel \text{def. of } \exists \text{ type} \\
\llbracket \Theta \vdash_{\ell} \exists i : \sigma. A \rrbracket
\end{array}$$



$$\llbracket \Theta \mid \Gamma; \Delta_1, \Delta_2 \vdash_\ell \text{let } \{s, a\} = t_1 \text{ in } t_2 : B \rrbracket :$$

$$\begin{aligned}
& F^{[\Theta]} \llbracket \Theta \vdash_c \Gamma \rrbracket \otimes^{[\Theta]} \llbracket \Theta \vdash_\ell \Delta_1, \Delta_2 \rrbracket \\
& \quad \downarrow \text{split}' \\
& (F^{[\Theta]} \llbracket \Theta \vdash_c \Gamma \rrbracket \otimes^{[\Theta]} \llbracket \Theta \vdash_\ell \Delta_1 \rrbracket) \otimes^{[\Theta]} (F^{[\Theta]} \llbracket \Theta \vdash_c \Gamma \rrbracket \otimes^{[\Theta]} \llbracket \Theta \vdash_\ell \Delta_2 \rrbracket) \\
& \quad \downarrow \llbracket \Theta \mid \Gamma; \Delta_1 \vdash_\ell t_1 : \exists i : \sigma. A \rrbracket \otimes^{[\Theta]} \text{id} \\
& \hat{\exists}_{[\sigma]} \llbracket \Theta, i : \sigma \vdash_\ell A \rrbracket \otimes^{[\Theta]} (F^{[\Theta]} \llbracket \Theta \vdash_c \Gamma \rrbracket \otimes^{[\Theta]} \llbracket \Theta \vdash_\ell \Delta_2 \rrbracket) \\
& \quad \parallel \text{Frobenius reciprocity} \\
& \hat{\exists}_{[\sigma]} \left( \llbracket \Theta, i : \sigma \vdash_\ell A \rrbracket \otimes^{[\Theta] \times [\sigma]} \hat{\text{wk}}_{[\sigma]} (F^{[\Theta]} \llbracket \Theta \vdash_c \Gamma \rrbracket \otimes^{[\Theta]} \llbracket \Theta \vdash_\ell \Delta_2 \rrbracket) \right) \\
& \quad \downarrow \hat{\exists}_{[\sigma]} \left( \text{id} \otimes^{[\Theta] \times [\sigma]} m_{F^{[\Theta]} \llbracket \Theta \vdash_c \Gamma \rrbracket, \llbracket \Theta \vdash_\ell \Delta_2 \rrbracket}^{-1} \right) \\
& \hat{\exists}_{[\sigma]} \left( \llbracket \Theta, i : \sigma \vdash_\ell A \rrbracket \otimes^{[\Theta] \times [\sigma]} (\hat{\text{wk}}_{[\sigma]} (F^{[\Theta]} \llbracket \Theta \vdash_c \Gamma \rrbracket) \otimes^{[\Theta] \times [\sigma]} \hat{\text{wk}}_{[\sigma]} (\llbracket \Theta \vdash_\ell \Delta_2 \rrbracket)) \right) \\
& \quad \parallel \text{LNL property} \\
& \hat{\exists}_{[\sigma]} \left( \llbracket \Theta, i : \sigma \vdash_\ell A \rrbracket \otimes^{[\Theta] \times [\sigma]} (F^{[\Theta] \times [\sigma]} (\hat{\text{wk}}_{[\sigma]} \llbracket \Theta \vdash_c \Gamma \rrbracket) \otimes^{[\Theta] \times [\sigma]} \hat{\text{wk}}_{[\sigma]} (\llbracket \Theta \vdash_\ell \Delta_2 \rrbracket)) \right) \\
& \quad \parallel s \text{ is not free in } \Gamma \text{ and } \Delta_2 \\
& \hat{\exists}_{[\sigma]} (\llbracket \Theta, i : \sigma \vdash_\ell A \rrbracket \otimes^{[\Theta] \times [\sigma]} (F^{[\Theta] \times [\sigma]} \llbracket \Theta, s : \sigma \vdash_c \Gamma \rrbracket \otimes^{[\Theta] \times [\sigma]} \llbracket \Theta, s : \sigma \vdash_\ell \Delta_2 \rrbracket)) \\
& \quad \downarrow \hat{\exists}_{[\sigma]} (\varsigma^{[\Theta] \times [\sigma]}) \text{ (commutativity and associativity of } \otimes^{[\Theta] \times [\sigma]}) \\
& \hat{\exists}_{[\sigma]} (F^{[\Theta] \times [\sigma]} \llbracket \Theta, s : \sigma \vdash_c \Gamma \rrbracket \otimes^{[\Theta] \times [\sigma]} (\llbracket \Theta, s : \sigma \vdash_\ell \Delta_2 \rrbracket \otimes^{[\Theta] \times [\sigma]} \llbracket \Theta, i : \sigma \vdash_\ell A \rrbracket)) \\
& \quad \parallel \text{identity preservation law for } \langle - \rangle^+ \\
& \hat{\exists}_{[\sigma]} (F^{[\Theta] \times [\sigma]} \llbracket \Theta, s : \sigma \vdash_c \Gamma \rrbracket \otimes^{[\Theta] \times [\sigma]} (\llbracket \Theta, s : \sigma \vdash_\ell \Delta_2 \rrbracket \otimes^{[\Theta] \times [\sigma]} \text{id}_{[\Theta] \times [\sigma]}^+ \llbracket \Theta, i : \sigma \vdash_\ell A \rrbracket)) \\
& \quad \parallel \text{CCC law} \\
& \hat{\exists}_{[\sigma]} (F^{[\Theta] \times [\sigma]} \llbracket \Theta, s : \sigma \vdash_c \Gamma \rrbracket \otimes^{[\Theta] \times [\sigma]} (\llbracket \Theta, s : \sigma \vdash_\ell \Delta_2 \rrbracket \otimes^{[\Theta] \times [\sigma]} (\pi_1 \circ \langle \text{id}_{[\Theta] \times [\sigma]}, \llbracket \Theta, s : \sigma \vdash s : \sigma \rrbracket \rangle)^+ \llbracket \Theta, i : \sigma \vdash_\ell A \rrbracket)) \\
& \quad \parallel \text{composition preservation law for } \langle - \rangle^+ \\
& \hat{\exists}_{[\sigma]} (F^{[\Theta] \times [\sigma]} \llbracket \Theta, s : \sigma \vdash_c \Gamma \rrbracket \otimes^{[\Theta] \times [\sigma]} (\llbracket \Theta, s : \sigma \vdash_\ell \Delta_2 \rrbracket \otimes^{[\Theta] \times [\sigma]} \langle \text{id}_{[\Theta] \times [\sigma]}, \llbracket \Theta, s : \sigma \vdash s : \sigma \rrbracket \rangle^+ (\pi_1^+ \llbracket \Theta, i : \sigma \vdash_\ell A \rrbracket)) \\
& \quad \parallel \text{weakening (} s \text{ is not free in } A, \text{ and } \pi_1^+ = \hat{\text{wk}}) \\
& \hat{\exists}_{[\sigma]} (F^{[\Theta] \times [\sigma]} \llbracket \Theta, s : \sigma \vdash_c \Gamma \rrbracket \otimes^{[\Theta] \times [\sigma]} (\llbracket \Theta, s : \sigma \vdash_\ell \Delta_2 \rrbracket \otimes^{[\Theta] \times [\sigma]} \langle \text{id}_{[\Theta] \times [\sigma]}, \llbracket \Theta, s : \sigma \vdash s : \sigma \rrbracket \rangle^+ \llbracket \Theta, s : \sigma, i : \sigma \vdash_\ell A \rrbracket)) \\
& \quad \parallel \text{soundness of substitution} \\
& \hat{\exists}_{[\sigma]} (F^{[\Theta] \times [\sigma]} \llbracket \Theta, s : \sigma \vdash_c \Gamma \rrbracket \otimes^{[\Theta] \times [\sigma]} (\llbracket \Theta, s : \sigma \vdash_\ell \Delta_2 \rrbracket \otimes^{[\Theta] \times [\sigma]} \llbracket \Theta, s : \sigma \vdash_\ell \{s/i\}A \rrbracket)) \\
& \quad \parallel \text{denotation of contexts} \\
& \hat{\exists}_{[\sigma]} (F^{[\Theta] \times [\sigma]} \llbracket \Theta, s : \sigma \vdash_c \Gamma \rrbracket \otimes^{[\Theta] \times [\sigma]} \llbracket \Theta, s : \sigma \vdash_\ell \Delta_2, a : \{s/i\}A \rrbracket) \\
& \quad \downarrow \hat{\exists}_{[\sigma]} \dashv \hat{\text{wk}}_{[\sigma]} \text{ transpose for } \llbracket \Theta, s : \sigma \mid \Gamma; \Delta_2, a : \{s/i\}A \vdash_\ell t_2 : B \rrbracket \\
& \llbracket \Theta \vdash_\ell B \rrbracket
\end{aligned}$$

$$\begin{array}{c}
\llbracket \Theta \mid \Gamma; \Delta_1, \Delta_2 \vdash_\ell \text{select } (t_1, t_2) \text{ as } [a_1 \mapsto t'_1] \parallel [a_2 \mapsto t'_2] : \Diamond C \rrbracket : \\
\\
F'[\llbracket \Theta \vdash_c \Gamma \rrbracket] \otimes' [\llbracket \Theta \vdash_\ell \Delta_1, \Delta_2 \rrbracket] \\
\downarrow (\text{split} \otimes' \text{id}) \circ \varsigma \circ (\text{dup} \otimes' \text{id}) \\
F'[\llbracket \Theta \vdash_c \Gamma \rrbracket] \otimes' (F'[\llbracket \Theta \vdash_c \Gamma \rrbracket] \otimes' [\llbracket \Theta \vdash_\ell \Delta_1 \rrbracket]) \otimes' (F'[\llbracket \Theta \vdash_c \Gamma \rrbracket] \otimes' [\llbracket \Theta \vdash_\ell \Delta_2 \rrbracket]) \\
\downarrow \text{id} \otimes [\llbracket t_1 \rrbracket] \otimes [\llbracket t_2 \rrbracket] \\
F'[\llbracket \Theta \vdash_c \Gamma \rrbracket] \otimes' \Diamond' [\llbracket \Theta \vdash_\ell A \rrbracket] \otimes' \Diamond' [\llbracket \Theta \vdash_\ell B \rrbracket] \\
\downarrow \text{id} \otimes \text{race}' \\
F'[\llbracket \Theta \vdash_c \Gamma \rrbracket] \otimes' \Diamond' ([\llbracket \Theta \vdash_\ell A \rrbracket] \otimes' \Diamond' [\llbracket \Theta \vdash_\ell B \rrbracket] \oplus \Diamond' [\llbracket \Theta \vdash_\ell A \rrbracket] \otimes' [\llbracket \Theta \vdash_\ell B \rrbracket]) \\
\downarrow \text{st}'^{F'} \\
\Diamond' (F'[\llbracket \Theta \vdash_c \Gamma \rrbracket] \otimes' ([\llbracket \Theta \vdash_\ell A \rrbracket] \otimes' \Diamond' [\llbracket \Theta \vdash_\ell B \rrbracket] \oplus \Diamond' [\llbracket \Theta \vdash_\ell A \rrbracket] \otimes' [\llbracket \Theta \vdash_\ell B \rrbracket])) \\
\downarrow \Diamond' \text{dist}' \\
\Diamond' ((F'[\llbracket \Theta \vdash_c \Gamma \rrbracket] \otimes' [\llbracket \Theta \vdash_\ell A \rrbracket] \otimes' \Diamond' [\llbracket \Theta \vdash_\ell B \rrbracket]) \oplus (F'[\llbracket \Theta \vdash_c \Gamma \rrbracket] \otimes' \Diamond' [\llbracket \Theta \vdash_\ell A \rrbracket] \otimes' [\llbracket \Theta \vdash_\ell B \rrbracket])) \\
\downarrow \Diamond' [\llbracket t'_1 \rrbracket, \llbracket t'_2 \rrbracket]' \\
\Diamond' \Diamond' [\llbracket \Theta \vdash_\ell C \rrbracket] \\
\downarrow \mu'_{[\llbracket \Theta \vdash_\ell C \rrbracket]} \\
\Diamond' [\llbracket \Theta \vdash_\ell C \rrbracket]
\end{array}$$

## 11 Semantics of substitution

In order to prove the soundness of our system, we need to specify some lemmas about our meta-syntactic substitution operation. In particular, we need to interpret index substitutions, Cartesian substitutions and linear substitutions, and prove that the operations are sound.

### 11.1 Index substitution

#### 11.1.1 Interpretation of index weakening

**Definition 11.1.** We interpret the index membership relation  $s : \sigma \in \Theta$  as a morphism  $\llbracket s : \sigma \in \Theta \rrbracket : \llbracket \Theta \rrbracket \rightarrow \llbracket \sigma \rrbracket$  corresponding to the relevant projection morphism:

$$\begin{aligned}
\llbracket s : \sigma \in \Theta, s : \sigma \rrbracket &\triangleq \pi_2 \\
\llbracket s : \sigma \in \Theta, s' : \sigma' \rrbracket &\triangleq \llbracket s : \sigma \in \Theta \rrbracket \circ \pi_1
\end{aligned}$$

**Definition 11.2.** We interpret the index subcontext relation  $\Theta' \supseteq \Theta$  as a morphism  $\llbracket \Theta' \supseteq \Theta \rrbracket : \llbracket \Theta' \rrbracket \rightarrow \llbracket \Theta \rrbracket$  in the category  $\text{Ctx}$  of contexts:

$$\begin{aligned}
\llbracket \cdot \supseteq \cdot \rrbracket &\triangleq \text{id}_1 \\
\llbracket \Theta', s : \sigma \supseteq \Theta \rrbracket &\triangleq \llbracket \Theta' \supseteq \Theta \rrbracket \circ \pi_1 \\
\llbracket \Theta', s : \sigma \supseteq \Theta, s : \sigma \rrbracket &\triangleq \llbracket \Theta' \supseteq \Theta \rrbracket \times \text{id}_{\llbracket \sigma \rrbracket}
\end{aligned}$$

**Lemma 11.3** (Soundness of context membership). If  $s : \sigma \in \Theta$  and  $\Theta' \supseteq \Theta$ , then  $\llbracket s : \sigma \in \Theta' \rrbracket = \llbracket s : \sigma \in \Theta \rrbracket \circ \llbracket \Theta' \supseteq \Theta \rrbracket$ .

*Proof.* By induction on the membership relation  $s : \sigma \in \Theta$ .

- $s : \sigma \in \Theta, s : \sigma$ :

In one case we have  $\Theta', s : \sigma \supseteq \Theta, s : \sigma$ :

$$\begin{aligned} \llbracket s : \sigma \in \Theta', s : \sigma \rrbracket &= \pi_2 \\ &= \pi_2 \circ \langle \llbracket \Theta' \supseteq \Theta \rrbracket \circ \pi_1, \pi_2 \rangle \\ &= \pi_2 \circ (\llbracket \Theta' \supseteq \Theta \rrbracket \times \text{id}) \\ &= \llbracket s : \sigma \in \Theta, s : \sigma \rrbracket \circ \llbracket \Theta', s : \sigma \supseteq \Theta, s : \sigma \rrbracket \end{aligned}$$

Otherwise, if  $\Theta', s' : \sigma' \supseteq \Theta, s : \sigma$  we have:

$$\begin{aligned} \llbracket s : \sigma \in \Theta', s' : \sigma' \rrbracket &= \llbracket s : \sigma \in \Theta' \rrbracket \circ \pi_1 \\ &= \llbracket s : \sigma \in \Theta, s : \sigma \rrbracket \circ \llbracket \Theta' \supseteq \Theta, s : \sigma \rrbracket \circ \pi_1 \\ &= \llbracket s : \sigma \in \Theta, s : \sigma \rrbracket \circ \llbracket \Theta', s' : \sigma' \supseteq \Theta, s : \sigma \rrbracket \end{aligned}$$

- $s : \sigma \in \Theta, s' : \sigma'$ :

We consider the case  $\Theta', s' : \sigma' \supseteq \Theta, s' : \sigma'$ :

$$\begin{aligned} \llbracket s : \sigma \in \Theta', s' : \sigma' \rrbracket &= \llbracket s : \sigma \in \Theta' \rrbracket \circ \pi_1 \\ &= \llbracket s : \sigma \in \Theta \rrbracket \circ \llbracket \Theta' \supseteq \Theta \rrbracket \circ \pi_1 \\ &= \llbracket s : \sigma \in \Theta \rrbracket \circ \pi_1 \circ (\llbracket \Theta' \supseteq \Theta \rrbracket \times \text{id}) \\ &= \llbracket s : \sigma \in \Theta, s' : \sigma' \rrbracket \circ \llbracket \Theta', s' : \sigma' \supseteq \Theta, s' : \sigma' \rrbracket \end{aligned}$$

□

### 11.1.2 Interpretation of index substitutions

**Definition 11.4.** We interpret an index substitution  $\Theta' \vdash_s \zeta \triangleright \Theta$  as a morphism  $\llbracket \zeta \rrbracket : \llbracket \Theta' \rrbracket \rightarrow \llbracket \Theta \rrbracket$  in the category  $\text{Ctx}$  of contexts:

$$\begin{aligned} \llbracket \Theta' \vdash_s \zeta \triangleright \cdot \rrbracket &\triangleq !_{[\Theta']} : \llbracket \Theta' \rrbracket \rightarrow 1 \\ \llbracket \Theta' \vdash_s \zeta, i \mapsto s \triangleright \Theta, i : \sigma \rrbracket &\triangleq \langle \llbracket \Theta' \vdash_s \zeta \triangleright \Theta \rrbracket, \llbracket \Theta' \vdash_s s : \sigma \rrbracket \rangle \end{aligned}$$

This follows the standard categorical semantics approach of interpreting substitutions as context morphisms, with the difference that we are working in a hyperdoctrine framework. Thus, substitutions will not be interpreted as composition (as  $\llbracket \zeta \rrbracket : \llbracket \Theta' \rrbracket \rightarrow \llbracket \Theta \rrbracket$  lives in  $\text{Ctx}$  rather than the category of Cartesian or linear types), but as a pullback via the reindexing functor  $\llbracket \zeta \rrbracket^* : \text{Set}^{[\Theta]} \rightarrow \text{Set}^{[\Theta']}$ .

**Lemma 11.5** (Semantics of index context extension). For a substitution  $\Theta' \vdash_s \zeta \triangleright \Theta$  and index  $i : \sigma$  with  $\zeta \# i$ , we have

$$\llbracket (\Theta', i : \sigma) \vdash_s \zeta, i \mapsto i \triangleright (\Theta, i : \sigma) \rrbracket = \llbracket \zeta \rrbracket \times \text{id}_{[\sigma]} : \llbracket \Theta' \rrbracket \times \llbracket \sigma \rrbracket \rightarrow \llbracket \Theta \rrbracket \times \llbracket \sigma \rrbracket$$

*Proof.* The crucial point of the proof is that the weakening lemma can only be applied once we “detached” the  $i \mapsto i$  mapping from the substitution, as otherwise  $i$  is not free.

$$\begin{aligned}
\llbracket (\Theta', i : \sigma) \vdash_s \zeta, i \mapsto i \triangleright (\Theta, i : \sigma) \rrbracket &= \langle \llbracket (\Theta', i : \sigma) \vdash_s \zeta \triangleright \Theta \rrbracket, \llbracket \Theta', i : \sigma \vdash_s i : \sigma \rrbracket \rangle \\
&= \langle \llbracket \Theta' \vdash_s \zeta \triangleright \Theta \rrbracket \circ \llbracket \Theta', i : \sigma \supseteq \Theta' \rrbracket, \pi_2 \rangle \\
&= \langle \llbracket \zeta \rrbracket \circ \pi_1, \pi_2 \rangle \\
&= \llbracket \zeta \rrbracket \times \text{id}_{\text{Id}}
\end{aligned}$$

□

**Theorem 11.6** (Soundness of index substitution into Cartesian types). If  $\Theta \vdash_c X$  type and  $\Theta' \vdash_s \zeta \triangleright \Theta$ , then

$$\llbracket \Theta' \vdash_c \zeta(X) \rrbracket = \llbracket \zeta \rrbracket^* \llbracket \Theta \vdash_c X \rrbracket$$

*Proof.* We proceed by induction on the derivation of the well-formed type judgment  $\Theta \vdash_c X$  type. The equalities follow from the definitions of interpretation, substitution and indexing, as well as (mutually) inductive hypotheses.

- ( $\Theta \vdash_c 1$  type): Interpretation of the unit type is independent of the index.

$$\llbracket \zeta \rrbracket^* \llbracket \Theta \vdash_c 1 \rrbracket = \llbracket \zeta \rrbracket^* (\mathbb{1}^{\text{Id}}) = \mathbb{1}^{\text{Id}} = \llbracket \Theta' \vdash_c 1 \rrbracket = \llbracket \Theta' \vdash_c \zeta(1) \rrbracket$$

- ( $\Theta \vdash_c X \rightarrow Y$  type):

$$\begin{aligned}
\llbracket \zeta \rrbracket^* \llbracket \Theta \vdash_c X \rightarrow Y \rrbracket &= \llbracket \zeta \rrbracket^* (\llbracket \Theta \vdash_c X \rrbracket \rightarrow^{\text{Id}} \llbracket \Theta \vdash_c Y \rrbracket) && \text{(semantics of } \rightarrow \text{)} \\
&= \llbracket \zeta \rrbracket^* \llbracket \Theta \vdash_c X \rrbracket \rightarrow^{\text{Id}} \llbracket \zeta \rrbracket^* \llbracket \Theta \vdash_c Y \rrbracket && (\llbracket \zeta \rrbracket^* \text{ is closed}) \\
&= \llbracket \Theta' \vdash_c \zeta(X) \rrbracket \rightarrow^{\text{Id}} \llbracket \Theta' \vdash_c \zeta(Y) \rrbracket && \text{(IH)} \\
&= \llbracket \Theta' \vdash_c \zeta(X) \rightarrow \zeta(Y) \rrbracket && \text{(semantics of } \rightarrow \text{)} \\
&= \llbracket \Theta' \vdash_c \zeta(X \rightarrow Y) \rrbracket && \text{(syntactic substitution)}
\end{aligned}$$

- ( $\Theta \vdash_c G A$  type):

$$\begin{aligned}
\llbracket \zeta \rrbracket^* \llbracket \Theta \vdash_c G A \rrbracket &= \llbracket \zeta \rrbracket^* (G^{\text{Id}} \llbracket \Theta \vdash_\ell A \rrbracket) && \text{(semantics of } G \text{)} \\
&= G^{\text{Id}} (\llbracket \zeta \rrbracket^+ \llbracket \Theta \vdash_\ell A \rrbracket) && \text{(LNL property)} \\
&= G^{\text{Id}} \llbracket \Theta' \vdash_\ell \zeta(A) \rrbracket && \text{(mutual IH)} \\
&= \llbracket \Theta' \vdash_c G(\zeta(A)) \rrbracket && \text{(semantics of } G \text{)} \\
&= \llbracket \Theta' \vdash_c \zeta(G A) \rrbracket && \text{(syntactic substitution)}
\end{aligned}$$

□

**Theorem 11.7** (Soundness of index substitution into linear types). If  $\Theta \vdash_\ell A$  type and  $\Theta' \vdash_s \zeta \triangleright \Theta$ , then

$$\llbracket \Theta' \vdash_\ell \zeta(A) \rrbracket = \llbracket \zeta \rrbracket^+ \llbracket \Theta \vdash_\ell A \rrbracket$$

*Proof.* We proceed by induction on the derivation of the well-formed type judgment  $\Theta \vdash_\ell A$  type. The equalities follow from the definitions of interpretation, substitution and indexing, as well as (mutually) inductive hypotheses.

- $(\Theta \vdash_\ell \mathbf{I} \text{ type})$ : Interpretation of the unit type is independent of the index.

$$[\![\zeta]\!]^+ [\![\Theta \vdash_\ell \mathbf{I}]\!] = [\![\zeta]\!]^+ (\mathbf{I}^{\text{[eq]}}) = \mathbf{I}^{\text{[eq]}} = [\![\Theta' \vdash_\ell \mathbf{I}]\!] = [\![\Theta' \vdash_\ell \zeta(\mathbf{I})]\!]$$

- $(\Theta \vdash_\ell A \otimes B \text{ type})$ :

$$\begin{aligned} [\![\zeta]\!]^+ [\![\Theta \vdash_\ell A \otimes B]\!] &= [\![\zeta]\!]^+ ([\![\Theta \vdash_\ell A]\!] \otimes^{\text{[eq]}} [\![\Theta \vdash_\ell B]\!]) && \text{(semantics of } \otimes) \\ &= [\![\zeta]\!]^+ [\![\Theta \vdash_\ell A]\!] \otimes^{\text{[eq]}} [\![\zeta]\!]^+ [\![\Theta \vdash_\ell B]\!] && ([\![\zeta]\!]^+ \text{ is monoidal}) \\ &= [\![\Theta' \vdash_\ell \zeta(A)]\!] \otimes^{\text{[eq]}} [\![\Theta' \vdash_\ell \zeta(B)]\!] && \text{(IH)} \\ &= [\![\Theta' \vdash_\ell \zeta(A) \otimes \zeta(B)]\!] && \text{(semantics of } \otimes) \\ &= [\![\Theta' \vdash_\ell \zeta(A \otimes B)]\!] && \text{(syntactic substitution)} \end{aligned}$$

- $(\Theta \vdash_\ell A \multimap B \text{ type})$ :

$$\begin{aligned} [\![\zeta]\!]^+ [\![\Theta \vdash_\ell A \multimap B]\!] &= [\![\zeta]\!]^+ ([\![\Theta \vdash_\ell A]\!] \multimap_{\mathcal{R}}^{\text{[eq]}} [\![\Theta \vdash_\ell B]\!]) && \text{(semantics of } \multimap) \\ &= [\![\zeta]\!]^+ [\![\Theta \vdash_\ell A]\!] \multimap_{\mathcal{R}}^{\text{[eq]}} [\![\zeta]\!]^+ [\![\Theta \vdash_\ell B]\!] && ([\![\zeta]\!]^+ \text{ is closed}) \\ &= [\![\Theta' \vdash_\ell \zeta(A)]\!] \multimap_{\mathcal{R}}^{\text{[eq]}} [\![\Theta' \vdash_\ell \zeta(B)]\!] && \text{(IH)} \\ &= [\![\Theta' \vdash_\ell \zeta(A) \multimap \zeta(B)]\!] && \text{(semantics of } \multimap) \\ &= [\![\Theta' \vdash_\ell \zeta(A \multimap B)]\!] && \text{(syntactic substitution)} \end{aligned}$$

- $(\Theta \vdash_\ell F X \text{ type})$ :

$$\begin{aligned} [\![\zeta]\!]^+ [\![\Theta \vdash_\ell F X]\!] &= [\![\zeta]\!]^+ (F^{\text{[eq]}} [\![\Theta \vdash_\ell X]\!]) && \text{(semantics of } F) \\ &= F^{\text{[eq]}} ([\![\zeta]\!]^* [\![\Theta \vdash_\ell X]\!]) && \text{(LNL property)} \\ &= F^{\text{[eq]}} [\![\Theta' \vdash_\ell \zeta(X)]\!] && \text{(mutual IH)} \\ &= [\![\Theta' \vdash_\ell F(\zeta(X))]\!] && \text{(semantics of } F) \\ &= [\![\Theta' \vdash_\ell \zeta(F X)]\!] && \text{(syntactic substitution)} \end{aligned}$$

- $(\Theta \vdash_\ell A @ \tau \text{ type})$ :

$$\begin{aligned} [\![\zeta]\!]^+ [\![\Theta \vdash_\ell A @ \tau]\!] &= [\![\zeta]\!]^+ (\triangleright^{\text{[eq]}} [\![\Theta \vdash_\ell A]\!]) && \text{(semantics of } @) \\ &= \triangleright^{\text{[eq]}} ([\![\zeta]\!]^+ [\![\Theta \vdash_\ell A]\!]) && \text{(reindexing of delays)} \\ &= \triangleright^{\text{[eq]}} [\![\Theta' \vdash_\ell \zeta(A)]\!] && \text{(IH)} \\ &= [\![\Theta' \vdash_\ell \zeta(A) @ \zeta(\tau)]\!] && \text{(semantics of } @) \\ &= [\![\Theta' \vdash_\ell \zeta(A @ \tau)]\!] && \text{(syntactic substitution)} \end{aligned}$$

- $(\Theta \vdash_\ell \Diamond A \text{ type})$ :

$$\begin{aligned} [\![\zeta]\!]^+ [\![\Theta \vdash_\ell \Diamond A]\!] &= [\![\zeta]\!]^+ (\Diamond^{\text{[eq]}} [\![\Theta \vdash_\ell A]\!]) && \text{(semantics of } \Diamond) \\ &= \Diamond^{\text{[eq]}} ([\![\zeta]\!]^+ [\![\Theta \vdash_\ell A]\!]) && \text{(reindexing of events)} \\ &= \Diamond^{\text{[eq]}} [\![\Theta' \vdash_\ell \zeta(A)]\!] && \text{(IH)} \\ &= [\![\Theta' \vdash_\ell \Diamond(\zeta(A))]\!] && \text{(semantics of } \Diamond) \\ &= [\![\Theta' \vdash_\ell \zeta(\Diamond A)]\!] && \text{(syntactic substitution)} \end{aligned}$$

- $(\Theta \vdash_\ell \text{Widget}^t \tau \iota \text{ type})$ :

$$\begin{aligned}
\llbracket \zeta \rrbracket^+ \llbracket \Theta \vdash_\ell \text{Widget}^t \tau \iota \rrbracket &= \llbracket \zeta \rrbracket^+ (\text{Widget}^t_{\llbracket \Theta \vdash_s \iota : \text{id} \rrbracket} \downarrow \llbracket \Theta \vdash_s \tau : \text{time} \rrbracket) && \text{(semantics of Widget)} \\
&= \text{Widget}^t_{\llbracket \zeta \rrbracket^+ \llbracket \Theta \vdash_s \iota : \text{id} \rrbracket} \downarrow \llbracket \zeta \rrbracket^+ \llbracket \Theta \vdash_s \tau : \text{time} \rrbracket && \text{(reindexing of widgets)} \\
&= \text{Widget}^t_{\llbracket \Theta \vdash_s \zeta(\iota) : \text{id} \rrbracket} \downarrow \llbracket \Theta \vdash_s \zeta(\tau) : \text{time} \rrbracket && \text{(reindexing application)} \\
&= \llbracket \Theta \vdash_\ell \text{Widget}^t \zeta(\tau) \zeta(\iota) \rrbracket && \text{(semantics of Widget)} \\
&= \llbracket \Theta \vdash_\ell \zeta(\text{Widget}^t \tau \iota) \rrbracket && \text{(syntactic substitution)}
\end{aligned}$$

- $(\Theta \vdash_\ell \forall i : \sigma. A \text{ type})$ :

$$\begin{aligned}
\llbracket \zeta \rrbracket^+ \llbracket \Theta \vdash_\ell \forall i : \sigma. A \rrbracket &= \llbracket \zeta \rrbracket^+ (\widehat{\mathbb{V}}_{[\Theta], [\sigma]} \llbracket \Theta, i : \sigma \vdash_\ell A \rrbracket) && \text{(semantics of } \forall) \\
&= \widehat{\mathbb{V}}_{[\Theta'], [\sigma]} ((\llbracket \zeta \rrbracket \times \text{id}_{[\sigma]})^+ \llbracket \Theta, i : \sigma \vdash_\ell A \rrbracket) && \text{(Beck–Chevalley condition)} \\
&= \widehat{\mathbb{V}}_{[\Theta'], [\sigma]} ((\llbracket (\Theta', i : \sigma) \vdash_s \zeta, i \mapsto i \triangleright (\Theta, i : \sigma) \rrbracket^+ \llbracket \Theta, i : \sigma \vdash_\ell A \rrbracket)) && \text{(Lemma 11.5)} \\
&= \widehat{\mathbb{V}}_{[\Theta'], [\sigma]} \llbracket \Theta', i : \sigma \vdash_\ell (\zeta, i \mapsto i)(A) \rrbracket && \text{(IH)} \\
&= \widehat{\mathbb{V}}_{[\Theta'], [\sigma]} \llbracket \Theta', i : \sigma \vdash_\ell \zeta(A) \rrbracket && \text{(identity substitution)} \\
&= \llbracket \Theta' \vdash_\ell \forall i : \sigma. \zeta(A) \rrbracket && \text{(semantics of } \forall) \\
&= \llbracket \Theta' \vdash_\ell \zeta(\forall i : \sigma. A) \rrbracket && \text{(syntactic substitution } (\zeta \# i))
\end{aligned}$$

- $(\Theta \vdash_\ell \exists i : \sigma. A \text{ type})$ :

$$\begin{aligned}
\llbracket \zeta \rrbracket^+ \llbracket \Theta \vdash_\ell \exists i : \sigma. A \rrbracket &= \llbracket \zeta \rrbracket^+ (\widehat{\mathbb{V}}_{[\Theta], [\sigma]} \llbracket \Theta, i : \sigma \vdash_\ell A \rrbracket) && \text{(semantics of } \exists) \\
&= \widehat{\mathbb{V}}_{[\Theta'], [\sigma]} ((\llbracket \zeta \rrbracket \times \text{id}_{[\sigma]})^+ \llbracket \Theta, i : \sigma \vdash_\ell A \rrbracket) && \text{(Beck–Chevalley condition)} \\
&= \widehat{\mathbb{V}}_{[\Theta'], [\sigma]} ((\llbracket (\Theta', i : \sigma) \vdash_s \zeta, i \mapsto i \triangleright (\Theta, i : \sigma) \rrbracket^+ \llbracket \Theta, i : \sigma \vdash_\ell A \rrbracket)) && \text{(Lemma 11.5)} \\
&= \widehat{\mathbb{V}}_{[\Theta'], [\sigma]} \llbracket \Theta', i : \sigma \vdash_\ell (\zeta, i \mapsto i)(A) \rrbracket && \text{(IH)} \\
&= \widehat{\mathbb{V}}_{[\Theta'], [\sigma]} \llbracket \Theta', i : \sigma \vdash_\ell \zeta(A) \rrbracket && \text{(identity substitution)} \\
&= \llbracket \Theta' \vdash_\ell \exists i : \sigma. \zeta(A) \rrbracket && \text{(semantics of } \exists) \\
&= \llbracket \Theta' \vdash_\ell \zeta(\exists i : \sigma. A) \rrbracket && \text{(syntactic substitution } (\zeta \# i))
\end{aligned}$$

□

**Theorem 11.8** (Soundness of index substitution into Cartesian terms). If  $\Theta \mid \Gamma \vdash_c e : X$  and  $\Theta' \vdash_s \zeta \triangleright \Theta$ , then

$$\llbracket \Theta' \mid \zeta(\Gamma) \vdash_c \zeta(e) : \zeta(X) \rrbracket = \llbracket \zeta \rrbracket^* \llbracket \Theta \mid \Gamma \vdash_c e : X \rrbracket$$

*Proof.* We proceed by induction on the derivation of the well-formed type judgment  $\Theta \mid \Gamma \vdash_c e : X$ . The precomposition steps rely on the soundness of index substitution into Cartesian types.

- $(\Theta \mid \Gamma \vdash_c \star : 1)$ :

$$\llbracket \zeta \rrbracket^* \llbracket \Theta \mid \Gamma \vdash_c \star : 1 \rrbracket = \llbracket \zeta \rrbracket^* (!_{[\Theta \vdash_c \Gamma]}^{[\Theta]} : \llbracket \Theta \vdash_c \Gamma \rrbracket \rightarrow^{[\Theta]} \mathbb{1}^{[\Theta]}) \quad \text{(semantics of } \star : 1)$$

$$\begin{aligned}
&= !_{\llbracket \Theta' \vdash_c \zeta(\Gamma) \rrbracket}^{\llbracket \Theta' \rrbracket} : \llbracket \Theta' \vdash_c \zeta(\Gamma) \rrbracket \rightarrow^{\llbracket \Theta' \rrbracket} \mathbb{1}^{\llbracket \Theta' \rrbracket} && \text{(precomposition)} \\
&= \llbracket \Theta' \mid \zeta(\Gamma) \vdash_c \star : 1 \rrbracket && \text{(semantics of } \star : 1 \text{)} \\
&= \llbracket \Theta' \mid \zeta(\Gamma) \vdash_c \zeta(\star) : \zeta(1) \rrbracket && \text{(syntactic substitution)}
\end{aligned}$$

- $(\Theta \mid \Gamma, x : X \vdash_c x : X)$ :

$$\begin{aligned}
&\llbracket \zeta \rrbracket^* \llbracket \Theta \mid \Gamma, x : X \vdash_c x : X \rrbracket \\
&= \llbracket \zeta \rrbracket^* (\pi_2^{\llbracket \Theta \rrbracket} : \llbracket \Theta \vdash_c \Gamma, x : X \rrbracket \rightarrow^{\llbracket \Theta \rrbracket} \llbracket \Theta \vdash_c X \rrbracket) && \text{(semantics of } x : X \text{)} \\
&= \pi_2^{\llbracket \Theta' \rrbracket} : \llbracket \Theta' \vdash_c \zeta(\Gamma), \zeta(x) : \zeta(X) \rrbracket \rightarrow^{\llbracket \Theta' \rrbracket} \llbracket \Theta' \vdash_c \zeta(X) \rrbracket && \text{(precomposition)} \\
&= \llbracket \Theta' \mid \zeta(\Gamma), \zeta(x) : \zeta(X) \vdash_c \zeta(x) : \zeta(X) \rrbracket && \text{(semantics of } \zeta(x) : \zeta(X) \text{)} \\
&= \llbracket \Theta' \mid \zeta(\Gamma, x : X) \vdash_c \zeta(x) : \zeta(X) \rrbracket && \text{(syntactic substitution)}
\end{aligned}$$

- $(\Theta \mid \Gamma, y : Y \vdash_c x : X)$ :

$$\begin{aligned}
&\llbracket \zeta \rrbracket^* \llbracket \Theta \mid \Gamma, y : Y \vdash_c x : X \rrbracket \\
&= \llbracket \zeta \rrbracket^* (\llbracket \Theta \mid \Gamma \vdash_c x : X \rrbracket \circ \pi_1^{\llbracket \Theta \rrbracket} : \llbracket \Theta \vdash_c \Gamma, y : Y \rrbracket \rightarrow^{\llbracket \Theta \rrbracket} \llbracket \Theta \vdash_c X \rrbracket) && \text{(semantics of } x : X \text{)} \\
&= (\llbracket \zeta \rrbracket^* \llbracket \Theta \mid \Gamma \vdash_c x : X \rrbracket) \circ (\llbracket \zeta \rrbracket^* \pi_1^{\llbracket \Theta \rrbracket} : \llbracket \Theta' \vdash_c \zeta(\Gamma), x : \zeta(X) \rrbracket \rightarrow^{\llbracket \Theta' \rrbracket} \llbracket \Theta' \vdash_c \zeta(X) \rrbracket) && \text{(functoriality of } \llbracket \zeta \rrbracket^* \text{)} \\
&= (\llbracket \Theta \mid \zeta(\Gamma) \vdash_c \zeta(x) : \zeta(X) \rrbracket) \circ (\llbracket \zeta \rrbracket^* \pi_1^{\llbracket \Theta \rrbracket}) && \text{(IH)} \\
&= (\llbracket \Theta \mid \zeta(\Gamma) \vdash_c \zeta(x) : \zeta(X) \rrbracket) \circ \pi_1^{\llbracket \Theta \rrbracket} && \text{(precomposition)} \\
&= \llbracket \Theta' \mid \zeta(\Gamma), \zeta(y) : \zeta(Y) \vdash_c \zeta(x) : \zeta(X) \rrbracket && \text{(semantics of } \zeta(x) : \zeta(X) \text{)} \\
&= \llbracket \Theta' \mid \zeta(\Gamma, y : Y) \vdash_c \zeta(x) : \zeta(X) \rrbracket && \text{(syntactic substitution)}
\end{aligned}$$

- $(\Theta \mid \Gamma \vdash_c \lambda x. e : X \rightarrow Y)$ :

$$\begin{aligned}
&\llbracket \zeta \rrbracket^* \llbracket \Theta \mid \Gamma \vdash_c \lambda x. e : X \rightarrow Y \rrbracket \\
&= \llbracket \zeta \rrbracket^* (\text{curry}^{\llbracket \Theta \rrbracket} \llbracket \Theta \mid \Gamma, x : X \vdash_c e : Y \rrbracket) && \text{(semantics of } \lambda x. e : X \rightarrow Y \text{)} \\
&= \text{curry}^{\llbracket \Theta' \rrbracket} (\llbracket \zeta \rrbracket^* \llbracket \Theta \mid \Gamma, x : X \vdash_c e : Y \rrbracket) && \text{(precomposition)} \\
&= \text{curry}^{\llbracket \Theta' \rrbracket} \llbracket \Theta' \mid \zeta(\Gamma), x : \zeta(X) \vdash_c \zeta(e) : \zeta(Y) \rrbracket && \text{(IH)} \\
&= \llbracket \Theta' \mid \zeta(\Gamma) \vdash_c \lambda x. \zeta(e) : \zeta(X) \rightarrow \zeta(Y) \rrbracket && \text{(semantics of } \lambda x. \zeta(e) : \zeta(X) \rightarrow \zeta(Y) \text{)} \\
&= \llbracket \Theta' \mid \zeta(\Gamma) \vdash_c \zeta(\lambda x. e) : \zeta(X \rightarrow Y) \rrbracket && \text{(syntactic substitution } (\zeta \# x) \text{)}
\end{aligned}$$

- $(\Theta \mid \Gamma \vdash_c e_1 e_2 : Y)$ :

$$\begin{aligned}
&\llbracket \zeta \rrbracket^* \llbracket \Theta \mid \Gamma \vdash_c e_1 e_2 : Y \rrbracket \\
&= \llbracket \zeta \rrbracket^* (\text{eval}^{\llbracket \Theta \rrbracket} \circ \langle \llbracket \Theta \mid \Gamma \vdash_c e_1 : X \rightarrow Y \rrbracket, \llbracket \Theta \mid \Gamma \vdash_c e_2 : X \rrbracket \rangle^{\llbracket \Theta \rrbracket}) && \text{(semantics of } e_1 e_2 : Y \text{)} \\
&= \text{eval}^{\llbracket \Theta' \rrbracket} \circ \langle \llbracket \zeta \rrbracket^* \llbracket \Theta \mid \Gamma \vdash_c e_1 : X \rightarrow Y \rrbracket, \llbracket \zeta \rrbracket^* \llbracket \Theta \mid \Gamma \vdash_c e_2 : X \rrbracket \rangle^{\llbracket \Theta' \rrbracket} && \text{(precomposition)} \\
&= \text{eval}^{\llbracket \Theta' \rrbracket} \circ \langle \llbracket \Theta' \mid \zeta(\Gamma) \vdash_c \zeta(e_1) : \zeta(X \rightarrow Y) \rrbracket, \llbracket \Theta' \mid \zeta(\Gamma) \vdash_c \zeta(e_2) : \zeta(X) \rrbracket \rangle^{\llbracket \Theta' \rrbracket} && \text{(IH)} \\
&= \text{eval}^{\llbracket \Theta' \rrbracket} \circ \langle \llbracket \Theta' \mid \zeta(\Gamma) \vdash_c \zeta(e_1) : \zeta(X) \rightarrow \zeta(Y) \rrbracket, \llbracket \Theta' \mid \zeta(\Gamma) \vdash_c \zeta(e_2) : \zeta(X) \rrbracket \rangle^{\llbracket \Theta' \rrbracket} && \text{(syntactic substitution)} \\
&= \llbracket \Theta' \mid \zeta(\Gamma) \vdash_c \zeta(e_1) \zeta(e_2) : \zeta(Y) \rrbracket && \text{(semantics of } \zeta(e_1) \zeta(e_2) : \zeta(Y) \text{)} \\
&= \llbracket \Theta' \mid \zeta(\Gamma) \vdash_c \zeta(e_1 e_2) : \zeta(Y) \rrbracket && \text{(syntactic substitution)}
\end{aligned}$$

- $(\Theta \mid \Gamma \vdash_c \mathbf{G} \, t : \mathbf{G} \, A)$ :

$$\begin{aligned}
& \llbracket \zeta \rrbracket^* \llbracket \Theta \mid \Gamma \vdash_c \mathbf{G} \, t : \mathbf{G} \, A \rrbracket \\
&= \llbracket \zeta \rrbracket^* \left( G^{[\Theta]} \left( \llbracket \Theta \mid \Gamma; \cdot \vdash_\ell t : A \rrbracket \circ \rho_{F^{[\Theta]} \llbracket \Theta \vdash_c \Gamma \rrbracket}^{-1} \right) \circ \eta_{\llbracket \Theta \vdash_c \Gamma \rrbracket}^{[\Theta]} \right) \quad (\text{semantics of } \mathbf{G} \, t : \mathbf{G} \, A) \\
&= \llbracket \zeta \rrbracket^* G^{[\Theta]} \left( \llbracket \Theta \mid \Gamma; \cdot \vdash_\ell t : A \rrbracket \circ \rho_{F^{[\Theta]} \llbracket \Theta \vdash_c \Gamma \rrbracket}^{-1} \right) \circ \llbracket \zeta \rrbracket^* \eta_{\llbracket \Theta \vdash_c \Gamma \rrbracket}^{[\Theta]} \quad (\text{functoriality}) \\
&= G^{[\Theta]} \llbracket \zeta \rrbracket^+ \left( \llbracket \Theta \mid \Gamma; \cdot \vdash_\ell t : A \rrbracket \circ \rho_{F^{[\Theta]} \llbracket \Theta \vdash_c \Gamma \rrbracket}^{-1} \right) \circ \eta_{\llbracket \zeta \rrbracket^* \llbracket \Theta \vdash_c \Gamma \rrbracket}^{[\Theta]} \quad (\text{LNL properties}) \\
&= G^{[\Theta']} \left( \llbracket \zeta \rrbracket^+ \llbracket \Theta \mid \Gamma; \cdot \vdash_\ell t : A \rrbracket \circ \llbracket \zeta \rrbracket^+ \rho_{F^{[\Theta]} \llbracket \Theta \vdash_c \Gamma \rrbracket}^{-1} \right) \circ \eta_{\llbracket \zeta \rrbracket^* \llbracket \Theta \vdash_c \Gamma \rrbracket}^{[\Theta']} \quad (\text{functoriality}) \\
&= G^{[\Theta']} \left( \llbracket \Theta' \mid \zeta(\Gamma); \cdot \vdash_\ell \zeta(t) : \zeta(A) \rrbracket \circ \rho_{\llbracket \zeta \rrbracket^+ F^{[\Theta]} \llbracket \Theta \vdash_c \Gamma \rrbracket}^{-1} \right) \circ \eta_{\llbracket \zeta \rrbracket^* \llbracket \Theta \vdash_c \Gamma \rrbracket}^{[\Theta']} \\
&\quad (\text{mutual IH and precomposition}) \\
&= G^{[\Theta']} \left( \llbracket \Theta' \mid \zeta(\Gamma); \cdot \vdash_\ell \zeta(t) : \zeta(A) \rrbracket \circ \rho_{F^{[\Theta']} \llbracket \Theta' \vdash_c \zeta(\Gamma) \rrbracket}^{-1} \right) \circ \eta_{\llbracket \zeta \rrbracket^* \llbracket \Theta' \vdash_c \zeta(\Gamma) \rrbracket}^{[\Theta']} \\
&\quad (\text{LNL properties and soundness of subst. into types}) \\
&= \llbracket \Theta' \mid \Gamma' \vdash_c \mathbf{G} \, (\zeta(t)) : \mathbf{G} \, \zeta(A) \rrbracket \quad (\text{semantics of } \mathbf{G} \, (\zeta(t)) : \mathbf{G} \, \zeta(A)) \\
&= \llbracket \Theta' \mid \zeta(\Gamma) \vdash_c \zeta(\mathbf{G} \, t) : \zeta(\mathbf{G} \, A) \rrbracket \quad (\text{syntactic substitution})
\end{aligned}$$

□

To prove soundness of index substitution into linear terms, we need some lemmas concerning the interaction of substitution and the helper functions **drop** and **split**.

**Lemma 11.9.** For a substitution  $\Theta' \vdash_s \zeta \triangleright \Theta$  and contexts  $\Theta, \Gamma$  and  $\Delta$ , we have:

$$\begin{aligned}
& \llbracket \zeta \rrbracket^+ \zeta^{[\Theta]} = \zeta^{[\Theta']} \\
& \llbracket \zeta \rrbracket^+ \mathbf{drop}_{\Theta, \Gamma, \Delta} = \mathbf{drop}_{\Theta', \zeta(\Gamma), \zeta(\Delta)} \\
& \llbracket \zeta \rrbracket^+ \mathbf{split}_{\Theta, \Gamma, \Delta_1, \Delta_2} = \mathbf{split}_{\Theta', \zeta(\Gamma), \zeta(\Delta_1), \zeta(\Delta_2)}
\end{aligned}$$

*Proof.* Reindexing and application of definitions. □

**Theorem 11.10** (Soundness of index substitution into linear terms). If  $\Theta \mid \Gamma; \Delta \vdash_\ell t :_\tau A$  and  $\Theta' \vdash_s \zeta \triangleright \Theta$ , then

$$\llbracket \zeta \rrbracket^+ \llbracket \Theta \mid \Gamma; \Delta \vdash_\ell t :_\tau A \rrbracket = \llbracket \Theta' \mid \zeta(\Gamma); \zeta(\Delta) \vdash_\ell \zeta(t) :_{\zeta(\tau)} \zeta(A) \rrbracket$$

*Proof.* We proceed by induction on the derivation of the well-formed type judgment  $\Theta \mid \Gamma; \Delta \vdash_\ell t :_\tau A$ . The precomposition steps rely on the soundness of index substitution into linear types.

- $(\Theta \mid \Gamma; \Delta \vdash_\ell \langle \rangle : \mathbf{I})$ :

$$\begin{aligned}
\llbracket \zeta \rrbracket^+ \llbracket \Theta \mid \Gamma; \Delta \vdash_\ell \langle \rangle : \mathbf{I} \rrbracket &= \llbracket \zeta \rrbracket^+ \mathbf{drop}_{\Theta, \Gamma, \Delta} && (\text{semantics of } \langle \rangle : \mathbf{I}) \\
&= \mathbf{drop}_{\Theta', \zeta(\Gamma), \zeta(\Delta)} && (\text{Lemma 11.9}) \\
&= \llbracket \Theta' \mid \zeta(\Gamma); \zeta(\Delta) \vdash_\ell \zeta(\langle \rangle) : \zeta(\mathbf{I}) \rrbracket && (\text{semantics of } \langle \rangle : \mathbf{I})
\end{aligned}$$



- $(\Theta \mid \Gamma; a : A \vdash_\ell a : A)$ :

$$\begin{aligned}
& \llbracket \zeta \rrbracket^* \llbracket \Theta \mid \Gamma; a : A \vdash_\ell a : A \rrbracket \\
&= \llbracket \zeta \rrbracket^+ \mathbf{drop}_{\Theta, \Gamma, a : A} && \text{(semantics of } a : A \text{)} \\
&= \mathbf{drop}_{\Theta', \zeta(\Gamma), a : \zeta(A)} && \text{(Lemma 11.9)} \\
&= \llbracket \Theta \mid \Gamma; a : \zeta(A) \vdash_\ell \zeta(a) : \zeta(A) \rrbracket && \text{(semantics of } a : A \text{)}
\end{aligned}$$

- $(\Theta \mid \Gamma; \Delta \vdash_\ell \lambda a. t : A \multimap B)$ :

$$\begin{aligned}
& \llbracket \zeta \rrbracket^+ \llbracket \Theta \mid \Gamma; \Delta \vdash_\ell \lambda a. t : A \multimap B \rrbracket \\
&= \llbracket \zeta \rrbracket^+ (\mathbf{curry}^{\text{eq}} \llbracket \Theta \mid \Gamma; \Delta, a : A \vdash_\ell t : B \rrbracket) && \text{(semantics of } \lambda a. t : A \multimap B \text{)} \\
&= \mathbf{curry}^{\text{eq}'} (\llbracket \zeta \rrbracket^+ \llbracket \Theta \mid \Gamma; \Delta, a : A \vdash_\ell t : B \rrbracket) && \text{(precomposition)} \\
&= \mathbf{curry}^{\text{eq}'} \llbracket \Theta' \mid \zeta(\Gamma); \zeta(\Delta), a : \zeta(A) \vdash_\ell \zeta(t) : \zeta(B) \rrbracket && \text{(IH)} \\
&= \llbracket \Theta' \mid \zeta(\Gamma); \zeta(\Delta) \vdash_\ell \lambda a. \zeta(t) : \zeta(A) \multimap \zeta(B) \rrbracket && \text{(semantics of } \lambda a. \zeta(t) : \zeta(A) \multimap \zeta(B) \text{)} \\
&= \llbracket \Theta' \mid \zeta(\Gamma); \zeta(\Delta) \vdash_\ell \zeta(\lambda a. T) : \zeta(A \multimap B) \rrbracket && \text{(syntactic substitution } (\zeta \# x) \text{)}
\end{aligned}$$

- $(\Theta \mid \Gamma; \Delta \vdash_\ell t_1 t_2 : B)$ :

$$\begin{aligned}
& \llbracket \zeta \rrbracket^+ \llbracket \Theta \mid \Gamma; \Delta \vdash_\ell t_1 t_2 : B \rrbracket \\
&= \llbracket \zeta \rrbracket^+ (\mathbf{eval}^{\text{eq}} \circ (\llbracket t_1 \rrbracket \otimes^{\text{eq}} \llbracket t_2 \rrbracket) \circ \mathbf{split}_{\Theta, \Gamma, \Delta_1, \Delta_2}) && \text{(semantics of } t_1 t_2 : B \text{)} \\
&= \mathbf{eval}^{\text{eq}'} \circ (\llbracket \zeta \rrbracket^+ \llbracket t_1 \rrbracket \otimes^{\text{eq}'} \llbracket \zeta \rrbracket^+ \llbracket t_2 \rrbracket) \circ \mathbf{split}_{\Theta', \zeta(\Gamma), \zeta(\Delta_1), \zeta(\Delta_2)} && \text{(precomposition and Lemma 11.9)} \\
&= \mathbf{eval}^{\text{eq}'} \circ (\llbracket \zeta(t_1) \rrbracket \otimes^{\text{eq}'} \llbracket \zeta(t_2) \rrbracket) \circ \mathbf{split}_{\Theta', \zeta(\Gamma), \zeta(\Delta_1), \zeta(\Delta_2)} && \text{(IH)} \\
&= \llbracket \Theta' \mid \zeta(\Gamma); \zeta(\Delta) \vdash_\ell \zeta(t_1) \zeta(t_2) : \zeta(B) \rrbracket && \text{(semantics of } \zeta(t_1) \zeta(t_2) : \zeta(B) \text{)} \\
&= \llbracket \Theta' \mid \zeta(\Gamma); \zeta(\Delta) \vdash_\ell \zeta(t_1 t_2) : \zeta(B) \rrbracket && \text{(syntactic substitution)}
\end{aligned}$$

- $(\Theta \mid \Gamma; \Delta \vdash_\ell \text{let } \langle \rangle = t_1 \text{ in } t_2 : B)$ :

$$\begin{aligned}
& \llbracket \zeta \rrbracket^+ \llbracket \Theta \mid \Gamma; \Delta_1, \Delta_2 \vdash_\ell \text{let } \langle \rangle = t_1 \text{ in } t_2 : B \rrbracket \\
&= \llbracket \zeta \rrbracket^+ (\lambda_{\llbracket \Theta \vdash_\ell B \rrbracket}^{\text{eq}} \circ (\llbracket t_1 \rrbracket \otimes^{\text{eq}} \llbracket t_2 \rrbracket) \circ \mathbf{split}_{\Theta, \Gamma, \Delta_1, \Delta_2}) && \text{(semantics of unit binding)} \\
&= \lambda_{\llbracket \Theta' \vdash_\ell B \rrbracket}^{\text{eq}'} \circ (\llbracket \zeta \rrbracket^+ \llbracket t_1 \rrbracket \otimes^{\text{eq}'} \llbracket \zeta \rrbracket^+ \llbracket t_2 \rrbracket) \circ \mathbf{split}_{\Theta', \zeta(\Gamma), \zeta(\Delta_1), \zeta(\Delta_2)} && \text{(precomposition and Lemma 11.9)} \\
&= \lambda_{\llbracket \Theta' \vdash_\ell B \rrbracket}^{\text{eq}'} \circ (\llbracket \zeta(t_1) \rrbracket \otimes^{\text{eq}'} \llbracket \zeta(t_2) \rrbracket) \circ \mathbf{split}_{\Theta', \zeta(\Gamma), \zeta(\Delta_1), \zeta(\Delta_2)} && \text{(IH)} \\
&= \llbracket \Theta' \mid \zeta(\Gamma); \zeta(\Delta_1), \zeta(\Delta_2) \vdash_\ell \text{let } \langle \rangle = \zeta(t_1) \text{ in } \zeta(t_2) : \zeta(B) \rrbracket && \text{(semantics of unit binding)} \\
&= \llbracket \Theta' \mid \zeta(\Gamma); \zeta(\Delta_1, \Delta_2) \vdash_\ell \zeta(\text{let } \langle \rangle = t_1 \text{ in } t_2) : \zeta(B) \rrbracket && \text{(syntactic substitution)}
\end{aligned}$$

- $(\Theta \mid \Gamma; \Delta \vdash_\ell (t_1, t_2) : A \otimes B)$ :

$$\begin{aligned}
& \llbracket \zeta \rrbracket^+ \llbracket \Theta \mid \Gamma; \Delta_1, \Delta_2 \vdash_\ell (t_1, t_2) : A \otimes B \rrbracket \\
&= \llbracket \zeta \rrbracket^+ ((\llbracket t_1 \rrbracket \otimes^{\text{eq}} \llbracket t_2 \rrbracket) \circ \mathbf{split}_{\Theta, \Gamma, \Delta_1, \Delta_2}) && \text{(semantics of pairing)} \\
&= (\llbracket \zeta \rrbracket^+ \llbracket t_1 \rrbracket \otimes^{\text{eq}'} \llbracket \zeta \rrbracket^+ \llbracket t_2 \rrbracket) \circ \mathbf{split}_{\Theta', \zeta(\Gamma), \zeta(\Delta_1), \zeta(\Delta_2)} && \text{(precomposition and Lemma 11.9)}
\end{aligned}$$

$$\begin{aligned}
&= (\llbracket \zeta(t_1) \rrbracket \otimes^{\text{I}^{\Theta'}} \llbracket \zeta(t_2) \rrbracket) \circ \text{split}_{\Theta', \zeta(\Gamma), \zeta(\Delta_1), \zeta(\Delta_2)} && \text{(IH)} \\
&= \llbracket \Theta' \mid \zeta(\Gamma); \zeta(\Delta_1), \zeta(\Delta_2) \vdash_{\ell} (\zeta(t_1), \zeta(t_2)) : \zeta(A) \otimes \zeta(B) \rrbracket && \text{(semantics of pairing)} \\
&= \llbracket \Theta' \mid \zeta(\Gamma); \zeta(\Delta_1, \Delta_2) \vdash_{\ell} \zeta((t_1, t_2)) : \zeta(A \otimes B) \rrbracket && \text{(syntactic substitution)}
\end{aligned}$$

- $(\Theta \mid \Gamma; \Delta \vdash_{\ell} \text{let } (a, b) = t_1 \text{ in } t_2 : C)$ :

$$\begin{aligned}
&\llbracket \zeta \rrbracket^+ \llbracket \Theta \mid \Gamma; \Delta \vdash_{\ell} \text{let } (a, b) = t_1 \text{ in } t_2 : C \rrbracket \\
&= \llbracket \zeta \rrbracket^+ (\llbracket t_2 \rrbracket \circ \zeta^{\text{I}^{\Theta}} \circ (\llbracket t_1 \rrbracket \otimes^{\text{I}^{\Theta}} \text{id}) \circ \text{split}_{\Theta, \Gamma, \Delta_1, \Delta_2}) && \text{(semantics of pair binding)} \\
&= (\llbracket \zeta \rrbracket^+ \llbracket t_2 \rrbracket \circ \zeta^{\text{I}^{\Theta'}} \circ (\llbracket \zeta \rrbracket^+ \llbracket t_1 \rrbracket \otimes^{\text{I}^{\Theta'}} \llbracket \zeta \rrbracket^+ \text{id}) \circ \text{split}_{\Theta', \zeta(\Gamma), \zeta(\Delta_1), \zeta(\Delta_2)}) && \text{(precomposition and Lemma 11.9)} \\
&= (\llbracket \zeta(t_2) \rrbracket \circ \zeta^{\text{I}^{\Theta'}} \circ (\llbracket \zeta(t_1) \rrbracket \otimes^{\text{I}^{\Theta'}} \text{id}) \circ \text{split}_{\Theta', \zeta(\Gamma), \zeta(\Delta_1), \zeta(\Delta_2)}) && \text{(IH)} \\
&= \llbracket \Theta' \mid \zeta(\Gamma); \zeta(\Delta_1), \zeta(\Delta_2) \vdash_{\ell} \text{let } (a, b) = \zeta(t_1) \text{ in } \zeta(t_2) : \zeta(C) \rrbracket && \text{(semantics of pair binding)} \\
&= \llbracket \Theta' \mid \zeta(\Gamma); \zeta(\Delta_1, \Delta_2) \vdash_{\ell} \zeta(\text{let } (a, b) = t_1 \text{ in } t_2 : C) \rrbracket && \text{(syntactic substitution)}
\end{aligned}$$

- $(\Theta \mid \Gamma; \Delta \vdash_{\ell} \text{evt } t : \Diamond A)$ :

$$\begin{aligned}
&\llbracket \zeta \rrbracket^+ \llbracket \Theta \mid \Gamma; \Delta \vdash_{\ell} \text{evt } t : \Diamond A \rrbracket \\
&= \llbracket \zeta \rrbracket^+ (\eta_{\llbracket \Theta \vdash_{\ell} A \rrbracket}^{\text{I}^{\Theta}} \circ \llbracket t \rrbracket) && \text{(semantics of events)} \\
&= \llbracket \zeta \rrbracket^+ \eta_{\llbracket \Theta \vdash_{\ell} A \rrbracket}^{\text{I}^{\Theta}} \circ \llbracket \zeta \rrbracket^+ \llbracket t \rrbracket && \text{(precomposition)} \\
&= \eta_{\llbracket \Theta \vdash_{\ell} A \rrbracket}^{\text{I}^{\Theta'}} \circ \llbracket \zeta(t) \rrbracket && \text{(IH)} \\
&= \llbracket \Theta' \mid \zeta(\Gamma); \zeta(\Delta) \vdash_{\ell} \text{evt } \zeta(t) : \Diamond(\zeta(A)) \rrbracket && \text{(semantics of events)} \\
&= \llbracket \Theta' \mid \zeta(\Gamma); \zeta(\Delta) \vdash_{\ell} \zeta(\text{evt } t) : \zeta(\Diamond A) \rrbracket && \text{(syntactic substitution)}
\end{aligned}$$

- $(\Theta \mid \Gamma; \Delta \vdash_{\ell} \text{let evt } a = t_1 \text{ in } t_2 : \Diamond B)$ :

$$\begin{aligned}
&\llbracket \zeta \rrbracket^+ \llbracket \Theta \mid \Gamma; \Delta \vdash_{\ell} \text{let evt } a = t_1 \text{ in } t_2 : \Diamond B \rrbracket \\
&= \llbracket \zeta \rrbracket^+ (\mu_{\llbracket \Theta \vdash_{\ell} B \rrbracket}^{\text{I}^{\Theta}} \circ \Diamond^{\text{I}^{\Theta}} \llbracket t_2 \rrbracket \circ \text{st}_{\llbracket \Theta \vdash_c \Gamma \rrbracket, \llbracket \Theta \vdash_{\ell} \Delta \rrbracket}^{\text{I}^{\Theta}} \circ (\text{id} \otimes^{\text{I}^{\Theta}} \llbracket t_1 \rrbracket) \circ \zeta^{\text{I}^{\Theta}} \circ (\text{dup}_{\llbracket \Theta \vdash_c \Gamma \rrbracket} \otimes^{\text{I}^{\Theta}} \text{id})) && \text{(semantics of event binding)} \\
&= \mu_{\llbracket \Theta \vdash_{\ell} B \rrbracket}^{\text{I}^{\Theta'}} \circ \Diamond^{\text{I}^{\Theta'}} (\llbracket \zeta \rrbracket^+ \llbracket t_2 \rrbracket) \circ \text{st}_{\llbracket \zeta \rrbracket^+ \llbracket \Theta \vdash_c \Gamma \rrbracket, \llbracket \zeta \rrbracket^+ \llbracket \Theta \vdash_{\ell} \Delta \rrbracket}^{\text{I}^{\Theta'}} \circ (\text{id} \otimes^{\text{I}^{\Theta'}} \llbracket \zeta \rrbracket^+ \llbracket t_1 \rrbracket) \circ \zeta^{\text{I}^{\Theta'}} \circ (\text{dup}_{\llbracket \zeta \rrbracket^+ \llbracket \Theta \vdash_c \Gamma \rrbracket} \otimes^{\text{I}^{\Theta'}} \text{id}) && \text{(precomposition)} \\
&= \mu_{\llbracket \Theta \vdash_{\ell} B \rrbracket}^{\text{I}^{\Theta'}} \circ \Diamond^{\text{I}^{\Theta'}} \llbracket \zeta(t_2) \rrbracket \circ \text{st}_{\llbracket \Theta \vdash_c \zeta(\Gamma) \rrbracket, \llbracket \Theta \vdash_{\ell} \zeta(\Delta) \rrbracket}^{\text{I}^{\Theta'}} \circ (\text{id} \otimes^{\text{I}^{\Theta'}} \llbracket \zeta(t_1) \rrbracket) \circ \zeta^{\text{I}^{\Theta'}} \circ (\text{dup}_{\llbracket \Theta \vdash_c \zeta(\Gamma) \rrbracket} \otimes^{\text{I}^{\Theta'}} \text{id}) && \text{(IH and soundness of index substitution into types)} \\
&= \llbracket \Theta' \mid \zeta(\Gamma); \zeta(\Delta) \vdash_{\ell} \text{let evt } a = \zeta(t_1) \text{ in } \zeta(t_2) : \Diamond(\zeta(B)) \rrbracket && \text{(semantics of event binding)} \\
&= \llbracket \Theta' \mid \zeta(\Gamma); \zeta(\Delta) \vdash_{\ell} \zeta(\text{let evt } a = t_1 \text{ in } t_2 : \Diamond B) \rrbracket && \text{(syntactic substitution)}
\end{aligned}$$

- $(\Theta \mid \Gamma; \Delta \vdash_{\ell} t @ \tau : A @ \tau)$ :

$$\begin{aligned}
&\llbracket \zeta \rrbracket^+ \llbracket \Theta \mid \Gamma; \Delta \vdash_{\ell} t @ \tau : A @ \tau \rrbracket \\
&= \llbracket \zeta \rrbracket^+ \llbracket \Theta \mid \Gamma; \Delta \vdash_{\ell} t :_{\tau} A \rrbracket && \text{(semantics of delay)} \\
&= \llbracket \Theta' \mid \zeta(\Gamma); \zeta(\Delta) \vdash_{\ell} \zeta(t) :_{\zeta(\tau)} \zeta(A) \rrbracket && \text{(IH)}
\end{aligned}$$

$$\begin{aligned}
&= \llbracket \Theta' \mid \zeta(\Gamma); \zeta(\Delta) \vdash_\ell \zeta(t) @ \zeta(\tau) : \zeta(A) @ \zeta(\tau) \rrbracket && \text{(semantics of delay)} \\
&= \llbracket \Theta' \mid \zeta(\Gamma); \zeta(\Delta) \vdash_\ell \zeta(t @ \tau) : \zeta(A @ \tau) \rrbracket && \text{(syntactic substitution)}
\end{aligned}$$

- $(\Theta \mid \Gamma; \Delta_1, \Delta_2 \vdash_\ell \text{let } a @ \tau = t_1 \text{ in } t_2 : B)$ :

$$\begin{aligned}
&\llbracket \zeta \rrbracket^+ \llbracket \Theta \mid \Gamma; \Delta_1, \Delta_2 \vdash_\ell \text{let } a @ \tau = t_1 \text{ in } t_2 : B \rrbracket \\
&= \llbracket \zeta \rrbracket^+ (\llbracket \Theta \mid \Gamma; \Delta_2, a :_\tau A \vdash_\ell t_2 : B \rrbracket \circ \varsigma^{\llbracket \Theta \rrbracket} \circ (\llbracket t_2 \rrbracket \otimes^{\llbracket \Theta \rrbracket} \text{id}) \circ \text{split}_{\Theta, \Gamma, \Delta_1, \Delta_2}) && \text{(semantics of delay)} \\
&= \llbracket \zeta \rrbracket^+ \llbracket \Theta \mid \Gamma; \Delta_2, a :_\tau A \vdash_\ell t_2 : B \rrbracket \circ \varsigma^{\llbracket \Theta' \rrbracket} \circ (\llbracket \zeta \rrbracket^+ \llbracket t_2 \rrbracket \otimes^{\llbracket \Theta' \rrbracket} \text{id}) \circ \text{split}_{\Theta', \zeta(\Gamma), \zeta(\Delta_1), \zeta(\Delta_2)} && \text{(precomposition and Lemma 11.9)} \\
&= \llbracket \Theta' \mid \zeta(\Gamma); \zeta(\Delta_2), a :_{\zeta(\tau)} \zeta(A) \vdash_\ell \zeta(t_2) : \zeta(B) \rrbracket \circ \varsigma^{\llbracket \Theta' \rrbracket} \circ (\llbracket \zeta(t_2) \rrbracket \otimes^{\llbracket \Theta' \rrbracket} \text{id}) \circ \text{split}_{\Theta', \zeta(\Gamma), \zeta(\Delta_1), \zeta(\Delta_2)} && \text{(IH)} \\
&= \llbracket \Theta' \mid \zeta(\Gamma); \zeta(\Delta_1), \zeta(\Delta_2) \vdash_\ell \text{let } a @ \zeta(\tau) = \zeta(t_1) \text{ in } \zeta(t_2) : \zeta(B) \rrbracket && \text{(semantics of delay binding)} \\
&= \llbracket \Theta' \mid \zeta(\Gamma); \zeta(\Delta_1, \Delta_2) \vdash_\ell \zeta(\text{let } a @ \tau = t_1 \text{ in } t_2) : \zeta(B) \rrbracket && \text{(syntactic substitution)}
\end{aligned}$$

- $(\Theta \mid \Gamma; \cdot \vdash_\ell \text{runG } e : A)$ :

$$\begin{aligned}
&\llbracket \zeta \rrbracket^+ \llbracket \Theta \mid \Gamma; \cdot \vdash_\ell \text{runG } t : A \rrbracket \\
&= \llbracket \zeta \rrbracket^+ (\epsilon_{\llbracket \Theta \vdash_\ell B \rrbracket} \circ F^{\llbracket \Theta \rrbracket} \llbracket \Theta \mid \Gamma \vdash_c e : \mathbf{G } A \rrbracket \circ \rho_{F^{\llbracket \Theta \rrbracket} \llbracket \Theta \vdash_c \Gamma \rrbracket}) && \text{(semantics of runG)} \\
&= \epsilon_{\llbracket \Theta' \vdash_\ell \zeta(B) \rrbracket} \circ \llbracket \zeta \rrbracket^+ F^{\llbracket \Theta \rrbracket} \llbracket \Theta \mid \Gamma \vdash_c e : \mathbf{G } A \rrbracket \circ \rho_{\llbracket \zeta \rrbracket^+ (F^{\llbracket \Theta \rrbracket} \llbracket \Theta \vdash_c \Gamma \rrbracket)} && \text{(precomposition)} \\
&= \epsilon_{\llbracket \Theta' \vdash_\ell \zeta(B) \rrbracket} \circ F^{\llbracket \Theta' \rrbracket} (\llbracket \zeta \rrbracket^* \llbracket \Theta \mid \Gamma \vdash_c e : \mathbf{G } A \rrbracket) \circ \rho_{F^{\llbracket \Theta' \rrbracket} (\llbracket \zeta \rrbracket^* \llbracket \Theta \vdash_c \Gamma \rrbracket)} && \text{(LNL property)} \\
&= \epsilon_{\llbracket \Theta' \vdash_\ell \zeta(B) \rrbracket} \circ F^{\llbracket \Theta' \rrbracket} (\llbracket \Theta' \mid \zeta(\Gamma) \vdash_c \zeta(e) : \mathbf{G } (\zeta(A)) \rrbracket) \circ \rho_{F^{\llbracket \Theta' \rrbracket} (\llbracket \Theta' \vdash_c \zeta(\Gamma) \rrbracket)} && \text{(mutual IH)} \\
&= \llbracket \Theta' \mid \zeta(\Gamma); \cdot \vdash_\ell \text{runG } \zeta(e) : \zeta(A) \rrbracket && \text{(semantics of runG)} \\
&= \llbracket \Theta' \mid \zeta(\Gamma); \cdot \vdash_\ell \zeta(\text{runG } e) : \zeta(A) \rrbracket && \text{(syntactic substitution)}
\end{aligned}$$

- $(\Theta \mid \Gamma; \cdot \vdash_\ell \mathbf{F } e : \mathbf{F } X)$ :

$$\begin{aligned}
&\llbracket \zeta \rrbracket^+ \llbracket \Theta \mid \Gamma; \cdot \vdash_\ell \mathbf{F } e : \mathbf{F } X \rrbracket \\
&= \llbracket \zeta \rrbracket^+ (F^{\llbracket \Theta \rrbracket} \llbracket \Theta \mid \Gamma \vdash_c e : X \rrbracket \circ \rho_{F^{\llbracket \Theta \rrbracket} \llbracket \Theta \vdash_c \Gamma \rrbracket}) && \text{(semantics of F)} \\
&= \llbracket \zeta \rrbracket^+ F^{\llbracket \Theta \rrbracket} \llbracket \Theta \mid \Gamma \vdash_c e : X \rrbracket \circ \rho_{\llbracket \zeta \rrbracket^+ (F^{\llbracket \Theta \rrbracket} \llbracket \Theta \vdash_c \Gamma \rrbracket)} && \text{(precomposition)} \\
&= F^{\llbracket \Theta' \rrbracket} (\llbracket \zeta \rrbracket^* \llbracket \Theta \mid \Gamma \vdash_c e : X \rrbracket) \circ \rho_{F^{\llbracket \Theta' \rrbracket} (\llbracket \zeta \rrbracket^* \llbracket \Theta \vdash_c \Gamma \rrbracket)} && \text{(LNL property)} \\
&= F^{\llbracket \Theta' \rrbracket} (\llbracket \Theta' \mid \zeta(\Gamma) \vdash_c \zeta(e) : \zeta(X) \rrbracket) \circ \rho_{F^{\llbracket \Theta' \rrbracket} (\llbracket \Theta' \vdash_c \zeta(\Gamma) \rrbracket)} && \text{(mutual IH)} \\
&= \llbracket \Theta' \mid \zeta(\Gamma); \cdot \vdash_\ell \mathbf{F } \zeta(e) : \mathbf{F } (\zeta(A)) \rrbracket && \text{(semantics of F)} \\
&= \llbracket \Theta' \mid \zeta(\Gamma); \cdot \vdash_\ell \zeta(\mathbf{F } e) : \zeta(\mathbf{F } X) \rrbracket && \text{(syntactic substitution)}
\end{aligned}$$

- $(\Theta \mid \Gamma; \Delta_1, \Delta_2 \vdash_\ell \text{let } \mathbf{F } x = t_1 \text{ in } t_2 : B)$ :

$$\begin{aligned}
&\llbracket \zeta \rrbracket^+ \llbracket \Theta \mid \Gamma; \Delta_1, \Delta_2 \vdash_\ell \text{let } a @ \tau = t_1 \text{ in } t_2 : B \rrbracket \\
&= \llbracket \zeta \rrbracket^+ (\llbracket \Theta \mid \Gamma, x : X; \Delta_2 \vdash_\ell t_2 : B \rrbracket \circ \mathbf{m}_{\llbracket \Theta \vdash_c X \rrbracket, \llbracket \Theta \vdash_c \Gamma \rrbracket \otimes^{\llbracket \Theta \rrbracket} \llbracket \Theta \vdash_\ell \Delta_2 \rrbracket} \circ \varsigma^{\llbracket \Theta \rrbracket} \circ (\llbracket t_2 \rrbracket \otimes^{\llbracket \Theta \rrbracket} \text{id}) \circ \text{split}_{\Theta, \Gamma, \Delta_1, \Delta_2}) && \text{(semantics of F binding)}
\end{aligned}$$

$$\begin{aligned}
&= \llbracket \zeta \rrbracket^+ \llbracket \Theta \mid \Gamma, x : X; \Delta_2 \vdash_\ell t_2 : B \rrbracket \circ \mathbf{m}_{\llbracket \zeta(X) \rrbracket, \llbracket \zeta(\Gamma) \rrbracket \otimes^{\llbracket \Theta' \rrbracket} \llbracket \zeta(\Delta_2) \rrbracket} \circ \zeta^{\llbracket \Theta' \rrbracket} \circ (\llbracket \zeta \rrbracket^+ \llbracket t_2 \rrbracket \otimes^{\llbracket \Theta' \rrbracket} \text{id}) \circ \text{split}_{\Theta, \zeta(\Gamma), \zeta(\Delta_1), \zeta(\Delta_2)} \\
&\quad \text{(precomposition and Lemma 11.9)} \\
&= \llbracket \Theta' \mid \zeta(\Gamma), x : \zeta(X); \zeta(\Delta_2) \vdash_\ell \zeta(t_2) : \zeta(B) \rrbracket \circ \mathbf{m} \circ \zeta^{\llbracket \Theta' \rrbracket} \circ (\llbracket \zeta(t_2) \rrbracket \otimes^{\llbracket \Theta' \rrbracket} \text{id}) \circ \text{split}_{\Theta, \zeta(\Gamma), \zeta(\Delta_1), \zeta(\Delta_2)} \\
&\quad \text{(IH)} \\
&= \llbracket \Theta' \mid \zeta(\Gamma); \zeta(\Delta_1), \zeta(\Delta_2) \vdash_\ell \text{let } \mathbf{F} \ a = \zeta(t_1) \text{ in } \zeta(t_2) : \zeta(B) \rrbracket \quad \text{(semantics of } \mathbf{F} \text{ binding)} \\
&= \llbracket \Theta' \mid \zeta(\Gamma); \zeta(\Delta_1, \Delta_2) \vdash_\ell \zeta(\text{let } \mathbf{F} \ a = t_1 \text{ in } t_2) : \zeta(B) \rrbracket \quad \text{(syntactic substitution)}
\end{aligned}$$

- $(\Theta \mid \Gamma; \Delta \vdash_\ell \Lambda i : \sigma. t : \forall i : \sigma. A) :$

$$\phi_{A,B} : \text{Rel}_{\mathcal{R}}^{\llbracket \Theta \rrbracket \times \llbracket \sigma \rrbracket}(\hat{\mathbf{wk}}(A), B) \Rightarrow \text{Rel}_{\mathcal{R}}^{\llbracket \Theta \rrbracket}(A, \hat{\mathbf{V}}_{\llbracket \sigma \rrbracket}(B))$$

$$\begin{aligned}
&\llbracket \zeta \rrbracket^+ \llbracket \Theta \mid \Gamma; \Delta \vdash_\ell \Lambda i : \sigma. t : \forall i : \sigma. A \rrbracket \\
&= \llbracket \zeta \rrbracket^+ \left( \phi_{F^{\llbracket \Theta \rrbracket} \llbracket \Theta \vdash_c \Gamma \rrbracket \otimes^{\llbracket \Theta \rrbracket} \llbracket \Theta \vdash_\ell \Delta \rrbracket, \llbracket \Theta, i : \sigma \vdash_\ell A \rrbracket} \left( \llbracket \Theta, i : \sigma \mid \Gamma; \Delta \vdash_\ell t : A \rrbracket \circ \mathbf{m}_{F^{\llbracket \Theta \rrbracket} \llbracket \Theta \vdash_c \Gamma \rrbracket, \llbracket \Theta \vdash_\ell \Delta \rrbracket}^{-1}} \right) \right) \\
&\quad \text{(semantics of universal quantification)} \\
&= \llbracket \zeta \rrbracket^+ \left( \hat{\mathbf{V}}_{\llbracket \Theta \rrbracket \times \llbracket \sigma \rrbracket}(\llbracket \Theta, i : \sigma \mid \Gamma; \Delta \vdash_\ell t : A \rrbracket \circ \mathbf{m}_{F^{\llbracket \Theta \rrbracket} \llbracket \Theta \vdash_c \Gamma \rrbracket, \llbracket \Theta \vdash_\ell \Delta \rrbracket}^{-1}}) \circ \eta_{F^{\llbracket \Theta \rrbracket} \llbracket \Theta \vdash_c \Gamma \rrbracket \otimes^{\llbracket \Theta \rrbracket} \llbracket \Theta \vdash_\ell \Delta \rrbracket} \right) \\
&\quad \text{(from hom-set equivalence to unit)} \\
&= \llbracket \zeta \rrbracket^+ (\hat{\mathbf{V}}_{\llbracket \Theta \rrbracket \times \llbracket \sigma \rrbracket}(\llbracket \Theta, i : \sigma \mid \Gamma; \Delta \vdash_\ell t : A \rrbracket \circ \mathbf{m}_{F^{\llbracket \Theta \rrbracket} \llbracket \Theta \vdash_c \Gamma \rrbracket, \llbracket \Theta \vdash_\ell \Delta \rrbracket}^{-1}})) \circ \llbracket \zeta \rrbracket^+ (\eta_{F^{\llbracket \Theta \rrbracket} \llbracket \Theta \vdash_c \Gamma \rrbracket \otimes^{\llbracket \Theta \rrbracket} \llbracket \Theta \vdash_\ell \Delta \rrbracket}) \\
&\quad \text{(functoriality)} \\
&= \hat{\mathbf{V}}_{\llbracket \Theta' \rrbracket \times \llbracket \sigma \rrbracket}((\llbracket \zeta \rrbracket \times \text{id}_{\llbracket \sigma \rrbracket})^+ \llbracket \Theta, i : \sigma \mid \Gamma; \Delta \vdash_\ell t : A \rrbracket \circ (\llbracket \zeta \rrbracket \times \text{id}_{\llbracket \sigma \rrbracket})^+ \mathbf{m}_{F^{\llbracket \Theta \rrbracket} \llbracket \Theta \vdash_c \Gamma \rrbracket, \llbracket \Theta \vdash_\ell \Delta \rrbracket}^{-1}}) \circ \eta_{F^{\llbracket \Theta' \rrbracket} \llbracket \Theta' \vdash_c \zeta(\Gamma) \rrbracket \otimes^{\llbracket \Theta' \rrbracket} \llbracket \Theta' \vdash_\ell \zeta(\Delta) \rrbracket} \\
&\quad \text{(Beck–Chevalley condition and } LNL \text{ property)} \\
&= \hat{\mathbf{V}}_{\llbracket \Theta' \rrbracket \times \llbracket \sigma \rrbracket}(\llbracket \zeta, i \mapsto i \rrbracket^+ \llbracket \Theta, i : \sigma \mid \Gamma; \Delta \vdash_\ell t : A \rrbracket \circ \mathbf{m}_{F^{\llbracket \Theta' \rrbracket} \llbracket \Theta' \vdash_c \zeta(\Gamma) \rrbracket, \llbracket \Theta' \vdash_\ell \zeta(\Delta) \rrbracket}^{-1}}) \circ \eta_{\dots} \\
&\quad \text{(Lemma 11.5 and precomposition } ((\llbracket \zeta \rrbracket \times \text{id}_{\llbracket \sigma \rrbracket})^+ \circ \mathbf{wk}_{\llbracket \sigma \rrbracket} = (\pi_1 \circ \llbracket \zeta \rrbracket \times \text{id}_{\llbracket \sigma \rrbracket})^+ = \llbracket \zeta \rrbracket)) \\
&= \hat{\mathbf{V}}_{\llbracket \Theta' \rrbracket \times \llbracket \sigma \rrbracket}(\llbracket \Theta', i : \sigma \mid (\zeta, i \mapsto i)(\Gamma); (\zeta, i \mapsto i)(\Delta) \vdash_\ell (\zeta, i \mapsto i)(t) : (\zeta, i \mapsto i)(A) \rrbracket \circ \mathbf{m}_{\dots}^{-1}) \circ \eta_{\dots} \quad \text{(IH)} \\
&= \hat{\mathbf{V}}_{\llbracket \Theta' \rrbracket \times \llbracket \sigma \rrbracket}(\llbracket \Theta', i : \sigma \mid \zeta(\Gamma); \zeta(\Delta) \vdash_\ell \zeta(t) : \zeta(A) \rrbracket \circ \mathbf{m}_{F^{\llbracket \Theta' \rrbracket} \llbracket \Theta' \vdash_c \zeta(\Gamma) \rrbracket, \llbracket \Theta' \vdash_\ell \zeta(\Delta) \rrbracket}^{-1}}) \circ \eta_{F^{\llbracket \Theta' \rrbracket} \llbracket \Theta' \vdash_c \zeta(\Gamma) \rrbracket \otimes^{\llbracket \Theta' \rrbracket} \llbracket \Theta' \vdash_\ell \zeta(\Delta) \rrbracket} \\
&\quad \text{(identity substitution)} \\
&= \phi_{F^{\llbracket \Theta' \rrbracket} \llbracket \Theta' \vdash_c \zeta(\Gamma) \rrbracket \otimes^{\llbracket \Theta' \rrbracket} \llbracket \Theta' \vdash_\ell \zeta(\Delta) \rrbracket, \llbracket \Theta', i : \sigma \vdash_\ell \zeta(A) \rrbracket} \left( \llbracket \Theta', i : \sigma \mid \zeta(\Gamma); \zeta(\Delta) \vdash_\ell \zeta(t) : \zeta(A) \rrbracket \circ \mathbf{m}_{F^{\llbracket \Theta' \rrbracket} \llbracket \Theta' \vdash_c \zeta(\Gamma) \rrbracket, \llbracket \Theta' \vdash_\ell \zeta(\Delta) \rrbracket}^{-1}} \right) \\
&\quad \text{(from unit to hom-set equivalence)} \\
&= \llbracket \Theta' \mid \zeta(\Gamma); \zeta(\Delta) \vdash_\ell \Lambda i : \sigma. \zeta(t) : \forall i : \sigma. \zeta(A) \rrbracket \quad \text{(semantics of universal quantification)} \\
&= \llbracket \Theta' \mid \zeta(\Gamma); \zeta(\Delta) \vdash_\ell \zeta(\Lambda i : \sigma. t) : \zeta(\forall i : \sigma. A) \rrbracket \quad \text{(syntactic substitution)}
\end{aligned}$$

- $(\Theta \mid \Gamma; \Delta \vdash_\ell t_s : \{s/i\}A) :$

$$\begin{aligned}
&\llbracket \zeta \rrbracket^+ \llbracket \Theta \mid \Gamma; \Delta \vdash_\ell t_s : \{s/i\}A \rrbracket \\
&= \llbracket \zeta \rrbracket^+ (\langle \text{id}_{\llbracket \sigma \rrbracket}, \llbracket \Theta \vdash_s s : \sigma \rrbracket \rangle^+ (\epsilon_{\llbracket \Theta, i : \sigma \vdash_\ell A \rrbracket}) \circ \llbracket \Theta \mid \Gamma; \Delta \vdash_\ell t : \forall i : \sigma. A \rrbracket) \\
&\quad \text{(semantics of index application)} \\
&= (\langle \text{id}_{\llbracket \sigma \rrbracket}, \llbracket \Theta \vdash_s s : \sigma \rrbracket \rangle \circ \llbracket \zeta \rrbracket^+ (\epsilon_{\llbracket \Theta, i : \sigma \vdash_\ell A \rrbracket})) \circ \llbracket \zeta \rrbracket^+ \llbracket \Theta \mid \Gamma; \Delta \vdash_\ell t : \forall i : \sigma. A \rrbracket \\
&\quad \text{(functoriality and definition of reindexing)} \\
&= (\langle \llbracket \zeta \rrbracket, \llbracket \Theta' \vdash_s \zeta(s) : \sigma \rrbracket \rangle^+ (\epsilon_{\llbracket \Theta, i : \sigma \vdash_\ell A \rrbracket})) \circ \llbracket \zeta \rrbracket^+ \llbracket \Theta \mid \Gamma; \Delta \vdash_\ell t : \forall i : \sigma. A \rrbracket \\
&\quad \text{(composition and soundness of index substitution into index judgments)}
\end{aligned}$$

$$\begin{aligned}
&= ((\llbracket \zeta \rrbracket \times \text{id}_{[\sigma]}) \circ \langle \text{id}_{[\Theta']}, \llbracket \Theta' \vdash_s \zeta(s) : \sigma \rrbracket \rangle)^+ (\epsilon_{\llbracket \Theta, i : \sigma \vdash_\ell A \rrbracket}) \circ \llbracket \zeta \rrbracket^+ \llbracket \Theta \mid \Gamma; \Delta \vdash_\ell t : \forall i : \sigma. A \rrbracket \\
&\quad \text{(CCC property)} \\
&= \langle \text{id}_{[\Theta']}, \llbracket \Theta' \vdash_s \zeta(s) : \sigma \rrbracket \rangle^+ (\llbracket \zeta \rrbracket \times \text{id}_{[\sigma]})^+ (\epsilon_{\llbracket \Theta, i : \sigma \vdash_\ell A \rrbracket}) \circ \llbracket \zeta \rrbracket^+ \llbracket \Theta \mid \Gamma; \Delta \vdash_\ell t : \forall i : \sigma. A \rrbracket \\
&\quad \text{(contravariant functor preserves composition)} \\
&= \langle \text{id}_{[\Theta']}, \llbracket \Theta' \vdash_s \zeta(s) : \sigma \rrbracket \rangle^+ \llbracket \zeta, i \mapsto i \rrbracket^+ (\epsilon_{\llbracket \Theta, i : \sigma \vdash_\ell A \rrbracket}) \circ \llbracket \zeta \rrbracket^+ \llbracket \Theta \mid \Gamma; \Delta \vdash_\ell t : \forall i : \sigma. A \rrbracket \\
&\quad \text{(Lemma 11.5)} \\
&= \langle \text{id}_{[\Theta']}, \llbracket \Theta' \vdash_s \zeta(s) : \sigma \rrbracket \rangle^+ (\epsilon_{\llbracket \Theta', i : \sigma \vdash_\ell \zeta(A) \rrbracket}) \circ \llbracket \zeta \rrbracket^+ \llbracket \Theta \mid \Gamma; \Delta \vdash_\ell t : \forall i : \sigma. A \rrbracket \\
&\quad \text{(LNL property and identity substitution (since } \zeta \# i)) \\
&= \langle \text{id}_{[\Theta']}, \llbracket \Theta' \vdash_s \zeta(s) : \sigma \rrbracket \rangle^+ (\epsilon_{\llbracket \Theta', i : \sigma \vdash_\ell \zeta(A) \rrbracket}) \circ \llbracket \Theta' \mid \zeta(\Gamma); \zeta(\Delta) \vdash_\ell \zeta(t) : \forall i : \sigma. \zeta(A) \rrbracket \\
&\quad \text{(IH and syntactic substitution for } \forall \text{ types)} \\
&= \llbracket \Theta' \mid \zeta(\Gamma); \zeta(\Delta) \vdash_\ell \zeta(t)_{\zeta(s)} : \{\zeta(s)/i\}(\zeta(A)) \rrbracket \quad \text{(semantics of index application)} \\
&= \llbracket \Theta' \mid \zeta(\Gamma); \zeta(\Delta) \vdash_\ell \zeta(t_s) : \zeta(\{s/i\}A) \rrbracket \quad \text{(syntactic substitution)}
\end{aligned}$$

- $(\Theta \mid \Gamma; \Delta \vdash_\ell \{s, t\} : \exists i : \sigma. A) :$

$$\begin{aligned}
&\llbracket \zeta \rrbracket^+ \llbracket \Theta \mid \Gamma; \Delta \vdash_\ell \{s, t\} : \exists i : \sigma. A \rrbracket \\
&= \llbracket \zeta \rrbracket^+ (\langle \text{id}_{[\Theta]}, \llbracket \Theta \vdash_s s : \sigma \rrbracket \rangle^+ (\eta_{\llbracket \Theta, i : \sigma \vdash_\ell A \rrbracket}) \circ \llbracket \Theta \mid \Gamma; \Delta \vdash_\ell t : \{s/i\}A \rrbracket) \\
&\quad \text{(semantics of existential quantification)} \\
&= (\langle \text{id}_{[\Theta]}, \llbracket \Theta \vdash_s s : \sigma \rrbracket \rangle \circ \llbracket \zeta \rrbracket)^+ (\eta_{\llbracket \Theta, i : \sigma \vdash_\ell A \rrbracket}) \circ \llbracket \zeta \rrbracket^+ \llbracket \Theta \mid \Gamma; \Delta \vdash_\ell t : \{s/i\}A \rrbracket \\
&\quad \text{(functoriality and definition of reindexing)} \\
&= (\langle \llbracket \zeta \rrbracket, \llbracket \Theta' \vdash_s \zeta(s) : \sigma \rrbracket \rangle^+ (\eta_{\llbracket \Theta, i : \sigma \vdash_\ell A \rrbracket}) \circ \llbracket \zeta \rrbracket^+ \llbracket \Theta \mid \Gamma; \Delta \vdash_\ell t : \{s/i\}A \rrbracket) \\
&\quad \text{(composition and soundness of index substitution into index judgments)} \\
&= ((\llbracket \zeta \rrbracket \times \text{id}_{[\sigma]}) \circ \langle \text{id}_{[\Theta']}, \llbracket \Theta' \vdash_s \zeta(s) : \sigma \rrbracket \rangle)^+ (\eta_{\llbracket \Theta, i : \sigma \vdash_\ell A \rrbracket}) \circ \llbracket \zeta \rrbracket^+ \llbracket \Theta \mid \Gamma; \Delta \vdash_\ell t : \{s/i\}A \rrbracket \\
&\quad \text{(CCC property)} \\
&= \langle \text{id}_{[\Theta']}, \llbracket \Theta' \vdash_s \zeta(s) : \sigma \rrbracket \rangle^+ (\llbracket \zeta \rrbracket \times \text{id}_{[\sigma]})^+ (\eta_{\llbracket \Theta, i : \sigma \vdash_\ell A \rrbracket}) \circ \llbracket \zeta \rrbracket^+ \llbracket \Theta \mid \Gamma; \Delta \vdash_\ell t : \{s/i\}A \rrbracket \\
&\quad \text{(contravariant functor preserves composition)} \\
&= \langle \text{id}_{[\Theta']}, \llbracket \Theta' \vdash_s \zeta(s) : \sigma \rrbracket \rangle^+ \llbracket \zeta, i \mapsto i \rrbracket^+ (\eta_{\llbracket \Theta, i : \sigma \vdash_\ell A \rrbracket}) \circ \llbracket \zeta \rrbracket^+ \llbracket \Theta \mid \Gamma; \Delta \vdash_\ell t : \{s/i\}A \rrbracket \\
&\quad \text{(Lemma 11.5)} \\
&= \langle \text{id}_{[\Theta']}, \llbracket \Theta' \vdash_s \zeta(s) : \sigma \rrbracket \rangle^+ (\eta_{\llbracket \Theta', i : \sigma \vdash_\ell \zeta(A) \rrbracket}) \circ \llbracket \zeta \rrbracket^+ \llbracket \Theta \mid \Gamma; \Delta \vdash_\ell t : \{s/i\}A \rrbracket \\
&\quad \text{(LNL property and identity substitution (since } \zeta \# i)) \\
&= \langle \text{id}_{[\Theta']}, \llbracket \Theta' \vdash_s \zeta(s) : \sigma \rrbracket \rangle^+ (\eta_{\llbracket \Theta', i : \sigma \vdash_\ell \zeta(A) \rrbracket}) \circ \llbracket \Theta' \mid \zeta(\Gamma); \zeta(\Delta) \vdash_\ell \zeta(t) : \{\zeta(s)/i\}(\zeta(A)) \rrbracket \\
&\quad \text{(IH and syntactic substitution for } \exists \text{ types)} \\
&= \llbracket \Theta' \mid \zeta(\Gamma); \zeta(\Delta) \vdash_\ell \{\zeta(s), \zeta(t)\} : \exists i : \sigma. \zeta(A) \rrbracket \quad \text{(semantics of existential quantification)} \\
&= \llbracket \Theta' \mid \zeta(\Gamma); \zeta(\Delta) \vdash_\ell \zeta(\{s, t\}) : \zeta(\exists i : \sigma. A) \rrbracket \quad \text{(syntactic substitution)}
\end{aligned}$$

- $(\Theta \mid \Gamma; \Delta_1, \Delta_2 \vdash_\ell \text{let } \{s, a\} = t_1 \text{ in } t_2 : B)$ :

$$\psi_{A,B} : \text{Rel}_{\mathcal{R}}^{[\Theta] \times [\sigma]}(A, \hat{\text{wk}}_{[\sigma]}(B)) \Rightarrow \text{Rel}_{\mathcal{R}}^{[\Theta]}(\hat{\Delta}_{[\sigma]}(A), B)$$

$$\begin{aligned}
& \llbracket \zeta \rrbracket^+ \llbracket \Theta \mid \Gamma; \Delta_1, \Delta_2 \vdash_\ell \text{let } \{s, a\} = t_1 \text{ in } t_2 : B \rrbracket \\
&= \llbracket \zeta \rrbracket^+ \left( \psi_{F^{[\Theta] \times [\sigma]} \llbracket \Theta, s : \sigma \vdash_c \Gamma \rrbracket \otimes^{[\Theta] \times [\sigma]} \llbracket \Theta, s : \sigma \vdash_\ell \Delta_2, a : \{s/i\} A \rrbracket, \llbracket \Theta \vdash_\ell B \rrbracket} (\llbracket \Theta, s : \sigma \mid \Gamma; \Delta_2, a : \{s/i\} A \vdash_\ell t_2 : B \rrbracket)} \right. \\
&\quad \left. \circ \hat{\Delta}_{[\Theta], [\sigma]} \left( \zeta^{[\Theta] \times [\sigma]} \circ (\text{id} \otimes^{[\Theta] \times [\sigma]} m_{F^{[\Theta]} \llbracket \Theta \vdash_c \Gamma \rrbracket, \llbracket \Theta \vdash_\ell \Delta_2 \rrbracket}}^{-1}) \right) \circ (\llbracket \Theta \mid \Gamma; \Delta_1 \vdash_\ell t_1 : \exists i : \sigma. A \rrbracket \otimes^{[\Theta]} \text{id}) \circ \text{split}_{\Theta, \Gamma, \Delta_1, \Delta_2} \right) \\
&\quad \text{(semantics of existential binding)} \\
&= \llbracket \zeta \rrbracket^+ \left( \epsilon_{\llbracket \Theta \vdash_\ell B \rrbracket} \circ \hat{\Delta}_{[\Theta], [\sigma]} (\llbracket \Theta, s : \sigma \mid \Gamma; \Delta_2, a : \{s/i\} A \vdash_\ell t_2 : B \rrbracket) \right. \\
&\quad \left. \circ \hat{\Delta}_{[\Theta], [\sigma]} \left( \zeta^{[\Theta] \times [\sigma]} \circ (\text{id} \otimes^{[\Theta] \times [\sigma]} m_{F^{[\Theta]} \llbracket \Theta \vdash_c \Gamma \rrbracket, \llbracket \Theta \vdash_\ell \Delta_2 \rrbracket}}^{-1}) \right) \circ (\llbracket \Theta \mid \Gamma; \Delta_1 \vdash_\ell t_1 : \exists i : \sigma. A \rrbracket \otimes^{[\Theta]} \text{id}) \circ \text{split}_{\Theta, \Gamma, \Delta_1, \Delta_2} \right) \\
&\quad \text{(from hom-set equivalence to counit)} \\
&= \llbracket \zeta \rrbracket^+ \epsilon_{\llbracket \Theta \vdash_\ell B \rrbracket} \circ \llbracket \zeta \rrbracket^+ \hat{\Delta}_{[\Theta], [\sigma]} \left( \llbracket \Theta, s : \sigma \mid \Gamma; \Delta_2, a : \{s/i\} A \vdash_\ell t_2 : B \rrbracket \circ \zeta^{[\Theta] \times [\sigma]} \circ (\text{id} \otimes^{[\Theta] \times [\sigma]} m_{F^{[\Theta]} \llbracket \Theta \vdash_c \Gamma \rrbracket, \llbracket \Theta \vdash_\ell \Delta_2 \rrbracket}}^{-1}) \right) \\
&\quad \circ (\llbracket \zeta \rrbracket^+ \llbracket \Theta \mid \Gamma; \Delta_1 \vdash_\ell t_1 : \exists i : \sigma. A \rrbracket \otimes^{[\Theta]} \text{id}) \circ \text{split}_{\Theta', \zeta(\Gamma), \zeta(\Delta)_1, \zeta(\Delta)_2} \\
&\quad \text{(functoriality, precomposition and Lemma 11.9)} \\
&= \epsilon_{\llbracket \Theta' \vdash_\ell \zeta(B) \rrbracket} \circ \hat{\Delta}_{[\Theta'], [\sigma]} (\llbracket \zeta \rrbracket \times \text{id})^+ \left( \llbracket \Theta, s : \sigma \mid \Gamma; \Delta_2, a : \{s/i\} A \vdash_\ell t_2 : B \rrbracket \circ \zeta^{[\Theta] \times [\sigma]} \right. \\
&\quad \left. \circ (\text{id} \otimes^{[\Theta] \times [\sigma]} m_{F^{[\Theta]} \llbracket \Theta \vdash_c \Gamma \rrbracket, \llbracket \Theta \vdash_\ell \Delta_2 \rrbracket}}^{-1}) \right) \circ (\llbracket \zeta \rrbracket^+ \llbracket \Theta \mid \Gamma; \Delta_1 \vdash_\ell t_1 : \exists i : \sigma. A \rrbracket \otimes^{[\Theta]} \text{id}) \circ \text{split}_{\Theta', \zeta(\Gamma), \zeta(\Delta)_1, \zeta(\Delta)_2} \\
&\quad \text{(LNL property and Beck–Chevalley condition)} \\
&= \epsilon_{\llbracket \Theta' \vdash_\ell \zeta(B) \rrbracket} \circ \hat{\Delta}_{[\Theta'], [\sigma]} \left( (\llbracket \zeta \rrbracket \times \text{id})^+ \llbracket \Theta, s : \sigma \mid \Gamma; \Delta_2, a : \{s/i\} A \vdash_\ell t_2 : B \rrbracket \circ \zeta^{[\Theta] \times [\sigma]} \right. \\
&\quad \left. \circ (\text{id} \otimes^{[\Theta] \times [\sigma]} m_{F^{[\Theta]} \llbracket \Theta \vdash_c \Gamma \rrbracket, \llbracket \Theta \vdash_\ell \Delta_2 \rrbracket}}^{-1}) \right) \circ (\llbracket \zeta \rrbracket^+ \llbracket \Theta \mid \Gamma; \Delta_1 \vdash_\ell t_1 : \exists i : \sigma. A \rrbracket \otimes^{[\Theta]} \text{id}) \circ \text{split}_{\Theta', \zeta(\Gamma), \zeta(\Delta)_1, \zeta(\Delta)_2} \\
&\quad \text{(functoriality and precomposition)} \\
&= \epsilon_{\llbracket \Theta' \vdash_\ell \zeta(B) \rrbracket} \circ \hat{\Delta}_{[\Theta'], [\sigma]} \left( \llbracket \zeta, i \mapsto i \rrbracket^+ \llbracket \Theta, s : \sigma \mid \Gamma; \Delta_2, a : \{s/i\} A \vdash_\ell t_2 : B \rrbracket \circ \zeta^{[\Theta] \times [\sigma]} \right. \\
&\quad \left. \circ (\text{id} \otimes^{[\Theta] \times [\sigma]} m_{F^{[\Theta]} \llbracket \Theta \vdash_c \Gamma \rrbracket, \llbracket \Theta \vdash_\ell \Delta_2 \rrbracket}}^{-1}) \right) \circ (\llbracket \zeta \rrbracket^+ \llbracket \Theta \mid \Gamma; \Delta_1 \vdash_\ell t_1 : \exists i : \sigma. A \rrbracket \otimes^{[\Theta]} \text{id}) \circ \text{split}_{\Theta', \zeta(\Gamma), \zeta(\Delta)_1, \zeta(\Delta)_2} \\
&\quad \text{(Lemma 11.5)} \\
&= \epsilon_{\llbracket \Theta' \vdash_\ell \zeta(B) \rrbracket} \circ \hat{\Delta}_{[\Theta'], [\sigma]} \left( \llbracket \Theta', s : \sigma \mid \zeta(\Gamma); \zeta(\Delta_2), a : \{s/i\}(\zeta(A)) \vdash_\ell \zeta(t_2) : \zeta(B) \rrbracket \circ \zeta^{[\Theta'] \times [\sigma]} \right. \\
&\quad \left. \circ (\text{id} \otimes^{[\Theta'] \times [\sigma]} m_{F^{[\Theta']} \llbracket \Theta' \vdash_c \zeta(\Gamma) \rrbracket, \llbracket \Theta' \vdash_\ell \zeta(\Delta_2) \rrbracket}}^{-1}) \right) \circ (\llbracket \Theta' \mid \zeta(\Gamma); \zeta(\Delta_1) \vdash_\ell \zeta(t_1) : \zeta(\exists i : \sigma. A) \rrbracket \otimes^{[\Theta']} \text{id}) \circ \text{split}_{\Theta', \zeta(\Gamma), \zeta(\Delta)_1, \zeta(\Delta)_2} \\
&\quad \text{(IH and } \zeta(\{s/i\}A) = \{s/i\}(\zeta(A)) \text{ since } s \text{ and } i \text{ are not free in } \zeta) \\
&= \left( \psi_{F^{[\Theta'] \times [\sigma]} \llbracket \Theta', s : \sigma \vdash_c \zeta(\Gamma) \rrbracket \otimes^{[\Theta'] \times [\sigma]} \llbracket \Theta', s : \sigma \vdash_\ell \zeta(\Delta_2), a : \{s/i\} \zeta(A) \rrbracket, \llbracket \Theta' \vdash_\ell \zeta(B) \rrbracket} \right. \\
&\quad \left. (\llbracket \Theta', s : \sigma \mid \zeta(\Gamma); \zeta(\Delta_2), a : \{s/i\}(\zeta(A)) \vdash_\ell \zeta(t_2) : \zeta(B) \rrbracket) \right. \\
&\quad \left. \circ \hat{\Delta}_{[\Theta'], [\sigma]} \left( \zeta^{[\Theta'] \times [\sigma]} \circ (\text{id} \otimes^{[\Theta'] \times [\sigma]} m_{F^{[\Theta']} \llbracket \Theta' \vdash_c \zeta(\Gamma) \rrbracket, \llbracket \Theta' \vdash_\ell \zeta(\Delta_2) \rrbracket}}^{-1}) \right) \right. \\
&\quad \left. \circ (\llbracket \Theta' \mid \zeta(\Gamma); \zeta(\Delta_1) \vdash_\ell \zeta(t_1) : \zeta(\exists i : \sigma. A) \rrbracket \otimes^{[\Theta']} \text{id}) \circ \text{split}_{\Theta', \zeta(\Gamma), \zeta(\Delta)_1, \zeta(\Delta)_2} \right) \\
&\quad \text{(from counit to hom-set equivalence)} \\
&= \llbracket \Theta' \mid \zeta(\Gamma); \zeta(\Delta_1, \Delta_2) \vdash_\ell \text{let } \{s, a\} = \zeta(t_1) \text{ in } \zeta(t_2) : \zeta(B) \rrbracket \quad \text{(semantics of existential binding)} \\
&= \llbracket \Theta' \mid \zeta(\Gamma); \zeta(\Delta_1, \Delta_2) \vdash_\ell \zeta(\text{let } \{s, a\} = t_1 \text{ in } t_2) : \zeta(B) \rrbracket \quad \text{(syntactic substitution)}
\end{aligned}$$

- $(\Theta \mid \Gamma; \Delta \vdash_\ell \text{select } (t_1, t_2) \text{ as } [a_1 \mapsto t'_1] \parallel [a_2 \mapsto t'_2] : \Diamond C)$ :

$$\llbracket \zeta \rrbracket^+ \llbracket \Theta \mid \Gamma; \Delta \vdash_\ell \text{select } (t_1, t_2) \text{ as } [a_1 \mapsto t'_1] \parallel [a_2 \mapsto t'_2] : \Diamond C \rrbracket$$

$$\begin{aligned}
&= \llbracket \zeta \rrbracket^+ (\mu_{\llbracket \Theta \vdash_\ell C \rrbracket}^{\llbracket \Theta \rrbracket} \circ \Diamond^{\llbracket \Theta \rrbracket} (\llbracket t'_1 \rrbracket, \llbracket t'_2 \rrbracket)^{\llbracket \Theta \rrbracket} \circ \text{dist}^{\llbracket \Theta \rrbracket}) \circ \text{st}^{F^{\llbracket \Theta \rrbracket}} \circ (\text{id} \otimes^{\llbracket \Theta \rrbracket} \text{race}_{\llbracket \Theta \vdash_\ell A \rrbracket, \llbracket \Theta \vdash_\ell B \rrbracket}^{\llbracket \Theta \rrbracket}) \\
&\quad \circ (\text{id} \otimes^{\llbracket \Theta \rrbracket} \llbracket t_1 \rrbracket \otimes^{\llbracket \Theta \rrbracket} \llbracket t_2 \rrbracket) \circ (\text{split}_{\Theta, \Gamma, \Delta_1, \Delta_2} \otimes^{\llbracket \Theta \rrbracket} \text{id}) \circ \zeta^{\llbracket \Theta \rrbracket} \circ (\text{dup} \otimes^{\llbracket \Theta \rrbracket} \text{id}) \\
&\hspace{15em} \text{(semantics of selection)} \\
&= \mu_{\llbracket \Theta' \vdash_\ell \zeta(C) \rrbracket}^{\llbracket \Theta' \rrbracket} \circ \Diamond^{\llbracket \Theta' \rrbracket} (\llbracket \zeta \rrbracket^+ \llbracket t'_1 \rrbracket, \llbracket \zeta \rrbracket^+ \llbracket t'_2 \rrbracket)^{\llbracket \Theta' \rrbracket} \circ \text{dist}^{\llbracket \Theta' \rrbracket} \circ \text{st}^{F^{\llbracket \Theta' \rrbracket}} \circ (\text{id} \otimes^{\llbracket \Theta' \rrbracket} \text{race}_{\llbracket \Theta' \vdash_\ell \zeta(A) \rrbracket, \llbracket \Theta' \vdash_\ell \zeta(B) \rrbracket}^{\llbracket \Theta' \rrbracket}) \\
&\quad \circ (\text{id} \otimes^{\llbracket \Theta' \rrbracket} \llbracket \zeta \rrbracket^+ \llbracket t_1 \rrbracket \otimes^{\llbracket \Theta' \rrbracket} \llbracket \zeta \rrbracket^+ \llbracket t_2 \rrbracket) \circ (\text{split}_{\Theta', \zeta(\Gamma), \zeta(\Delta)_1, \zeta(\Delta)_2} \otimes^{\llbracket \Theta' \rrbracket} \text{id}) \circ \zeta^{\llbracket \Theta' \rrbracket} \circ (\text{dup} \otimes^{\llbracket \Theta' \rrbracket} \text{id}) \\
&\hspace{15em} \text{(precomposition, soundness of index substitution into types and Lemma 11.9)} \\
&= \mu_{\llbracket \Theta' \vdash_\ell \zeta(C) \rrbracket}^{\llbracket \Theta' \rrbracket} \circ \Diamond^{\llbracket \Theta' \rrbracket} (\llbracket \zeta(t'_1) \rrbracket, \llbracket \zeta(t'_2) \rrbracket)^{\llbracket \Theta' \rrbracket} \circ \text{dist}^{\llbracket \Theta' \rrbracket} \circ \text{st}^{F^{\llbracket \Theta' \rrbracket}} \circ (\text{id} \otimes^{\llbracket \Theta' \rrbracket} \text{race}_{\llbracket \Theta' \vdash_\ell \zeta(A) \rrbracket, \llbracket \Theta' \vdash_\ell \zeta(B) \rrbracket}^{\llbracket \Theta' \rrbracket}) \\
&\quad \circ (\text{id} \otimes^{\llbracket \Theta' \rrbracket} \llbracket \zeta(t_1) \rrbracket \otimes^{\llbracket \Theta' \rrbracket} \llbracket \zeta(t_2) \rrbracket) \circ (\text{split}_{\Theta', \zeta(\Gamma), \zeta(\Delta)_1, \zeta(\Delta)_2} \otimes^{\llbracket \Theta' \rrbracket} \text{id}) \circ \zeta^{\llbracket \Theta' \rrbracket} \circ (\text{dup} \otimes^{\llbracket \Theta' \rrbracket} \text{id}) \\
&\hspace{15em} \text{(IH)} \\
&= \llbracket \Theta' \mid \zeta(\Gamma); \zeta(\Delta) \vdash_\ell \text{select } (\zeta(t_1), \zeta(t_2)) \text{ as } [a_1 \mapsto \zeta(t'_1)] \parallel [a_2 \mapsto \zeta(t'_2)]: \Diamond(\zeta(C)) \rrbracket \\
&\hspace{15em} \text{(semantics of selection)} \\
&= \llbracket \Theta' \mid \zeta(\Gamma); \zeta(\Delta) \vdash_\ell \zeta(\text{select } (t_1, t_2) \text{ as } [a_1 \mapsto t'_1] \parallel [a_2 \mapsto t'_2]): \zeta(\Diamond C) \rrbracket \\
&\hspace{15em} \text{(syntactic substitution)}
\end{aligned}$$

□

## 11.2 Cartesian substitution

### 11.2.1 Interpretation of Cartesian weakening

**Definition 11.11.** We interpret the Cartesian membership relation  $x : X \in_\Theta \Gamma$  as a morphism  $\llbracket x : X \in_\Theta \Gamma \rrbracket : \llbracket \Theta \vdash_c X \rrbracket \rightarrow \llbracket \Theta \vdash_c X \rrbracket$  in  $\mathbf{Set}^{\llbracket \Theta \rrbracket}$  corresponding to the relevant projection morphism:

$$\begin{aligned}
\llbracket x : X \in_\Theta \Gamma, x : X \rrbracket &\triangleq \pi_2^{\llbracket \Theta \rrbracket} \\
\llbracket x : X \in_\Theta \Gamma, x' : X' \rrbracket &\triangleq \llbracket x : X \in_\Theta \Gamma \rrbracket \circ \pi_1^{\llbracket \Theta \rrbracket}
\end{aligned}$$

**Definition 11.12.** We interpret the Cartesian subcontext relation  $\Gamma' \supseteq_\Theta \Gamma$  as a morphism  $\llbracket \Gamma' \supseteq_\Theta \Gamma \rrbracket : \llbracket \Theta \vdash_c \Gamma' \rrbracket \rightarrow \llbracket \Theta \vdash_c \Gamma \rrbracket$  in the category  $\mathbf{Set}^{\llbracket \Theta \rrbracket}$ :

$$\begin{aligned}
\llbracket \cdot \supseteq_\Theta \cdot \rrbracket &\triangleq \text{id}_{\mathbf{1}^{\llbracket \Theta \rrbracket}} \\
\llbracket \Gamma', x : X \supseteq_\Theta \Gamma \rrbracket &\triangleq \llbracket \Gamma' \supseteq_\Theta \Gamma \rrbracket \circ \pi_1^{\llbracket \Theta \rrbracket} \\
\llbracket \Gamma', x : X \supseteq_\Theta \Gamma, x : X \rrbracket &\triangleq \llbracket \Gamma' \supseteq_\Theta \Gamma \rrbracket \times^{\llbracket \Theta \rrbracket} \text{id}_{\llbracket \Theta \vdash_c X \rrbracket}
\end{aligned}$$

**Lemma 11.13** (Soundness of Cartesian context membership weakening). If  $x : X \in_\Theta \Gamma$  and  $\Gamma' \supseteq_\Theta \Gamma$ , then  $\llbracket x : X \in_\Theta \Gamma' \rrbracket = \llbracket x : X \in_\Theta \Gamma \rrbracket \circ \llbracket \Gamma' \supseteq_\Theta \Gamma \rrbracket : \llbracket \Theta \vdash_c \Gamma' \rrbracket \rightarrow \llbracket \Theta \vdash_c X \rrbracket$ .

*Proof.* By induction on the membership relation  $x : X \in_\Theta \Gamma$ .

- $x : X \in_\Theta \Gamma, x : X$ :

In one case we have  $\Gamma', x : X \supseteq_\Theta \Gamma, x : X$ :

$$\begin{aligned}
\llbracket x : X \in_\Theta \Gamma', x : X \rrbracket &= \pi_2^{\llbracket \Theta \rrbracket} \\
&= \pi_2^{\llbracket \Theta \rrbracket} \circ \langle \llbracket \Gamma' \supseteq_\Theta \Gamma \rrbracket \circ \pi_1^{\llbracket \Theta \rrbracket}, \pi_2^{\llbracket \Theta \rrbracket} \rangle \\
&= \pi_2^{\llbracket \Theta \rrbracket} \circ (\llbracket \Gamma' \supseteq_\Theta \Gamma \rrbracket \times^{\llbracket \Theta \rrbracket} \text{id}^{\llbracket \Theta \rrbracket})
\end{aligned}$$

$$= \llbracket x : X \in_{\Theta} \Gamma, x : X \rrbracket \circ \llbracket \Gamma', x : X \supseteq_{\Theta} \Gamma, x : X \rrbracket$$

Otherwise, if  $\Gamma', x' : X' \supseteq_{\Theta} \Gamma, x : X$  we have:

$$\begin{aligned} \llbracket x : X \in_{\Theta} \Gamma, x' : X' \rrbracket &= \llbracket x : X \in_{\Theta} \Gamma' \rrbracket \circ \pi_1^{[\Theta]} \\ &= \llbracket x : X \in_{\Theta} \Gamma, x : X \rrbracket \circ \llbracket \Gamma' \supseteq_{\Theta} \Gamma, x : X \rrbracket \circ \pi_1^{[\Theta]} \\ &= \llbracket x : X \in_{\Theta} \Gamma, x : X \rrbracket \circ \llbracket \Gamma', x' : X' \supseteq_{\Theta} \Gamma, x : X \rrbracket \end{aligned}$$

- $x : X \in_{\Theta} \Gamma, x' : X'$ :

We consider the case  $\Gamma', x' : X' \supseteq_{\Theta} \Gamma, x' : X'$ :

$$\begin{aligned} \llbracket x : X \in_{\Theta} \Gamma', x' : X' \rrbracket &= \llbracket x : X \in_{\Theta} \Gamma' \rrbracket \circ \pi_1^{[\Theta]} \\ &= \llbracket x : X \in_{\Theta} \Gamma \rrbracket \circ \llbracket \Gamma' \supseteq_{\Theta} \Gamma \rrbracket \circ \pi_1^{[\Theta]} \\ &= \llbracket x : X \in_{\Theta} \Gamma \rrbracket \circ \pi_1^{[\Theta]} \circ (\llbracket \Gamma' \supseteq_{\Theta} \Gamma \rrbracket \times^{[\Theta]} \text{id}^{[\Theta]}) \\ &= \llbracket x : X \in_{\Theta} \Gamma, x' : X' \rrbracket \circ \llbracket \Gamma', x' : X' \supseteq_{\Theta} \Gamma, x' : X' \rrbracket \end{aligned}$$

□

**Lemma 11.14** (Soundness of Cartesian term weakening). If  $\Theta \mid \Gamma \vdash_c e : X$  and  $\Gamma' \supseteq_{\Theta} \Gamma$ , then

$$\llbracket \Theta \mid \Gamma \vdash_c e : X \rrbracket \circ \llbracket \Gamma' \supseteq_{\Theta} \Gamma \rrbracket = \llbracket \Theta \mid \Gamma' \vdash_c e : X \rrbracket$$

*Proof.* Below we show the cases which are not a direct consequence of the induction hypothesis.

- $\Theta \mid \Gamma \vdash_c x : X$ :

$$\begin{aligned} \llbracket \Theta \mid \Gamma \vdash_c x : X \rrbracket \circ \llbracket \Gamma' \supseteq_{\Theta} \Gamma \rrbracket &= \llbracket x : X \in_{\Theta} \Gamma \rrbracket \circ \llbracket \Gamma' \supseteq_{\Theta} \Gamma \rrbracket \\ &\quad \text{(interp. of variables is the appropriate projection)} \\ &= \llbracket x : X \in_{\Theta} \Gamma' \rrbracket \\ &\quad \text{(soundness of Cartesian context membership weakening)} \\ &= \llbracket \Theta \mid \Gamma' \vdash_c x : X \rrbracket \end{aligned}$$

- $\Theta \mid \Gamma \vdash_c \lambda x. e : X \rightarrow Y$ :

$$\begin{aligned} \llbracket \Theta \mid \Gamma \vdash_c \lambda x. e : X \rightarrow Y \rrbracket \circ \llbracket \Gamma' \supseteq_{\Theta} \Gamma \rrbracket &= \text{curry}(\llbracket \Theta \mid \Gamma, x : X \vdash_c e : Y \rrbracket) \circ \llbracket \Gamma' \supseteq_{\Theta} \Gamma \rrbracket \\ &= \text{curry}(\llbracket \Theta \mid \Gamma', x : X \vdash_c e : Y \rrbracket \circ (\llbracket \Gamma' \supseteq_{\Theta} \Gamma \rrbracket \times \text{id}_{\llbracket \Theta \vdash_c X \rrbracket})) \\ &= \text{curry}(\llbracket \Theta \mid \Gamma', x : X \vdash_c e : Y \rrbracket \circ (\llbracket \Gamma', x : X \supseteq_{\Theta} \Gamma, x : X \rrbracket)) \\ &= \text{curry}(\llbracket \Theta \mid \Gamma', x : X \vdash_c e : Y \rrbracket) \\ &= \llbracket \Theta \mid \Gamma' \vdash_c \lambda x. e : X \rightarrow Y \rrbracket \end{aligned}$$

□



### 11.2.2 Interpretation of Cartesian substitution

**Definition 11.15.** We interpret a Cartesian substitution  $\Theta \mid \Gamma' \vdash_c \xi \triangleright \Gamma$  as a morphism  $\llbracket \xi \rrbracket : \llbracket \Theta \vdash_c \Gamma' \rrbracket \rightarrow^{\text{[eq]}} \llbracket \Theta \vdash_c \Gamma \rrbracket$  in the category  $\mathbf{Set}^{\text{[eq]}}$ :

$$\begin{aligned} \llbracket \Theta \mid \Gamma' \vdash_c \diamond \triangleright \cdot \rrbracket &\triangleq !_{\llbracket \Theta \vdash_c \Gamma' \rrbracket} : \llbracket \Theta \vdash_c \Gamma' \rrbracket \rightarrow' \mathbb{1}' \\ \llbracket \Theta \mid \Gamma' \vdash_c \xi, x \mapsto e \triangleright \Gamma, x : X \rrbracket &\triangleq \langle \llbracket \Theta \mid \Gamma' \vdash_c \xi \triangleright \Gamma \rrbracket, \llbracket \Theta \mid \Gamma' \vdash_c e : X \rrbracket \rangle \\ &: \llbracket \Theta \vdash_c \Gamma' \rrbracket \rightarrow' \llbracket \Theta \vdash_c \Gamma \rrbracket \otimes' \llbracket \Theta \vdash_c X \rrbracket \end{aligned}$$

As before, we lift all the standard constructions (such as  $\mathbb{1}$ ) into the  $\llbracket \Theta \rrbracket$ -indexed setting, writing  $\mathbb{1}^{\text{[eq]}}$  when needed. However, since in term-level substitutions the index context never changes, in the rest of this section we will not explicitly mark the lifting. Unlike in the case of index substitution, Cartesian substitutions live in the category  $\mathbf{Set}^{\text{[eq]}}$  for an index context  $\Theta$  and are therefore on the same level as the morphisms interpreting the terms. Thus the action of substitution will correspond to composition, rather than a pullback.

**Lemma 11.16** (Soundness of Cartesian substitution weakening). If  $\Theta \mid \Gamma' \vdash_c \xi \triangleright \Gamma$  and  $\Gamma'' \supseteq_{\Theta} \Gamma'$ , then

$$\llbracket \Theta \mid \Gamma' \vdash_c \xi \triangleright \Gamma \rrbracket \circ \llbracket \Gamma'' \supseteq_{\Theta} \Gamma' \rrbracket = \llbracket \Theta \mid \Gamma'' \vdash_c \xi \triangleright \Gamma \rrbracket : \llbracket \Theta \vdash_c \Gamma'' \rrbracket \rightarrow \llbracket \Theta \vdash_c \Gamma \rrbracket$$

*Proof.* By induction on the substitution  $\Theta \mid \Gamma' \vdash_c \xi \triangleright \Gamma$ .

- $\Theta \mid \Gamma' \vdash_c \diamond \triangleright \cdot$ :

$$\begin{aligned} \llbracket \Theta \mid \Gamma' \vdash_c \diamond \triangleright \cdot \rrbracket \circ \llbracket \Gamma'' \supseteq_{\Theta} \Gamma' \rrbracket &= !_{\Theta \vdash_c \Gamma'} \circ \llbracket \Gamma'' \supseteq_{\Theta} \Gamma' \rrbracket \\ &= !_{\Theta \vdash_c \Gamma''} \quad (\text{terminal map is unique}) \\ &= \llbracket \Theta \mid \Gamma'' \vdash_c \diamond \triangleright \cdot \rrbracket \end{aligned}$$

- $\Theta \mid \Gamma' \vdash_c \xi, x \mapsto e \triangleright \Gamma, x : X$ :

$$\begin{aligned} &\llbracket \Theta \mid \Gamma' \vdash_c \xi \triangleright \Gamma, x : X \rrbracket \circ \llbracket \Gamma'' \supseteq_{\Theta} \Gamma' \rrbracket \\ &= \langle \llbracket \Theta \mid \Gamma' \vdash_c \xi \triangleright \Gamma \rrbracket, \llbracket \Theta \mid \Gamma' \vdash_c e : X \rrbracket \rangle \circ \llbracket \Gamma'' \supseteq_{\Theta} \Gamma' \rrbracket \\ &= \langle \llbracket \Theta \mid \Gamma' \vdash_c \xi \triangleright \Gamma \rrbracket \circ \llbracket \Gamma'' \supseteq_{\Theta} \Gamma' \rrbracket, \llbracket \Theta \mid \Gamma' \vdash_c e : X \rrbracket \circ \llbracket \Gamma'' \supseteq_{\Theta} \Gamma' \rrbracket \rangle \\ &= \langle \llbracket \Theta \mid \Gamma' \vdash_c \xi \triangleright \Gamma \rrbracket \circ \llbracket \Gamma'' \supseteq_{\Theta} \Gamma' \rrbracket, \llbracket \Theta \mid \Gamma'' \vdash_c e : X \rrbracket \rangle \\ &\quad (\text{soundness of Cartesian term weakening}) \\ &= \langle \llbracket \Theta \mid \Gamma'' \vdash_c \xi \triangleright \Gamma \rrbracket, \llbracket \Theta \mid \Gamma'' \vdash_c e : X \rrbracket \rangle \quad (\text{IH}) \\ &= \llbracket \Theta \mid \Gamma'' \vdash_c \xi, x \mapsto e \triangleright \Gamma, x : X \rrbracket \end{aligned}$$

□

**Lemma 11.17** (Semantics of Cartesian context extension). For a substitution  $\Theta \mid \Gamma' \vdash_c \xi \triangleright \Gamma$  and Cartesian variable  $x : X$  with  $\xi \# x$ , we have:

$$\begin{aligned} \llbracket \Theta \mid \Gamma', x : X \vdash_c \xi, x \mapsto x \triangleright \Gamma, x : X \rrbracket &= \llbracket \xi \rrbracket \times \text{id}_{\llbracket \Theta \vdash_c X \rrbracket} \\ &: \llbracket \Theta \vdash_c \Gamma' \rrbracket \otimes \llbracket \Theta \vdash_c X \rrbracket \rightarrow \llbracket \Theta \vdash_c \Gamma \rrbracket \otimes \llbracket \Theta \vdash_c X \rrbracket \end{aligned}$$

*Proof.*

$$\begin{aligned}
& \llbracket \Theta \mid \Gamma', x : X \vdash_c \xi, x \mapsto x \triangleright \Gamma, x : X \rrbracket \\
&= \langle \llbracket \Theta \mid \Gamma', x : X \vdash_c \xi \triangleright \Gamma \rrbracket, \llbracket \Theta \mid \Gamma', x : X \vdash_c x : X \rrbracket \rangle \\
&= \langle \llbracket \Theta \mid \Gamma', x : X \vdash_c \xi \triangleright \Gamma \rrbracket, \pi_2 \rangle \\
&= \langle \llbracket \Theta \mid \Gamma' \vdash_c \xi \triangleright \Gamma \rrbracket \circ \llbracket \Gamma', x : X \supseteq_\Theta \Gamma' \rrbracket, \pi_2 \rangle \quad (\text{soundness of weakening}) \\
&= \langle \llbracket \Theta \mid \Gamma' \vdash_c \xi \triangleright \Gamma \rrbracket \circ \pi_1, \pi_2 \rangle \\
&= \llbracket \Theta \mid \Gamma' \vdash_c \xi \triangleright \Gamma \rrbracket \times \text{id}_{\llbracket \Theta \vdash_c X \rrbracket}
\end{aligned}$$

□

**Lemma 11.18** (Soundness of index substitution into Cartesian substitution). If  $\Theta \mid \Gamma' \vdash_c \xi \triangleright \Gamma$  and  $\Theta' \vdash_s \zeta \triangleright \Theta$ , then

$$\llbracket \zeta \rrbracket^* \llbracket \Theta \mid \Gamma' \vdash_c \xi \triangleright \Gamma \rrbracket = \llbracket \zeta(\Theta \mid \Gamma' \vdash_c \xi \triangleright \Gamma) \rrbracket$$

*Proof.* By induction on  $\Theta \mid \Gamma' \vdash_c \xi \triangleright \Gamma$ .

1.  $\Theta \mid \Gamma' \vdash_c \diamond \triangleright \cdot$ :

$$\begin{aligned}
\llbracket \zeta \rrbracket^* \llbracket \Theta \mid \Gamma' \vdash_c \diamond \triangleright \cdot \rrbracket &= \llbracket \zeta \rrbracket^* (!_{\llbracket \Theta \vdash_c \Gamma' \rrbracket} : \llbracket \Theta \vdash_c \Gamma' \rrbracket \rightarrow^{\llbracket \Theta \rrbracket} \mathbb{1}^{\llbracket \Theta \rrbracket}) \quad (\text{semantics of } \diamond) \\
&= !_{\llbracket \Theta' \vdash_c \Gamma \rrbracket} : \llbracket \Theta' \vdash_c \zeta(\Gamma) \rrbracket \rightarrow^{\llbracket \Theta' \rrbracket} \mathbb{1}^{\llbracket \Theta' \rrbracket} \quad (\text{precomposition}) \\
&= \llbracket \Theta' \mid \Gamma' \vdash_c \diamond \triangleright \cdot \rrbracket \quad (\text{semantics of } \diamond) \\
&= \llbracket \zeta(\Theta \mid \Gamma' \vdash_c \diamond \triangleright \cdot) \rrbracket \quad (\text{index substitution application})
\end{aligned}$$

2.  $\Theta \mid \Gamma' \vdash_c \xi, x \mapsto e \triangleright \Gamma$ :

$$\begin{aligned}
\llbracket \zeta \rrbracket^* \llbracket \Theta \mid \Gamma' \vdash_c \xi, x \mapsto e \triangleright \Gamma \rrbracket &= \llbracket \zeta \rrbracket^* \langle \llbracket \Theta \mid \Gamma' \vdash_c \xi \triangleright \Gamma \rrbracket, \llbracket \Theta \mid \Gamma' \vdash_c e : X \rrbracket \rangle^{\llbracket \Theta \rrbracket} \quad (\text{semantics of } \xi, x : e) \\
&= \langle \llbracket \zeta \rrbracket^* \llbracket \Theta \mid \Gamma' \vdash_c \xi \triangleright \Gamma \rrbracket, \llbracket \zeta \rrbracket^* \llbracket \Theta \mid \Gamma' \vdash_c e : X \rrbracket \rangle^{\llbracket \Theta' \rrbracket} \quad (\text{precomposition}) \\
&= \langle \llbracket \Theta' \mid \zeta(\Gamma') \vdash_c \zeta(\xi) \triangleright \zeta(\Gamma) \rrbracket, \llbracket \Theta' \mid \zeta(\Gamma') \vdash_c \zeta(e) : \zeta(X) \rrbracket \rangle^{\llbracket \Theta' \rrbracket} \quad (\text{IH and soundness of index subst.}) \\
&= \llbracket \Theta' \mid \zeta(\Gamma') \vdash_c \zeta(\xi), x \mapsto \zeta(e) \triangleright \zeta(\Gamma) \rrbracket \quad (\text{semantics of } \zeta(\xi), x \mapsto \zeta(e)) \\
&= \llbracket \zeta(\Theta \mid \Gamma' \vdash_c \xi, x \mapsto e \triangleright \Gamma) \rrbracket \quad (\text{index substitution application})
\end{aligned}$$

□

**Theorem 11.19** (Soundness of Cartesian substitution into Cartesian terms). If  $\Theta \mid \Gamma \vdash_c e : X$  and  $\Theta \mid \Gamma' \vdash_c \xi \triangleright \Gamma$ , then

$$\llbracket \Theta \mid \Gamma' \vdash_c [\xi]e : X \rrbracket = \llbracket \Theta \mid \Gamma \vdash_c e : X \rrbracket \circ \llbracket \xi \rrbracket$$

*Proof.* We proceed by induction on the derivation of the well-formed type judgment  $\Theta \mid \Gamma \vdash_c e : X$ .

- $(\Theta \mid \Gamma \vdash_c \bullet : 1)$ :

$$\begin{aligned}
\llbracket \Theta \mid \Gamma \vdash_c \bullet : 1 \rrbracket \circ \llbracket \xi \rrbracket &= !_{\llbracket \Theta \vdash_c \Gamma \rrbracket} \circ \llbracket \xi \rrbracket : \llbracket \Theta \vdash_c \Gamma \rrbracket \rightarrow \mathbb{1} && \text{(semantics of } \bullet : 1 \text{)} \\
&= !_{\llbracket \Theta \vdash_c \Gamma' \rrbracket} : \llbracket \Theta \vdash_c \Gamma' \rrbracket \rightarrow \mathbb{1} && \text{(unique map to terminal obj.)} \\
&= \llbracket \Theta \mid \Gamma' \vdash_c \bullet : 1 \rrbracket && \text{(semantics of } \bullet : 1 \text{)} \\
&= \llbracket \Theta \mid \Gamma' \vdash_c [\xi] \bullet : 1 \rrbracket && \text{(syntactic substitution)}
\end{aligned}$$

- $(\Theta \mid \Gamma, x : X \vdash_c x : X, \text{ and } \Theta \mid \Gamma' \vdash_c \xi, x \mapsto e \triangleright \Gamma, x : X)$ :

$$\begin{aligned}
&\llbracket \Theta \mid \Gamma, x : X \vdash_c x : X \rrbracket \circ \llbracket \xi, x \mapsto e \rrbracket \\
&= \pi_2 \circ \llbracket \xi, x \mapsto e \rrbracket : \llbracket \Theta \vdash_c \Gamma' \rrbracket \rightarrow \llbracket \Theta \vdash_c X \rrbracket && \text{(semantics of } x : X \text{)} \\
&= \pi_2 \circ \langle \llbracket \Theta \mid \Gamma' \vdash_c \xi \triangleright \Gamma \rrbracket, \llbracket \Theta \mid \Gamma' \vdash_c e : X \rrbracket \rangle && \text{(sem. of substitution)} \\
&= \llbracket \Theta \mid \Gamma' \vdash_c e : X \rrbracket && \text{(second projection)} \\
&= \llbracket \Theta \mid \Gamma' \vdash_c [\xi, x \mapsto e] x : X \rrbracket && \text{(syntactic substitution)}
\end{aligned}$$

- $(\Theta \mid \Gamma, y : Y \vdash_c x : X, \text{ and } \Theta \mid \Gamma' \vdash_c \xi, y \mapsto e \triangleright \Gamma, y : Y)$ :

$$\begin{aligned}
&\llbracket \Theta \mid \Gamma, y : Y \vdash_c x : X \rrbracket \circ \llbracket \xi, y \mapsto e \rrbracket \\
&= \llbracket \Theta \mid \Gamma \vdash_c x : X \rrbracket \circ \pi_1 \circ \llbracket \xi, y \mapsto e \rrbracket : \llbracket \Theta \vdash_c \Gamma' \rrbracket \rightarrow \llbracket \Theta \vdash_c X \rrbracket && \text{(semantics of } x : X \text{)} \\
&= \llbracket \Theta \mid \Gamma \vdash_c x : X \rrbracket \circ \pi_1 \circ \langle \llbracket \Theta \mid \Gamma' \vdash_c \xi \triangleright \Gamma \rrbracket, \llbracket \Theta \mid \Gamma' \vdash_c e : Y \rrbracket \rangle && \text{(sem. of substitution)} \\
&= \llbracket \Theta \mid \Gamma \vdash_c x : X \rrbracket \circ \langle \llbracket \Theta \mid \Gamma' \vdash_c \xi \triangleright \Gamma \rrbracket \rangle && \text{(first projection)} \\
&= \llbracket \Theta \mid \Gamma' \vdash_c [\xi] x : X \rrbracket && \text{(IH)} \\
&= \llbracket \Theta \mid \Gamma' \vdash_c [\xi, y \mapsto e] x : X \rrbracket && \text{(syntactic substitution)}
\end{aligned}$$

- $(\Theta \mid \Gamma \vdash_c \lambda x. e : X \rightarrow Y)$ :

$$\begin{aligned}
&\llbracket \Theta \mid \Gamma \vdash_c \lambda x. e : X \rightarrow Y \rrbracket \circ \llbracket \xi \rrbracket \\
&= \text{curry}(\llbracket \Theta \mid \Gamma, x : X \vdash_c e : Y \rrbracket) \circ \llbracket \xi \rrbracket && \text{(semantics of } \lambda x. e : X \rightarrow Y \text{)} \\
&= \text{curry}(\llbracket \Theta \mid \Gamma, x : X \vdash_c e : Y \rrbracket \circ (\llbracket \xi \rrbracket \otimes \text{id}_{\llbracket \Theta \vdash_c X \rrbracket})) && \text{(CCC prop.)} \\
&= \text{curry}(\llbracket \Theta \mid \Gamma, x : X \vdash_c e : Y \rrbracket \circ \llbracket \xi, x \mapsto x \rrbracket) && \text{(Lemma 11.17)} \\
&= \text{curry}(\llbracket \Theta \mid \Gamma', x : X \vdash_c [\xi] e : Y \rrbracket) && \text{(IH)} \\
&= \llbracket \Theta \mid \Gamma \vdash_c \lambda x. [\xi] t : X \rightarrow Y \rrbracket && \text{(semantics of } \lambda x. [\xi] e : X \rightarrow Y \text{)} \\
&= \llbracket \Theta \mid \Gamma \vdash_c [\xi](\lambda x. e) : X \rightarrow Y \rrbracket && \text{(syntactic substitution } (\xi \# x) \text{)}
\end{aligned}$$

- $(\Theta \mid \Gamma \vdash_c e_1 e_2 : Y)$ :

$$\begin{aligned}
&\llbracket \Theta \mid \Gamma \vdash_c e_1 e_2 : Y \rrbracket \circ \llbracket \xi \rrbracket \\
&= \text{eval} \circ \langle \llbracket \Theta \mid \Gamma \vdash_c e_1 : X \rightarrow Y \rrbracket, \llbracket \Theta \mid \Gamma \vdash_c e_2 : X \rrbracket \rangle \circ \llbracket \xi \rrbracket && \text{(semantics of } e_1 e_2 : Y \text{)} \\
&= \text{eval} \circ \langle \llbracket \Theta \mid \Gamma \vdash_c e_1 : X \rightarrow Y \rrbracket \circ \llbracket \xi \rrbracket, \llbracket \Theta \mid \Gamma \vdash_c e_2 : X \rrbracket \circ \llbracket \xi \rrbracket \rangle && \text{(CCC prop.)} \\
&= \text{eval} \circ \langle \llbracket \Theta \mid \Gamma' \vdash_c [\xi] e_1 : X \rightarrow Y \rrbracket, \llbracket \Theta \mid \Gamma' \vdash_c [\xi] e_2 : X \rrbracket \rangle && \text{(IH)} \\
&= \llbracket \Theta \mid \Gamma' \vdash_c ([\xi] e_1) ([\xi] e_2) : Y \rrbracket && \text{(semantics of } ([\xi] e_1) ([\xi] e_2) : Y \text{)} \\
&= \llbracket \Theta \mid \Gamma' \vdash_c [\xi](e_1 e_2) : Y \rrbracket && \text{(syntactic substitution)}
\end{aligned}$$

- $(\Theta \mid \Gamma \vdash_c \mathbf{G} \, t : \mathbf{G} \, A)$ :

$$\begin{aligned}
& \llbracket \Theta \mid \Gamma \vdash_c \mathbf{G} \, t : \mathbf{G} \, A \rrbracket \circ \llbracket \xi \rrbracket \\
&= G \left( \llbracket \Theta \mid \Gamma; \cdot \vdash_\ell t : A \rrbracket \circ \rho_{F[\llbracket \Theta \vdash_c \Gamma \rrbracket]}^{-1} \right) \circ \eta_{\llbracket \Theta \vdash_c \Gamma \rrbracket} \circ \llbracket \xi \rrbracket && \text{(semantics of } \mathbf{G} \, t : \mathbf{G} \, A) \\
&= G \left( \llbracket \Theta \mid \Gamma; \cdot \vdash_\ell t : A \rrbracket \circ \rho_{F[\llbracket \Theta \vdash_c \Gamma \rrbracket]}^{-1} \right) \circ GF[\llbracket \xi \rrbracket] \circ \eta_{\llbracket \Theta \vdash_c \Gamma \rrbracket} && \text{(naturality)} \\
&= G \left( \llbracket \Theta \mid \Gamma; \cdot \vdash_\ell t : A \rrbracket \circ \rho_{F[\llbracket \Theta \vdash_c \Gamma \rrbracket]}^{-1} \circ F[\llbracket \xi \rrbracket] \right) \circ \eta_{\llbracket \Theta \vdash_c \Gamma \rrbracket} && \text{(functoriality)} \\
&= G \left( \llbracket \Theta \mid \Gamma; \cdot \vdash_\ell t : A \rrbracket \circ F[\llbracket \xi \rrbracket] \otimes \text{id}_{\llbracket \Theta \vdash_\ell \Delta \rrbracket} \circ \rho_{F[\llbracket \Theta \vdash_c \Gamma \rrbracket]}^{-1} \right) \circ \eta_{\llbracket \Theta \vdash_c \Gamma \rrbracket} && \text{(naturality)} \\
&= G \left( \llbracket \Theta \mid \Gamma'; \cdot \vdash_\ell [\xi]t : A \rrbracket \circ \rho_{F[\llbracket \Theta \vdash_c \Gamma' \rrbracket]}^{-1} \right) \circ \eta_{\llbracket \Theta \vdash_c \Gamma' \rrbracket} && \text{(mutual IH)} \\
&= \llbracket \Theta \mid \Gamma' \vdash_c \mathbf{G} \, ([\xi]t) : \mathbf{G} \, A \rrbracket && \text{(semantics of } \mathbf{G} \, ([\xi]t) : \mathbf{G} \, A) \\
&= \llbracket \Theta \mid \Gamma' \vdash_c [\xi](\mathbf{G} \, t) : \mathbf{G} \, A \rrbracket && \text{(syntactic substitution)}
\end{aligned}$$

□

**Lemma 11.20.** For contexts  $\Theta, \Gamma, \Delta$  a Cartesian substitution  $\Theta \mid \Gamma' \vdash_c \xi \triangleright \Gamma$ , we have:

$$\begin{aligned}
& \text{drop}_{\Theta, \Gamma, \Delta} \circ (F[\llbracket \xi \rrbracket] \otimes \text{id}_{\llbracket \Theta \vdash_\ell \Delta \rrbracket}) = \text{drop}_{\Theta, \Gamma', \Delta} \\
& \text{split}_{\Theta, \Gamma, \Delta_1, \Delta_2} \circ (F[\llbracket \xi \rrbracket] \otimes \text{id}_{\llbracket \Theta \vdash_\ell \Delta_1, \Delta_2 \rrbracket}) = ((F[\llbracket \xi \rrbracket] \otimes \text{id}_{\llbracket \Theta \vdash_\ell \Delta_1 \rrbracket}) \otimes (F[\llbracket \xi \rrbracket] \otimes \text{id}_{\llbracket \Theta \vdash_\ell \Delta_2 \rrbracket})) \circ \text{split}_{\Theta, \Gamma', \Delta_1, \Delta_2}
\end{aligned}$$

*Proof.* Follow from the naturality of  $\mathbf{m}$  and  $\mathbf{u}$  that are used to define  $\text{drop}$  and  $\text{split}$ . The general “rearranging” operator  $\varsigma$  is a composition of associators and commutators, which are all natural. Thus, composition with  $\varsigma$  can be exchanged in the appropriate way, and the soundness of the tranformation will be a consequence of naturality. □

**Theorem 11.21** (Soundness of Cartesian substitution into linear terms). If  $\Theta \mid \Delta; \Gamma \vdash_\ell t : A$  and  $\Theta \mid \Gamma' \vdash_c \xi \triangleright \Gamma$ , then

$$\llbracket \Theta \mid \Gamma'; \Delta \vdash_\ell [\xi]t : A \rrbracket = \llbracket \Theta \mid \Gamma; \Delta \vdash_\ell t : A \rrbracket \circ (F[\llbracket \xi \rrbracket] \otimes \text{id}_{\llbracket \Theta \vdash_\ell \Delta \rrbracket})$$

*Proof.* We proceed by induction on the derivation of the well-formed type judgment  $\Theta \mid \Gamma; \Delta \vdash_\ell t : A$ .

- $(\Theta \mid \Gamma; a : A \vdash_\ell a : A)$ :

$$\begin{aligned}
& \llbracket \Theta \mid \Gamma; a : A \vdash_\ell a : A \rrbracket \circ (F[\llbracket \xi \rrbracket] \otimes \text{id}_{\llbracket \Theta \vdash_\ell A \rrbracket}) \\
&= \text{drop}_{\Theta, \Gamma, a : A} \circ (F[\llbracket \xi \rrbracket] \otimes \text{id}_{\llbracket \Theta \vdash_\ell A \rrbracket}) && \text{(semantics of } a : A) \\
&= \text{drop}_{\Theta, \Gamma', a : A} && \text{(Lemma 11.20)} \\
&= \llbracket \Theta \mid \Gamma'; a : A \vdash_\ell a : A \rrbracket && \text{(semantics of } a : A)
\end{aligned}$$

- $(\Theta \mid \Gamma; \Delta \vdash_\ell \lambda a. t : A \multimap B)$ :

$$\begin{aligned}
& \llbracket \Theta \mid \Gamma; \Delta \vdash_\ell \lambda a. t : A \multimap B \rrbracket \circ (F[\llbracket \xi \rrbracket] \otimes \text{id}_{\llbracket \Theta \vdash_\ell \Delta \rrbracket}) \\
&= \text{curry}(\llbracket \Theta \mid \Gamma; \Delta, a : A \vdash_\ell t : B \rrbracket \circ \varsigma) \circ (F[\llbracket \xi \rrbracket] \otimes \text{id}_{\llbracket \Theta \vdash_\ell \Delta \rrbracket}) && \text{(semantics of } \lambda a. t : A \multimap B) \\
&= \text{curry}(\llbracket \Theta \mid \Gamma; \Delta, a : A \vdash_\ell t : B \rrbracket \circ \varsigma \circ (F[\llbracket \xi \rrbracket] \otimes \text{id}_{\llbracket \Theta \vdash_\ell \Delta \rrbracket} \otimes \text{id}_{\llbracket \Theta \vdash_\ell A \rrbracket})) && \text{(SMCC law)} \\
&= \text{curry}(\llbracket \Theta \mid \Gamma; \Delta, a : A \vdash_\ell t : B \rrbracket \circ (F[\llbracket \xi \rrbracket] \otimes \text{id}_{\llbracket \Theta \vdash_\ell \Delta, a : A \rrbracket}) \circ \varsigma) && \text{(sem. of contexts and naturality)}
\end{aligned}$$

$$\begin{aligned}
&= \text{curry}(\llbracket \Theta \mid \Gamma'; \Delta, a : A \vdash_\ell [\xi]t : B \rrbracket \circ \varsigma) && \text{(IH)} \\
&= \llbracket \Theta \mid \Gamma'; \Delta \vdash_\ell \lambda a. [\xi]t : A \multimap B \rrbracket && \text{(semantics of } \lambda a. [\xi]t : A \multimap B \text{)} \\
&= \llbracket \Theta \mid \Gamma'; \Delta \vdash_\ell [\xi](\lambda a. t) : A \multimap B \rrbracket && \text{(syntactic substitution)}
\end{aligned}$$

•  $(\Theta \mid \Gamma; \Delta_1, \Delta_2 \vdash_\ell t_1 t_2 : B)$ :

$$\begin{aligned}
&\llbracket \Theta \mid \Gamma; \Delta_1, \Delta_2 \vdash_\ell t_1 t_2 : B \rrbracket \circ (F\llbracket \xi \rrbracket \otimes \text{id}_{\llbracket \Theta \vdash_\ell \Delta_1, \Delta_2 \rrbracket}) \\
&= \text{eval} \circ (\llbracket \Theta \mid \Gamma; \Delta_1 \vdash_\ell t_1 : A \multimap B \rrbracket \otimes \llbracket \Theta \mid \Gamma; \Delta_2 \vdash_\ell t_2 : A \rrbracket) \circ \text{split}_{\Theta, \Gamma, \Delta_1, \Delta_2} \circ (F\llbracket \xi \rrbracket \otimes \text{id}_{\llbracket \Theta \vdash_\ell \Delta_1, \Delta_2 \rrbracket}) \\
&\quad \text{(semantics of } t_1 t_2 : B \text{)} \\
&= \text{eval} \circ (\llbracket t_1 \rrbracket \otimes \llbracket t_2 \rrbracket) \circ ((F\llbracket \xi \rrbracket \otimes \text{id}_{\llbracket \Theta \vdash_\ell \Delta_1 \rrbracket}) \otimes (F\llbracket \xi \rrbracket \otimes \text{id}_{\llbracket \Theta \vdash_\ell \Delta_2 \rrbracket})) \circ \text{split}_{\Theta, \Gamma', \Delta_1, \Delta_2} \quad \text{(Lemma 11.20)} \\
&= \text{eval} \circ ((\llbracket t_1 \rrbracket \circ (F\llbracket \xi \rrbracket \otimes \text{id}_{\llbracket \Theta \vdash_\ell \Delta_1 \rrbracket})) \otimes (\llbracket t_2 \rrbracket \circ (F\llbracket \xi \rrbracket \otimes \text{id}_{\llbracket \Theta \vdash_\ell \Delta_2 \rrbracket}))) \circ \text{split}_{\Theta, \Gamma', \Delta_1, \Delta_2} \quad \text{(SMCC prop.)} \\
&= \text{eval} \circ (\llbracket \Theta \mid \Gamma'; \Delta_1 \vdash_\ell [\xi]t_1 : A \multimap B \rrbracket \otimes \llbracket \Theta \mid \Gamma'; \Delta_2 \vdash_\ell [\xi]t_2 : A \rrbracket) \circ \text{split}_{\Theta, \Gamma', \Delta_1, \Delta_2} \quad \text{(IHs)} \\
&= \llbracket \Theta \mid \Gamma'; \Delta_1, \Delta_2 \vdash_\ell ([\xi]t_1) ([\xi]t_2) : B \rrbracket && \text{(semantics of } ([\xi]t_1) ([\xi]t_2) : B \text{)} \\
&= \llbracket \Theta \mid \Gamma'; \Delta_1, \Delta_2 \vdash_\ell [\xi](t_1 t_2) : B \rrbracket && \text{(syntactic substitution)}
\end{aligned}$$

•  $(\Theta \mid \Gamma; \cdot \vdash_\ell \bullet : \mathbb{I})$ :

$$\begin{aligned}
&\llbracket \Theta \mid \Gamma; \cdot \vdash_\ell \bullet : \mathbb{I} \rrbracket \circ (F\llbracket \xi \rrbracket \otimes \text{id}_{\mathbb{I}}) = \text{drop}_{\Theta, \Gamma, \cdot} \circ (F\llbracket \xi \rrbracket \otimes \text{id}_{\llbracket \Theta \vdash_\ell \Delta \rrbracket}) && \text{(semantics of } \bullet : \mathbb{I} \text{)} \\
&= \text{drop}_{\Theta, \Gamma', \cdot} && \text{(Lemma 11.20)} \\
&= \llbracket \Theta \mid \Gamma'; \cdot \vdash_\ell \bullet : \mathbb{I} \rrbracket && \text{(semantics of } \bullet : \mathbb{I} \text{)} \\
&= \llbracket \Theta \mid \Gamma'; \cdot \vdash_\ell [\xi]\bullet : \mathbb{I} \rrbracket && \text{(syntactic substitution)}
\end{aligned}$$

•  $(\Theta \mid \Gamma; \Delta_1, \Delta_2 \vdash_\ell \text{let } \langle \rangle = t_1 \text{ in } t_2 : C)$ :

$$\begin{aligned}
&\llbracket \Theta \mid \Gamma; \Delta_1, \Delta_2 \vdash_\ell \text{let } \langle \rangle = t_1 \text{ in } t_2 : C \rrbracket \circ (F\llbracket \xi \rrbracket \otimes \text{id}_{\llbracket \Theta \vdash_\ell \Delta_1, \Delta_2 \rrbracket}) \\
&= \lambda_{\llbracket \Theta \vdash_\ell B \rrbracket} \circ (\llbracket \Theta \mid \Gamma; \Delta_1 \vdash_\ell t_1 : \mathbb{I} \rrbracket \otimes \llbracket \Theta \mid \Gamma; \Delta_2 \vdash_\ell t_2 : B \rrbracket) \circ \text{split}_{\Theta, \Gamma, \Delta_1, \Delta_2} \circ (F\llbracket \xi \rrbracket \otimes \text{id}_{\llbracket \Theta \vdash_\ell \Delta_1, \Delta_2 \rrbracket}) \\
&\quad \text{(semantics of } \text{let } \langle \rangle = t_1 \text{ in } t_2 : B \text{)} \\
&= \lambda_{\llbracket \Theta \vdash_\ell B \rrbracket} \circ (\llbracket t_1 \rrbracket \otimes \llbracket t_2 \rrbracket) \circ ((F\llbracket \xi \rrbracket \otimes \text{id}_{\llbracket \Theta \vdash_\ell \Delta_1 \rrbracket}) \otimes (F\llbracket \xi \rrbracket \otimes \text{id}_{\llbracket \Theta \vdash_\ell \Delta_2 \rrbracket})) \circ \text{split}_{\Theta, \Gamma', \Delta_1, \Delta_2} \\
&\quad \text{(Lemma 11.20)} \\
&= \lambda_{\llbracket \Theta \vdash_\ell B \rrbracket} \circ ((\llbracket t_1 \rrbracket \circ (F\llbracket \xi \rrbracket \otimes \text{id}_{\llbracket \Theta \vdash_\ell \Delta_1 \rrbracket})) \otimes (\llbracket t_2 \rrbracket \circ (F\llbracket \xi \rrbracket \otimes \text{id}_{\llbracket \Theta \vdash_\ell \Delta_2 \rrbracket}))) \circ \text{split}_{\Theta, \Gamma', \Delta_1, \Delta_2} \\
&\quad \text{(SMCC property)} \\
&= \lambda_{\llbracket \Theta \vdash_\ell B \rrbracket} \circ (\llbracket \Theta \mid \Gamma'; \Delta_1 \vdash_\ell [\xi]t_1 : \mathbb{I} \rrbracket \otimes \llbracket \Theta \mid \Gamma'; \Delta_2 \vdash_\ell [\xi]t_2 : B \rrbracket) \circ \text{split}_{\Theta, \Gamma', \Delta_1, \Delta_2} \quad \text{(IHs)} \\
&= \llbracket \Theta \mid \Gamma'; \Delta_1, \Delta_2 \vdash_\ell \text{let } \langle \rangle = [\xi]t_1 \text{ in } [\xi]t_2 : B \rrbracket && \text{(semantics of } \text{let } \langle \rangle = [\xi]t_1 \text{ in } [\xi]t_2 : B \text{)} \\
&= \llbracket \Theta \mid \Gamma'; \Delta_1, \Delta_2 \vdash_\ell [\xi](\text{let } \langle \rangle = t_2 \text{ in } t_2) : B \rrbracket && \text{(syntactic substitution)}
\end{aligned}$$

•  $(\Theta \mid \Gamma; \Delta_1, \Delta_2 \vdash_\ell (t_1, t_2) : A \otimes B)$ :

$$\begin{aligned}
&\llbracket \Theta \mid \Gamma; \Delta_1, \Delta_2 \vdash_\ell (t_1, t_2) : A \otimes B \rrbracket \circ (F\llbracket \xi \rrbracket \otimes \text{id}_{\llbracket \Theta \vdash_\ell \Delta_1, \Delta_2 \rrbracket}) \\
&= (\llbracket \Theta \mid \Gamma; \Delta_1 \vdash_\ell t_1 : A \rrbracket \otimes \llbracket \Theta \mid \Gamma; \Delta_2 \vdash_\ell t_2 : B \rrbracket) \circ \text{split}_{\Theta, \Gamma, \Delta_1, \Delta_2} \circ (F\llbracket \xi \rrbracket \otimes \text{id}_{\llbracket \Theta \vdash_\ell \Delta_1, \Delta_2 \rrbracket}) \\
&\quad \text{(semantics of } (t_1, t_2) : A \otimes B \text{)} \\
&= (\llbracket t_1 \rrbracket \otimes \llbracket t_2 \rrbracket) \circ ((F\llbracket \xi \rrbracket \otimes \text{id}_{\llbracket \Theta \vdash_\ell \Delta_1 \rrbracket}) \otimes (F\llbracket \xi \rrbracket \otimes \text{id}_{\llbracket \Theta \vdash_\ell \Delta_2 \rrbracket})) \circ \text{split}_{\Theta, \Gamma', \Delta_1, \Delta_2} \quad \text{(Lemma 11.20)} \\
&= (((\llbracket t_1 \rrbracket \circ (F\llbracket \xi \rrbracket \otimes \text{id}_{\llbracket \Theta \vdash_\ell \Delta_1 \rrbracket})) \otimes (\llbracket t_2 \rrbracket \circ (F\llbracket \xi \rrbracket \otimes \text{id}_{\llbracket \Theta \vdash_\ell \Delta_2 \rrbracket}))) \circ \text{split}_{\Theta, \Gamma', \Delta_1, \Delta_2} \quad \text{(SMCC prop.)} \\
&= (\llbracket \Theta \mid \Gamma'; \Delta_1 \vdash_\ell [\xi]t_1 : A \rrbracket \otimes \llbracket \Theta \mid \Gamma'; \Delta_2 \vdash_\ell [\xi]t_2 : B \rrbracket) \circ \text{split}_{\Theta, \Gamma', \Delta_1, \Delta_2} \quad \text{(IHs)} \\
&= \llbracket \Theta \mid \Gamma'; \Delta_1, \Delta_2 \vdash_\ell ([\xi]t_1, [\xi]t_2) : A \otimes B \rrbracket && \text{(semantics of } ([\xi]t_1, [\xi]t_2) : A \otimes B \text{)} \\
&= \llbracket \Theta \mid \Gamma'; \Delta_1, \Delta_2 \vdash_\ell [\xi](t_1, t_2) : A \otimes B \rrbracket && \text{(syntactic substitution)}
\end{aligned}$$

- $(\Theta \mid \Gamma; \Delta_1, \Delta_2 \vdash_\ell \text{let } (a, b) = t_1 \text{ in } t_2 : C)$ :

$$\begin{aligned}
& \llbracket \Theta \mid \Gamma; \Delta_1, \Delta_2 \vdash_\ell \text{let } (a, b) = t_1 \text{ in } t_2 : C \rrbracket \circ (F[\xi] \otimes \text{id}_{\llbracket \Theta \vdash_\ell \Delta_1, \Delta_2 \rrbracket}) \\
&= \llbracket \Theta \mid \Gamma; \Delta_2, a : A, b : B \vdash_\ell t_2 : C \rrbracket \circ \varsigma \circ (\llbracket \Theta \mid \Gamma; \Delta_1 \vdash_\ell t_1 : A \otimes B \rrbracket \otimes \text{id}) \circ \text{split} \circ (F[\xi] \otimes \text{id}) \\
&\quad \text{(semantics of let } (a, b) = t_1 \text{ in } t_2 : C) \\
&= \llbracket t_2 \rrbracket \circ \varsigma \circ (\llbracket t_1 \rrbracket \otimes \text{id}) \circ ((F[\xi] \otimes \text{id}_{\llbracket \Theta \vdash_\ell \Delta_1 \rrbracket}) \otimes (F[\xi] \otimes \text{id}_{\llbracket \Theta \vdash_\ell \Delta_2 \rrbracket})) \circ \text{split}_{\Theta, \Gamma', \Delta_1, \Delta_2} \\
&\quad \text{(Lemma 11.20)} \\
&= \llbracket t_2 \rrbracket \circ \varsigma \circ ((\llbracket t_1 \rrbracket \circ (F[\xi] \otimes \text{id}_{\llbracket \Theta \vdash_\ell \Delta_1 \rrbracket})) \otimes (F[\xi] \otimes \text{id}_{\llbracket \Theta \vdash_\ell \Delta_2 \rrbracket})) \circ \text{split}_{\Theta, \Gamma', \Delta_1, \Delta_2} \quad \text{(SMCC prop.)} \\
&= \llbracket t_2 \rrbracket \circ \varsigma \circ (\llbracket \Theta \mid \Gamma'; \Delta_1 \vdash_\ell [\xi]t_1 : A \otimes B \rrbracket \otimes (F[\xi] \otimes \text{id}_{\llbracket \Theta \vdash_\ell \Delta_2 \rrbracket})) \circ \text{split}_{\Theta, \Gamma', \Delta_1, \Delta_2} \quad \text{(IH on } t_1) \\
&= \llbracket t_2 \rrbracket \circ \varsigma \circ (\text{id}_{\llbracket \Theta \vdash_\ell A \rrbracket} \otimes \text{id}_{\llbracket \Theta \vdash_\ell B \rrbracket} \otimes (F[\xi] \otimes \text{id}_{\llbracket \Theta \vdash_\ell \Delta_2 \rrbracket})) \circ (\llbracket [\xi]t_1 \rrbracket \otimes (\text{id}_{F[\Theta \vdash_c \Gamma']} \otimes \text{id}_{\llbracket \Theta \vdash_\ell \Delta_2 \rrbracket})) \circ \text{split} \\
&\quad \text{(SMCC prop.)} \\
&= \llbracket t_2 \rrbracket \circ (F[\xi] \otimes \text{id}_{\llbracket \Theta \vdash_\ell \Delta_2, a : A, b : B \rrbracket}) \circ \varsigma \circ (\llbracket [\xi]t_1 \rrbracket \otimes \text{id}_{F[\Theta \vdash_c \Gamma'] \otimes \llbracket \Theta \vdash_\ell \Delta_2 \rrbracket}) \circ \text{split}_{\Theta, \Gamma', \Delta_1, \Delta_2} \\
&\quad \text{(naturality of } \varsigma \text{ and SMCC props.)} \\
&= \llbracket \Theta \mid \Gamma'; \Delta_2, a : A, b : B \vdash_\ell [\xi]t_2 : C \rrbracket \circ \varsigma \circ (\llbracket [\xi]t_1 \rrbracket \otimes \text{id}_{F[\Theta \vdash_c \Gamma'] \otimes \llbracket \Theta \vdash_\ell \Delta_2 \rrbracket}) \circ \text{split}_{\Theta, \Gamma', \Delta_1, \Delta_2} \\
&\quad \text{(IH on } t_2) \\
&= \llbracket \Theta \mid \Gamma'; \Delta_1, \Delta_2 \vdash_\ell \text{let } (a, b) = [\xi]t_1 \text{ in } [\xi]t_2 : C \rrbracket \quad \text{(semantics of let } (a, b) = [\xi]t_1 \text{ in } [\xi]t_2 : C) \\
&= \llbracket \Theta \mid \Gamma'; \Delta_1, \Delta_2 \vdash_\ell [\xi](\text{let } (a, b) = t_1 \text{ in } t_2) : C \rrbracket \quad \text{(syntactic substitution)}
\end{aligned}$$

- $(\Theta \mid \Gamma; \Delta \vdash_\ell \text{evt } t : \Diamond A)$ :

$$\begin{aligned}
& \llbracket \Theta \mid \Gamma; \Delta \vdash_\ell \text{evt } t : \Diamond A \rrbracket \circ (F[\xi] \otimes \text{id}_{\llbracket \Theta \vdash_\ell \Delta \rrbracket}) \\
&= \eta_{\llbracket \Theta \vdash_\ell A \rrbracket} \circ \llbracket \Theta \mid \Gamma; \Delta \vdash_\ell t : A \rrbracket \circ (F[\xi] \otimes \text{id}_{\llbracket \Theta \vdash_\ell \Delta \rrbracket}) \quad \text{(semantics of evt } t : \Diamond A) \\
&= \eta_{\llbracket \Theta \vdash_\ell A \rrbracket} \circ \llbracket \Theta \mid \Gamma'; \Delta \vdash_\ell [\xi]t : A \rrbracket \quad \text{(IH)} \\
&= \llbracket \Theta \mid \Gamma'; \Delta \vdash_\ell \text{evt } ([\xi]t) : \Diamond A \rrbracket \quad \text{(semantics of evt } ([\xi]t) : \Diamond A) \\
&= \llbracket \Theta \mid \Gamma'; \Delta \vdash_\ell [\xi](\text{evt } t) : \Diamond A \rrbracket \quad \text{(syntactic substitution)}
\end{aligned}$$

- $(\Theta \mid \Gamma; \Delta \vdash_\ell \text{let evt } a = t_1 \text{ in } t_2 : \Diamond B)$ :

$$\begin{aligned}
& \llbracket \Theta \mid \Gamma; \Delta \vdash_\ell \text{let evt } a = t_1 \text{ in } t_2 : \Diamond B \rrbracket \circ (F[\xi] \otimes \text{id}_{\llbracket \Theta \vdash_\ell \Delta \rrbracket}) \\
&= \mu_{\llbracket \Theta \vdash_\ell B \rrbracket} \circ \Diamond \llbracket t_2 \rrbracket \circ \text{st}_{\llbracket \Theta \vdash_c \Gamma' \rrbracket, \llbracket \Theta \vdash_\ell A \rrbracket}^F \circ (\text{id} \otimes \llbracket t_1 \rrbracket) \circ \varsigma \circ (\text{dup}_{\llbracket \Theta \vdash_c \Gamma' \rrbracket} \otimes \text{id}) \circ (F[\xi] \otimes \text{id}_{\llbracket \Theta \vdash_\ell \Delta \rrbracket}) \\
&\quad \text{(semantics of let evt } a = t_1 \text{ in } t_2 : \Diamond B) \\
&= \mu_{\llbracket \Theta \vdash_\ell B \rrbracket} \circ \Diamond \llbracket t_2 \rrbracket \circ \text{st}_{\llbracket \Theta \vdash_c \Gamma' \rrbracket, \llbracket \Theta \vdash_\ell A \rrbracket}^F \circ (\text{id} \otimes \llbracket t_1 \rrbracket) \circ (F[\xi] \otimes (F[\xi] \otimes \text{id}_{\llbracket \Theta \vdash_\ell \Delta \rrbracket})) \circ \varsigma \circ (\text{dup}_{\llbracket \Theta \vdash_c \Gamma' \rrbracket} \otimes \text{id}) \\
&\quad \text{(naturality of duplication and } \varsigma) \\
&= \mu_{\llbracket \Theta \vdash_\ell B \rrbracket} \circ \Diamond \llbracket t_2 \rrbracket \circ \text{st}_{\llbracket \Theta \vdash_c \Gamma' \rrbracket, \llbracket \Theta \vdash_\ell A \rrbracket}^F \circ (F[\xi] \otimes (\llbracket t_1 \rrbracket \circ (F[\xi] \otimes \text{id}_{\llbracket \Theta \vdash_\ell \Delta \rrbracket}))) \circ \varsigma \circ (\text{dup}_{\llbracket \Theta \vdash_c \Gamma' \rrbracket} \otimes \text{id}) \\
&\quad \text{(SMCC prop.)} \\
&= \mu_{\llbracket \Theta \vdash_\ell B \rrbracket} \circ \Diamond \llbracket t_2 \rrbracket \circ \text{st}_{\llbracket \Theta \vdash_c \Gamma' \rrbracket, \llbracket \Theta \vdash_\ell A \rrbracket}^F \circ (F[\xi] \otimes \llbracket \Theta \mid \Gamma'; \Delta \vdash_\ell [\xi]t_1 : \Diamond A \rrbracket) \circ \varsigma \circ (\text{dup}_{\llbracket \Theta \vdash_c \Gamma' \rrbracket} \otimes \text{id}) \\
&\quad \text{(IH on } t_1) \\
&= \mu_{\llbracket \Theta \vdash_\ell B \rrbracket} \circ \Diamond \llbracket t_2 \rrbracket \circ \Diamond (F[\xi] \otimes \text{id}_{\llbracket \Theta \vdash_\ell A \rrbracket}) \circ \text{st}_{\llbracket \Theta \vdash_c \Gamma' \rrbracket, \llbracket \Theta \vdash_\ell A \rrbracket}^F \circ (\text{id}_{F[\Theta \vdash_c \Gamma']} \otimes \llbracket [\xi]t_1 \rrbracket) \circ \varsigma \circ (\text{dup}_{\llbracket \Theta \vdash_c \Gamma' \rrbracket} \otimes \text{id}) \\
&\quad \text{(naturality of strength)} \\
&= \mu_{\llbracket \Theta \vdash_\ell B \rrbracket} \circ \Diamond (\llbracket t_2 \rrbracket \circ (F[\xi] \otimes \text{id}_{\llbracket \Theta \vdash_\ell A \rrbracket})) \circ \text{st}_{\llbracket \Theta \vdash_c \Gamma' \rrbracket, \llbracket \Theta \vdash_\ell A \rrbracket}^F \circ (\text{id}_{F[\Theta \vdash_c \Gamma']} \otimes \llbracket [\xi]t_1 \rrbracket) \circ \varsigma \circ (\text{dup}_{\llbracket \Theta \vdash_c \Gamma' \rrbracket} \otimes \text{id}) \\
&\quad \text{(functoriality)} \\
&= \mu_{\llbracket \Theta \vdash_\ell B \rrbracket} \circ \Diamond (\llbracket \Theta \mid \Gamma'; a : A \vdash_\ell [\xi]t_2 : \Diamond B \rrbracket) \circ \text{st}_{\llbracket \Theta \vdash_c \Gamma' \rrbracket, \llbracket \Theta \vdash_\ell A \rrbracket}^F \circ (\text{id}_{F[\Theta \vdash_c \Gamma']} \otimes \llbracket [\xi]t_1 \rrbracket) \circ \varsigma \circ (\text{dup}_{\llbracket \Theta \vdash_c \Gamma' \rrbracket} \otimes \text{id}) \\
&\quad \text{(IH on } t_2)
\end{aligned}$$

$$\begin{aligned}
&= \llbracket \Theta \mid \Gamma; \Delta \vdash_\ell \text{let evt } a = [\xi]t_1 \text{ in } [\xi]t_2 : \Diamond B \rrbracket && \text{(semantics of let evt } a = [\xi]t_1 \text{ in } [\xi]t_2 : \Diamond B) \\
&= \llbracket \Theta \mid \Gamma; \Delta \vdash_\ell [\xi]\text{let evt } a = t_1 \text{ in } t_2 : \Diamond B \rrbracket && \text{(syntactic substitution)}
\end{aligned}$$

- $(\Theta \mid \Gamma; \Delta \vdash_\ell t @ \tau : A @ \tau)$ :

$$\begin{aligned}
&\llbracket \Theta \mid \Gamma; \Delta \vdash_\ell t @ \tau : A @ \tau \rrbracket \circ (F\llbracket \xi \rrbracket \otimes \text{id}_{\llbracket \Theta \vdash_\ell \Delta \rrbracket}) \\
&= \llbracket \Theta \mid \Gamma; \Delta \vdash_\ell t :_\tau A \rrbracket \circ (F\llbracket \xi \rrbracket \otimes \text{id}_{\llbracket \Theta \vdash_\ell \Delta \rrbracket}) && \text{(semantics of } t @ \tau : A @ \tau) \\
&= \llbracket \Theta \mid \Gamma'; \Delta \vdash_\ell [\xi]t :_\tau A \rrbracket && \text{(IH)} \\
&= \llbracket \Theta \mid \Gamma'; \Delta \vdash_\ell ([\xi]t) @ \tau : A @ \tau \rrbracket && \text{(semantics of } ([\xi]t) @ \tau : A @ \tau) \\
&= \llbracket \Theta \mid \Gamma'; \Delta \vdash_\ell [\xi](t @ \tau) : A @ \tau \rrbracket && \text{(syntactic substitution)}
\end{aligned}$$

- $(\Theta \mid \Gamma; \Delta_1, \Delta_2 \vdash_\ell \text{let } a @ \tau = t_1 \text{ in } t_2 : B)$ :

$$\begin{aligned}
&\llbracket \Theta \mid \Gamma; \Delta_1, \Delta_2 \vdash_\ell \text{let } a @ \tau = t_1 \text{ in } t_2 : B \rrbracket \circ (F\llbracket \xi \rrbracket \otimes \text{id}_{\llbracket \Theta \vdash_\ell \Delta_1, \Delta_2 \rrbracket}) \\
&= \llbracket \Theta \mid \Gamma; \Delta_2, a :_\tau A \vdash_\ell t_2 : B \rrbracket \circ \varsigma \circ (\llbracket \Theta \mid \Gamma; \Delta_1 \vdash_\ell t_1 : A @ \tau \rrbracket \otimes \text{id}) \circ \text{split} \circ (F\llbracket \xi \rrbracket \otimes \text{id}) \\
&\quad \text{(semantics of let } a @ \tau = t_1 \text{ in } t_2 : B) \\
&= \llbracket t_2 \rrbracket \circ \varsigma \circ (\llbracket t_1 \rrbracket \otimes \text{id}) \circ ((F\llbracket \xi \rrbracket \otimes \text{id}_{\llbracket \Theta \vdash_\ell \Delta_1 \rrbracket}) \otimes (F\llbracket \xi \rrbracket \otimes \text{id}_{\llbracket \Theta \vdash_\ell \Delta_2 \rrbracket})) \circ \text{split}_{\Theta, \Gamma', \Delta_1, \Delta_2} \\
&\quad \text{(Lemma 11.20)} \\
&= \llbracket t_2 \rrbracket \circ \varsigma \circ ((\llbracket t_1 \rrbracket \otimes (F\llbracket \xi \rrbracket \otimes \text{id}_{\llbracket \Theta \vdash_\ell \Delta_1 \rrbracket})) \otimes (F\llbracket \xi \rrbracket \otimes \text{id}_{\llbracket \Theta \vdash_\ell \Delta_2 \rrbracket})) \circ \text{split}_{\Theta, \Gamma', \Delta_1, \Delta_2} && \text{(SMCC prop.)} \\
&= \llbracket t_2 \rrbracket \circ \varsigma \circ (\llbracket \Theta \mid \Gamma'; \Delta_1 \vdash_\ell [\xi]t_1 : A @ \tau \rrbracket \otimes (F\llbracket \xi \rrbracket \otimes \text{id}_{\llbracket \Theta \vdash_\ell \Delta_2 \rrbracket})) \circ \text{split}_{\Theta, \Gamma', \Delta_1, \Delta_2} && \text{(IH on } t_1) \\
&= \llbracket t_2 \rrbracket \circ \varsigma \circ (\text{id}_{\llbracket \vdash_\ell \tau \rrbracket \llbracket \Theta \vdash_\ell A \rrbracket} \otimes (F\llbracket \xi \rrbracket \otimes \text{id}_{\llbracket \Theta \vdash_\ell \Delta_2 \rrbracket})) \circ (\llbracket [\xi]t_1 \rrbracket \otimes (\text{id}_{F\llbracket \Theta \vdash_c \Gamma' \rrbracket} \otimes \text{id}_{\llbracket \Theta \vdash_\ell \Delta_2 \rrbracket})) \circ \text{split} \\
&\quad \text{(SMCC prop.)} \\
&= \llbracket t_2 \rrbracket \circ (F\llbracket \xi \rrbracket \otimes \text{id}_{\llbracket \Theta \vdash_\ell \Delta_2, a :_\tau A \rrbracket}) \circ \varsigma \circ (\llbracket [\xi]t_1 \rrbracket \otimes \text{id}_{F\llbracket \Theta \vdash_c \Gamma' \rrbracket \otimes \llbracket \Theta \vdash_\ell \Delta_2 \rrbracket}) \circ \text{split}_{\Theta, \Gamma', \Delta_1, \Delta_2} \\
&\quad \text{(naturality of } \varsigma \text{ and SMCC props.)} \\
&= \llbracket \Theta \mid \Gamma'; \Delta_2, a :_\tau A \vdash_\ell [\xi]t_2 : B \rrbracket \circ \varsigma \circ (\llbracket [\xi]t_1 \rrbracket \otimes \text{id}_{F\llbracket \Theta \vdash_c \Gamma' \rrbracket \otimes \llbracket \Theta \vdash_\ell \Delta_2 \rrbracket}) \circ \text{split}_{\Theta, \Gamma', \Delta_1, \Delta_2} && \text{(IH on } t_2) \\
&= \llbracket \Theta \mid \Gamma'; \Delta_1, \Delta_2 \vdash_\ell \text{let } a @ \tau = [\xi]t_1 \text{ in } [\xi]t_2 : B \rrbracket && \text{(semantics of let } a @ \tau = [\xi]t_1 \text{ in } [\xi]t_2 : B) \\
&= \llbracket \Theta \mid \Gamma'; \Delta_1, \Delta_2 \vdash_\ell [\xi](\text{let } a @ \tau = t_1 \text{ in } t_2) : B \rrbracket && \text{(syntactic substitution)}
\end{aligned}$$

- $(\Theta \mid \Gamma; \cdot \vdash_\ell \text{runG } e : A)$ :

$$\begin{aligned}
&\llbracket \Theta \mid \Gamma; \cdot \vdash_\ell \text{runG } e : A \rrbracket \circ (F\llbracket \xi \rrbracket \otimes \text{id}_{\llbracket \Theta \vdash_\ell \Delta \rrbracket}) \\
&= \epsilon_{\llbracket \Theta \vdash_\ell A \rrbracket} \circ F\llbracket \Theta \mid \Gamma \vdash_c e : \mathbf{G} A \rrbracket \circ \rho_{F\llbracket \Theta \vdash_c \Gamma \rrbracket} \circ (F\llbracket \xi \rrbracket \otimes \text{id}_{\llbracket \Theta \vdash_\ell \Delta \rrbracket}) && \text{(semantics of runG } e : A) \\
&= \epsilon_{\llbracket \Theta \vdash_\ell A \rrbracket} \circ F\llbracket \Theta \mid \Gamma \vdash_c e : \mathbf{G} A \rrbracket \circ F\llbracket \xi \rrbracket \circ \rho_{F\llbracket \Theta \vdash_c \Gamma' \rrbracket} && \text{(naturality of } \rho) \\
&= \epsilon_{\llbracket \Theta \vdash_\ell A \rrbracket} \circ F(\llbracket \Theta \mid \Gamma \vdash_c e : \mathbf{G} A \rrbracket \circ \llbracket \xi \rrbracket) \circ \rho_{F\llbracket \Theta \vdash_c \Gamma' \rrbracket} && \text{(functoriality)} \\
&= \epsilon_{\llbracket \Theta \vdash_\ell A \rrbracket} \circ F\llbracket \Theta \mid \Gamma' \vdash_c [\xi]e : \mathbf{G} A \rrbracket \circ \rho_{F\llbracket \Theta \vdash_c \Gamma' \rrbracket} && \text{(mutual IH)} \\
&= \llbracket \Theta \mid \Gamma'; \cdot \vdash_\ell \text{runG } ([\xi]e) : A \rrbracket && \text{(semantics of runG } ([\xi]e) : A) \\
&= \llbracket \Theta \mid \Gamma'; \cdot \vdash_\ell [\xi](\text{runG } e) : A \rrbracket && \text{(syntactic substitution)}
\end{aligned}$$

- $(\Theta \mid \Gamma; \cdot \vdash_\ell \mathbf{F} e : \mathbf{F} X)$ :

$$\begin{aligned}
&\llbracket \Theta \mid \Gamma; \cdot \vdash_\ell \mathbf{F} e : \mathbf{F} X \rrbracket \circ (F\llbracket \xi \rrbracket \otimes \text{id}_{\llbracket \Theta \vdash_\ell \Delta \rrbracket}) \\
&= F\llbracket \Theta \mid \Gamma \vdash_c e : X \rrbracket \circ \rho_{F\llbracket \Theta \vdash_c \Gamma \rrbracket} \circ (F\llbracket \xi \rrbracket \otimes \text{id}_{\llbracket \Theta \vdash_\ell \Delta \rrbracket}) && \text{(semantics of } \mathbf{F} e : \mathbf{F} X) \\
&= F\llbracket \Theta \mid \Gamma \vdash_c e : X \rrbracket \circ F\llbracket \xi \rrbracket \circ \rho_{F\llbracket \Theta \vdash_c \Gamma' \rrbracket} && \text{(naturality of } \rho) \\
&= F(\llbracket \Theta \mid \Gamma \vdash_c e : X \rrbracket \circ \llbracket \xi \rrbracket) \circ \rho_{F\llbracket \Theta \vdash_c \Gamma' \rrbracket} && \text{(functoriality)}
\end{aligned}$$

$$\begin{aligned}
&= F(\llbracket \Theta \mid \Gamma \vdash_c [\xi]e : X \rrbracket) \circ \rho_{F[\Theta \vdash_c \Gamma']} && \text{(mutual IH)} \\
&= \llbracket \Theta \mid \Gamma'; \cdot \vdash_\ell F([\xi]e) : F X \rrbracket && \text{(semantics of } F([\xi]e) : F X) \\
&= \llbracket \Theta \mid \Gamma'; \cdot \vdash_\ell ([\xi]F e) : F X \rrbracket && \text{(syntactic substitution)}
\end{aligned}$$

- $(\Theta \mid \Gamma; \Delta_1, \Delta_2 \vdash_\ell \text{let } F x = t_1 \text{ in } t_2 : B):$

$$\begin{aligned}
&\llbracket \Theta \mid \Gamma; \Delta_1, \Delta_2 \vdash_\ell \text{let } a @ \tau = t_1 \text{ in } t_2 : B \rrbracket \circ (F[\llbracket \xi \rrbracket] \otimes \text{id}_{\llbracket \Theta \vdash_\ell \Delta_1, \Delta_2 \rrbracket}) \\
&= \llbracket \Theta \mid \Gamma, x : X; \Delta_2 \vdash_\ell t_2 : B \rrbracket \circ (\mathbf{m}_{\llbracket \Theta \vdash_c \Gamma \rrbracket, \llbracket \Theta \vdash_c X \rrbracket} \otimes \text{id}_{\llbracket \Theta \vdash_\ell \Delta_2 \rrbracket}) \circ \varsigma \\
&\quad \circ (\llbracket \Theta \mid \Gamma; \Delta_1 \vdash_\ell t_1 : F X \rrbracket \otimes \text{id}_{\llbracket \Theta \vdash_\ell \Delta_2 \rrbracket}) \circ \text{split}_{\Theta, \Gamma, \Delta_1, \Delta_2} \circ (F[\llbracket \xi \rrbracket] \otimes \text{id}) \\
&\quad \quad \quad \text{(semantics of let } F x = t_1 \text{ in } t_2 : B) \\
&= \llbracket \Theta \mid \Gamma, x : X; \Delta_2 \vdash_\ell t_2 : B \rrbracket \circ (\mathbf{m}_{\llbracket \Theta \vdash_c \Gamma \rrbracket, \llbracket \Theta \vdash_c X \rrbracket} \otimes \text{id}_{\llbracket \Theta \vdash_\ell \Delta_2 \rrbracket}) \circ \varsigma \\
&\quad \circ (\llbracket \Theta \mid \Gamma; \Delta_1 \vdash_\ell t_1 : F X \rrbracket \otimes \text{id}) \circ ((F[\llbracket \xi \rrbracket] \otimes \text{id}) \otimes (F[\llbracket \xi \rrbracket] \otimes \text{id})) \circ \text{split}_{\Theta, \Gamma', \Delta_1, \Delta_2} \\
&\quad \quad \quad \text{(Lemma 11.20)} \\
&= \llbracket \Theta \mid \Gamma, x : X; \Delta_2 \vdash_\ell t_2 : B \rrbracket \circ (\mathbf{m}_{\llbracket \Theta \vdash_c \Gamma \rrbracket, \llbracket \Theta \vdash_c X \rrbracket} \otimes \text{id}_{\llbracket \Theta \vdash_\ell \Delta_2 \rrbracket}) \circ \varsigma \\
&\quad \circ ((\llbracket t_1 \rrbracket \otimes (F[\llbracket \xi \rrbracket] \otimes \text{id}_{\llbracket \Theta \vdash_\ell \Delta_1 \rrbracket})) \otimes (F[\llbracket \xi \rrbracket] \otimes \text{id}_{\llbracket \Theta \vdash_\ell \Delta_2 \rrbracket})) \circ \text{split}_{\Theta, \Gamma', \Delta_1, \Delta_2} \quad \text{(SMCC prop.)} \\
&= \llbracket \Theta \mid \Gamma, x : X; \Delta_2 \vdash_\ell t_2 : B \rrbracket \circ (\mathbf{m}_{\llbracket \Theta \vdash_c \Gamma \rrbracket, \llbracket \Theta \vdash_c X \rrbracket} \otimes \text{id}_{\llbracket \Theta \vdash_\ell \Delta_2 \rrbracket}) \circ \varsigma \\
&\quad \circ (\llbracket \Theta \mid \Gamma'; \Delta_1 \vdash_\ell [\xi]t_1 : F X \rrbracket \otimes (F[\llbracket \xi \rrbracket] \otimes \text{id}_{\llbracket \Theta \vdash_\ell \Delta_2 \rrbracket})) \circ \text{split}_{\Theta, \Gamma', \Delta_1, \Delta_2} \quad \text{(IH on } t_1) \\
&= \llbracket \Theta \mid \Gamma, x : X; \Delta_2 \vdash_\ell t_2 : B \rrbracket \circ (\mathbf{m}_{\llbracket \Theta \vdash_c \Gamma \rrbracket, \llbracket \Theta \vdash_c X \rrbracket} \otimes \text{id}_{\llbracket \Theta \vdash_\ell \Delta_2 \rrbracket}) \circ \varsigma \\
&\quad \circ (\text{id}_{F[\llbracket \Theta \vdash_c X \rrbracket]} \otimes (F[\llbracket \xi \rrbracket] \otimes \text{id}_{\llbracket \Theta \vdash_\ell \Delta_2 \rrbracket})) \circ (\llbracket [\xi]t_1 \rrbracket \otimes (\text{id}_{F[\llbracket \Theta \vdash_c \Gamma' \rrbracket]} \otimes \text{id}_{\llbracket \Theta \vdash_\ell \Delta_2 \rrbracket})) \circ \text{split}_{\Theta, \Gamma', \Delta_1, \Delta_2} \\
&\quad \quad \quad \text{(SMCC prop.)} \\
&= \llbracket \Theta \mid \Gamma, x : X; \Delta_2 \vdash_\ell t_2 : B \rrbracket \circ (\mathbf{m}_{\llbracket \Theta \vdash_c \Gamma \rrbracket, \llbracket \Theta \vdash_c X \rrbracket} \otimes \text{id}_{\llbracket \Theta \vdash_\ell \Delta_2 \rrbracket}) \circ (F[\llbracket \xi \rrbracket] \otimes F(\text{id}_{\llbracket \Theta \vdash_c X \rrbracket})) \otimes \text{id}_{\llbracket \Theta \vdash_\ell \Delta_2 \rrbracket} \\
&\quad \circ \varsigma \circ (\llbracket [\xi]t_1 \rrbracket \otimes (\text{id}_{F[\llbracket \Theta \vdash_c \Gamma' \rrbracket]} \otimes \text{id}_{\llbracket \Theta \vdash_\ell \Delta_2 \rrbracket})) \circ \text{split} \quad \text{(naturality of } \varsigma \text{ and functoriality)} \\
&= \llbracket \Theta \mid \Gamma, x : X; \Delta_2 \vdash_\ell t_2 : B \rrbracket \circ F(\llbracket \xi \rrbracket \times \text{id}_{\llbracket \Theta \vdash_c X \rrbracket}) \otimes \text{id}_{\llbracket \Theta \vdash_\ell \Delta_2 \rrbracket} \circ (\mathbf{m}_{\llbracket \Theta \vdash_c \Gamma' \rrbracket, \llbracket \Theta \vdash_c X \rrbracket} \otimes \text{id}_{\llbracket \Theta \vdash_\ell \Delta_2 \rrbracket}) \\
&\quad \circ \varsigma \circ (\llbracket [\xi]t_1 \rrbracket \otimes (\text{id}_{F[\llbracket \Theta \vdash_c \Gamma' \rrbracket]} \otimes \text{id}_{\llbracket \Theta \vdash_\ell \Delta_2 \rrbracket})) \circ \text{split}_{\Theta, \Gamma', \Delta_1, \Delta_2} \quad \text{(naturality of } \mathbf{m}) \\
&= \llbracket \Theta \mid \Gamma, x : X; \Delta_2 \vdash_\ell t_2 : B \rrbracket \circ F(\llbracket \xi, x \mapsto x \rrbracket) \otimes \text{id}_{\llbracket \Theta \vdash_\ell \Delta_2 \rrbracket} \circ (\mathbf{m}_{\llbracket \Theta \vdash_c \Gamma' \rrbracket, \llbracket \Theta \vdash_c X \rrbracket} \otimes \text{id}_{\llbracket \Theta \vdash_\ell \Delta_2 \rrbracket}) \\
&\quad \circ \varsigma \circ (\llbracket [\xi]t_1 \rrbracket \otimes (\text{id}_{F[\llbracket \Theta \vdash_c \Gamma' \rrbracket]} \otimes \text{id}_{\llbracket \Theta \vdash_\ell \Delta_2 \rrbracket})) \circ \text{split}_{\Theta, \Gamma', \Delta_1, \Delta_2} \quad \text{(Lemma 11.17)} \\
&= \llbracket \Theta \mid \Gamma', x : X; \Delta_2 \vdash_\ell [\xi]t_2 : B \rrbracket \circ (\mathbf{m}_{\llbracket \Theta \vdash_c \Gamma' \rrbracket, \llbracket \Theta \vdash_c x \rrbracket} \otimes \text{id}_{\llbracket \Theta \vdash_\ell \Delta_2 \rrbracket}) \\
&\quad \circ \varsigma \circ (\llbracket [\xi]t_1 \rrbracket \otimes (\text{id}_{F[\llbracket \Theta \vdash_c \Gamma' \rrbracket]} \otimes \text{id}_{\llbracket \Theta \vdash_\ell \Delta_2 \rrbracket})) \circ \text{split}_{\Theta, \Gamma', \Delta_1, \Delta_2} \quad \text{(IH on } t_2) \\
&= \llbracket \Theta \mid \Gamma'; \Delta_1, \Delta_2 \vdash_\ell \text{let } F x = [\xi]t_1 \text{ in } [\xi]t_2 : B \rrbracket \quad \text{(semantics of let } F x = [\xi]t_1 \text{ in } [\xi]t_2 : B) \\
&= \llbracket \Theta \mid \Gamma'; \Delta_1, \Delta_2 \vdash_\ell [\xi](\text{let } F x = t_1 \text{ in } t_2) : B \rrbracket \quad \text{(syntactic substitution)}
\end{aligned}$$

- $(\Theta \mid \Gamma; \Delta \vdash_\ell \Lambda i : \sigma. t : \forall i : \sigma. A):$

$$\begin{aligned}
&\llbracket \Theta \mid \Gamma; \Delta \vdash_\ell \Lambda i : \sigma. t : \forall i : \sigma. A \rrbracket \circ (F[\llbracket \xi \rrbracket] \otimes \text{id}_{\llbracket \Theta \vdash_\ell \Delta \rrbracket}) \\
&= \phi_{F[\llbracket \Theta \vdash_c \Gamma \rrbracket] \otimes \llbracket \Theta \vdash_\ell \Delta \rrbracket, \llbracket \Theta, i : \sigma \vdash_\ell A \rrbracket}} \left( \llbracket \Theta, i : \sigma \mid \Gamma; \Delta \vdash_\ell t : A \rrbracket \circ \mathbf{m}_{F[\llbracket \Theta \vdash_c \Gamma \rrbracket], \llbracket \Theta \vdash_\ell \Delta \rrbracket}}^{-1} \right) \circ (F[\llbracket \xi \rrbracket] \otimes \text{id}_{\llbracket \Theta \vdash_\ell \Delta \rrbracket}) \\
&\quad \quad \quad \text{(semantics of } \Lambda i : \sigma. t : \forall i : \sigma. A) \\
&= \phi_{F[\llbracket \Theta \vdash_c \Gamma' \rrbracket] \otimes \llbracket \Theta \vdash_\ell \Delta \rrbracket, \llbracket \Theta, i : \sigma \vdash_\ell A \rrbracket}} \left( \llbracket \Theta, i : \sigma \mid \Gamma; \Delta \vdash_\ell t : A \rrbracket \circ \mathbf{m}_{F[\llbracket \Theta \vdash_c \Gamma \rrbracket], \llbracket \Theta \vdash_\ell \Delta \rrbracket}}^{-1} \circ \hat{\mathbf{w}}\mathbf{k}_{[\sigma]}(F[\llbracket \xi \rrbracket] \otimes \text{id}_{\llbracket \Theta \vdash_\ell \Delta \rrbracket}) \right) \\
&\quad \quad \quad \text{(naturality of } \phi) \\
&= \phi \left( \llbracket \Theta, i : \sigma \mid \Gamma; \Delta \vdash_\ell t : A \rrbracket \circ \hat{\mathbf{w}}\mathbf{k}_{[\sigma]}(F[\llbracket \xi \rrbracket]) \otimes \hat{\mathbf{w}}\mathbf{k}_{[\sigma]}(\text{id}_{\llbracket \Theta \vdash_\ell \Delta \rrbracket}) \circ \mathbf{m}_{F[\llbracket \Theta \vdash_c \Gamma' \rrbracket], \llbracket \Theta \vdash_\ell \Delta \rrbracket}}^{-1} \right) \\
&\quad \quad \quad \text{(naturality of } \mathbf{m}^{-1})
\end{aligned}$$



$$\begin{aligned}
&= \phi \left( \llbracket \Theta, i : \sigma \mid \Gamma; \Delta \vdash_\ell t : A \rrbracket \circ F(\mathbf{wk}_{[\sigma]} \llbracket \xi \rrbracket) \otimes \text{id}_{\llbracket \Theta, i : \sigma \vdash_\ell \Delta \rrbracket} \circ \mathbf{m}_{F[\llbracket \Theta \vdash_c \Gamma' \rrbracket, \llbracket \Theta \vdash_\ell \Delta \rrbracket]}^{-1} \right) \\
&\quad \text{(functoriality and LNL property)} \\
&= \phi \left( \llbracket \Theta, i : \sigma \mid \Gamma; \Delta \vdash_\ell t : A \rrbracket \circ F(\llbracket \Theta, i : \sigma \supseteq \Theta \rrbracket^* \llbracket \xi \rrbracket) \otimes \text{id}_{\llbracket \Theta, i : \sigma \vdash_\ell \Delta \rrbracket} \circ \mathbf{m}_{F[\llbracket \Theta \vdash_c \Gamma' \rrbracket, \llbracket \Theta \vdash_\ell \Delta \rrbracket]}^{-1} \right) \\
&\quad \text{(weakening is first projection)} \\
&= \phi \left( \llbracket \Theta, i : \sigma \mid \Gamma; \Delta \vdash_\ell t : A \rrbracket \circ F(\llbracket \Theta, i : \sigma \mid \Gamma' \vdash_c \xi \triangleright \Gamma \rrbracket) \otimes \text{id}_{\llbracket \Theta, i : \sigma \vdash_\ell \Delta \rrbracket} \circ \mathbf{m}_{F[\llbracket \Theta \vdash_c \Gamma' \rrbracket, \llbracket \Theta \vdash_\ell \Delta \rrbracket]}^{-1} \right) \\
&\quad \text{(soundness of index weakening substitution)} \\
&= \phi_{F[\llbracket \Theta \vdash_c \Gamma' \rrbracket \otimes \llbracket \Theta \vdash_\ell \Delta \rrbracket, \llbracket \Theta, i : \sigma \vdash_\ell A \rrbracket]} \left( \llbracket \Theta, i : \sigma \mid \Gamma'; \Delta \vdash_\ell [\xi] t : A \rrbracket \circ \mathbf{m}_{F[\llbracket \Theta \vdash_c \Gamma' \rrbracket, \llbracket \Theta \vdash_\ell \Delta \rrbracket]}^{-1} \right) \quad \text{(IH)} \\
&= \llbracket \Theta \mid \Gamma'; \Delta \vdash_\ell \Lambda i : \sigma. [\xi] t : \forall i : \sigma. A \rrbracket \quad \text{(semantics of } \Lambda i : \sigma. [\xi] t : \forall i : \sigma. A \text{)} \\
&= \llbracket \Theta \mid \Gamma'; \Delta \vdash_\ell [\xi](\Lambda i : \sigma. t) : \forall i : \sigma. A \rrbracket \quad \text{(syntactic substitution)}
\end{aligned}$$

- $(\Theta \mid \Gamma; \Delta \vdash_\ell t_s : \{s/i\}A)$ :

$$\begin{aligned}
&\llbracket \Theta \mid \Gamma; \Delta \vdash_\ell t_s : \{s/i\}A \rrbracket \circ (F[\llbracket \xi \rrbracket] \otimes \text{id}_{\llbracket \Theta \vdash_\ell \Delta \rrbracket}) \\
&= \langle \text{id}_{[\sigma]}, \llbracket \Theta \vdash_s s : \sigma \rrbracket \rangle^+ (\epsilon_{\llbracket \Theta, i : \sigma \vdash_\ell A \rrbracket}) \circ \llbracket \Theta \mid \Gamma; \Delta \vdash_\ell t : \forall i : \sigma. A \rrbracket \circ (F[\llbracket \xi \rrbracket] \otimes \text{id}_{\llbracket \Theta \vdash_\ell \Delta \rrbracket}) \\
&\quad \text{(semantics of } t_s : \{s/i\}A \text{)} \\
&= \langle \text{id}_{[\sigma]}, \llbracket \Theta \vdash_s s : \sigma \rrbracket \rangle^+ (\epsilon_{\llbracket \Theta, i : \sigma \vdash_\ell A \rrbracket}) \circ \llbracket \Theta \mid \Gamma'; \Delta \vdash_\ell [\xi] t : \forall i : \sigma. A \rrbracket \quad \text{(IH)} \\
&= \llbracket \Theta \mid \Gamma'; \Delta \vdash_\ell ([\xi] t)_s : \{s/i\}A \rrbracket \quad \text{(semantics of } ([\xi] t)_s : \{s/i\}A \text{)} \\
&= \llbracket \Theta \mid \Gamma'; \Delta \vdash_\ell [\xi](t_s) : \{s/i\}A \rrbracket \quad \text{(syntactic substitution)}
\end{aligned}$$

- $(\Theta \mid \Gamma; \Delta \vdash_\ell \{s, t\} : \exists i : \sigma. A)$ :

$$\begin{aligned}
&\llbracket \Theta \mid \Gamma; \Delta \vdash_\ell \{s, t\} : \exists i : \sigma. A \rrbracket \circ (F[\llbracket \xi \rrbracket] \otimes \text{id}_{\llbracket \Theta \vdash_\ell \Delta \rrbracket}) \\
&= \langle \text{id}_{[\sigma]}, \llbracket \Theta \vdash_s s : \sigma \rrbracket \rangle^+ (\eta[\llbracket \Theta, i : \sigma \vdash_\ell A \rrbracket]) \circ \llbracket \Theta \mid \Gamma; \Delta \vdash_\ell t : \{s/i\}A \rrbracket \circ (F[\llbracket \xi \rrbracket] \otimes \text{id}_{\llbracket \Theta \vdash_\ell \Delta \rrbracket}) \\
&\quad \text{(semantics of } t_s : \{s/i\}A \text{)} \\
&= \langle \text{id}_{[\sigma]}, \llbracket \Theta \vdash_s s : \sigma \rrbracket \rangle^+ (\epsilon_{\llbracket \Theta, i : \sigma \vdash_\ell A \rrbracket}) \circ \llbracket \Theta \mid \Gamma'; \Delta \vdash_\ell [\xi] t : \{s/i\}A \rrbracket \quad \text{(IH)} \\
&= \llbracket \Theta \mid \Gamma'; \Delta \vdash_\ell \{s, [\xi] t\} : \exists i : \sigma. A \rrbracket \quad \text{(semantics of } \{s, [\xi] t\} : \exists i : \sigma. A \text{)} \\
&= \llbracket \Theta \mid \Gamma'; \Delta \vdash_\ell [\xi]\{s, t\} : \exists i : \sigma. A \rrbracket \quad \text{(syntactic substitution)}
\end{aligned}$$

- $(\Theta \mid \Gamma; \Delta_1, \Delta_2 \vdash_\ell \text{let } \{s, a\} = t_1 \text{ in } t_2 : B)$ :

$$\begin{aligned}
&\llbracket \Theta \mid \Gamma; \Delta_1, \Delta_2 \vdash_\ell \text{let } \{s, a\} = t_1 \text{ in } t_2 : B \rrbracket \circ (F[\llbracket \xi \rrbracket] \otimes \text{id}_{\llbracket \Theta \vdash_\ell \Delta_1, \Delta_2 \rrbracket}) \\
&= \psi_{F[\llbracket \Theta, s : \sigma \vdash_c \Gamma \rrbracket \otimes \llbracket \Theta, s : \sigma \vdash_\ell \Delta_2, a : \{s/i\}A \rrbracket, \llbracket \Theta \vdash_\ell B \rrbracket]} (\llbracket \Theta, s : \sigma \mid \Gamma; \Delta_2, a : \{s/i\}A \vdash_\ell t_2 : B \rrbracket) \circ \hat{\exists}_{[\sigma]}(\varsigma) \\
&\quad \circ \hat{\exists}_{[\sigma]} \left( \text{id} \otimes \mathbf{m}_{F[\llbracket \Theta \vdash_c \Gamma \rrbracket, \llbracket \Theta \vdash_\ell \Delta_2 \rrbracket]}^{-1} \right) \circ (\llbracket \Theta \mid \Gamma; \Delta_1 \vdash_\ell t_1 : \exists i : \sigma. A \rrbracket \otimes \text{id}) \circ \text{split}_{\Theta, \Gamma, \Delta_1, \Delta_2} \circ (F[\llbracket \xi \rrbracket] \otimes \text{id}) \\
&\quad \text{(semantics of let } \{s, a\} = t_1 \text{ in } t_2 : B \text{)} \\
&= \psi_{F[\llbracket \Theta, s : \sigma \vdash_c \Gamma \rrbracket \otimes \llbracket \Theta, s : \sigma \vdash_\ell \Delta_2, a : \{s/i\}A \rrbracket, \llbracket \Theta \vdash_\ell B \rrbracket]} (\llbracket \Theta, s : \sigma \mid \Gamma; \Delta_2, a : \{s/i\}A \vdash_\ell t_2 : B \rrbracket) \circ \hat{\exists}_{[\sigma]}(\varsigma) \\
&\quad \circ \hat{\exists}_{[\sigma]} \left( \text{id} \otimes \mathbf{m}_{F[\llbracket \Theta \vdash_c \Gamma \rrbracket, \llbracket \Theta \vdash_\ell \Delta_2 \rrbracket]}^{-1} \right) \circ ((\llbracket \Theta \mid \Gamma; \Delta_1 \vdash_\ell t_1 : \exists i : \sigma. A \rrbracket \otimes (F[\llbracket \xi \rrbracket] \otimes \text{id})) \otimes (F[\llbracket \xi \rrbracket] \otimes \text{id})) \circ \text{split} \\
&\quad \text{(Lemma 11.20 and SMCC prop)} \\
&= \psi_{F[\llbracket \Theta, s : \sigma \vdash_c \Gamma \rrbracket \otimes \llbracket \Theta, s : \sigma \vdash_\ell \Delta_2, a : \{s/i\}A \rrbracket, \llbracket \Theta \vdash_\ell B \rrbracket]} (\llbracket \Theta, s : \sigma \mid \Gamma; \Delta_2, a : \{s/i\}A \vdash_\ell t_2 : B \rrbracket) \circ \varsigma \\
&\quad \circ \hat{\exists}_{[\sigma]} \left( \text{id} \otimes \mathbf{m}_{F[\llbracket \Theta \vdash_c \Gamma \rrbracket, \llbracket \Theta \vdash_\ell \Delta_2 \rrbracket]}^{-1} \right) \circ (\llbracket \Theta \mid \Gamma'; \Delta_1 \vdash_\ell [\xi] t_1 : \exists i : \sigma. A \rrbracket \otimes (F[\llbracket \xi \rrbracket] \otimes \text{id})) \circ \text{split} \\
&\quad \text{(IH on } t_1 \text{)} \\
&= \psi_{F[\llbracket \Theta, s : \sigma \vdash_c \Gamma \rrbracket \otimes \llbracket \Theta, s : \sigma \vdash_\ell \Delta_2, a : \{s/i\}A \rrbracket, \llbracket \Theta \vdash_\ell B \rrbracket]} (\llbracket \Theta, s : \sigma \mid \Gamma; \Delta_2, a : \{s/i\}A \vdash_\ell t_2 : B \rrbracket) \circ \hat{\exists}_{[\sigma]}(\varsigma)
\end{aligned}$$

$$\begin{aligned}
& \circ \hat{\exists}_{[\sigma]} \left( \text{id} \otimes \mathbf{m}_{F[\Theta \vdash_c \Gamma], [\Theta \vdash_\ell \Delta_2]}^{-1} \right) \circ (\hat{\exists}_{[\sigma]}(\text{id}_{[\Theta, i : \sigma \vdash_\ell A]}) \otimes (F[\xi] \otimes \text{id})) \circ ([[\xi]t_1] \otimes \text{id}) \circ \text{split}_{\Theta, \Gamma', \Delta_1, \Delta_2} \\
& \quad \text{(SMCC prop.)} \\
= & \psi_F[\Theta, s : \sigma \vdash_c \Gamma] \otimes [\Theta, s : \sigma \vdash_\ell \Delta_2, a : \{s/i\}A], [\Theta \vdash_\ell B] ([\Theta, s : \sigma \mid \Gamma; \Delta_2, a : \{s/i\}A \vdash_\ell t_2 : B]) \circ \hat{\exists}_{[\sigma]}(\varsigma) \\
& \circ \hat{\exists}_{[\sigma]} \left( \text{id} \otimes \mathbf{m}_{F[\Theta \vdash_c \Gamma], [\Theta \vdash_\ell \Delta_2]}^{-1} \right) \circ (\hat{\exists}_{[\sigma]}(\text{id}_{[\Theta, i : \sigma \vdash_\ell A]} \otimes \hat{\mathbf{w}}\mathbf{k}_{[\sigma]}(F[\xi] \otimes \text{id}))) \circ ([[\xi]t_1] \otimes \text{id}) \circ \text{split}_{\Theta, \Gamma', \Delta_1, \Delta_2} \\
& \quad \text{(Frobenius reciprocity)} \\
= & \psi_F[\Theta, s : \sigma \vdash_c \Gamma] \otimes [\Theta, s : \sigma \vdash_\ell \Delta_2, a : \{s/i\}A], [\Theta \vdash_\ell B] ([\Theta, s : \sigma \mid \Gamma; \Delta_2, a : \{s/i\}A \vdash_\ell t_2 : B]) \circ \hat{\exists}_{[\sigma]}(\varsigma) \\
& \circ \hat{\exists}_{[\sigma]} \left( \text{id}_{[\Theta, i : \sigma \vdash_\ell A]} \otimes (\mathbf{m}_{F[\Theta \vdash_c \Gamma], [\Theta \vdash_\ell \Delta_2]}^{-1} \circ \hat{\mathbf{w}}\mathbf{k}_{[\sigma]}(F[\xi] \otimes \text{id})) \right) \circ ([[\xi]t_1] \otimes \text{id}) \circ \text{split}_{\Theta, \Gamma', \Delta_1, \Delta_2} \\
& \quad \text{(functoriality and SMCC prop.)} \\
= & \psi_F[\Theta, s : \sigma \vdash_c \Gamma] \otimes [\Theta, s : \sigma \vdash_\ell \Delta_2, a : \{s/i\}A], [\Theta \vdash_\ell B] ([\Theta, s : \sigma \mid \Gamma; \Delta_2, a : \{s/i\}A \vdash_\ell t_2 : B]) \circ \hat{\exists}_{[\sigma]}(\varsigma) \\
& \circ \hat{\exists}_{[\sigma]} \left( \text{id}_{[\Theta, i : \sigma \vdash_\ell A]} \otimes \left( (\hat{\mathbf{w}}\mathbf{k}_{[\sigma]}(F[\xi]) \otimes \hat{\mathbf{w}}\mathbf{k}_{[\sigma]}(\text{id})) \circ \mathbf{m}_{F[\Theta \vdash_c \Gamma'], [\Theta \vdash_\ell \Delta_2]}^{-1} \right) \right) \circ ([[\xi]t_1] \otimes \text{id}) \circ \text{split}_{\Theta, \Gamma', \Delta_1, \Delta_2} \\
& \quad \text{(naturality of } \mathbf{m}^{-1} \text{)} \\
= & \psi_F[\Theta, s : \sigma \vdash_c \Gamma] \otimes [\Theta, s : \sigma \vdash_\ell \Delta_2, a : \{s/i\}A], [\Theta \vdash_\ell B] ([\Theta, s : \sigma \mid \Gamma; \Delta_2, a : \{s/i\}A \vdash_\ell t_2 : B]) \circ \hat{\exists}_{[\sigma]}(\varsigma) \\
& \circ \hat{\exists}_{[\sigma]} \left( (\text{id}_{[\Theta, i : \sigma \vdash_\ell A]} \otimes (\hat{\mathbf{w}}\mathbf{k}_{[\sigma]}(F[\xi]) \otimes \hat{\mathbf{w}}\mathbf{k}_{[\sigma]}(\text{id}))) \circ (\text{id}_{[\Theta, i : \sigma \vdash_\ell A]} \otimes \mathbf{m}_{F[\Theta \vdash_c \Gamma'], [\Theta \vdash_\ell \Delta_2]}^{-1}) \right) \circ ([[\xi]t_1] \otimes \text{id}) \circ \text{split} \\
& \quad \text{(SMCC prop.)} \\
= & \psi_F[\Theta, s : \sigma \vdash_c \Gamma] \otimes [\Theta, s : \sigma \vdash_\ell \Delta_2, a : \{s/i\}A], [\Theta \vdash_\ell B] ([\Theta, s : \sigma \mid \Gamma; \Delta_2, a : \{s/i\}A \vdash_\ell t_2 : B]) \\
& \circ \hat{\exists}_{[\sigma]} \left( \varsigma \circ (\text{id}_{[\Theta, i : \sigma \vdash_\ell A]} \otimes (\hat{\mathbf{w}}\mathbf{k}_{[\sigma]}(F[\xi]) \otimes \hat{\mathbf{w}}\mathbf{k}_{[\sigma]}(\text{id}_{[\Theta \vdash_\ell \Delta_2]}))) \right) \\
& \circ \hat{\exists}_{[\sigma]} (\text{id}_{[\Theta, i : \sigma \vdash_\ell A]} \otimes \mathbf{m}_{F[\Theta \vdash_c \Gamma'], [\Theta \vdash_\ell \Delta_2]}^{-1}) \circ ([[\xi]t_1] \otimes \text{id}) \circ \text{split} \quad \text{(functoriality)} \\
= & \psi_F[\Theta, s : \sigma \vdash_c \Gamma] \otimes [\Theta, s : \sigma \vdash_\ell \Delta_2, a : \{s/i\}A], [\Theta \vdash_\ell B] ([\Theta, s : \sigma \mid \Gamma; \Delta_2, a : \{s/i\}A \vdash_\ell t_2 : B]) \\
& \circ \hat{\exists}_{[\sigma]} \left( ((\hat{\mathbf{w}}\mathbf{k}_{[\sigma]}(F[\xi]) \otimes \hat{\mathbf{w}}\mathbf{k}_{[\sigma]}(\text{id}_{[\Theta \vdash_\ell \Delta_2]})) \otimes \text{id}_{[\Theta, i : \sigma \vdash_\ell A]}) \circ \varsigma \right) \\
& \circ \hat{\exists}_{[\sigma]} (\text{id}_{[\Theta, i : \sigma \vdash_\ell A]} \otimes \mathbf{m}_{F[\Theta \vdash_c \Gamma'], [\Theta \vdash_\ell \Delta_2]}^{-1}) \circ ([[\xi]t_1] \otimes \text{id}) \circ \text{split} \quad \text{(naturality of } \varsigma \text{)} \\
= & \psi_F[\Theta, s : \sigma \vdash_c \Gamma] \otimes [\Theta, s : \sigma \vdash_\ell \Delta_2, a : \{s/i\}A], [\Theta \vdash_\ell B] ([\Theta, s : \sigma \mid \Gamma; \Delta_2, a : \{s/i\}A \vdash_\ell t_2 : B]) \\
& \circ \hat{\exists}_{[\sigma]} \left( (F(\mathbf{w}\mathbf{k}_{[\sigma]}[\Theta \mid \Gamma' \vdash_c \xi \triangleright \Gamma]) \otimes (\text{id}_{[\Theta, s : \sigma \vdash_\ell \Delta_2]} \otimes \text{id}_{[\Theta, i : \sigma \vdash_\ell A]})) \right) \circ \hat{\exists}_{[\sigma]}(\varsigma) \\
& \circ \hat{\exists}_{[\sigma]} (\text{id}_{[\Theta, i : \sigma \vdash_\ell A]} \otimes \mathbf{m}_{F[\Theta \vdash_c \Gamma'], [\Theta \vdash_\ell \Delta_2]}^{-1}) \circ ([[\xi]t_1] \otimes \text{id}) \circ \text{split} \\
& \quad \text{(LNL property, functoriality, and soundness of index substitution)} \\
= & \psi_F[\Theta, s : \sigma \vdash_c \Gamma] \otimes [\Theta, s : \sigma \vdash_\ell \Delta_2, a : \{s/i\}A], [\Theta \vdash_\ell B] ([\Theta, s : \sigma \mid \Gamma; \Delta_2, a : \{s/i\}A \vdash_\ell t_2 : B]) \\
& \circ \hat{\exists}_{[\sigma]} (F[\Theta, s : \sigma \mid \Gamma' \vdash_c \xi \triangleright \Gamma] \otimes \text{id}_{[\Theta, s : \sigma \vdash_\ell \Delta_2, a : \{s/i\}A]}) \\
& \circ \hat{\exists}_{[\sigma]} \left( \varsigma \circ (\text{id} \otimes \mathbf{m}_{F[\Theta \vdash_c \Gamma'], [\Theta \vdash_\ell \Delta_2]}^{-1}) \right) \circ ([\Theta \mid \Gamma'; \Delta_1 \vdash_\ell [\xi]t_1 : \exists i : \sigma. A] \otimes^{\text{[eq]}} \text{id}) \circ \text{split}_{\Theta, \Gamma', \Delta_1, \Delta_2} \\
& \quad \text{(index weakening of substitution and functoriality (using } [\Theta, i : \sigma \vdash_\ell A] = [\Theta, s : \sigma \vdash_\ell \{s/i\}A] \text{))} \\
= & \psi_F[\Theta, s : \sigma \vdash_c \Gamma'] \otimes [\Theta, s : \sigma \vdash_\ell \Delta_2, a : \{s/i\}A], [\Theta \vdash_\ell B] \\
& \quad ([\Theta, s : \sigma \mid \Gamma; \Delta_2, a : \{s/i\}A \vdash_\ell t_2 : B] \circ (F[\Theta, s : \sigma \mid \Gamma' \vdash_c \xi \triangleright \Gamma] \otimes \text{id}_{[\Theta, s : \sigma \vdash_\ell \Delta_2, a : \{s/i\}A]})) \\
& \circ \hat{\exists}_{[\sigma]} \left( \varsigma \circ (\text{id} \otimes \mathbf{m}_{F[\Theta \vdash_c \Gamma'], [\Theta \vdash_\ell \Delta_2]}^{-1}) \right) \circ ([\Theta \mid \Gamma'; \Delta_1 \vdash_\ell [\xi]t_1 : \exists i : \sigma. A] \otimes^{\text{[eq]}} \text{id}) \circ \text{split}_{\Theta, \Gamma', \Delta_1, \Delta_2} \\
& \quad \text{(naturality of } \psi \text{)} \\
= & \psi_F[\Theta, s : \sigma \vdash_c \Gamma'] \otimes [\Theta, s : \sigma \vdash_\ell \Delta_2, a : \{s/i\}A], [\Theta \vdash_\ell B] ([\Theta, s : \sigma \mid \Gamma'; \Delta_2, a : \{s/i\}A \vdash_\ell [\xi]t_2 : B]) \\
& \circ \hat{\exists}_{[\sigma]} \left( \varsigma \circ (\text{id} \otimes \mathbf{m}_{F[\Theta \vdash_c \Gamma'], [\Theta \vdash_\ell \Delta_2]}^{-1}) \right) \circ ([\Theta \mid \Gamma'; \Delta_1 \vdash_\ell [\xi]t_1 : \exists i : \sigma. A] \otimes^{\text{[eq]}} \text{id}) \circ \text{split}_{\Theta, \Gamma', \Delta_1, \Delta_2} \\
& \quad \text{(IH on } t_2 \text{)}
\end{aligned}$$

$$\begin{aligned} &= \llbracket \Theta \mid \Gamma'; \Delta_1, \Delta_2 \vdash_e \text{let } \{s, a\} = [\xi]t_1 \text{ in } [\xi]t_2 : B \rrbracket && \text{(semantics of let } \{s, a\} = [\xi]t_1 \text{ in } [\xi]t_2 : B) \\ &= \llbracket \Theta \mid \Gamma'; \Delta_1, \Delta_2 \vdash_e [\xi](\text{let } \{s, a\} = t_1 \text{ in } t_2) : B \rrbracket && \text{(syntactic substitution)} \end{aligned}$$

$$\begin{aligned}
& (\Theta \mid \Gamma; \Delta_1, \Delta_2 \vdash_\ell \text{select } (t_1, t_2) \text{ as } [a_1 \mapsto t'_1] \parallel [a_2 \mapsto t'_2]: \Diamond C) : \Diamond C \\
&= [\Theta \mid \Gamma; \Delta_1, \Delta_2 \vdash_\ell \text{select } (t_1, t_2) \text{ as } [a_1 \mapsto t'_1] \parallel [a_2 \mapsto t'_2]: \Diamond C] \circ (F[\xi] \otimes \text{id}_{[\Theta \vdash_\ell \Delta_1, \Delta_2]}) \\
&= \mu_{[\Theta \vdash_\ell C]} \circ \Diamond(([[t'_1], [t'_2]] \circ \text{dist}) \circ \text{st}^F \circ (\text{id}_{F[\Theta \vdash_c \Gamma]} \otimes \text{race}_{[\Theta \vdash_\ell A], [\Theta \vdash_\ell B]})) \circ (\text{id}_{F[\Theta \vdash_c \Gamma]} \otimes [[t_1] \otimes [t_2]]) \\
&\quad \circ (\text{split}_{\Theta, \Gamma, \Delta_1, \Delta_2} \otimes \text{id}_{F[\Theta \vdash_c \Gamma]}) \circ \varsigma \circ (\text{dup}_{[\Theta \vdash_c \Gamma]} \otimes \text{id}) \circ (F[\xi] \otimes \text{id}_{[\Theta \vdash_\ell \Delta_1, \Delta_2]}) \\
&\hspace{10cm} (\text{semantics of select}) \\
&= \mu_{[\Theta \vdash_\ell C]} \circ \Diamond(([[t'_1], [t'_2]] \circ \text{dist}) \circ \text{st}^F \circ (\text{id}_{F[\Theta \vdash_c \Gamma]} \otimes \text{race}_{[\Theta \vdash_\ell A], [\Theta \vdash_\ell B]})) \circ (\text{id}_{F[\Theta \vdash_c \Gamma]} \otimes ([t_1] \otimes [t_2])) \\
&\quad \circ (F[\xi] \otimes (F[\xi] \otimes \text{id}_{[\Theta \vdash_\ell \Delta_1]})) \circ (F[\xi] \otimes \text{id}_{[\Theta \vdash_\ell \Delta_2]}) \circ (\text{split}_{\Theta, \Gamma', \Delta_1, \Delta_2} \otimes \text{id}_{F[\Theta \vdash_c \Gamma']}) \circ \varsigma \circ (\text{dup}_{[\Theta \vdash_c \Gamma']} \otimes \text{id}) \\
&\hspace{10cm} (\text{naturality}) \\
&= \mu_{[\Theta \vdash_\ell C]} \circ \Diamond(([[t'_1], [t'_2]] \circ \text{dist}) \circ \text{st}^F \circ (\text{id}_{F[\Theta \vdash_c \Gamma]} \otimes \text{race}_{[\Theta \vdash_\ell A], [\Theta \vdash_\ell B]})) \\
&\quad \circ (F[\xi] \otimes ((\Theta \mid \Gamma; \Delta_1 \vdash_\ell t_1: \Diamond A) \circ (F[\xi] \otimes \text{id}_{[\Theta \vdash_\ell \Delta_1]}))) \circ ((\Theta \mid \Gamma; \Delta_2 \vdash_\ell t_2: \Diamond B) \circ (F[\xi] \otimes \text{id}_{[\Theta \vdash_\ell \Delta_2]}))) \\
&\quad \circ (\text{split}_{\Theta, \Gamma', \Delta_1, \Delta_2} \otimes \text{id}_{F[\Theta \vdash_c \Gamma']}) \circ \varsigma \circ (\text{dup}_{[\Theta \vdash_c \Gamma']} \otimes \text{id}) \\
&\hspace{10cm} (\text{SMCC prop.}) \\
&= \mu_{[\Theta \vdash_\ell C]} \circ \Diamond(([[t'_1], [t'_2]] \circ \text{dist}) \circ \text{st}^F \circ (\text{id}_{F[\Theta \vdash_c \Gamma]} \otimes \text{race}_{[\Theta \vdash_\ell A], [\Theta \vdash_\ell B]})) \\
&\quad \circ (F[\xi] \otimes (\Theta \mid \Gamma'; \Delta_1 \vdash_\ell [\xi]t_1: \Diamond A) \otimes (\Theta \mid \Gamma'; \Delta_2 \vdash_\ell [\xi]t_2: \Diamond B)) \\
&\quad \circ (\text{split}_{\Theta, \Gamma', \Delta_1, \Delta_2} \otimes \text{id}_{F[\Theta \vdash_c \Gamma']}) \circ \varsigma \circ (\text{dup}_{[\Theta \vdash_c \Gamma']} \otimes \text{id}) \\
&\hspace{10cm} (\text{IH on } t_1 \text{ and } t_2) \\
&= \mu_{[\Theta \vdash_\ell C]} \circ \Diamond(([[t'_1], [t'_2]] \circ \text{dist}) \circ \text{st}^F \\
&\quad \circ (\text{id}_{F[\Theta \vdash_c \Gamma]} \otimes \text{race}_{[\Theta \vdash_\ell A], [\Theta \vdash_\ell B]})) \circ (F[\xi] \otimes (\Diamond \text{id}_{[\Theta \vdash_\ell A]} \otimes \Diamond \text{id}_{[\Theta \vdash_\ell B]})) \\
&\quad \circ (\text{id}_{F[\Theta \vdash_c \Gamma]} \otimes [[[\xi]t_1] \otimes [[\xi]t_2]]) \circ (\text{split}_{\Theta, \Gamma', \Delta_1, \Delta_2} \otimes \text{id}_{F[\Theta \vdash_c \Gamma']}) \circ \varsigma \circ (\text{dup}_{[\Theta \vdash_c \Gamma']} \otimes \text{id}) \\
&\hspace{10cm} (\text{SMCC prop. and functoriality}) \\
&= \mu_{[\Theta \vdash_\ell C]} \circ \Diamond(([[t'_1], [t'_2]] \circ \text{dist}) \circ \text{st}^F \circ (F[\xi] \otimes ((\text{id}_{[\Theta \vdash_\ell A]} \otimes \Diamond \text{id}_{[\Theta \vdash_\ell B]}) \oplus (\Diamond \text{id}_{[\Theta \vdash_\ell A]} \otimes \text{id}_{[\Theta \vdash_\ell B]})))) \\
&\quad \circ (\text{id}_{F[\Theta \vdash_c \Gamma']} \otimes \text{race}_{[\Theta \vdash_\ell A], [\Theta \vdash_\ell B]}) \\
&\quad \circ (\text{id}_{F[\Theta \vdash_c \Gamma]} \otimes [[[\xi]t_1] \otimes [[[\xi]t_2]]) \circ (\text{split}_{\Theta, \Gamma', \Delta_1, \Delta_2} \otimes \text{id}_{F[\Theta \vdash_c \Gamma']}) \circ \varsigma \circ (\text{dup}_{[\Theta \vdash_c \Gamma']} \otimes \text{id}) \\
&\hspace{10cm} (\text{naturality of race}) \\
&= \mu_{[\Theta \vdash_\ell C]} \circ \Diamond(([[t'_1], [t'_2]] \circ \text{dist}) \circ \Diamond(F[\xi] \otimes ((\text{id}_{[\Theta \vdash_\ell A]} \otimes \Diamond \text{id}_{[\Theta \vdash_\ell B]}) \oplus (\Diamond \text{id}_{[\Theta \vdash_\ell A]} \otimes \text{id}_{[\Theta \vdash_\ell B]})))) \circ \text{st}^F \\
&\quad \circ (\text{id}_{F[\Theta \vdash_c \Gamma']} \otimes \text{race}_{[\Theta \vdash_\ell A], [\Theta \vdash_\ell B]}) \\
&\quad \circ (\text{id}_{F[\Theta \vdash_c \Gamma]} \otimes [[[\xi]t_1] \otimes [[[\xi]t_2]]) \circ (\text{split}_{\Theta, \Gamma', \Delta_1, \Delta_2} \otimes \text{id}_{F[\Theta \vdash_c \Gamma']}) \circ \varsigma \circ (\text{dup}_{[\Theta \vdash_c \Gamma']} \otimes \text{id}) \\
&\hspace{10cm} (\text{naturality of strength}) \\
&= \mu_{[\Theta \vdash_\ell C]} \circ \Diamond(([[t'_1], [t'_2]] \circ \text{dist} \circ (F[\xi] \otimes (\text{id}_{[\Theta \vdash_\ell A]} \otimes \Diamond \text{id}_{[\Theta \vdash_\ell B]}) \oplus (\Diamond \text{id}_{[\Theta \vdash_\ell A]} \otimes \text{id}_{[\Theta \vdash_\ell B]})))) \circ \text{st}^F \\
&\quad \circ (\text{id}_{F[\Theta \vdash_c \Gamma']} \otimes \text{race}_{[\Theta \vdash_\ell A], [\Theta \vdash_\ell B]}) \\
&\quad \circ (\text{id}_{F[\Theta \vdash_c \Gamma]} \otimes [[[\xi]t_1] \otimes [[[\xi]t_2]]) \circ (\text{split}_{\Theta, \Gamma', \Delta_1, \Delta_2} \otimes \text{id}_{F[\Theta \vdash_c \Gamma']}) \circ \varsigma \circ (\text{dup}_{[\Theta \vdash_c \Gamma']} \otimes \text{id}) \\
&\hspace{10cm} (\text{functoriality}) \\
&= \mu_{[\Theta \vdash_\ell C]} \circ \Diamond\left(\left([\Theta \mid \Gamma; a: A, t_2: \Diamond B \vdash_\ell t'_1: \Diamond C], [\Theta \mid \Gamma; t_1: A, b: B \vdash_\ell t'_2: \Diamond C]\right)\right. \\
&\quad \left.\circ ((F[\xi] \otimes \text{id}_{a:A, t_2: \Diamond B}) \otimes (F[\xi] \otimes \text{id}_{t_1: \Diamond A, b: B}))\right) \\
&\quad \circ \Diamond \text{dist} \circ \text{st}^F \circ (\text{id}_{F[\Theta \vdash_c \Gamma']} \otimes \text{race}_{[\Theta \vdash_\ell A], [\Theta \vdash_\ell B]}) \\
&\quad \circ (\text{id}_{F[\Theta \vdash_c \Gamma]} \otimes [[[\xi]t_1] \otimes [[[\xi]t_2]]) \circ (\text{split}_{\Theta, \Gamma', \Delta_1, \Delta_2} \otimes \text{id}_{F[\Theta \vdash_c \Gamma']}) \circ \varsigma \circ (\text{dup}_{[\Theta \vdash_c \Gamma']} \otimes \text{id}) \\
&\hspace{10cm} (\text{naturality of dist and functoriality}) \\
&= \mu_{[\Theta \vdash_\ell C]} \circ \Diamond\left(\left([\Theta \mid \Gamma'; a: A, t_2: \Diamond B \vdash_\ell [\xi]t'_1: \Diamond C], [\Theta \mid \Gamma'; t_1: A, b: B \vdash_\ell [\xi]t'_2: \Diamond C]\right)\right)
\end{aligned}$$

$$\begin{aligned}
& \circ \diamond \text{dist} \circ \text{st}^F \circ (\text{id}_{F[\Theta \vdash_c \Gamma']} \otimes \text{race}_{[\Theta \vdash_\ell A], [\Theta \vdash_\ell B]}) \\
& \circ (\text{id}_{F[\Theta \vdash_c \Gamma]} \otimes [[[\xi]t_1]] \otimes [[[\xi]t_2]]) \circ (\text{split}_{\Theta, \Gamma', \Delta_1, \Delta_2} \otimes \text{id}_{F[\Theta \vdash_c \Gamma']}) \circ \varsigma \circ (\text{dup}_{[\Theta \vdash_c \Gamma']} \otimes \text{id}) \\
& \quad \text{(IH on } t'_1 \text{ and } t'_2) \\
= & \mu_{[\Theta \vdash_\ell C]} \circ \diamond ([[\Theta \mid \Gamma'; a : A, t_2 : \diamond B \vdash_\ell [\xi]t'_1 : \diamond C]], [[\Theta \mid \Gamma'; t_1 : A, b : B \vdash_\ell [\xi]t'_2 : \diamond C]]) \circ \text{dist} \\
& \circ \text{st}^F \circ (\text{id}_{F[\Theta \vdash_c \Gamma']} \otimes \text{race}_{[\Theta \vdash_\ell A], [\Theta \vdash_\ell B]}) \\
& \circ (\text{id}_{F[\Theta \vdash_c \Gamma]} \otimes [[[\xi]t_1]] \otimes [[[\xi]t_2]]) \circ (\text{split}_{\Theta, \Gamma', \Delta_1, \Delta_2} \otimes \text{id}_{F[\Theta \vdash_c \Gamma']}) \circ \varsigma \circ (\text{dup}_{[\Theta \vdash_c \Gamma']} \otimes \text{id}) \\
& \quad \text{(functoriality)} \\
= & [[\Theta \mid \Gamma'; \Delta_1, \Delta_2 \vdash_\ell \text{select}([\xi]t_1, [\xi]t_2) \text{ as } [a_1 \mapsto [\xi]t'_1] \parallel [a_2 \mapsto [\xi]t'_2] : \diamond C]] \quad \text{(semantics of select)} \\
= & [[\Theta \mid \Gamma'; \Delta_1, \Delta_2 \vdash_\ell [\xi](\text{select}(t_1, t_2) \text{ as } [a_1 \mapsto t'_1] \parallel [a_2 \mapsto t'_2]) : \diamond C]] \quad \text{(syntactic substitution)}
\end{aligned}$$

□

## 11.3 Linear substitution

### 11.3.1 Interpretation of linear substitution

**Definition 11.22.** We interpret a linear substitution  $\Theta; \Gamma \mid \Delta' \vdash_\ell \hat{\xi} \triangleright \Delta$  as a morphism  $[[\hat{\xi}]] : [[\Theta \vdash_\ell \Delta']] \rightarrow^{[\Theta]} [[\Theta \vdash_\ell \Delta]]$  in the category  $\text{Rel}_{\mathcal{R}}^{[\Theta]}$ :

$$\begin{aligned}
[[\Theta; \Gamma \mid \cdot \vdash_\ell \diamond \triangleright \cdot]] & \triangleq \text{id}_{\Gamma'} : \Gamma' \rightarrow'_{\mathcal{R}} \Gamma' \\
[[\Theta; \Gamma \mid \Delta'_1, \Delta'_2 \vdash_\ell \hat{\xi}, a \mapsto t \triangleright \Delta_1, a :_\tau A]] & \triangleq [[\Theta; \Gamma \mid \Delta'_1 \vdash_\ell \hat{\xi} \triangleright \Delta_1]] \otimes' [[\Theta \mid \Gamma; \Delta'_2 \vdash_\ell t : A]] \\
& : [[\Theta \vdash_\ell \Delta'_1]] \otimes [[\Theta \vdash_\ell \Delta'_2]] \rightarrow'_{\mathcal{R}} [[\Theta \vdash_\ell \Delta_1]] \otimes' [[\Theta \vdash_\ell A]]
\end{aligned}$$

As before, we lift all the standard constructions (such as  $\text{I}$ ) into the  $[[\Theta]]$ -indexed setting, writing  $[\![\cdot]\!]$  when needed. However, since in term-level substitutions the index context never changes, in the rest of this section we will not explicitly mark the lifting. Unlike in the case of index substitution, linear substitutions live in the category  $\text{Rel}_{\mathcal{R}}^{[\Theta]}$  for an index context  $\Theta$  and are therefore on the same level as the morphisms interpreting the terms. Thus the action of substitution will correspond to composition, rather than a pullback.

**Lemma 11.23** (Semantics of linear context extension). For a substitution  $\Theta; \Gamma \mid \Delta' \vdash_\ell \hat{\xi} \triangleright \Delta$  and linear context  $\Delta''$ , we have:

$$\begin{aligned}
[[\Theta; \Gamma \mid \Delta', \Delta'' \vdash_\ell \hat{\xi}, \text{id}_{\Delta''} \triangleright \Delta, \Delta'']] & = [[\xi]] \times \text{id}_{[[\Theta \vdash_c X]]} \\
& : [[\Theta \vdash_c \Delta']] \otimes [[\Theta \vdash_c X]] \rightarrow [[\Theta \vdash_c \Gamma]] \otimes [[\Theta \vdash_c X]]
\end{aligned}$$

*Proof.*

$$\begin{aligned}
& [[\Theta \mid \Gamma', x : X \vdash_c \xi, x \mapsto x \triangleright \Gamma, x : X]] \\
= & \langle [[\Theta \mid \Gamma', x : X \vdash_c \xi \triangleright \Gamma]], [[\Theta \mid \Gamma', x : X \vdash_c x : X]] \rangle \\
= & \langle [[\Theta \mid \Gamma', x : X \vdash_c \xi \triangleright \Gamma]], \pi_2 \rangle \\
= & \langle [[\Theta \mid \Gamma' \vdash_c \xi \triangleright \Gamma]] \circ [[\Gamma', x : X \supseteq_\Theta \Gamma']], \pi_2 \rangle \quad \text{(soundness of weakening)} \\
= & \langle [[\Theta \mid \Gamma' \vdash_c \xi \triangleright \Gamma]] \circ \pi_1, \pi_2 \rangle \\
= & [[\Theta \mid \Gamma' \vdash_c \xi \triangleright \Gamma]] \times \text{id}_{[[\Theta \vdash_c X]]}
\end{aligned}$$

□

**Lemma 11.24.** For contexts  $\Theta, \Gamma, \Delta$  a linear substitution  $\Theta; \Gamma \mid \Delta' \vdash_{\ell} \hat{\xi} \triangleright \Delta$ , we have:

$$\begin{aligned} \text{drop}_{\Theta, \Gamma, \Delta} \circ (\text{id}_{F[\Theta \vdash_c \Gamma]} \otimes \llbracket \hat{\xi} \rrbracket) &= \llbracket \hat{\xi} \rrbracket \circ \text{drop}_{\Theta, \Gamma, \Delta'} \\ \text{split}_{\Theta, \Gamma, \Delta_1, \Delta_2} \circ (\text{id}_{F[\Theta \vdash_c \Gamma]} \otimes \llbracket \hat{\xi}_1, \hat{\xi}_2 \rrbracket) &= \left( (\text{id}_{F[\Theta \vdash_c \Gamma]} \otimes \llbracket \hat{\xi}_1 \rrbracket) \otimes (\text{id}_{F[\Theta \vdash_c \Gamma]} \otimes \llbracket \hat{\xi}_2 \rrbracket) \right) \circ \text{split}_{\Theta, \Gamma, \Delta'_1, \Delta'_2} \end{aligned}$$

*Proof.* The property for **drop** follows from the naturality of  $\mathbf{u}$  and  $\lambda$ . For **split**, we use the substitution separation transformation:

$$\begin{aligned} & \text{split}_{\Theta, \Gamma, \Delta_1, \Delta_2} \circ (\text{id}_{F[\Theta \vdash_c \Gamma]} \otimes \llbracket \hat{\xi}_1, \hat{\xi}_2 \rrbracket) \\ &= \varsigma \circ (\text{dup}_{[\Theta \vdash_c \Gamma]} \otimes \text{sep}_{\Delta_1, \Delta_2}) \circ (\text{id}_{F[\Theta \vdash_c \Gamma]} \otimes \llbracket \hat{\xi}_1, \hat{\xi}_2 \rrbracket) && \text{(definition of split)} \\ &= \varsigma \circ (\text{dup}_{[\Theta \vdash_c \Gamma]} \otimes (\text{sep}_{\Delta_1, \Delta_2} \circ \llbracket \hat{\xi}_1, \hat{\xi}_2 \rrbracket)) && \text{(bifunctionality)} \\ &= \varsigma \circ (\text{dup}_{[\Theta \vdash_c \Gamma]} \otimes (\llbracket \hat{\xi}_1 \rrbracket \otimes \llbracket \hat{\xi}_2 \rrbracket \circ \text{sep}_{\Delta'_1, \Delta'_2})) && \text{(naturality of sep)} \\ &= \varsigma \circ \left( (\text{id}_{F[\Theta \vdash_c \Gamma]} \otimes \text{id}_{F[\Theta \vdash_c \Gamma]}) \otimes (\llbracket \hat{\xi}_1 \rrbracket \otimes \llbracket \hat{\xi}_2 \rrbracket) \right) \circ (\text{dup}_{[\Theta \vdash_c \Gamma]} \otimes \text{sep}_{\Delta'_1, \Delta'_2}) && \text{(bifunctionality)} \\ &= \left( (\text{id}_{F[\Theta \vdash_c \Gamma]} \otimes \llbracket \hat{\xi}_1 \rrbracket) \otimes (\text{id}_{F[\Theta \vdash_c \Gamma]} \otimes \llbracket \hat{\xi}_2 \rrbracket) \right) \circ \varsigma \circ (\text{dup}_{[\Theta \vdash_c \Gamma]} \otimes \text{sep}_{\Delta'_1, \Delta'_2}) && \text{(naturality of } \varsigma) \\ &= \left( (\text{id}_{F[\Theta \vdash_c \Gamma]} \otimes \llbracket \hat{\xi}_1 \rrbracket) \otimes (\text{id}_{F[\Theta \vdash_c \Gamma]} \otimes \llbracket \hat{\xi}_2 \rrbracket) \right) \circ \text{split}_{\Theta, \Gamma, \Delta'_1, \Delta'_2} && \text{(definition of split)} \end{aligned}$$

□

**Theorem 11.25** (Soundness of linear substitution into linear terms). If  $\Theta \mid \Delta; \Gamma \vdash_{\ell} t : A$  and  $\Theta; \Gamma \mid \Delta' \vdash_{\ell} \hat{\xi} \triangleright \Delta$ , then

$$\llbracket \Theta \mid \Gamma; \Delta \vdash_{\ell} t : A \rrbracket \circ (\text{id}_{F[\Theta \vdash_c \Gamma]} \otimes \llbracket \hat{\xi} \rrbracket) = \llbracket \Theta \mid \Gamma; \Delta' \vdash_{\ell} [\hat{\xi}]t : A \rrbracket$$

*Proof.* We proceed by induction on the derivation of the well-formed type judgment  $\Theta \mid \Gamma; \Delta \vdash_{\ell} t : A$ .

- $(\Theta \mid \Gamma; a : A \vdash_{\ell} a : A \text{ and } \Theta; \Gamma \mid \Delta' \vdash_{\ell} a \mapsto t \triangleright a : A)$ :

$$\begin{aligned} & \llbracket \Theta \mid \Gamma; a : A \vdash_{\ell} a : A \rrbracket \circ (\text{id}_{F[\Theta \vdash_c \Gamma]} \otimes \llbracket \Theta; \Gamma \mid \Delta' \vdash_{\ell} a \mapsto t \triangleright a : A \rrbracket) \\ &= \text{drop}_{\Theta, \Gamma, a : A} \circ (\text{id}_{F[\Theta \vdash_c \Gamma]} \otimes \llbracket \Theta; \Gamma \mid \Delta' \vdash_{\ell} a \mapsto t \triangleright a : A \rrbracket) && \text{(semantics of } a : A) \\ &= \llbracket \Theta; \Gamma \mid \Delta' \vdash_{\ell} a \mapsto t \triangleright a : A \rrbracket \circ \text{drop}_{\Theta, \Gamma, \Delta'} && \text{(Lemma 11.24)} \\ &= \llbracket \Theta \mid \Gamma; \Delta' \vdash_{\ell} t : A \rrbracket && \text{(interpretation of single substitution)} \\ &= \llbracket \Theta \mid \Gamma; \Delta' \vdash_{\ell} [a \mapsto t]a : A \rrbracket && \text{(syntactic substitution)} \end{aligned}$$

- $(\Theta \mid \Gamma; \Delta \vdash_{\ell} \lambda a. t : A \multimap B)$ :

$$\begin{aligned} & \llbracket \Theta \mid \Gamma; \Delta \vdash_{\ell} \lambda a. t : A \multimap B \rrbracket \circ (\text{id}_{F[\Theta \vdash_c \Gamma]} \otimes \llbracket \hat{\xi} \rrbracket) \\ &= \text{curry}(\llbracket \Theta \mid \Gamma; \Delta, a : A \vdash_{\ell} t : B \rrbracket \circ \varsigma) \circ (\text{id}_{F[\Theta \vdash_c \Gamma]} \otimes \llbracket \hat{\xi} \rrbracket) && \text{(semantics of } \lambda a. t : A \multimap B) \\ &= \text{curry}(\llbracket \Theta \mid \Gamma; \Delta, a : A \vdash_{\ell} t : B \rrbracket \circ \varsigma \circ ((\text{id}_{F[\Theta \vdash_c \Gamma]} \otimes \llbracket \hat{\xi} \rrbracket) \otimes \text{id}_{[\Theta \vdash_{\ell} A]})) && \text{(SMCC law)} \\ &= \text{curry}(\llbracket \Theta \mid \Gamma; \Delta, a : A \vdash_{\ell} t : B \rrbracket \circ (\text{id}_{F[\Theta \vdash_c \Gamma]} \otimes (\llbracket \hat{\xi} \rrbracket \otimes \text{id}_{[\Theta \vdash_{\ell} A]})) \circ \varsigma) && \text{(naturality of } \varsigma) \\ &= \text{curry}(\llbracket \Theta \mid \Gamma; \Delta, a : A \vdash_{\ell} t : B \rrbracket \circ (\text{id}_{F[\Theta \vdash_c \Gamma]} \otimes \llbracket \hat{\xi}, a \mapsto a \rrbracket) \circ \varsigma) && \text{(def. of linear substitution)} \\ &= \text{curry}(\llbracket \Theta \mid \Gamma; \Delta', a : A \vdash_{\ell} [\hat{\xi}]t : B \rrbracket \circ \varsigma) && \text{(IH)} \\ &= \llbracket \Theta \mid \Gamma; \Delta' \vdash_{\ell} \lambda a. [\hat{\xi}]t : A \multimap B \rrbracket && \text{(semantics of } \lambda a. [\hat{\xi}]t : A \multimap B) \\ &= \llbracket \Theta \mid \Gamma'; \Delta' \vdash_{\ell} [\hat{\xi}](\lambda a. t) : A \multimap B \rrbracket && \text{(syntactic substitution)} \end{aligned}$$

- $(\Theta \mid \Gamma; \Delta_1, \Delta_2 \vdash_\ell t_1 t_2 : B)$ :

$$\begin{aligned}
& \llbracket \Theta \mid \Gamma; \Delta_1, \Delta_2 \vdash_\ell t_1 t_2 : B \rrbracket \circ (\text{id}_{F[\Theta \vdash_c \Gamma]} \otimes \llbracket \hat{\xi}_1, \hat{\xi}_2 \rrbracket) \\
&= \text{eval} \circ (\llbracket \Theta \mid \Gamma; \Delta_1 \vdash_\ell t_1 : A \multimap B \rrbracket \otimes \llbracket \Theta \mid \Gamma; \Delta_2 \vdash_\ell t_2 : A \rrbracket) \circ \text{split}_{\Theta, \Gamma, \Delta_1, \Delta_2} \circ (\text{id}_{F[\Theta \vdash_c \Gamma]} \otimes \llbracket \hat{\xi}_1, \hat{\xi}_2 \rrbracket) \\
&\quad \text{(semantics of } t_1 t_2 : B \text{)} \\
&= \text{eval} \circ (\llbracket t_1 \rrbracket \otimes \llbracket t_2 \rrbracket) \circ ((\text{id}_{F[\Theta \vdash_c \Gamma]} \otimes \llbracket \hat{\xi}_1 \rrbracket) \otimes (\text{id}_{F[\Theta \vdash_c \Gamma]} \otimes \llbracket \hat{\xi}_2 \rrbracket)) \circ \text{split}_{\Theta, \Gamma, \Delta'_1, \Delta'_2} \quad \text{(Lemma 11.20)} \\
&= \text{eval} \circ ((\llbracket t_1 \rrbracket \circ (\text{id}_{F[\Theta \vdash_c \Gamma]} \otimes \llbracket \hat{\xi}_1 \rrbracket)) \otimes (\llbracket t_2 \rrbracket \circ (\text{id}_{F[\Theta \vdash_c \Gamma]} \otimes \llbracket \hat{\xi}_2 \rrbracket))) \circ \text{split}_{\Theta, \Gamma, \Delta'_1, \Delta'_2} \quad \text{(CCC prop.)} \\
&= \text{eval} \circ (\llbracket \Theta \mid \Gamma; \Delta'_1 \vdash_\ell [\xi]t_1 : A \multimap B \rrbracket \otimes \llbracket \Theta \mid \Gamma; \Delta'_2 \vdash_\ell [\xi]t_2 : A \rrbracket) \circ \text{split}_{\Theta, \Gamma, \Delta'_1, \Delta'_2} \quad \text{(IHs)} \\
&= \llbracket \Theta \mid \Gamma; \Delta'_1, \Delta'_2 \vdash_\ell ([\xi]t_1)([\xi]t_2) : B \rrbracket \quad \text{(semantics of } ([\xi]t_1)([\xi]t_2) : B \text{)} \\
&= \llbracket \Theta \mid \Gamma'; \Delta'_1, \Delta'_2 \vdash_\ell [\xi](t_1 t_2) : B \rrbracket \quad \text{(syntactic substitution)}
\end{aligned}$$

- $(\Theta \mid \Gamma; \cdot \vdash_\ell \bullet : \mathbb{I})$ :

$$\begin{aligned}
& \llbracket \Theta \mid \Gamma; \cdot \vdash_\ell \bullet : \mathbb{I} \rrbracket \circ (\text{id}_{F[\Theta \vdash_c \Gamma]} \otimes \llbracket \Theta; \Gamma \mid \cdot \vdash_\ell \diamond \triangleright \cdot \rrbracket) \\
&= \text{drop}_{\Theta, \Gamma, \cdot} \circ (\text{id}_{F[\Theta \vdash_c \Gamma]} \otimes \llbracket \Theta; \Gamma \mid \cdot \vdash_\ell \diamond \triangleright \cdot \rrbracket) \quad \text{(semantics of } \bullet : \mathbb{I} \text{)} \\
&= \llbracket \Theta; \Gamma \mid \cdot \vdash_\ell \diamond \triangleright \cdot \rrbracket \circ \text{drop}_{\Theta, \Gamma, \cdot} \quad \text{(Lemma 11.24)} \\
&= \text{id}_{\mathbb{I}} \circ \text{drop}_{\Theta, \Gamma, \cdot} \quad \text{(def. of empty linear substitution)} \\
&= \llbracket \Theta \mid \Gamma; \cdot \vdash_\ell \bullet : \mathbb{I} \rrbracket \quad \text{(semantics of } \bullet : \mathbb{I} \text{)} \\
&= \llbracket \Theta \mid \Gamma; \cdot \vdash_\ell [\diamond]\bullet : \mathbb{I} \rrbracket \quad \text{(syntactic substitution)}
\end{aligned}$$

- $(\Theta \mid \Gamma; \Delta_1, \Delta_2 \vdash_\ell \text{let } \langle \rangle = t_1 \text{ in } t_2 : C)$ :

$$\begin{aligned}
& \llbracket \Theta \mid \Gamma; \Delta_1, \Delta_2 \vdash_\ell \text{let } \langle \rangle = t_1 \text{ in } t_2 : C \rrbracket \circ (\text{id}_{F[\Theta \vdash_c \Gamma]} \otimes \llbracket \hat{\xi}_1, \hat{\xi}_2 \rrbracket) \\
&= \lambda_{[\Theta \vdash_c B]} \circ (\llbracket \Theta \mid \Gamma; \Delta_1 \vdash_\ell t_1 : \mathbb{I} \rrbracket \otimes \llbracket \Theta \mid \Gamma; \Delta_2 \vdash_\ell t_2 : B \rrbracket) \circ \text{split}_{\Theta, \Gamma, \Delta_1, \Delta_2} \circ (\text{id}_{F[\Theta \vdash_c \Gamma]} \otimes \llbracket \hat{\xi}_1, \hat{\xi}_2 \rrbracket) \\
&\quad \text{(semantics of } \text{let } \langle \rangle = t_1 \text{ in } t_2 : B \text{)} \\
&= \lambda_{[\Theta \vdash_c B]} \circ (\llbracket t_1 \rrbracket \otimes \llbracket t_2 \rrbracket) \circ ((\text{id}_{F[\Theta \vdash_c \Gamma]} \otimes \llbracket \hat{\xi}_1 \rrbracket) \otimes (\text{id}_{F[\Theta \vdash_c \Gamma]} \otimes \llbracket \hat{\xi}_2 \rrbracket)) \circ \text{split}_{\Theta, \Gamma, \Delta'_1, \Delta'_2} \quad \text{(Lemma 11.20)} \\
&= \lambda_{[\Theta \vdash_c B]} \circ (\llbracket t_1 \rrbracket \circ (\text{id}_{F[\Theta \vdash_c \Gamma]} \otimes \llbracket \hat{\xi}_1 \rrbracket)) \otimes (\llbracket t_2 \rrbracket \circ (\text{id}_{F[\Theta \vdash_c \Gamma]} \otimes \llbracket \hat{\xi}_2 \rrbracket)) \circ \text{split}_{\Theta, \Gamma, \Delta'_1, \Delta'_2} \\
&\quad \text{(CCC property)} \\
&= \lambda_{[\Theta \vdash_c B]} \circ (\llbracket \Theta \mid \Gamma; \Delta'_1 \vdash_\ell [\hat{\xi}]t_1 : \mathbb{I} \rrbracket \otimes \llbracket \Theta \mid \Gamma; \Delta'_2 \vdash_\ell [\hat{\xi}]t_2 : B \rrbracket) \circ \text{split}_{\Theta, \Gamma, \Delta'_1, \Delta'_2} \quad \text{(IHs)} \\
&= \llbracket \Theta \mid \Gamma; \Delta'_1, \Delta'_2 \vdash_\ell \text{let } \langle \rangle = [\hat{\xi}]t_1 \text{ in } [\hat{\xi}]t_2 : B \rrbracket \quad \text{(semantics of } \text{let } \langle \rangle = [\hat{\xi}]t_1 \text{ in } [\hat{\xi}]t_2 : B \text{)} \\
&= \llbracket \Theta \mid \Gamma; \Delta'_1, \Delta'_2 \vdash_\ell [\hat{\xi}](\text{let } \langle \rangle = t_2 \text{ in } t_2) : B \rrbracket \quad \text{(syntactic substitution)}
\end{aligned}$$

- $(\Theta \mid \Gamma; \Delta_1, \Delta_2 \vdash_\ell (t_1, t_2) : A \otimes B)$ :

$$\begin{aligned}
& \llbracket \Theta \mid \Gamma; \Delta_1, \Delta_2 \vdash_\ell (t_1, t_2) : A \otimes B \rrbracket \circ (\text{id}_{F[\Theta \vdash_c \Gamma]} \otimes \llbracket \hat{\xi}_1, \hat{\xi}_2 \rrbracket) \\
&= (\llbracket \Theta \mid \Gamma; \Delta_1 \vdash_\ell t_1 : A \rrbracket \otimes \llbracket \Theta \mid \Gamma; \Delta_2 \vdash_\ell t_2 : B \rrbracket) \circ \text{split}_{\Theta, \Gamma, \Delta_1, \Delta_2} \circ (\text{id}_{F[\Theta \vdash_c \Gamma]} \otimes \llbracket \hat{\xi}_1, \hat{\xi}_2 \rrbracket) \\
&\quad \text{(semantics of } (t_1, t_2) : A \otimes B \text{)} \\
&= (\llbracket t_1 \rrbracket \otimes \llbracket t_2 \rrbracket) \circ ((\text{id}_{F[\Theta \vdash_c \Gamma]} \otimes \llbracket \hat{\xi}_1 \rrbracket) \otimes (\text{id}_{F[\Theta \vdash_c \Gamma]} \otimes \llbracket \hat{\xi}_2 \rrbracket)) \circ \text{split}_{\Theta, \Gamma, \Delta'_1, \Delta'_2} \quad \text{(Lemma 11.24)} \\
&= ((\llbracket t_1 \rrbracket \circ (\text{id}_{F[\Theta \vdash_c \Gamma]} \otimes \llbracket \hat{\xi}_1 \rrbracket)) \otimes (\llbracket t_2 \rrbracket \circ (\text{id}_{F[\Theta \vdash_c \Gamma]} \otimes \llbracket \hat{\xi}_2 \rrbracket))) \circ \text{split}_{\Theta, \Gamma, \Delta'_1, \Delta'_2} \quad \text{(CCC prop.)} \\
&= (\llbracket \Theta \mid \Gamma; \Delta'_1 \vdash_\ell [\hat{\xi}]t_1 : A \rrbracket \otimes \llbracket \Theta \mid \Gamma; \Delta'_2 \vdash_\ell [\hat{\xi}]t_2 : B \rrbracket) \circ \text{split}_{\Theta, \Gamma, \Delta'_1, \Delta'_2} \quad \text{(IHs)} \\
&= \llbracket \Theta \mid \Gamma; \Delta'_1, \Delta'_2 \vdash_\ell ([\hat{\xi}]t_1, [\hat{\xi}]t_2) : A \otimes B \rrbracket \quad \text{(semantics of } ([\hat{\xi}]t_1, [\hat{\xi}]t_2) : A \otimes B \text{)} \\
&= \llbracket \Theta \mid \Gamma; \Delta'_1, \Delta'_2 \vdash_\ell [\hat{\xi}](t_1, t_2) : A \otimes B \rrbracket \quad \text{(syntactic substitution)}
\end{aligned}$$

- $(\Theta \mid \Gamma; \Delta_1, \Delta_2 \vdash_\ell \text{let } (a, b) = t_1 \text{ in } t_2 : C)$ :

$$\begin{aligned}
& \llbracket \Theta \mid \Gamma; \Delta_1, \Delta_2 \vdash_\ell \text{let } (a, b) = t_1 \text{ in } t_2 : C \rrbracket \circ (\text{id}_{F[\Theta \vdash_c \Gamma]} \otimes \llbracket \hat{\xi}_1, \hat{\xi}_2 \rrbracket) \\
&= \llbracket t_2 \rrbracket \circ \varsigma \circ (\llbracket \Theta \mid \Gamma; \Delta_1 \vdash_\ell t_1 : A \otimes B \rrbracket \otimes \text{id}_{F[\Theta \vdash_c \Gamma] \otimes [\Theta \vdash_\ell \Delta_2]}) \circ \text{split}_{\Theta, \Gamma, \Delta_1, \Delta_2} \circ (\text{id}_{F[\Theta \vdash_c \Gamma]} \otimes \llbracket \hat{\xi}_1, \hat{\xi}_2 \rrbracket) \\
&\quad \text{(semantics of let } (a, b) = t_1 \text{ in } t_2 : C) \\
&= \llbracket t_2 \rrbracket \circ \varsigma \circ (\llbracket \Theta \mid \Gamma; \Delta_1 \vdash_\ell t_1 : A \otimes B \rrbracket \otimes \text{id}) \circ ((\text{id} \otimes \llbracket \hat{\xi}_1 \rrbracket) \otimes (\text{id} \otimes \llbracket \hat{\xi}_2 \rrbracket)) \circ \text{split}_{\Theta, \Gamma, \Delta'_1, \Delta'_2} \\
&\quad \text{(Lemma 11.20)} \\
&= \llbracket t_2 \rrbracket \circ \varsigma \circ ((\llbracket \Theta \mid \Gamma; \Delta_1 \vdash_\ell t_1 : A \otimes B \rrbracket \circ (\text{id}_{F[\Theta \vdash_c \Gamma]} \otimes \llbracket \hat{\xi}_1 \rrbracket)) \otimes (\text{id}_{F[\Theta \vdash_c \Gamma]} \otimes \llbracket \hat{\xi}_2 \rrbracket)) \circ \text{split}_{\Theta, \Gamma, \Delta'_1, \Delta'_2} \\
&\quad \text{(bifunctionality)} \\
&= \llbracket t_2 \rrbracket \circ \varsigma \circ (\llbracket \Theta \mid \Gamma; \Delta'_1 \vdash_\ell [\hat{\xi}]t_1 : A \otimes B \rrbracket \otimes (\text{id}_{F[\Theta \vdash_c \Gamma]} \otimes \llbracket \hat{\xi}_2 \rrbracket)) \circ \text{split}_{\Theta, \Gamma, \Delta'_1, \Delta'_2} \quad \text{(IH on } t_1) \\
&= \llbracket t_2 \rrbracket \circ \varsigma \circ (\text{id}_{[\Theta \vdash_\ell A]} \otimes \text{id}_{[\Theta \vdash_\ell B]} \otimes (\text{id}_{F[\Theta \vdash_c \Gamma]} \otimes \llbracket \hat{\xi}_2 \rrbracket)) \circ ((\llbracket \hat{\xi} \rrbracket t_1) \otimes (\text{id}_{F[\Theta \vdash_c \Gamma]} \otimes \text{id}_{[\Theta \vdash_\ell \Delta'_2]})) \circ \text{split} \\
&\quad \text{(bifunctionality)} \\
&= \llbracket \Theta \mid \Gamma; \Delta_2, a : A, b : B \vdash_\ell t_2 : C \rrbracket \circ (\text{id}_{F[\Theta \vdash_c \Gamma]} \otimes \llbracket \hat{\xi}_2 \rrbracket \otimes \text{id}_{[\Theta \vdash_\ell A]} \otimes \text{id}_{[\Theta \vdash_\ell B]}) \circ \varsigma \circ ((\llbracket \hat{\xi} \rrbracket t_1) \otimes \text{id}) \circ \text{split} \\
&\quad \text{(naturality of } \varsigma \text{ and bifunctionality)} \\
&= \llbracket \Theta \mid \Gamma; \Delta_2, a : A, b : B \vdash_\ell t_2 : C \rrbracket \circ (\text{id}_{F[\Theta \vdash_c \Gamma]} \otimes \llbracket \hat{\xi}_2, a \mapsto a, b \mapsto b \rrbracket) \circ \varsigma \circ ((\llbracket \hat{\xi} \rrbracket t_1) \otimes \text{id}) \circ \text{split} \\
&\quad \text{(def. of linear substitution)} \\
&= \llbracket \Theta \mid \Gamma'; \Delta_2, a : A, b : B \vdash_\ell [\xi]t_2 : C \rrbracket \circ \varsigma \circ ((\llbracket \xi \rrbracket t_1) \otimes \text{id}_{F[\Theta \vdash_c \Gamma'] \otimes [\Theta \vdash_\ell \Delta_2]}) \circ \text{split}_{\Theta, \Gamma', \Delta_1, \Delta_2} \\
&\quad \text{(IH on } t_2) \\
&= \llbracket \Theta \mid \Gamma'; \Delta_1, \Delta_2 \vdash_\ell \text{let } (a, b) = [\xi]t_1 \text{ in } [\xi]t_2 : C \rrbracket \quad \text{(semantics of let } (a, b) = [\xi]t_1 \text{ in } [\xi]t_2 : C) \\
&= \llbracket \Theta \mid \Gamma'; \Delta_1, \Delta_2 \vdash_\ell [\xi](\text{let } (a, b) = t_1 \text{ in } t_2) : C \rrbracket \quad \text{(syntactic substitution)}
\end{aligned}$$

- $(\Theta \mid \Gamma; \Delta \vdash_\ell \text{evt } t : \Diamond A)$ :

$$\begin{aligned}
& \llbracket \Theta \mid \Gamma; \Delta \vdash_\ell \text{evt } t : \Diamond A \rrbracket \circ (\text{id}_{F[\Theta \vdash_c \Gamma]} \otimes \llbracket \hat{\xi} \rrbracket) \\
&= \eta_{[\Theta \vdash_\ell A]} \circ \llbracket \Theta \mid \Gamma; \Delta \vdash_\ell t : A \rrbracket \circ (\text{id}_{F[\Theta \vdash_c \Gamma]} \otimes \llbracket \hat{\xi} \rrbracket) \quad \text{(semantics of evt } t : \Diamond A) \\
&= \eta_{[\Theta \vdash_\ell A]} \circ \llbracket \Theta \mid \Gamma; \Delta' \vdash_\ell [\hat{\xi}]t : A \rrbracket \quad \text{(IH)} \\
&= \llbracket \Theta \mid \Gamma; \Delta' \vdash_\ell \text{evt } ([\hat{\xi}]t) : \Diamond A \rrbracket \quad \text{(semantics of evt } ([\hat{\xi}]t) : \Diamond A) \\
&= \llbracket \Theta \mid \Gamma; \Delta' \vdash_\ell [\hat{\xi}](\text{evt } t) : \Diamond A \rrbracket \quad \text{(syntactic substitution)}
\end{aligned}$$

- $(\Theta \mid \Gamma; \Delta \vdash_\ell \text{let evt } a = t_1 \text{ in } t_2 : \Diamond B)$ :

$$\begin{aligned}
& \llbracket \Theta \mid \Gamma; \Delta \vdash_\ell \text{let evt } a = t_1 \text{ in } t_2 : \Diamond B \rrbracket \circ (\text{id}_{F[\Theta \vdash_c \Gamma]} \otimes \llbracket \hat{\xi} \rrbracket) \\
&= \mu_{[\Theta \vdash_\ell B]} \circ \Diamond \llbracket t_2 \rrbracket \circ \text{st}_{[\Theta \vdash_c \Gamma], [\Theta \vdash_\ell A]}^F \circ (\text{id} \otimes \llbracket t_1 \rrbracket) \circ \varsigma \circ (\text{dup}_{[\Theta \vdash_c \Gamma]} \otimes \text{id}) \circ (\text{id}_{F[\Theta \vdash_c \Gamma]} \otimes \llbracket \hat{\xi} \rrbracket) \\
&\quad \text{(semantics of let evt } a = t_1 \text{ in } t_2 : \Diamond B) \\
&= \mu_{[\Theta \vdash_\ell B]} \circ \Diamond \llbracket t_2 \rrbracket \circ \text{st}_{[\Theta \vdash_c \Gamma], [\Theta \vdash_\ell A]}^F \circ (\text{id} \otimes \llbracket t_1 \rrbracket) \circ (\text{id}_{F[\Theta \vdash_c \Gamma]} \otimes (\text{id}_{F[\Theta \vdash_c \Gamma]} \otimes \llbracket \hat{\xi} \rrbracket)) \circ \varsigma \circ (\text{dup}_{[\Theta \vdash_c \Gamma]} \otimes \text{id}) \\
&\quad \text{(naturality of duplication and } \varsigma) \\
&= \mu_{[\Theta \vdash_\ell B]} \circ \Diamond \llbracket t_2 \rrbracket \circ \text{st}_{[\Theta \vdash_c \Gamma], [\Theta \vdash_\ell A]}^F \circ (\text{id}_{F[\Theta \vdash_c \Gamma]} \otimes (\llbracket t_1 \rrbracket \circ (\text{id}_{F[\Theta \vdash_c \Gamma]} \otimes \llbracket \hat{\xi} \rrbracket))) \circ \varsigma \circ (\text{dup}_{[\Theta \vdash_c \Gamma]} \otimes \text{id}) \\
&\quad \text{(bifunctionality)} \\
&= \mu_{[\Theta \vdash_\ell B]} \circ \Diamond \llbracket t_2 \rrbracket \circ \text{st}_{[\Theta \vdash_c \Gamma], [\Theta \vdash_\ell A]}^F \circ (\text{id}_{F[\Theta \vdash_c \Gamma]} \otimes \llbracket \Theta \mid \Gamma; \Delta' \vdash_\ell [\hat{\xi}]t_1 : \Diamond A \rrbracket) \circ \varsigma \circ (\text{dup}_{[\Theta \vdash_c \Gamma]} \otimes \text{id}) \\
&\quad \text{(IH on } t_1) \\
&= \llbracket \Theta \mid \Gamma; \Delta \vdash_\ell \text{let evt } a = [\xi]t_1 \text{ in } t_2 : \Diamond B \rrbracket \quad \text{(semantics of let evt } a = [\xi]t_1 \text{ in } t_2 : \Diamond B) \\
&= \llbracket \Theta \mid \Gamma; \Delta \vdash_\ell [\hat{\xi}](\text{let evt } a = t_1 \text{ in } t_2) : \Diamond B \rrbracket \quad \text{(syntactic substitution)}
\end{aligned}$$

- $(\Theta \mid \Gamma; \Delta \vdash_\ell t @ \tau : A @ \tau)$ :

$$\begin{aligned}
& \llbracket \Theta \mid \Gamma; \Delta \vdash_\ell t @ \tau : A @ \tau \rrbracket \circ (\text{id}_{F[\Theta \vdash_c \Gamma]} \otimes \llbracket \hat{\xi} \rrbracket) \\
&= \llbracket \Theta \mid \Gamma; \Delta \vdash_\ell t :_\tau A \rrbracket \circ (\text{id}_{F[\Theta \vdash_c \Gamma]} \otimes \llbracket \hat{\xi} \rrbracket) && \text{(semantics of } t @ \tau : A @ \tau) \\
&= \llbracket \Theta \mid \Gamma; \Delta' \vdash_\ell [\hat{\xi}]t :_\tau A \rrbracket && \text{(IH)} \\
&= \llbracket \Theta \mid \Gamma; \Delta' \vdash_\ell ([\hat{\xi}]t) @ \tau : A @ \tau \rrbracket && \text{(semantics of } ([\hat{\xi}]t) @ \tau : A @ \tau) \\
&= \llbracket \Theta \mid \Gamma; \Delta' \vdash_\ell [\hat{\xi}](t @ \tau) : A @ \tau \rrbracket && \text{(syntactic substitution)}
\end{aligned}$$

- $(\Theta \mid \Gamma; \Delta_1, \Delta_2 \vdash_\ell \text{let } a @ \tau = t_1 \text{ in } t_2 : B)$ :

$$\begin{aligned}
& \llbracket \Theta \mid \Gamma; \Delta_1, \Delta_2 \vdash_\ell \text{let } a @ \tau = t_1 \text{ in } t_2 : B \rrbracket \circ (\text{id}_{F[\Theta \vdash_c \Gamma]} \otimes \llbracket \hat{\xi}_1, \hat{\xi}_2 \rrbracket) \\
&= \llbracket \Theta \mid \Gamma; \Delta_2, a :_\tau A \vdash_\ell t_2 : B \rrbracket \circ \varsigma \circ (\llbracket \Theta \mid \Gamma; \Delta_1 \vdash_\ell t_1 : A @ \tau \rrbracket \otimes \text{id}) \circ \text{split} \circ (\text{id}_{F[\Theta \vdash_c \Gamma]} \otimes \llbracket \hat{\xi}_1, \hat{\xi}_2 \rrbracket) \\
& \quad \text{(semantics of } \text{let } a @ \tau = t_1 \text{ in } t_2 : B) \\
&= \llbracket t_2 \rrbracket \circ \varsigma \circ (\llbracket t_1 \rrbracket \otimes \text{id}) \circ ((\text{id}_{F[\Theta \vdash_c \Gamma]} \otimes \llbracket \hat{\xi}_1 \rrbracket) \otimes (\text{id}_{F[\Theta \vdash_c \Gamma]} \otimes \llbracket \hat{\xi}_2 \rrbracket)) \circ \text{split}_{\Theta, \Gamma, \Delta'_1, \Delta'_2} \quad \text{(Lemma 11.24)} \\
&= \llbracket t_2 \rrbracket \circ \varsigma \circ ((\llbracket t_1 \rrbracket \otimes (\text{id}_{F[\Theta \vdash_c \Gamma]} \otimes \llbracket \hat{\xi}_1 \rrbracket)) \otimes (\text{id}_{F[\Theta \vdash_c \Gamma]} \otimes \llbracket \hat{\xi}_2 \rrbracket)) \circ \text{split}_{\Theta, \Gamma, \Delta'_1, \Delta'_2} \quad \text{(bifunctionality)} \\
&= \llbracket t_2 \rrbracket \circ \varsigma \circ (\llbracket \Theta \mid \Gamma; \Delta'_1 \vdash_\ell [\hat{\xi}]t_1 : A @ \tau \rrbracket \otimes (\text{id}_{F[\Theta \vdash_c \Gamma]} \otimes \llbracket \hat{\xi}_2 \rrbracket)) \circ \text{split}_{\Theta, \Gamma, \Delta'_1, \Delta'_2} \quad \text{(IH on } t_1) \\
&= \llbracket t_2 \rrbracket \circ \varsigma \circ (\text{id}_{\triangleright[\tau]}[\Theta \vdash_\ell A]) \otimes (\text{id}_{F[\Theta \vdash_c \Gamma]} \otimes \llbracket \hat{\xi}_2 \rrbracket)) \circ (\llbracket [\hat{\xi}]t_1 \rrbracket \otimes (\text{id}_{F[\Theta \vdash_c \Gamma]} \otimes \text{id}_{[\Theta \vdash_\ell \Delta'_2]})) \circ \text{split} \\
& \quad \text{(bifunctionality)} \\
&= \llbracket t_2 \rrbracket \circ (\text{id}_{F[\Theta \vdash_c \Gamma]} \otimes \llbracket \hat{\xi}_2 \rrbracket \otimes \text{id}_{\triangleright[\tau]}[\Theta \vdash_\ell A]) \circ \varsigma \circ (\llbracket [\hat{\xi}]t_1 \rrbracket \otimes \text{id}_{F[\Theta \vdash_c \Gamma'] \otimes [\Theta \vdash_\ell \Delta'_2]}) \circ \text{split}_{\Theta, \Gamma, \Delta'_1, \Delta'_2} \\
& \quad \text{(naturality of } \varsigma \text{ and bifunctionality)} \\
&= \llbracket t_2 \rrbracket \circ (\text{id}_{F[\Theta \vdash_c \Gamma]} \otimes \llbracket \hat{\xi}_2, a \mapsto a \rrbracket) \circ \varsigma \circ (\llbracket [\hat{\xi}]t_1 \rrbracket \otimes \text{id}_{F[\Theta \vdash_c \Gamma'] \otimes [\Theta \vdash_\ell \Delta'_2]}) \circ \text{split}_{\Theta, \Gamma, \Delta'_1, \Delta'_2} \\
& \quad \text{(def. of linear substitution)} \\
&= \llbracket \Theta \mid \Gamma; \Delta'_2, a :_\tau A \vdash_\ell [\hat{\xi}]t_2 : B \rrbracket \circ \varsigma \circ (\llbracket [\hat{\xi}]t_1 \rrbracket \otimes \text{id}_{F[\Theta \vdash_c \Gamma'] \otimes [\Theta \vdash_\ell \Delta'_2]}) \circ \text{split}_{\Theta, \Gamma, \Delta'_1, \Delta'_2} \quad \text{(IH on } t_2) \\
&= \llbracket \Theta \mid \Gamma; \Delta'_1, \Delta'_2 \vdash_\ell \text{let } a @ \tau = [\hat{\xi}]t_1 \text{ in } [\hat{\xi}]t_2 : B \rrbracket && \text{(semantics of } \text{let } a @ \tau = [\hat{\xi}]t_1 \text{ in } [\hat{\xi}]t_2 : B) \\
&= \llbracket \Theta \mid \Gamma; \Delta'_1, \Delta'_2 \vdash_\ell [\hat{\xi}](\text{let } a @ \tau = t_1 \text{ in } t_2) : B \rrbracket && \text{(syntactic substitution)}
\end{aligned}$$

- $(\Theta \mid \Gamma; \cdot \vdash_\ell \text{runG } e : A)$ :

$$\begin{aligned}
& \llbracket \Theta \mid \Gamma; \cdot \vdash_\ell \text{runG } e : A \rrbracket \circ (\text{id}_{F[\Theta \vdash_c \Gamma]} \otimes \llbracket \hat{\xi} \rrbracket) \\
&= \epsilon_{[\Theta \vdash_\ell A]} \circ F[\llbracket \Theta \mid \Gamma \vdash_c e : \mathbf{G} A \rrbracket] \circ \rho_{F[\Theta \vdash_c \Gamma]} \circ (\text{id}_{F[\Theta \vdash_c \Gamma]} \otimes \llbracket \hat{\xi} \rrbracket) && \text{(semantics of } \text{runG } e : A) \\
&= \epsilon_{[\Theta \vdash_\ell A]} \circ F[\llbracket \Theta \mid \Gamma \vdash_c e : \mathbf{G} A \rrbracket] \circ \text{id}_{F[\Theta \vdash_c \Gamma]} \circ \rho_{F[\Theta \vdash_c \Gamma']} && \text{(naturality of } \rho) \\
&= \epsilon_{[\Theta \vdash_\ell A]} \circ F[\llbracket \Theta \mid \Gamma \vdash_c e : \mathbf{G} A \rrbracket] \circ \rho_{F[\Theta \vdash_c \Gamma']} && \text{(identity)} \\
&= \llbracket \Theta \mid \Gamma; \cdot \vdash_\ell \text{runG } e : A \rrbracket && \text{(semantics of } \text{runG } e : A) \\
&= \llbracket \Theta \mid \Gamma; \cdot \vdash_\ell [\diamond](\text{runG } e) : A \rrbracket && \text{(syntactic substitution)}
\end{aligned}$$

- $(\Theta \mid \Gamma; \cdot \vdash_\ell \mathbf{F} e : \mathbf{F} X)$ :

$$\begin{aligned}
& \llbracket \Theta \mid \Gamma; \cdot \vdash_\ell \mathbf{F} e : \mathbf{F} X \rrbracket \circ (F[\llbracket \hat{\xi} \rrbracket] \otimes \text{id}_{[\Theta \vdash_\ell \Delta]}) \\
&= F[\llbracket \Theta \mid \Gamma \vdash_c e : X \rrbracket] \circ \rho_{F[\Theta \vdash_c \Gamma]} \circ (\text{id}_{F[\Theta \vdash_c \Gamma]} \otimes \llbracket \hat{\xi} \rrbracket) && \text{(semantics of } \mathbf{F} e : \mathbf{F} X) \\
&= F[\llbracket \Theta \mid \Gamma \vdash_c e : X \rrbracket] \circ \text{id}_{F[\Theta \vdash_c \Gamma]} \circ \rho_{F[\Theta \vdash_c \Gamma']} && \text{(naturality of } \rho) \\
&= F[\llbracket \Theta \mid \Gamma \vdash_c e : X \rrbracket] \circ \rho_{F[\Theta \vdash_c \Gamma']} && \text{(identity)} \\
&= \llbracket \Theta \mid \Gamma'; \cdot \vdash_\ell \mathbf{F} e : \mathbf{F} X \rrbracket && \text{(semantics of } \mathbf{F} e : \mathbf{F} X) \\
&= \llbracket \Theta \mid \Gamma'; \cdot \vdash_\ell [\diamond]\mathbf{F} e : \mathbf{F} X \rrbracket && \text{(syntactic substitution)}
\end{aligned}$$



- $(\Theta \mid \Gamma; \Delta_1, \Delta_2 \vdash_\ell \text{let } F \ x = t_1 \text{ in } t_2 : B):$

$$\begin{aligned}
& \llbracket \Theta \mid \Gamma; \Delta_1, \Delta_2 \vdash_\ell \text{let } a @ \tau = t_1 \text{ in } t_2 : B \rrbracket \circ (\text{id}_{F[\Theta \vdash_c \Gamma]} \otimes \llbracket \hat{\xi}_1, \hat{\xi}_2 \rrbracket) \\
= & \llbracket \Theta \mid \Gamma, x : X; \Delta_2 \vdash_\ell t_2 : B \rrbracket \circ (\mathbf{m}_{[\Theta \vdash_c \Gamma], [\Theta \vdash_c X]} \otimes \text{id}_{[\Theta \vdash_\ell \Delta_2]}) \circ \varsigma \\
& \circ (\llbracket \Theta \mid \Gamma; \Delta_1 \vdash_\ell t_1 : F \ X \rrbracket \otimes \text{id}_{F[\Theta \vdash_c \Gamma] \otimes [\Theta \vdash_\ell \Delta_2]}) \circ \text{split}_{\Theta, \Gamma, \Delta_1, \Delta_2} \circ (\text{id}_{F[\Theta \vdash_c \Gamma]} \otimes \llbracket \hat{\xi}_1, \hat{\xi}_2 \rrbracket) \\
& \quad \text{(semantics of let } F \ x = t_1 \text{ in } t_2 : B) \\
= & \llbracket \Theta \mid \Gamma, x : X; \Delta_2 \vdash_\ell t_2 : B \rrbracket \circ (\mathbf{m}_{[\Theta \vdash_c \Gamma], [\Theta \vdash_c X]} \otimes \text{id}_{[\Theta \vdash_\ell \Delta_2]}) \circ \varsigma \\
& \circ (\llbracket \Theta \mid \Gamma; \Delta_1 \vdash_\ell t_1 : F \ X \rrbracket \otimes \text{id}) \circ ((\text{id}_{F[\Theta \vdash_c \Gamma]} \otimes \llbracket \hat{\xi}_1 \rrbracket) \otimes (\text{id}_{F[\Theta \vdash_c \Gamma]} \otimes \llbracket \hat{\xi}_2 \rrbracket)) \circ \text{split}_{\Theta, \Gamma, \Delta'_1, \Delta'_2} \\
& \quad \text{(Lemma 11.24)} \\
= & \llbracket \Theta \mid \Gamma, x : X; \Delta_2 \vdash_\ell t_2 : B \rrbracket \circ (\mathbf{m}_{[\Theta \vdash_c \Gamma], [\Theta \vdash_c X]} \otimes \text{id}_{[\Theta \vdash_\ell \Delta_2]}) \circ \varsigma \\
& \circ ((\llbracket t_1 \rrbracket \circ (\text{id}_{F[\Theta \vdash_c \Gamma]} \otimes \llbracket \hat{\xi}_1 \rrbracket)) \otimes (\text{id}_{F[\Theta \vdash_c \Gamma]} \otimes \llbracket \hat{\xi}_2 \rrbracket)) \circ \text{split}_{\Theta, \Gamma, \Delta'_1, \Delta'_2} \quad \text{(bifunctionality)} \\
= & \llbracket \Theta \mid \Gamma, x : X; \Delta_2 \vdash_\ell t_2 : B \rrbracket \circ (\mathbf{m}_{[\Theta \vdash_c \Gamma], [\Theta \vdash_c X]} \otimes \text{id}_{[\Theta \vdash_\ell \Delta_2]}) \circ \varsigma \\
& \circ (\llbracket \Theta \mid \Gamma; \Delta'_1 \vdash_\ell [\hat{\xi}]t_1 : F \ X \rrbracket \otimes (\text{id}_{F[\Theta \vdash_c \Gamma]} \otimes \llbracket \hat{\xi}_2 \rrbracket)) \circ \text{split}_{\Theta, \Gamma, \Delta'_1, \Delta'_2} \quad \text{(IH on } t_1) \\
= & \llbracket \Theta \mid \Gamma, x : X; \Delta_2 \vdash_\ell t_2 : B \rrbracket \circ (\mathbf{m}_{[\Theta \vdash_c \Gamma], [\Theta \vdash_c X]} \otimes \text{id}_{[\Theta \vdash_\ell \Delta_2]}) \circ \varsigma \\
& \circ (\text{id}_{F[\Theta \vdash_c X]} \otimes (\text{id}_{F[\Theta \vdash_c \Gamma]} \otimes \llbracket \hat{\xi}_2 \rrbracket)) \circ (\llbracket [\hat{\xi}]t_1 \rrbracket \otimes (\text{id}_{F[\Theta \vdash_c \Gamma']} \otimes \text{id}_{[\Theta \vdash_\ell \Delta_2]})) \circ \text{split}_{\Theta, \Gamma, \Delta'_1, \Delta'_2} \\
& \quad \text{(bifunctionality)} \\
= & \llbracket \Theta \mid \Gamma, x : X; \Delta_2 \vdash_\ell t_2 : B \rrbracket \circ (\mathbf{m}_{[\Theta \vdash_c \Gamma], [\Theta \vdash_c X]} \otimes \text{id}_{[\Theta \vdash_\ell \Delta_2]}) \circ (F\text{id}_{[\Theta \vdash_c \Gamma]} \xi \otimes F\text{id}_{[\Theta \vdash_c X]}) \otimes \llbracket \hat{\xi}_2 \rrbracket \\
& \circ \varsigma \circ (\llbracket [\hat{\xi}]t_1 \rrbracket \otimes (\text{id}_{F[\Theta \vdash_c \Gamma] \otimes [\Theta \vdash_\ell \Delta'_2]})) \circ \text{split}_{\Theta, \Gamma, \Delta'_1, \Delta'_2} \quad \text{(naturality of } \varsigma \text{ and functoriality)} \\
= & \llbracket \Theta \mid \Gamma, x : X; \Delta_2 \vdash_\ell t_2 : B \rrbracket \circ F(\text{id}_{[\Theta \vdash_c \Gamma]} \times \text{id}_{[\Theta \vdash_c X]}) \otimes \llbracket \hat{\xi}_2 \rrbracket \circ (\mathbf{m}_{[\Theta \vdash_c \Gamma], [\Theta \vdash_c X]} \otimes \text{id}_{[\Theta \vdash_\ell \Delta'_2]}) \\
& \circ \varsigma \circ (\llbracket [\hat{\xi}]t_1 \rrbracket \otimes (\text{id}_{F[\Theta \vdash_c \Gamma] \otimes [\Theta \vdash_\ell \Delta'_2]})) \circ \text{split}_{\Theta, \Gamma, \Delta'_1, \Delta'_2} \quad \text{(naturality of } \mathbf{m}) \\
= & \llbracket \Theta \mid \Gamma, x : X; \Delta_2 \vdash_\ell t_2 : B \rrbracket \circ \text{id}_{F([\Theta \vdash_c \Gamma] \times [\Theta \vdash_c X])} \otimes \llbracket \hat{\xi}_2 \rrbracket \circ (\mathbf{m}_{[\Theta \vdash_c \Gamma], [\Theta \vdash_c X]} \otimes \text{id}_{[\Theta \vdash_\ell \Delta'_2]}) \\
& \circ \varsigma \circ (\llbracket [\hat{\xi}]t_1 \rrbracket \otimes (\text{id}_{F[\Theta \vdash_c \Gamma] \otimes [\Theta \vdash_\ell \Delta'_2]})) \circ \text{split}_{\Theta, \Gamma, \Delta'_1, \Delta'_2} \quad \text{(bifunctionality and functoriality)} \\
= & \llbracket \Theta \mid \Gamma, x : X; \Delta'_2 \vdash_\ell [\hat{\xi}]t_2 : B \rrbracket \circ (\mathbf{m}_{[\Theta \vdash_c \Gamma, x : X]} \otimes \text{id}_{[\Theta \vdash_\ell \Delta'_2]}) \circ \varsigma \\
& \circ (\llbracket \Theta \mid \Gamma; \Delta'_1 \vdash_\ell [\hat{\xi}]t_1 : F \ X \rrbracket \otimes \text{id}_{F[\Theta \vdash_c \Gamma] \otimes [\Theta \vdash_\ell \Delta_2]}) \circ \text{split}_{\Theta, \Gamma, \Delta'_1, \Delta'_2} \quad \text{(IH on } t_2) \\
= & \llbracket \Theta \mid \Gamma; \Delta'_1, \Delta'_2 \vdash_\ell \text{let } F \ x = [\hat{\xi}]t_1 \text{ in } [\hat{\xi}]t_2 : B \rrbracket \quad \text{(semantics of let } F \ x = [\xi]t_1 \text{ in } [\xi]t_2 : B) \\
= & \llbracket \Theta \mid \Gamma; \Delta'_1, \Delta'_2 \vdash_\ell [\hat{\xi}](\text{let } F \ x = t_1 \text{ in } t_2) : B \rrbracket \quad \text{(syntactic substitution)}
\end{aligned}$$

- $(\Theta \mid \Gamma; \Delta \vdash_\ell \Lambda i : \sigma. t : \forall i : \sigma. A):$

$$\begin{aligned}
& \llbracket \Theta \mid \Gamma; \Delta \vdash_\ell \Lambda i : \sigma. t : \forall i : \sigma. A \rrbracket \circ (\text{id}_{F[\Theta \vdash_c \Gamma]} \otimes \llbracket \hat{\xi} \rrbracket) \\
= & \phi_{F[\Theta \vdash_c \Gamma] \otimes [\Theta \vdash_\ell \Delta], [\Theta, i : \sigma \vdash_\ell A]} \left( \llbracket \Theta, i : \sigma \mid \Gamma; \Delta \vdash_\ell t : A \rrbracket \circ \mathbf{m}_{F[\Theta \vdash_c \Gamma], [\Theta \vdash_\ell \Delta]}^{-1} \right) \circ (\text{id}_{F[\Theta \vdash_c \Gamma]} \otimes \llbracket \hat{\xi} \rrbracket) \\
& \quad \text{(semantics of } \Lambda i : \sigma. t : \forall i : \sigma. A) \\
= & \phi_{F[\Theta \vdash_c \Gamma'] \otimes [\Theta \vdash_\ell \Delta], [\Theta, i : \sigma \vdash_\ell A]} \left( \llbracket \Theta, i : \sigma \mid \Gamma; \Delta \vdash_\ell t : A \rrbracket \circ \mathbf{m}_{F[\Theta \vdash_c \Gamma], [\Theta \vdash_\ell \Delta]}^{-1} \circ \hat{\mathbf{w}}_{k_{[\sigma]}}(\text{id}_{F[\Theta \vdash_c \Gamma]} \otimes \llbracket \hat{\xi} \rrbracket) \right) \\
& \quad \text{(naturality of } \phi) \\
= & \phi \left( \llbracket \Theta, i : \sigma \mid \Gamma; \Delta \vdash_\ell t : A \rrbracket \circ \hat{\mathbf{w}}_{k_{[\sigma]}}(\text{id}_{F[\Theta \vdash_c \Gamma]}) \otimes \hat{\mathbf{w}}_{k_{[\sigma]}}(\llbracket \hat{\xi} \rrbracket) \circ \mathbf{m}_{F[\Theta \vdash_c \Gamma], [\Theta \vdash_\ell \Delta']}^{-1} \right) \\
& \quad \text{(naturality of } \mathbf{m}^{-1}) \\
= & \phi \left( \llbracket \Theta, i : \sigma \mid \Gamma; \Delta \vdash_\ell t : A \rrbracket \circ \text{id}_{F[\Theta, i : \sigma \vdash_c \Gamma]} \otimes \hat{\mathbf{w}}_{k_{[\sigma]}}(\llbracket \Theta; \Gamma \mid \Delta' \vdash_\ell \hat{\xi} \triangleright \Delta \rrbracket) \circ \mathbf{m}_{F[\Theta \vdash_c \Gamma], [\Theta \vdash_\ell \Delta']}^{-1} \right) \\
& \quad \text{(functoriality and LNL property)}
\end{aligned}$$

$$\begin{aligned}
&= \phi \left( \llbracket \Theta, i : \sigma \mid \Gamma; \Delta \vdash_\ell t : A \rrbracket \circ \text{id}_{F[\llbracket \Theta, i : \sigma \vdash_c \Gamma \rrbracket]} \otimes \llbracket \Theta, i : \sigma; \Gamma \mid \Delta' \vdash_\ell \hat{\xi} \triangleright \Delta \rrbracket \circ \mathbf{m}_{F[\llbracket \Theta \vdash_c \Gamma \rrbracket], [\llbracket \Theta \vdash_\ell \Delta' \rrbracket]}^{-1} \right) \\
&\quad \text{(soundness of index weakening)} \\
&= \phi_{F[\llbracket \Theta \vdash_c \Gamma' \rrbracket] \otimes [\llbracket \Theta \vdash_\ell \Delta \rrbracket], [\llbracket \Theta, i : \sigma \vdash_\ell A \rrbracket]} \left( \llbracket \Theta, i : \sigma \mid \Gamma; \Delta' \vdash_\ell [\hat{\xi}]t : A \rrbracket \circ \mathbf{m}_{F[\llbracket \Theta \vdash_c \Gamma \rrbracket], [\llbracket \Theta \vdash_\ell \Delta' \rrbracket]}^{-1} \right) \quad \text{(IH)} \\
&= \llbracket \Theta \mid \Gamma'; \Delta \vdash_\ell \Lambda i : \sigma. [\xi]t : \forall i : \sigma. A \rrbracket \quad \text{(semantics of } \Lambda i : \sigma. [\xi]t : \forall i : \sigma. A \text{)} \\
&= \llbracket \Theta \mid \Gamma'; \Delta \vdash_\ell [\xi](\Lambda i : \sigma. t) : \forall i : \sigma. A \rrbracket \quad \text{(syntactic substitution)}
\end{aligned}$$

- $(\Theta \mid \Gamma; \Delta \vdash_\ell t_s : \{s/i\}A)$ :

$$\begin{aligned}
&\llbracket \Theta \mid \Gamma; \Delta \vdash_\ell t_s : \{s/i\}A \rrbracket \circ (\text{id}_{F[\llbracket \Theta \vdash_c \Gamma \rrbracket]} \otimes \llbracket \hat{\xi} \rrbracket) \\
&= \langle \text{id}_{[\Theta]}, \llbracket \Theta \vdash_s s : \sigma \rrbracket \rangle^+ (\epsilon_{[\llbracket \Theta, i : \sigma \vdash_\ell A \rrbracket]}) \circ \llbracket \Theta \mid \Gamma; \Delta \vdash_\ell t : \forall i : \sigma. A \rrbracket \circ (\text{id}_{F[\llbracket \Theta \vdash_c \Gamma \rrbracket]} \otimes \llbracket \hat{\xi} \rrbracket) \\
&\quad \text{(semantics of } t_s : \{s/i\}A \text{)} \\
&= \langle \text{id}_{[\Theta]}, \llbracket \Theta \vdash_s s : \sigma \rrbracket \rangle^+ (\epsilon_{[\llbracket \Theta, i : \sigma \vdash_\ell A \rrbracket]}) \circ \llbracket \Theta \mid \Gamma; \Delta' \vdash_\ell [\hat{\xi}]t : \forall i : \sigma. A \rrbracket \quad \text{(IH)} \\
&= \llbracket \Theta \mid \Gamma; \Delta' \vdash_\ell ([\hat{\xi}]t)_s : \{s/i\}A \rrbracket \quad \text{(semantics of } ([\hat{\xi}]t)_s : \{s/i\}A \text{)} \\
&= \llbracket \Theta \mid \Gamma; \Delta' \vdash_\ell [\hat{\xi}](t_s) : \{s/i\}A \rrbracket \quad \text{(syntactic substitution)}
\end{aligned}$$

- $(\Theta \mid \Gamma; \Delta \vdash_\ell \{s, t\} : \exists i : \sigma. A)$ :

$$\begin{aligned}
&\llbracket \Theta \mid \Gamma; \Delta \vdash_\ell \{s, t\} : \exists i : \sigma. A \rrbracket \circ (\text{id}_{F[\llbracket \Theta \vdash_c \Gamma \rrbracket]} \otimes \llbracket \hat{\xi} \rrbracket) \\
&= \langle \text{id}_{[\Theta]}, \llbracket \Theta \vdash_s s : \sigma \rrbracket \rangle^+ (\eta_{[\llbracket \Theta, i : \sigma \vdash_\ell A \rrbracket]}) \circ \llbracket \Theta \mid \Gamma; \Delta \vdash_\ell t : \{s/i\}A \rrbracket \circ (\text{id}_{F[\llbracket \Theta \vdash_c \Gamma \rrbracket]} \otimes \llbracket \hat{\xi} \rrbracket) \\
&\quad \text{(semantics of } t_s : \{s/i\}A \text{)} \\
&= \langle \text{id}_{[\Theta]}, \llbracket \Theta \vdash_s s : \sigma \rrbracket \rangle^+ (\epsilon_{[\llbracket \Theta, i : \sigma \vdash_\ell A \rrbracket]}) \circ \llbracket \Theta \mid \Gamma; \Delta' \vdash_\ell [\hat{\xi}]t : \{s/i\}A \rrbracket \quad \text{(IH)} \\
&= \llbracket \Theta \mid \Gamma; \Delta' \vdash_\ell \{s, [\hat{\xi}]t\} : \exists i : \sigma. A \rrbracket \quad \text{(semantics of } \{s, [\hat{\xi}]t\} : \exists i : \sigma. A \text{)} \\
&= \llbracket \Theta \mid \Gamma; \Delta' \vdash_\ell [\hat{\xi}]\{s, t\} : \exists i : \sigma. A \rrbracket \quad \text{(syntactic substitution)}
\end{aligned}$$

- $(\Theta \mid \Gamma; \Delta_1, \Delta_2 \vdash_\ell \text{let } \{s, a\} = t_1 \text{ in } t_2 : B)$ :

$$\begin{aligned}
&\llbracket \Theta \mid \Gamma; \Delta_1, \Delta_2 \vdash_\ell \text{let } \{s, a\} = t_1 \text{ in } t_2 : B \rrbracket \circ (\text{id}_{F[\llbracket \Theta \vdash_c \Gamma \rrbracket]} \otimes \llbracket \hat{\xi}_1, \hat{\xi}_2 \rrbracket) \\
&= \psi_{F[\llbracket \Theta, s : \sigma \vdash_c \Gamma \rrbracket] \otimes [\llbracket \Theta, s : \sigma \vdash_\ell \Delta_2, a : \{s/i\}A \rrbracket], [\llbracket \Theta \vdash_\ell B \rrbracket]} (\llbracket \Theta, s : \sigma \mid \Gamma; \Delta_2, a : \{s/i\}A \vdash_\ell t_2 : B \rrbracket) \circ \hat{\exists}_{[\sigma]}(\varsigma) \\
&\quad \circ \hat{\exists}_{[\sigma]}(\text{id} \otimes \mathbf{m}^{-1}) \circ (\llbracket \Theta \mid \Gamma; \Delta_1 \vdash_\ell t_1 : \exists i : \sigma. A \rrbracket \circ \text{id}) \circ \text{split}_{\Theta, \Gamma, \Delta_1, \Delta_2} \circ (\text{id}_{F[\llbracket \Theta \vdash_c \Gamma \rrbracket]} \otimes \llbracket \hat{\xi}_1, \hat{\xi}_2 \rrbracket) \\
&\quad \text{(semantics of let } \{s, a\} = t_1 \text{ in } t_2 : B \text{)} \\
&= \psi_{F[\llbracket \Theta, s : \sigma \vdash_c \Gamma \rrbracket] \otimes [\llbracket \Theta, s : \sigma \vdash_\ell \Delta_2, a : \{s/i\}A \rrbracket], [\llbracket \Theta \vdash_\ell B \rrbracket]} (\llbracket \Theta, s : \sigma \mid \Gamma; \Delta_2, a : \{s/i\}A \vdash_\ell t_2 : B \rrbracket) \circ \hat{\exists}_{[\sigma]}(\varsigma) \\
&\quad \circ \hat{\exists}_{[\sigma]}(\text{id} \otimes \mathbf{m}^{-1}) \circ ((\llbracket \Theta \mid \Gamma; \Delta_1 \vdash_\ell t_1 : \exists i : \sigma. A \rrbracket \circ (\text{id}_{F[\llbracket \Theta \vdash_c \Gamma \rrbracket]} \otimes \llbracket \hat{\xi}_1 \rrbracket)) \otimes (\text{id}_{F[\llbracket \Theta \vdash_c \Gamma \rrbracket]} \otimes \llbracket \hat{\xi}_2 \rrbracket)) \circ \text{split} \\
&\quad \text{(Lemma 11.24 and bifunctionality)} \\
&= \psi_{F[\llbracket \Theta, s : \sigma \vdash_c \Gamma \rrbracket] \otimes [\llbracket \Theta, s : \sigma \vdash_\ell \Delta_2, a : \{s/i\}A \rrbracket], [\llbracket \Theta \vdash_\ell B \rrbracket]} (\llbracket \Theta, s : \sigma \mid \Gamma; \Delta_2, a : \{s/i\}A \vdash_\ell t_2 : B \rrbracket) \circ \varsigma \\
&\quad \circ \hat{\exists}_{[\sigma]} \left( \text{id} \otimes \mathbf{m}_{F[\llbracket \Theta \vdash_c \Gamma \rrbracket], [\llbracket \Theta \vdash_\ell \Delta_2 \rrbracket]}^{-1} \right) \circ (\llbracket \Theta \mid \Gamma; \Delta_1' \vdash_\ell [\hat{\xi}]t_1 : \exists i : \sigma. A \rrbracket \otimes (\text{id}_{F[\llbracket \Theta \vdash_c \Gamma \rrbracket]} \otimes \llbracket \hat{\xi}_2 \rrbracket)) \circ \text{split} \\
&\quad \text{(IH on } t_1 \text{)} \\
&= \psi_{F[\llbracket \Theta, s : \sigma \vdash_c \Gamma \rrbracket] \otimes [\llbracket \Theta, s : \sigma \vdash_\ell \Delta_2, a : \{s/i\}A \rrbracket], [\llbracket \Theta \vdash_\ell B \rrbracket]} (\llbracket \Theta, s : \sigma \mid \Gamma; \Delta_2, a : \{s/i\}A \vdash_\ell t_2 : B \rrbracket) \circ \hat{\exists}_{[\sigma]}(\varsigma) \\
&\quad \circ \hat{\exists}_{[\sigma]} \left( \text{id} \otimes \mathbf{m}_{F[\llbracket \Theta \vdash_c \Gamma \rrbracket], [\llbracket \Theta \vdash_\ell \Delta_2 \rrbracket]}^{-1} \right) \circ (\hat{\exists}_{[\sigma]}(\text{id}_{[\Theta, i : \sigma \vdash_\ell A]}) \otimes (\text{id}_{F[\llbracket \Theta \vdash_c \Gamma \rrbracket]} \otimes \llbracket \hat{\xi}_2 \rrbracket)) \circ (([\hat{\xi}]t_1) \otimes \text{id}) \circ \text{split} \\
&\quad \text{(bifunctionality)} \\
&= \psi_{F[\llbracket \Theta, s : \sigma \vdash_c \Gamma \rrbracket] \otimes [\llbracket \Theta, s : \sigma \vdash_\ell \Delta_2, a : \{s/i\}A \rrbracket], [\llbracket \Theta \vdash_\ell B \rrbracket]} (\llbracket \Theta, s : \sigma \mid \Gamma; \Delta_2, a : \{s/i\}A \vdash_\ell t_2 : B \rrbracket) \circ \hat{\exists}_{[\sigma]}(\varsigma)
\end{aligned}$$

$$\begin{aligned}
& \circ \hat{\Xi}_{[\sigma]} \left( \text{id} \otimes \mathbf{m}_{F[\Theta \vdash_c \Gamma], [\Theta \vdash_\ell \Delta_2]}^{-1} \right) \circ (\hat{\Xi}_{[\sigma]}(\text{id}_{[\Theta, i : \sigma \vdash_\ell A]} \otimes \hat{\mathbf{w}}_{k_{[\sigma]}}(\text{id}_{F[\Theta \vdash_c \Gamma]} \otimes [\hat{\xi}_2]))) \circ ([\hat{\xi}]t_1 \otimes \text{id}) \circ \text{split} \\
& \quad \text{(Frobenius reciprocity)} \\
= & \psi_F[\Theta, s : \sigma \vdash_c \Gamma] \otimes [\Theta, s : \sigma \vdash_\ell \Delta_2, a : \{s/i\}A], [\Theta \vdash_\ell B] ([\Theta, s : \sigma \mid \Gamma; \Delta_2, a : \{s/i\}A \vdash_\ell t_2 : B]) \circ \hat{\Xi}_{[\sigma]}(\varsigma) \\
& \circ \hat{\Xi}_{[\sigma]} \left( \text{id}_{[\Theta, i : \sigma \vdash_\ell A]} \otimes (\mathbf{m}_{F[\Theta \vdash_c \Gamma], [\Theta \vdash_\ell \Delta_2]}^{-1} \otimes \hat{\mathbf{w}}_{k_{[\sigma]}}(\text{id}_{F[\Theta \vdash_c \Gamma]} \otimes [\hat{\xi}_2])) \right) \circ ([\hat{\xi}]t_1 \otimes \text{id}) \circ \text{split} \\
& \quad \text{(functoriality and bifunctoriality)} \\
= & \psi_F[\Theta, s : \sigma \vdash_c \Gamma] \otimes [\Theta, s : \sigma \vdash_\ell \Delta_2, a : \{s/i\}A], [\Theta \vdash_\ell B] ([\Theta, s : \sigma \mid \Gamma; \Delta_2, a : \{s/i\}A \vdash_\ell t_2 : B]) \circ \hat{\Xi}_{[\sigma]}(\varsigma) \\
& \circ \hat{\Xi}_{[\sigma]} \left( \text{id}_{[\Theta, i : \sigma \vdash_\ell A]} \otimes \left( (\hat{\mathbf{w}}_{k_{[\sigma]}} \text{id}_{F[\Theta \vdash_c \Gamma]} \otimes \hat{\mathbf{w}}_{k_{[\sigma]}}[\hat{\xi}_2]) \circ \mathbf{m}_{F[\Theta \vdash_c \Gamma], [\Theta \vdash_\ell \Delta'_2]}^{-1} \right) \right) \circ ([\hat{\xi}]t_1 \otimes \text{id}) \circ \text{split} \\
& \quad \text{(naturality of } \mathbf{m}^{-1} \text{)} \\
= & \psi_F[\Theta, s : \sigma \vdash_c \Gamma] \otimes [\Theta, s : \sigma \vdash_\ell \Delta_2, a : \{s/i\}A], [\Theta \vdash_\ell B] ([\Theta, s : \sigma \mid \Gamma; \Delta_2, a : \{s/i\}A \vdash_\ell t_2 : B]) \circ \hat{\Xi}_{[\sigma]}(\varsigma) \\
& \circ \hat{\Xi}_{[\sigma]} \left( (\text{id}_{[\Theta, i : \sigma \vdash_\ell A]} \otimes (\text{id}_{F[\Theta, i : \sigma \vdash_c \Gamma]} \otimes \hat{\mathbf{w}}_{k_{[\sigma]}}[\hat{\xi}_2])) \circ (\text{id}_{[\Theta, i : \sigma \vdash_\ell A]} \otimes \mathbf{m}^{-1}) \right) \circ ([\hat{\xi}]t_1 \otimes \text{id}) \circ \text{split} \\
& \quad \text{(bifunctoriality)} \\
= & \psi_F[\Theta, s : \sigma \vdash_c \Gamma] \otimes [\Theta, s : \sigma \vdash_\ell \Delta_2, a : \{s/i\}A], [\Theta \vdash_\ell B] ([\Theta, s : \sigma \mid \Gamma; \Delta_2, a : \{s/i\}A \vdash_\ell t_2 : B]) \\
& \circ \hat{\Xi}_{[\sigma]} \left( \varsigma \circ (\text{id}_{[\Theta, i : \sigma \vdash_\ell A]} \otimes (\text{id}_{F[\Theta, i : \sigma \vdash_c \Gamma]} \otimes \hat{\mathbf{w}}_{k_{[\sigma]}}[\hat{\xi}_2])) \right) \\
& \circ \hat{\Xi}_{[\sigma]} (\text{id}_{[\Theta, i : \sigma \vdash_\ell A]} \otimes \mathbf{m}_{F[\Theta \vdash_c \Gamma], [\Theta \vdash_\ell \Delta'_2]}^{-1}) \circ ([\hat{\xi}]t_1 \otimes \text{id}) \circ \text{split} \quad \text{(functoriality)} \\
= & \psi_F[\Theta, s : \sigma \vdash_c \Gamma] \otimes [\Theta, s : \sigma \vdash_\ell \Delta_2, a : \{s/i\}A], [\Theta \vdash_\ell B] ([\Theta, s : \sigma \mid \Gamma; \Delta_2, a : \{s/i\}A \vdash_\ell t_2 : B]) \\
& \circ \hat{\Xi}_{[\sigma]} \left( (\text{id}_{F[\Theta, i : \sigma \vdash_c \Gamma]} \otimes \hat{\mathbf{w}}_{k_{[\sigma]}}[\Theta; \Gamma \mid \Delta'_2 \vdash_\ell \hat{\xi}_2 \triangleright \Delta_2] \otimes \text{id}_{[\Theta, i : \sigma \vdash_\ell A]}) \circ \varsigma \right) \\
& \circ \hat{\Xi}_{[\sigma]} (\text{id}_{[\Theta, i : \sigma \vdash_\ell A]} \otimes \mathbf{m}_{F[\Theta \vdash_c \Gamma], [\Theta \vdash_\ell \Delta'_2]}^{-1}) \circ ([\hat{\xi}]t_1 \otimes \text{id}) \circ \text{split} \quad \text{(naturality of } \varsigma \text{)} \\
= & \psi_F[\Theta, s : \sigma \vdash_c \Gamma] \otimes [\Theta, s : \sigma \vdash_\ell \Delta_2, a : \{s/i\}A], [\Theta \vdash_\ell B] ([\Theta, s : \sigma \mid \Gamma; \Delta_2, a : \{s/i\}A \vdash_\ell t_2 : B]) \\
& \circ \hat{\Xi}_{[\sigma]} \left( (\text{id}_{F[\Theta, i : \sigma \vdash_c \Gamma]} \otimes [\Theta, s : \sigma; \Gamma \mid \Delta'_2 \vdash_\ell \hat{\xi}_2 \triangleright \Delta_2] \otimes \text{id}_{[\Theta, i : \sigma \vdash_\ell A]}) \circ \varsigma \right) \circ \hat{\Xi}_{[\sigma]}(\varsigma) \\
& \circ \hat{\Xi}_{[\sigma]} (\text{id}_{[\Theta, i : \sigma \vdash_\ell A]} \otimes \mathbf{m}_{F[\Theta \vdash_c \Gamma], [\Theta \vdash_\ell \Delta_2]}^{-1}) \circ ([\hat{\xi}]t_1 \otimes \text{id}) \circ \text{split} \\
& \quad \text{(soundness of index substitution)} \\
= & \psi_F[\Theta, s : \sigma \vdash_c \Gamma] \otimes [\Theta, s : \sigma \vdash_\ell \Delta_2, a : \{s/i\}A], [\Theta \vdash_\ell B] ([\Theta, s : \sigma \mid \Gamma; \Delta_2, a : \{s/i\}A \vdash_\ell t_2 : B]) \\
& \circ \hat{\Xi}_{[\sigma]} (\text{id}_{F[\Theta, i : \sigma \vdash_c \Gamma]} \otimes [\Theta, s : \sigma; \Gamma \mid \Delta'_2, a : \{s/i\}A \vdash_\ell \hat{\xi}_2, a \mapsto a \triangleright \Delta_2, a : \{s/i\}A]) \\
& \circ \hat{\Xi}_{[\sigma]} \left( \varsigma \circ (\text{id} \otimes \mathbf{m}_{F[\Theta \vdash_c \Gamma'], [\Theta \vdash_\ell \Delta_2]}^{-1}) \right) \circ ([\Theta \mid \Gamma'; \Delta_1 \vdash_\ell [\hat{\xi}]t_1 : \exists i : \sigma. A] \otimes^{\text{eq}} \text{id}) \circ \text{split}_{\Theta, \Gamma', \Delta_1, \Delta_2} \\
& \quad \text{(definition of linear substitution (using } [\Theta, i : \sigma \vdash_\ell A] = [\Theta, s : \sigma \vdash_\ell \{s/i\}A] \text{))} \\
= & \psi_F[\Theta, s : \sigma \vdash_c \Gamma] \otimes [\Theta, s : \sigma \vdash_\ell \Delta'_2, a : \{s/i\}A], [\Theta \vdash_\ell B] ([\Theta, s : \sigma \mid \Gamma; \Delta_2, a : \{s/i\}A \vdash_\ell t_2 : B]) \\
& \circ (\text{id}_{F[\Theta, s : \sigma \vdash_c \Gamma]} \otimes [\Theta, s : \sigma; \Gamma \mid \Delta'_2, a : \{s/i\}A \vdash_\ell \hat{\xi} \triangleright \Delta_2, a : \{s/i\}A]) \\
& \circ \hat{\Xi}_{[\sigma]} \left( \varsigma \circ (\text{id} \otimes \mathbf{m}_{F[\Theta \vdash_c \Gamma], [\Theta \vdash_\ell \Delta'_2]}^{-1}) \right) \circ ([\Theta \mid \Gamma; \Delta'_1 \vdash_\ell [\hat{\xi}]t_1 : \exists i : \sigma. A] \otimes^{\text{eq}} \text{id}) \circ \text{split}_{\Theta, \Gamma, \Delta'_1, \Delta'_2} \\
& \quad \text{(naturality of } \psi \text{)} \\
= & \psi_F[\Theta, s : \sigma \vdash_c \Gamma] \otimes [\Theta, s : \sigma \vdash_\ell \Delta'_2, a : \{s/i\}A], [\Theta \vdash_\ell B] ([\Theta, s : \sigma \mid \Gamma; \Delta'_2, a : \{s/i\}A \vdash_\ell [\hat{\xi}]t_2 : B]) \\
& \circ \hat{\Xi}_{[\sigma]} \left( \varsigma \circ (\text{id} \otimes \mathbf{m}_{F[\Theta \vdash_c \Gamma], [\Theta \vdash_\ell \Delta'_2]}^{-1}) \right) \circ ([\Theta \mid \Gamma; \Delta'_1 \vdash_\ell [\hat{\xi}]t_1 : \exists i : \sigma. A] \otimes^{\text{eq}} \text{id}) \circ \text{split}_{\Theta, \Gamma, \Delta'_1, \Delta'_2} \\
& \quad \text{(IH on } t_2 \text{)} \\
= & [\Theta \mid \Gamma; \Delta'_1, \Delta'_2 \vdash_\ell \text{let } \{s, a\} = [\hat{\xi}]t_1 \text{ in } [\hat{\xi}]t_2 : B] \quad \text{(semantics of let } \{s, a\} = [\hat{\xi}]t_1 \text{ in } [\hat{\xi}]t_2 : B \text{)} \\
= & [\Theta \mid \Gamma; \Delta'_1, \Delta'_2 \vdash_\ell [\hat{\xi}](\text{let } \{s, a\} = t_1 \text{ in } t_2) : B] \quad \text{(syntactic substitution)}
\end{aligned}$$

$$\begin{aligned}
& \bullet (\Theta \mid \Gamma; \Delta_1, \Delta_2 \vdash_\ell \text{select } (t_1, t_2) \text{ as } [a_1 \mapsto t'_1] \parallel [a_2 \mapsto t'_2] : \Diamond C): \\
& \quad \llbracket \Theta \mid \Gamma; \Delta_1, \Delta_2 \vdash_\ell \text{select } (t_1, t_2) \text{ as } [a_1 \mapsto t'_1] \parallel [a_2 \mapsto t'_2] : \Diamond C \rrbracket \circ (\text{id}_{F[\Theta \vdash_c \Gamma]} \otimes \llbracket \hat{\xi}_1, \hat{\xi}_2 \rrbracket) \\
& = \mu_{[\Theta \vdash_\ell C]} \circ \Diamond(\llbracket t'_1 \rrbracket, \llbracket t'_2 \rrbracket) \circ \text{dist} \circ \text{st}^F \circ (\text{id}_{F[\Theta \vdash_c \Gamma]} \otimes \text{race}_{[\Theta \vdash_\ell A], [\Theta \vdash_\ell B]}) \circ (\text{id}_{F[\Theta \vdash_c \Gamma]} \otimes \llbracket t_1 \rrbracket \otimes \llbracket t_2 \rrbracket) \\
& \quad \circ (\text{split}_{\Theta, \Gamma, \Delta_1, \Delta_2} \otimes \text{id}_{F[\Theta \vdash_c \Gamma]}) \circ \varsigma \circ (\text{dup}_{[\Theta \vdash_c \Gamma]} \otimes \text{id}) \circ (\text{id}_{F[\Theta \vdash_c \Gamma]} \otimes \llbracket \hat{\xi}_1, \hat{\xi}_2 \rrbracket) \quad (\text{semantics of select}) \\
& = \mu_{[\Theta \vdash_\ell C]} \circ \Diamond(\llbracket t'_1 \rrbracket, \llbracket t'_2 \rrbracket) \circ \text{dist} \circ \text{st}^F \circ (\text{id}_{F[\Theta \vdash_c \Gamma]} \otimes \text{race}_{[\Theta \vdash_\ell A], [\Theta \vdash_\ell B]}) \circ (\text{id}_{F[\Theta \vdash_c \Gamma]} \otimes \llbracket t_1 \rrbracket \otimes \llbracket t_2 \rrbracket) \\
& \quad \circ (\text{id}_{F[\Theta \vdash_c \Gamma]} \otimes (\text{id}_{F[\Theta \vdash_c \Gamma]} \otimes \llbracket \hat{\xi}_1 \rrbracket) \otimes (\text{id}_{F[\Theta \vdash_c \Gamma]} \otimes \llbracket \hat{\xi}_2 \rrbracket)) \circ (\text{split} \otimes \text{id}_{F[\Theta \vdash_c \Gamma]}) \circ \varsigma \circ (\text{dup}_{[\Theta \vdash_c \Gamma]} \otimes \text{id}) \quad (\text{naturality}) \\
& = \mu_{[\Theta \vdash_\ell C]} \circ \Diamond(\llbracket t'_1 \rrbracket, \llbracket t'_2 \rrbracket) \circ \text{dist} \circ \text{st}^F \circ (\text{id}_{F[\Theta \vdash_c \Gamma]} \otimes \text{race}_{[\Theta \vdash_\ell A], [\Theta \vdash_\ell B]}) \\
& \quad \circ (\text{id}_{F[\Theta \vdash_c \Gamma]} \otimes (\llbracket \Theta \mid \Gamma; \Delta_1 \vdash_\ell t_1 : \Diamond A \rrbracket \circ (\text{id}_{F[\Theta \vdash_c \Gamma]} \otimes \llbracket \hat{\xi}_1 \rrbracket))) \otimes (\llbracket \Theta \mid \Gamma; \Delta_2 \vdash_\ell t_2 : \Diamond B \rrbracket \circ (\text{id}_{F[\Theta \vdash_c \Gamma]} \otimes \llbracket \hat{\xi}_2 \rrbracket))) \\
& \quad \circ (\text{split}_{\Theta, \Gamma, \Delta'_1, \Delta'_2} \otimes \text{id}_{F[\Theta \vdash_c \Gamma]}) \circ \varsigma \circ (\text{dup}_{[\Theta \vdash_c \Gamma]} \otimes \text{id}) \quad (\text{bifunctionality}) \\
& = \mu_{[\Theta \vdash_\ell C]} \circ \Diamond(\llbracket t'_1 \rrbracket, \llbracket t'_2 \rrbracket) \circ \text{dist} \circ \text{st}^F \circ (\text{id}_{F[\Theta \vdash_c \Gamma]} \otimes \text{race}_{[\Theta \vdash_\ell A], [\Theta \vdash_\ell B]}) \\
& \quad \circ (\text{id}_{F[\Theta \vdash_c \Gamma]} \otimes \llbracket \Theta \mid \Gamma; \Delta'_1 \vdash_\ell [\hat{\xi}]t_1 : \Diamond A \rrbracket \otimes \llbracket \Theta \mid \Gamma; \Delta'_2 \vdash_\ell [\hat{\xi}]t_2 : \Diamond B \rrbracket) \\
& \quad \circ (\text{split}_{\Theta, \Gamma, \Delta'_1, \Delta'_2} \otimes \text{id}_{F[\Theta \vdash_c \Gamma]}) \circ \varsigma \circ (\text{dup}_{[\Theta \vdash_c \Gamma]} \otimes \text{id}) \quad (\text{IH on } t_1 \text{ and } t_2) \\
& = \llbracket \Theta \mid \Gamma'; \Delta_1, \Delta_2 \vdash_\ell \text{select } ([\hat{\xi}]t_1, [\hat{\xi}]t_2) \text{ as } [a_1 \mapsto t'_1] \parallel [a_2 \mapsto t'_2] : \Diamond C \rrbracket \quad (\text{semantics of select}) \\
& = \llbracket \Theta \mid \Gamma'; \Delta_1, \Delta_2 \vdash_\ell [\hat{\xi}](\text{select } (t_1, t_2) \text{ as } [a_1 \mapsto t'_1] \parallel [a_2 \mapsto t'_2]) : \Diamond C \rrbracket \quad (\text{syntactic substitution})
\end{aligned}$$

□
